# Supplementary material for: On Inductive Biases That Enable Generalization of Diffusion Transformers
Source: arXiv:2410.21273 source file (2024-10-28)
Supplement: Supplementary file 6 [file raw_psnr.tex]

\begin{table}[ht]
\centering
\small
\setlength\tabcolsep{1pt}
\setlength{\extrarowheight}{4pt}
\begin{tabular}{lc|c}
\cellcolor{dit}{\STAB{\rotatebox[origin=c]{90}{DiT-XS/1}}}
&
\raisebox{-0.5\height}{\includegraphics[width=.54\textwidth]{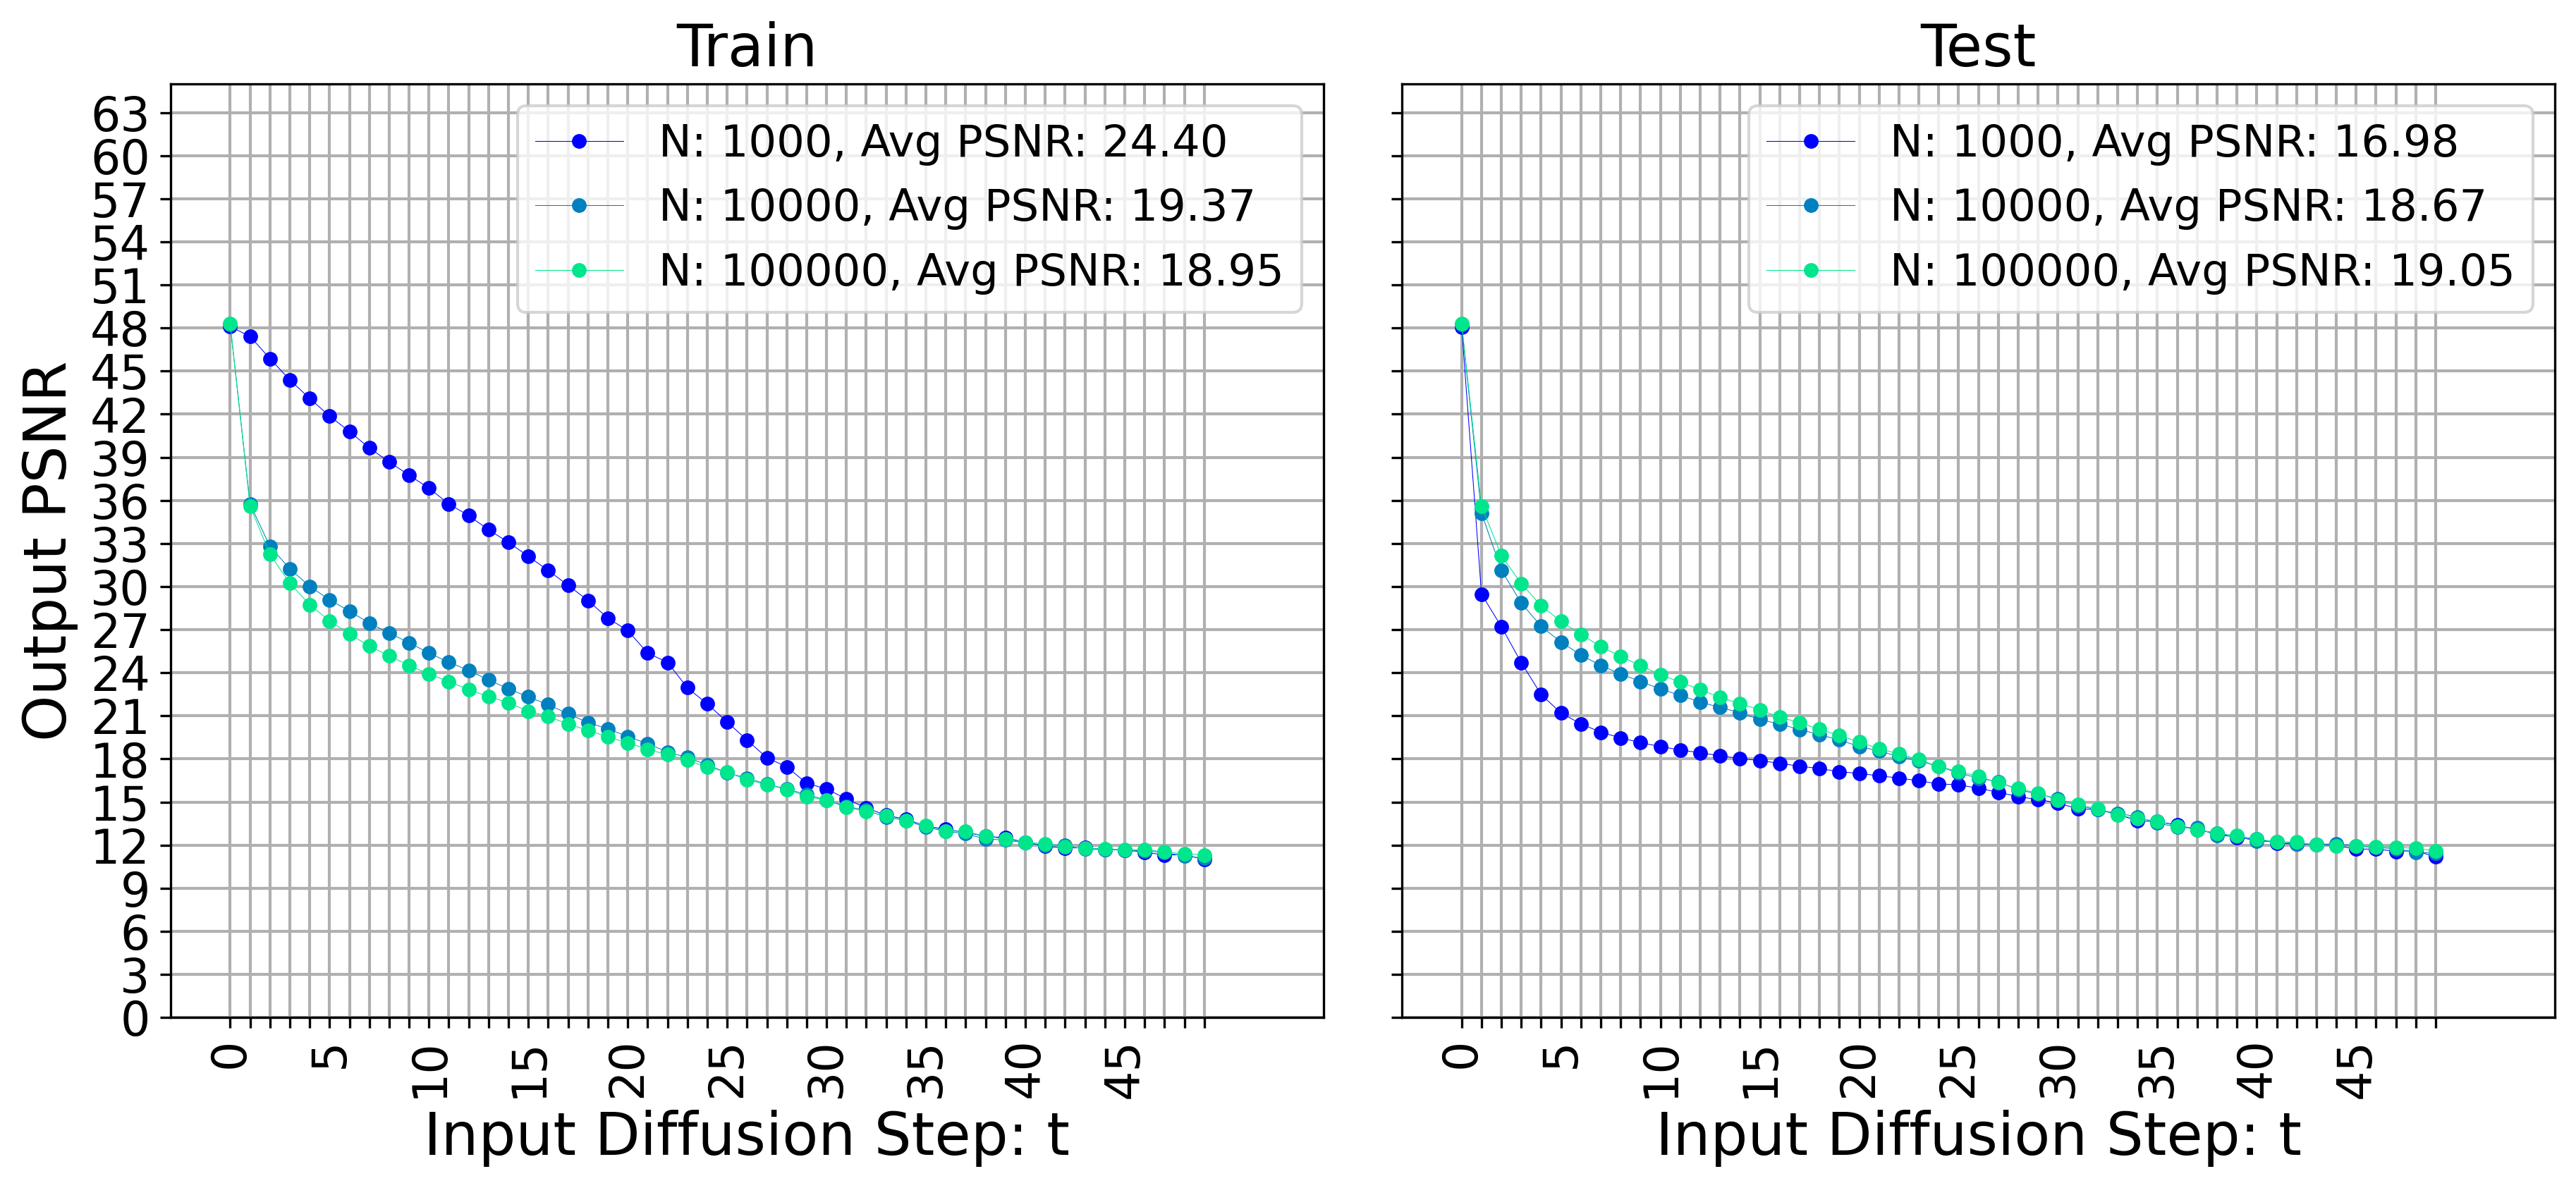}}
&
\raisebox{-0.5\height}{\includegraphics[width=.41\textwidth]{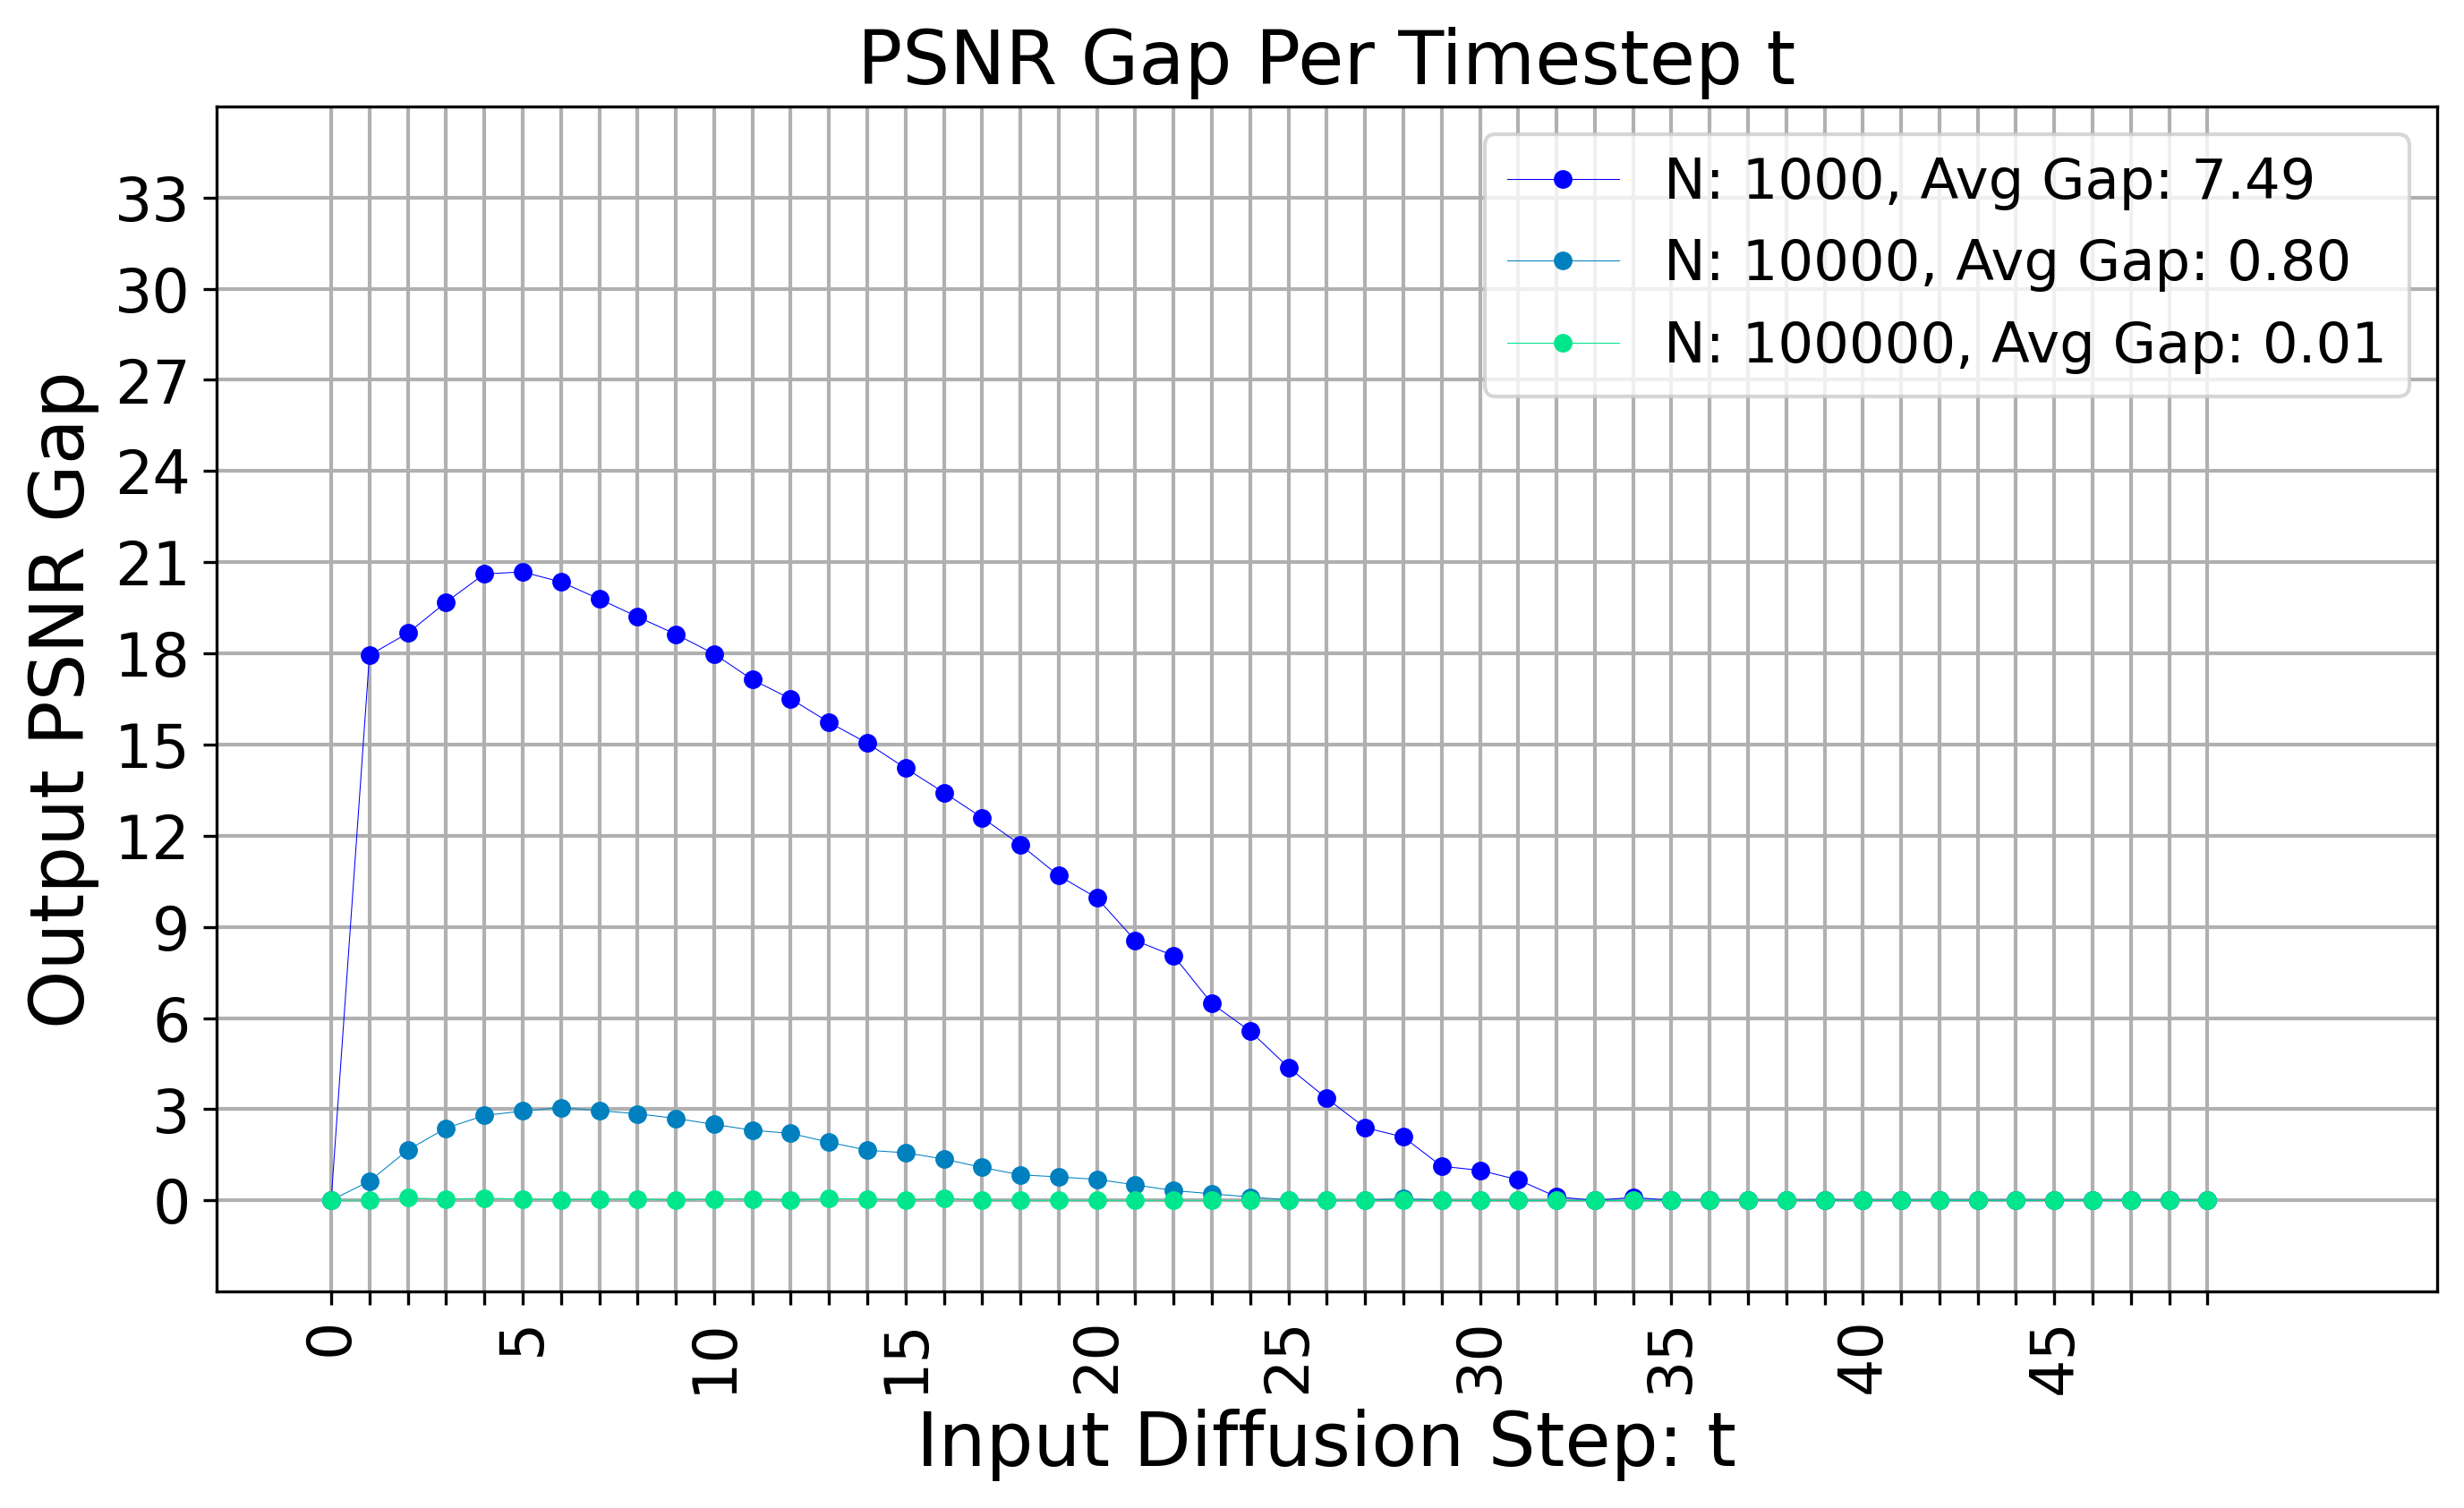}}
\\
\hline
\cellcolor{diff}{\STAB{\rotatebox[origin=c]{90}{DiT-XS/1 w/ Local}}}
&
\raisebox{-0.5\height}{\includegraphics[width=.54\textwidth]{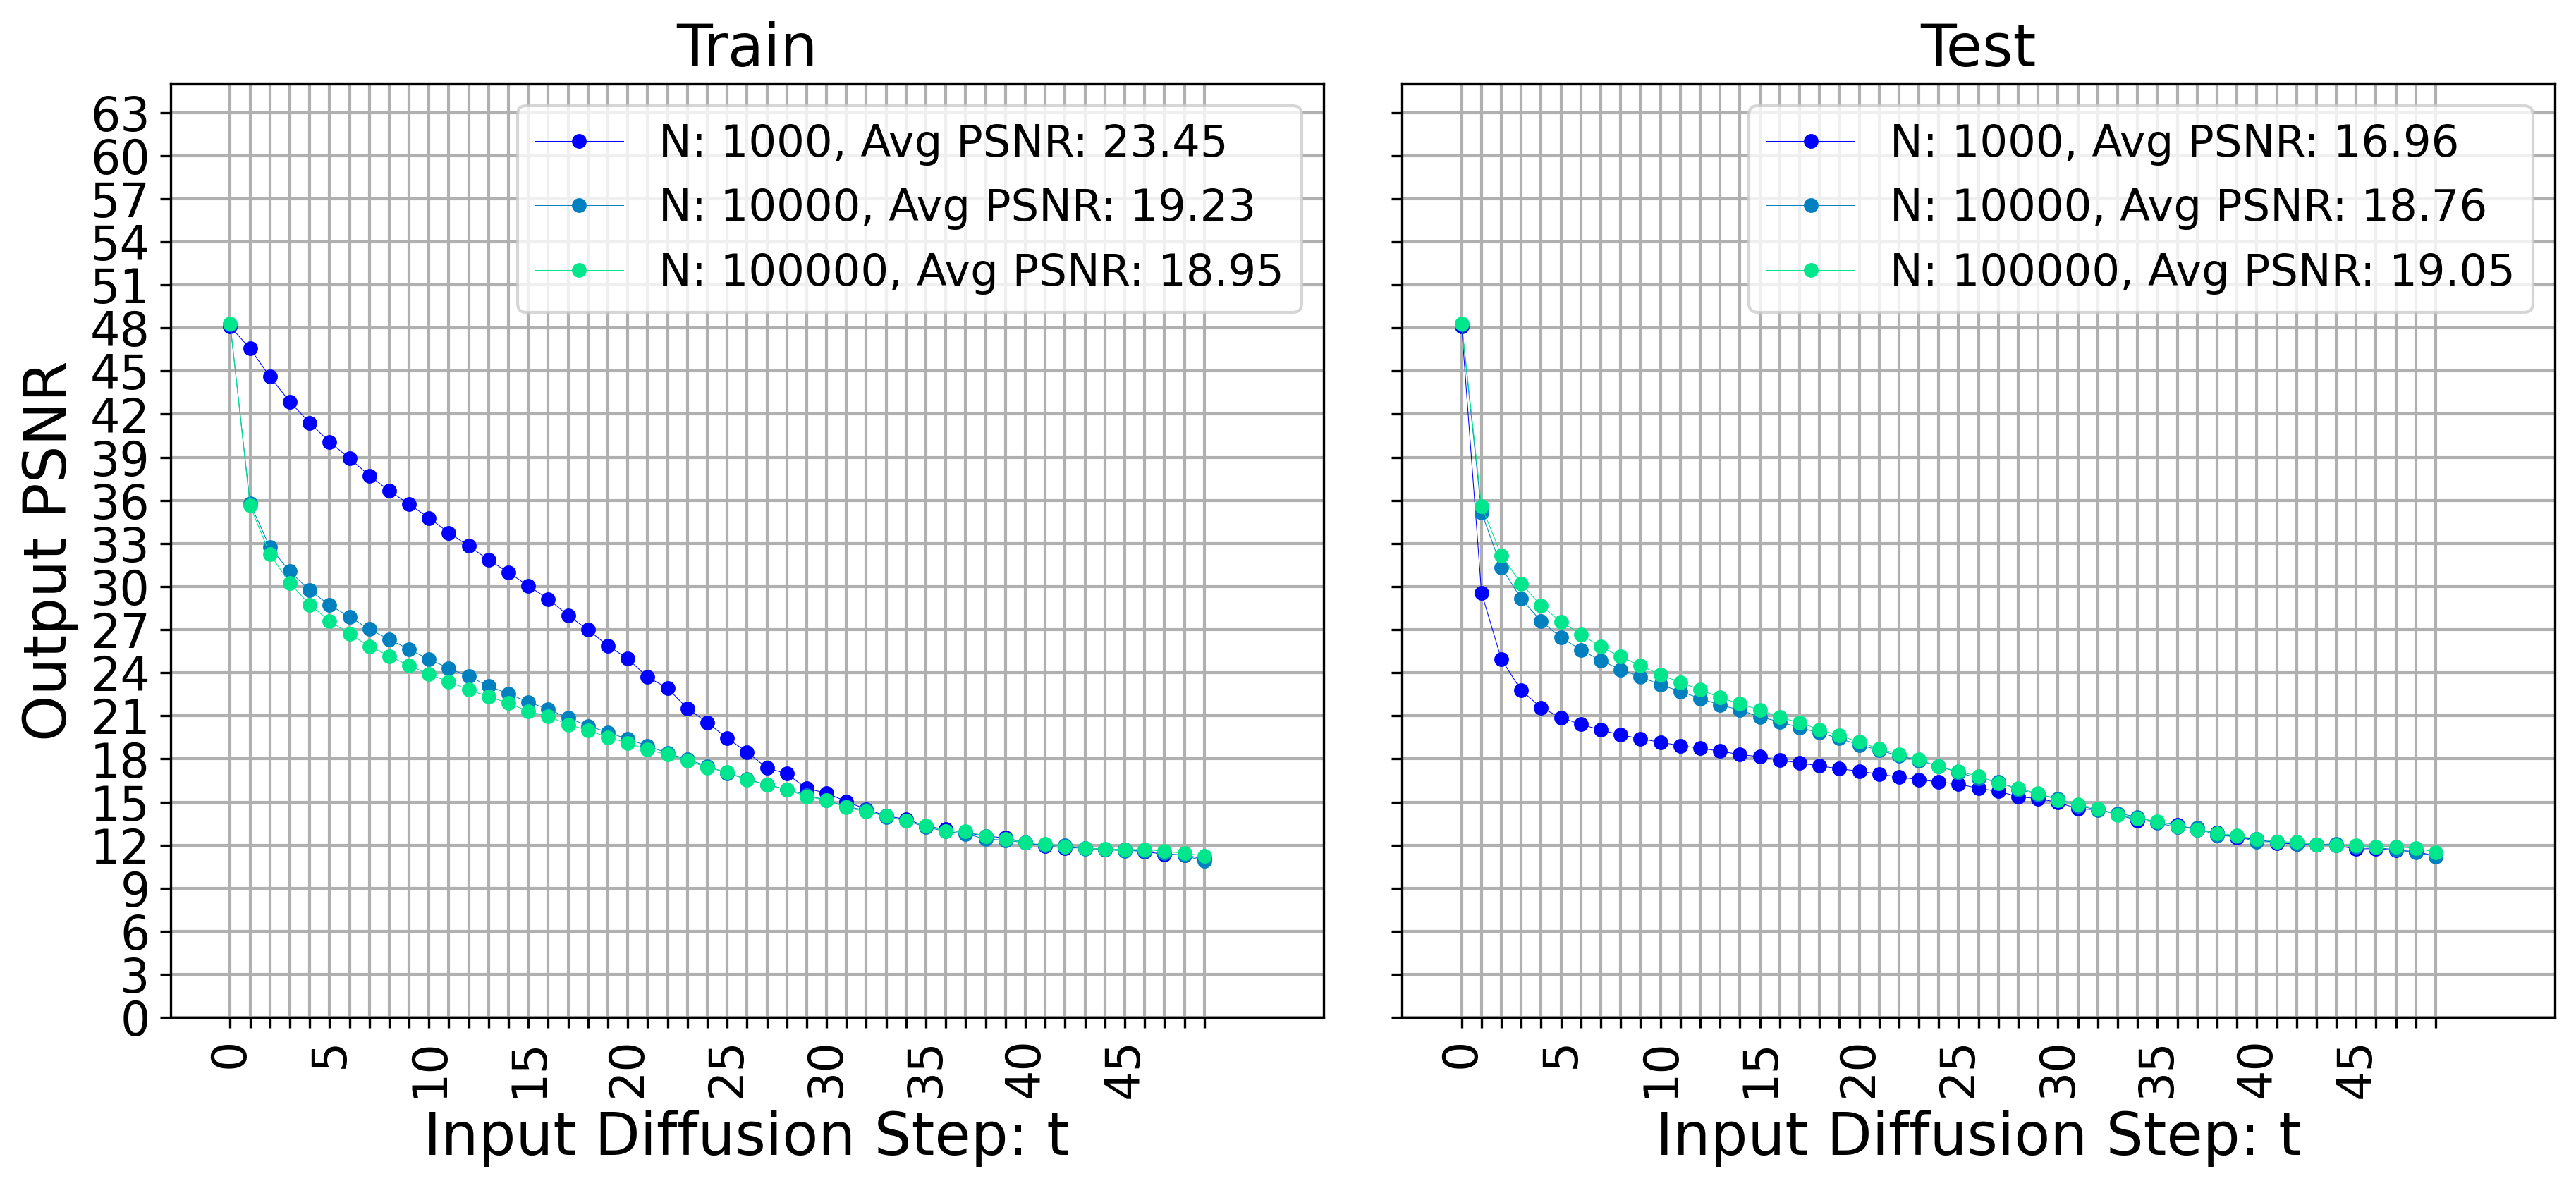}}
&
\raisebox{-0.5\height}{\includegraphics[width=.41\textwidth]{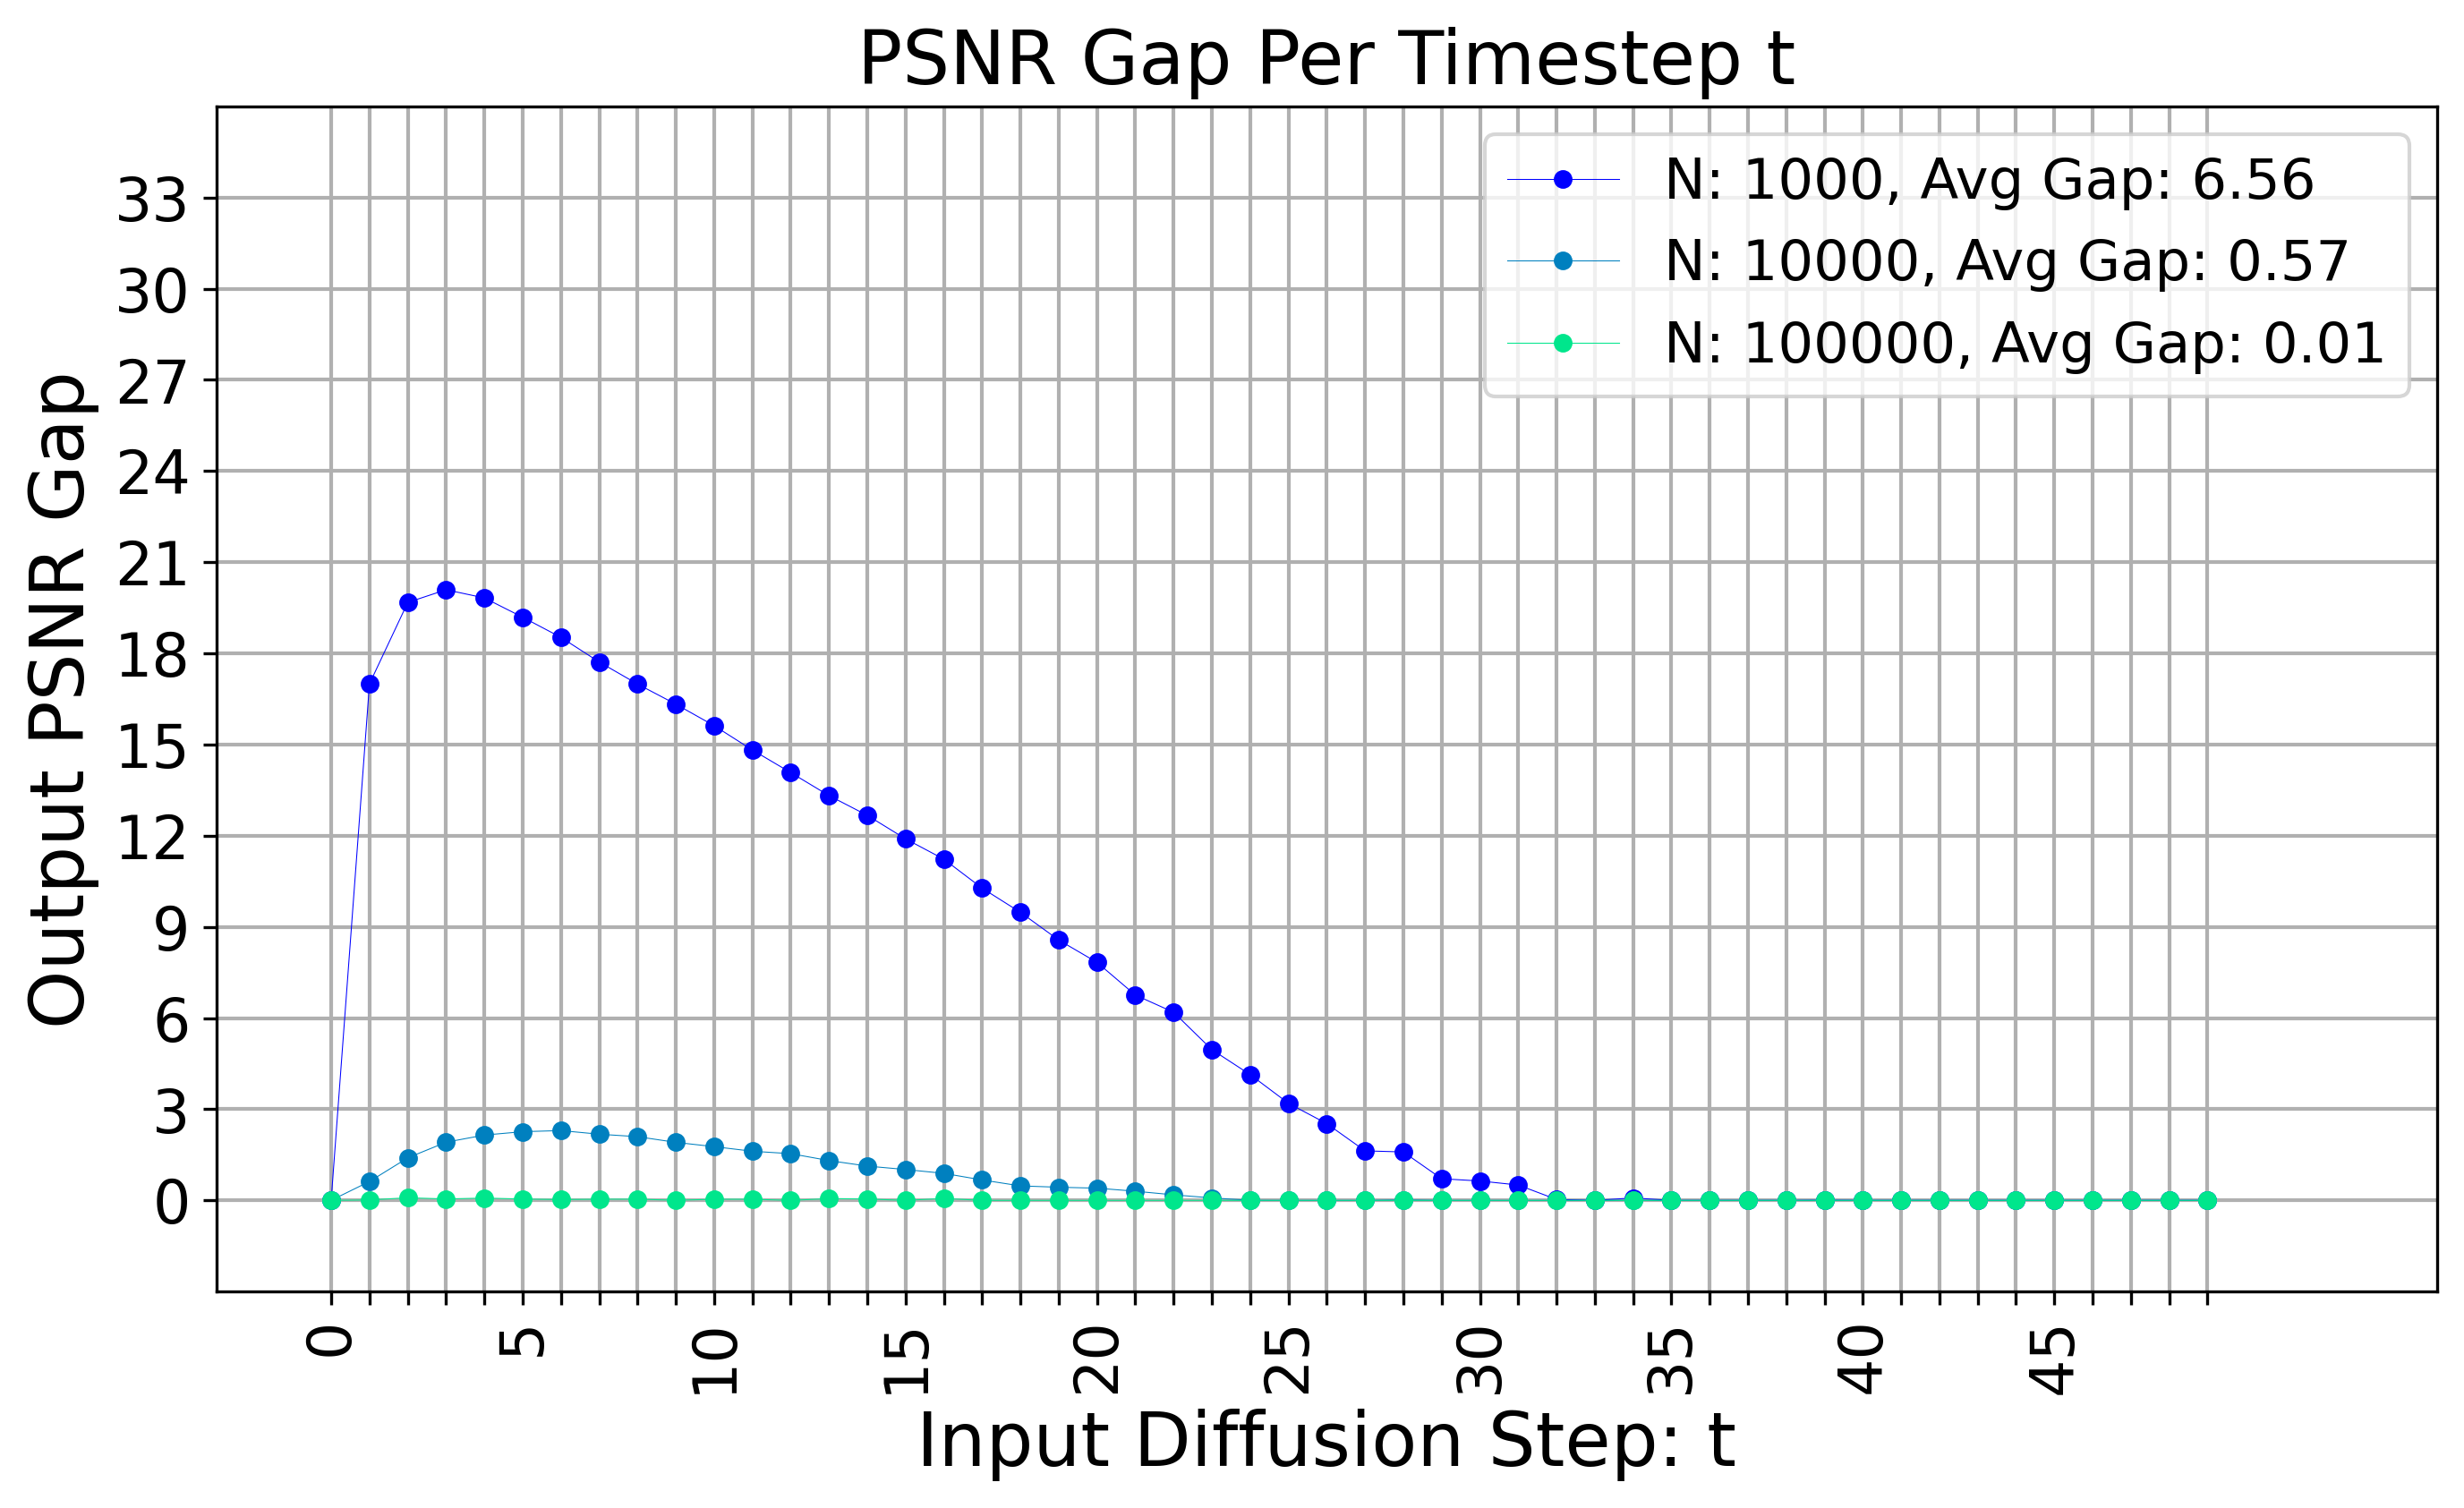}}
\\
\hline
\cellcolor{dit}{\STAB{\rotatebox[origin=c]{90}{DiT-S/1}}}
&
\raisebox{-0.5\height}{\includegraphics[width=.54\textwidth]{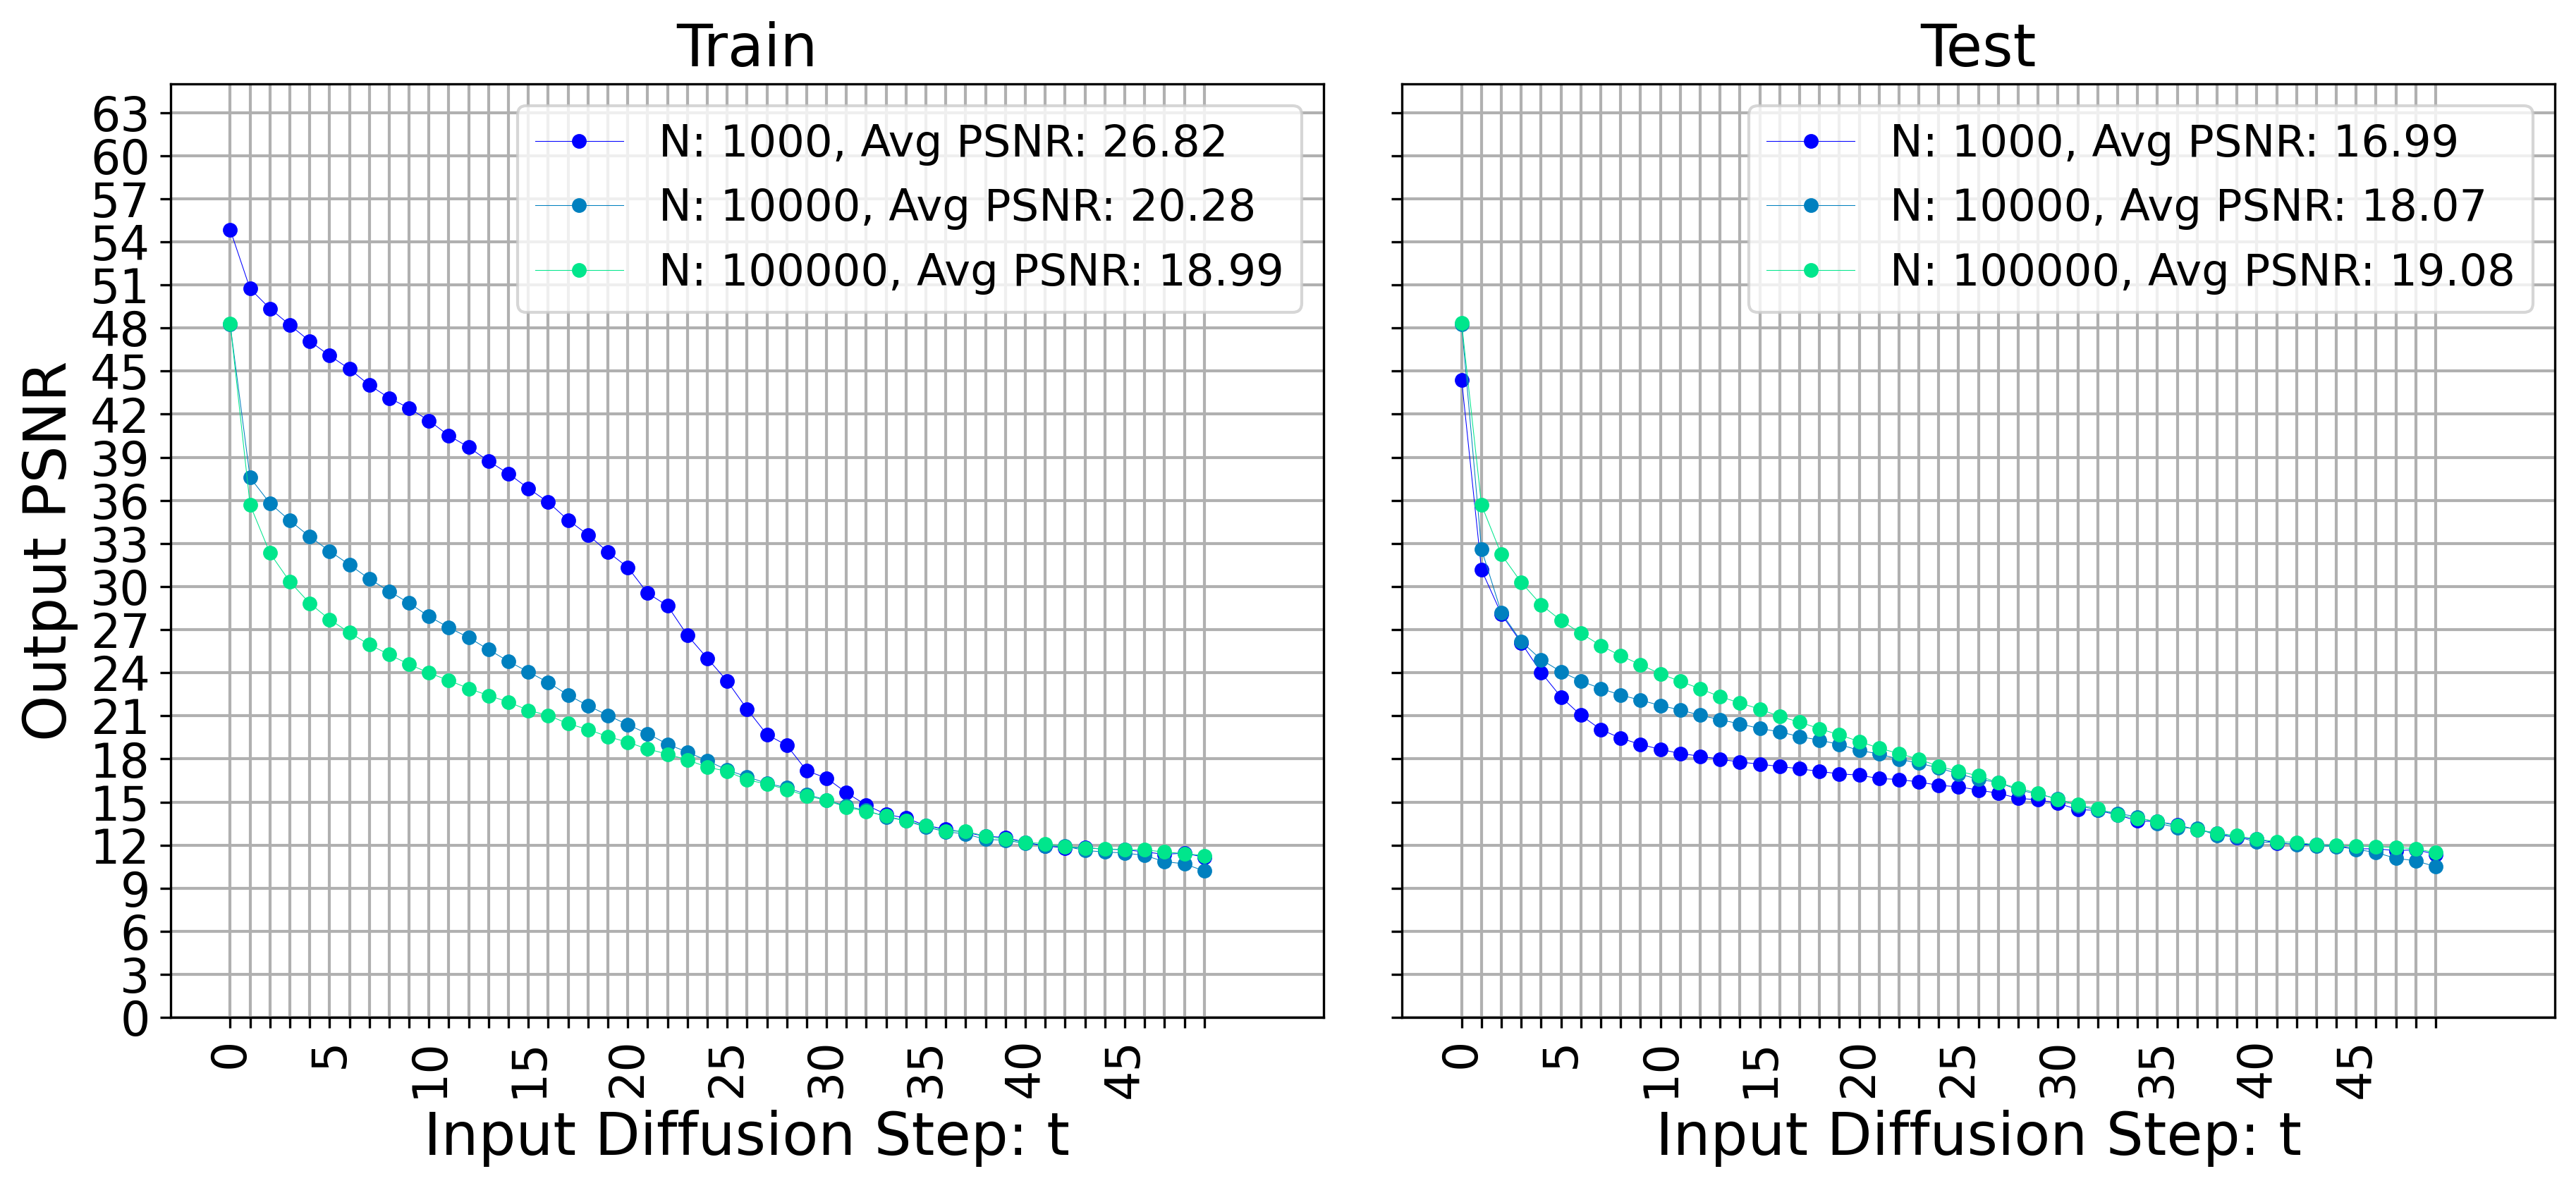}}
&
\raisebox{-0.5\height}{\includegraphics[width=.41\textwidth]{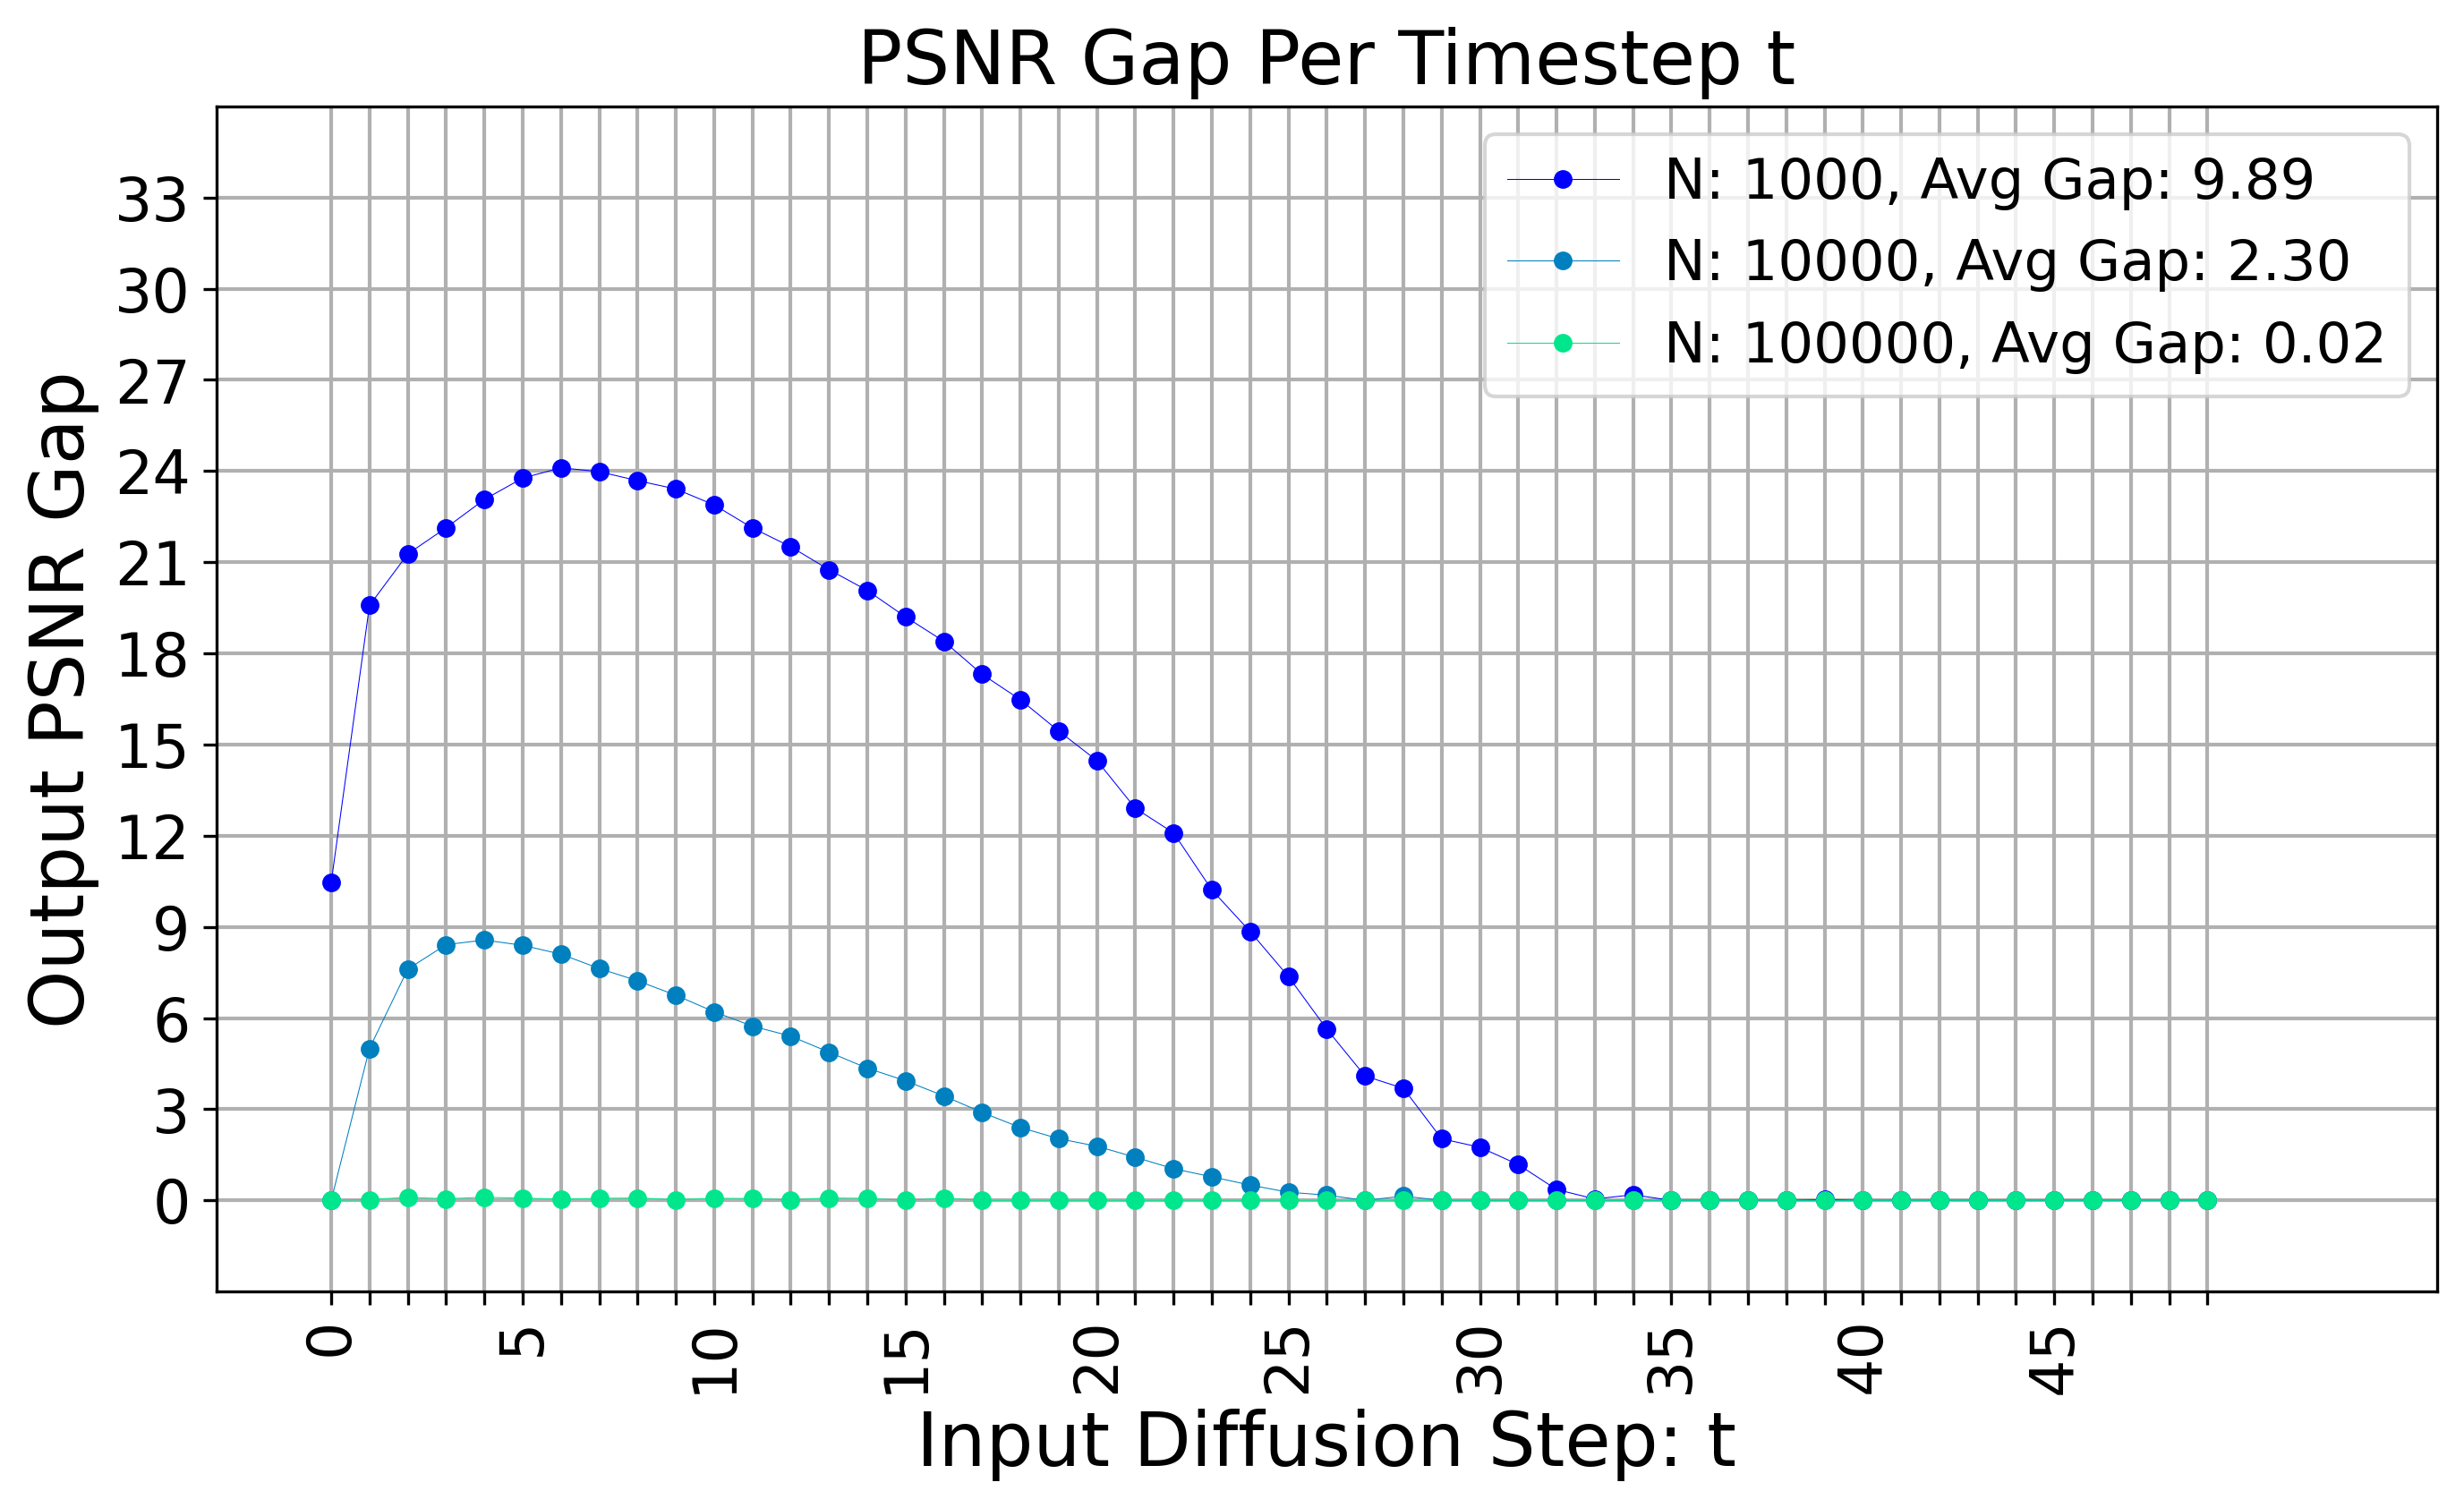}}
\\
\hline
\cellcolor{diff}{\STAB{\rotatebox[origin=c]{90}{DiT-S/1 w/ Local}}}
&
\raisebox{-0.5\height}{\includegraphics[width=.54\textwidth]{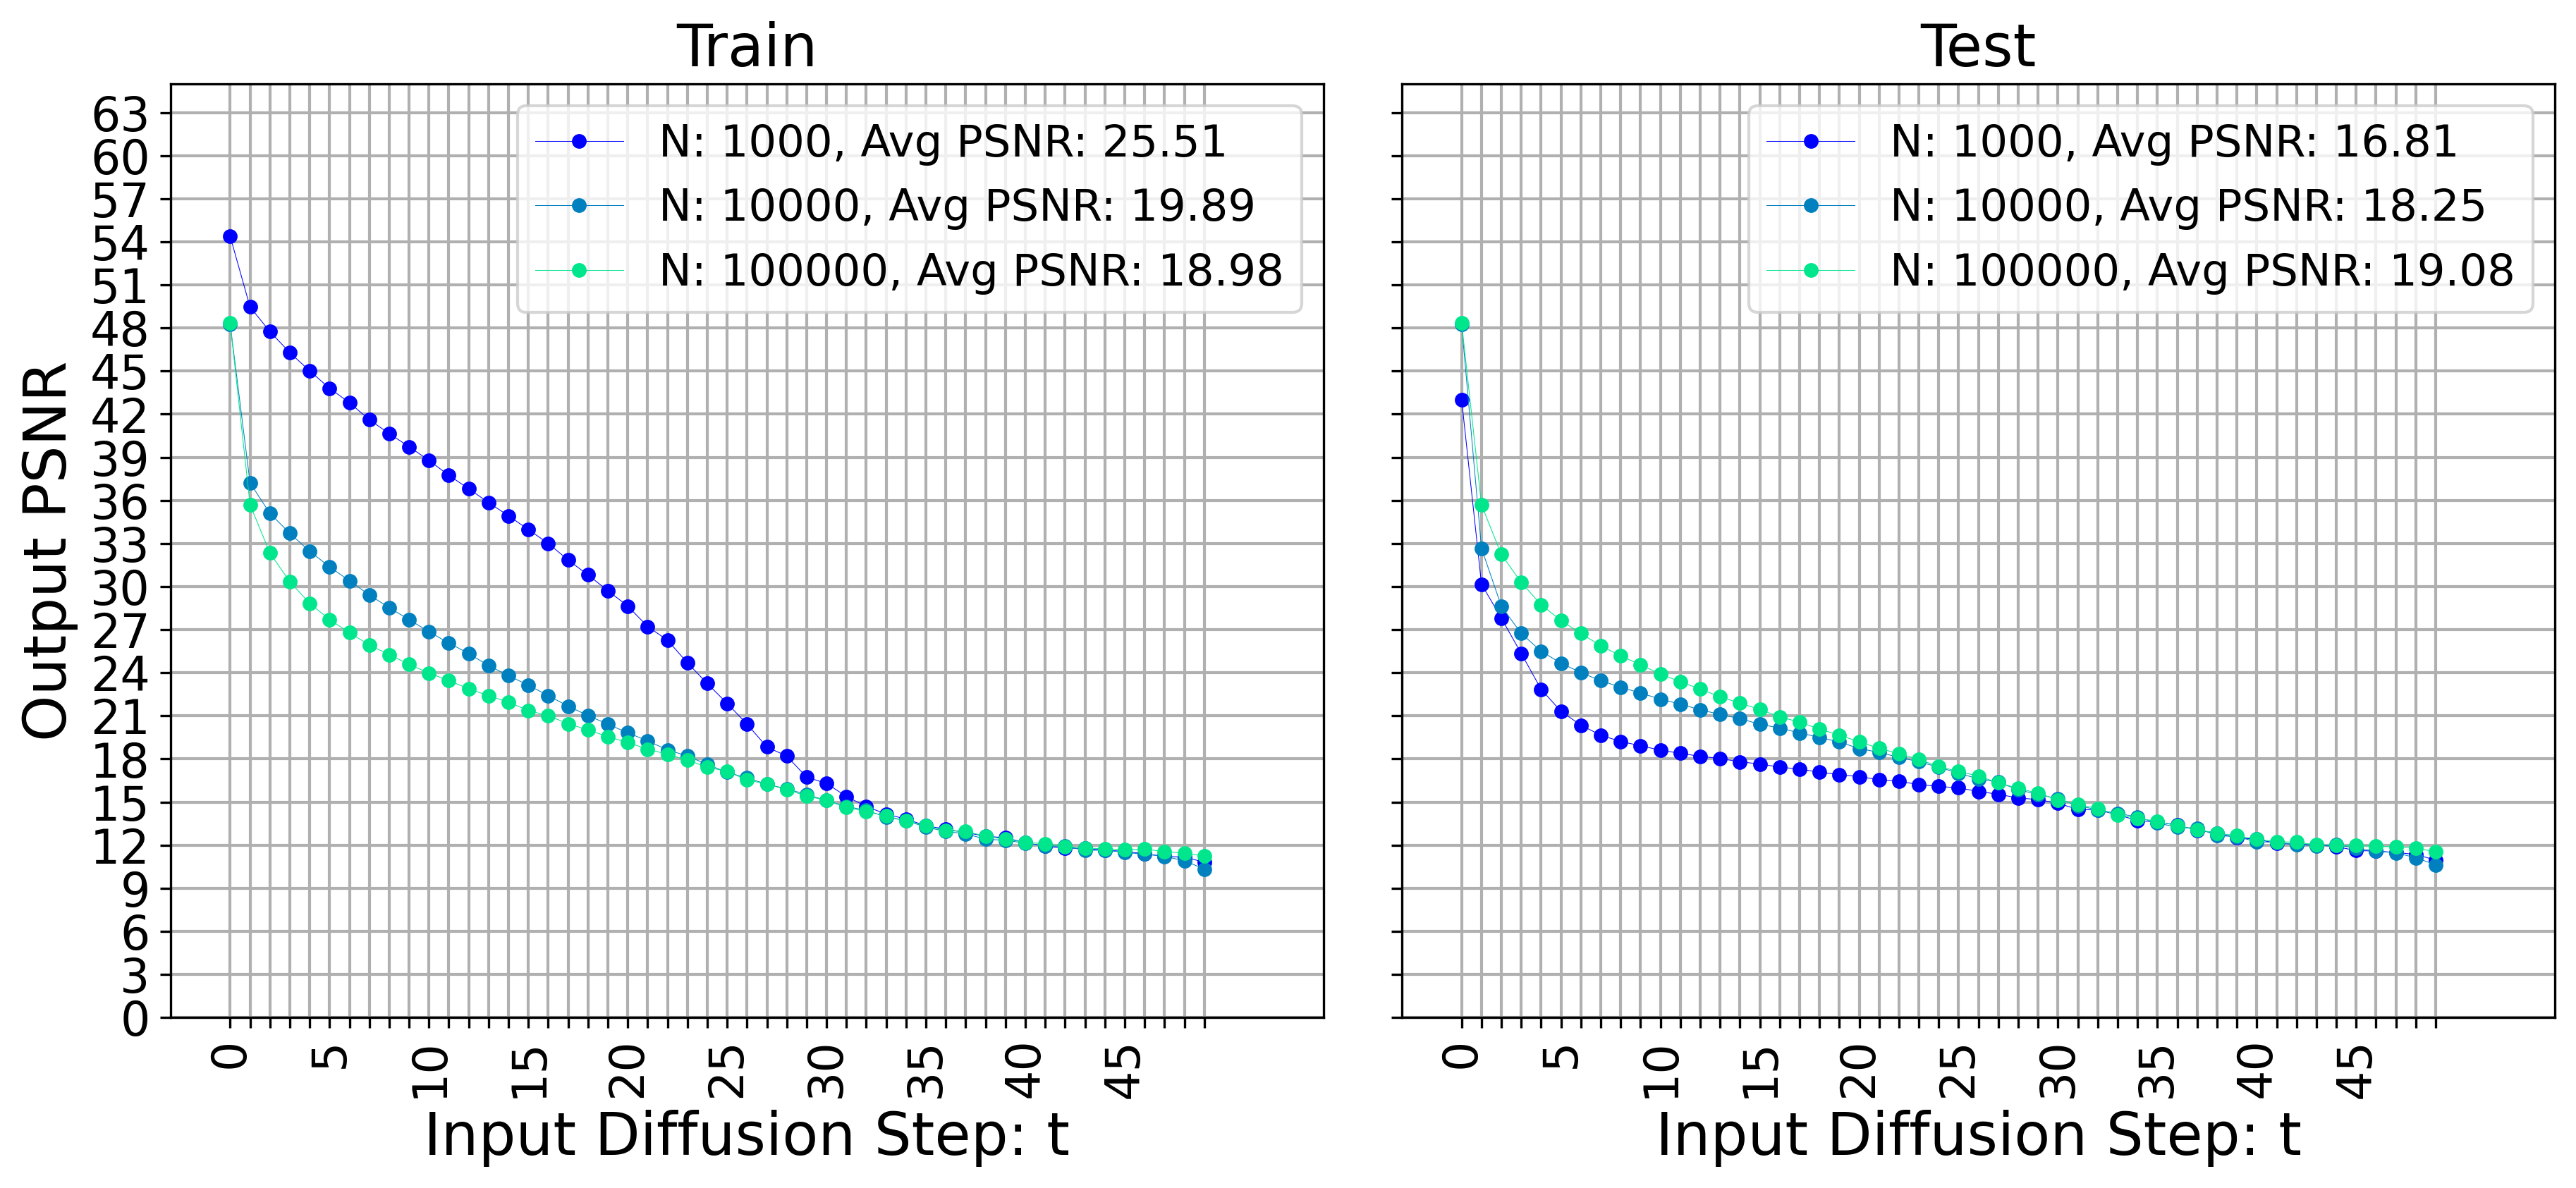}}
&
\raisebox{-0.5\height}{\includegraphics[width=.41\textwidth]{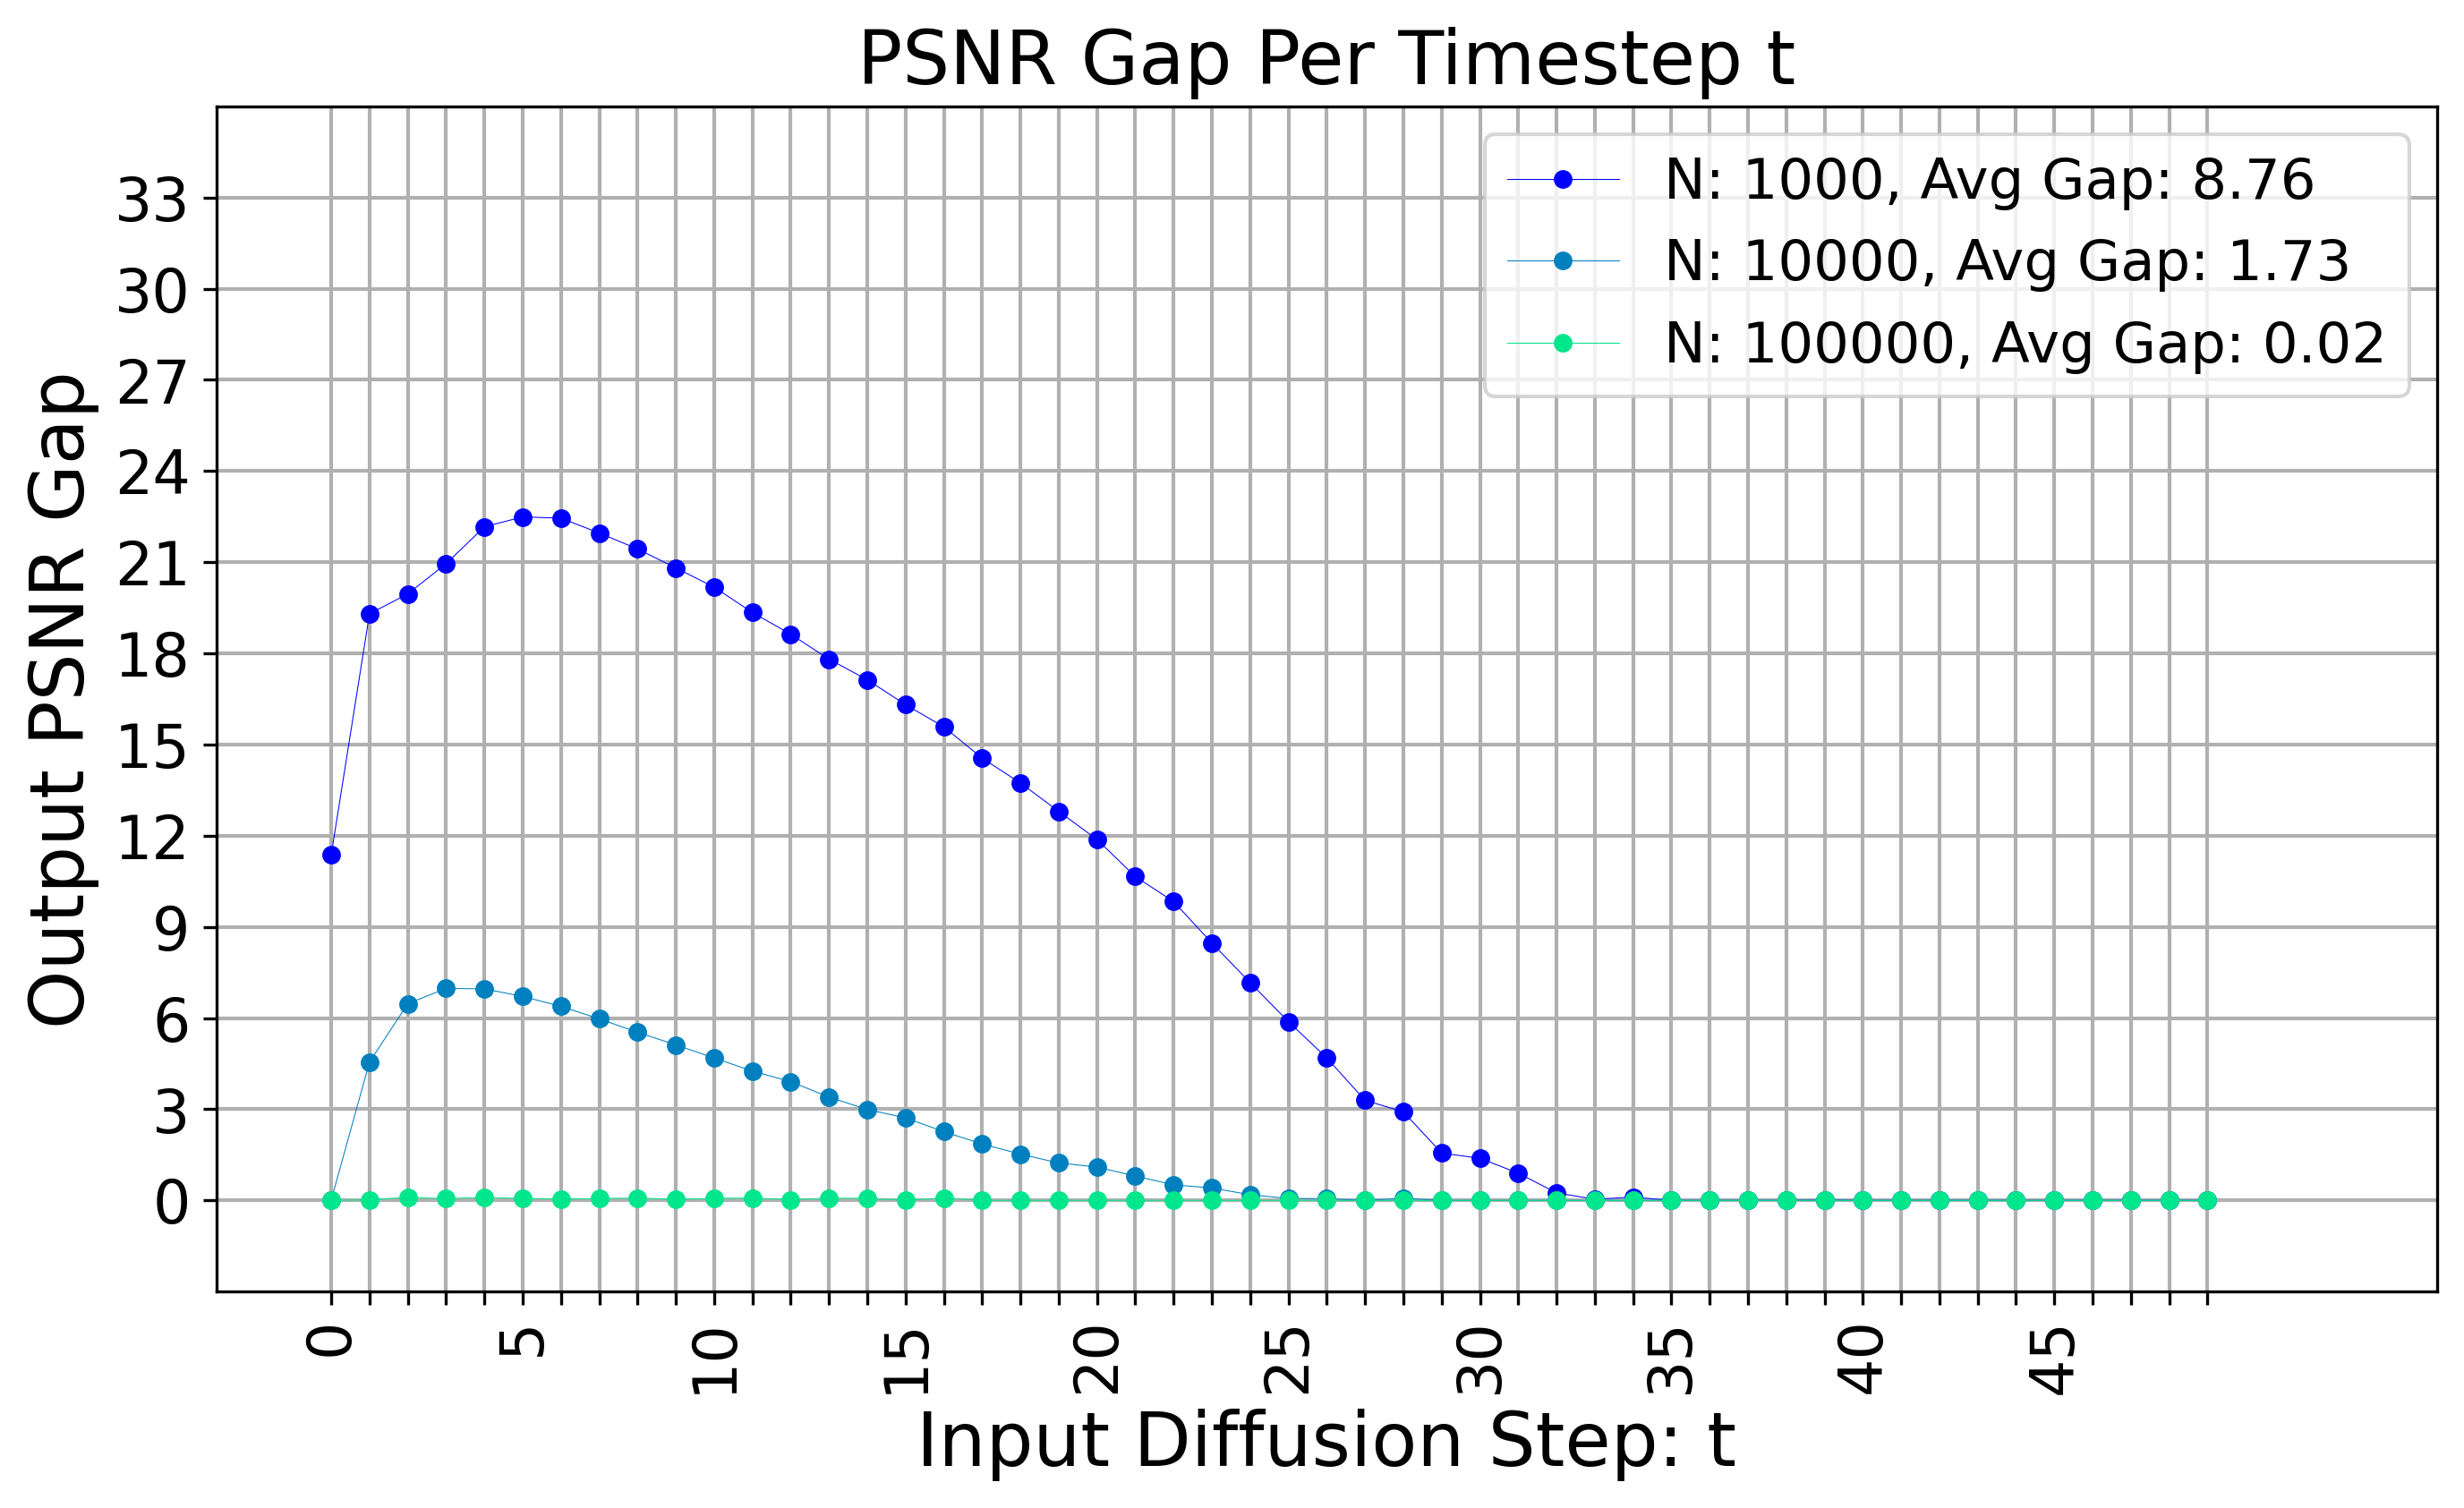}}
\\
&
\multicolumn{1}{c}{(a) PSNR Curves of Training and Testing Sets}
&
\multicolumn{1}{c}{(b) PSNR Gap}
\\
\end{tabular}

\captionof{figure}{The PSNR (a) and PSNR gap (b) comparison on the CelebA~\citep{liu2015faceattributes} dataset.}
\label{fig:row_psnr_celeba}
\end{table}

\begin{table}[ht]
\centering
\small
\setlength\tabcolsep{1pt}
\setlength{\extrarowheight}{4pt}
\begin{tabular}{lc|c}
\cellcolor{dit}{\STAB{\rotatebox[origin=c]{90}{DiT-XS/1}}}
&
\raisebox{-0.5\height}{\includegraphics[width=.54\textwidth]{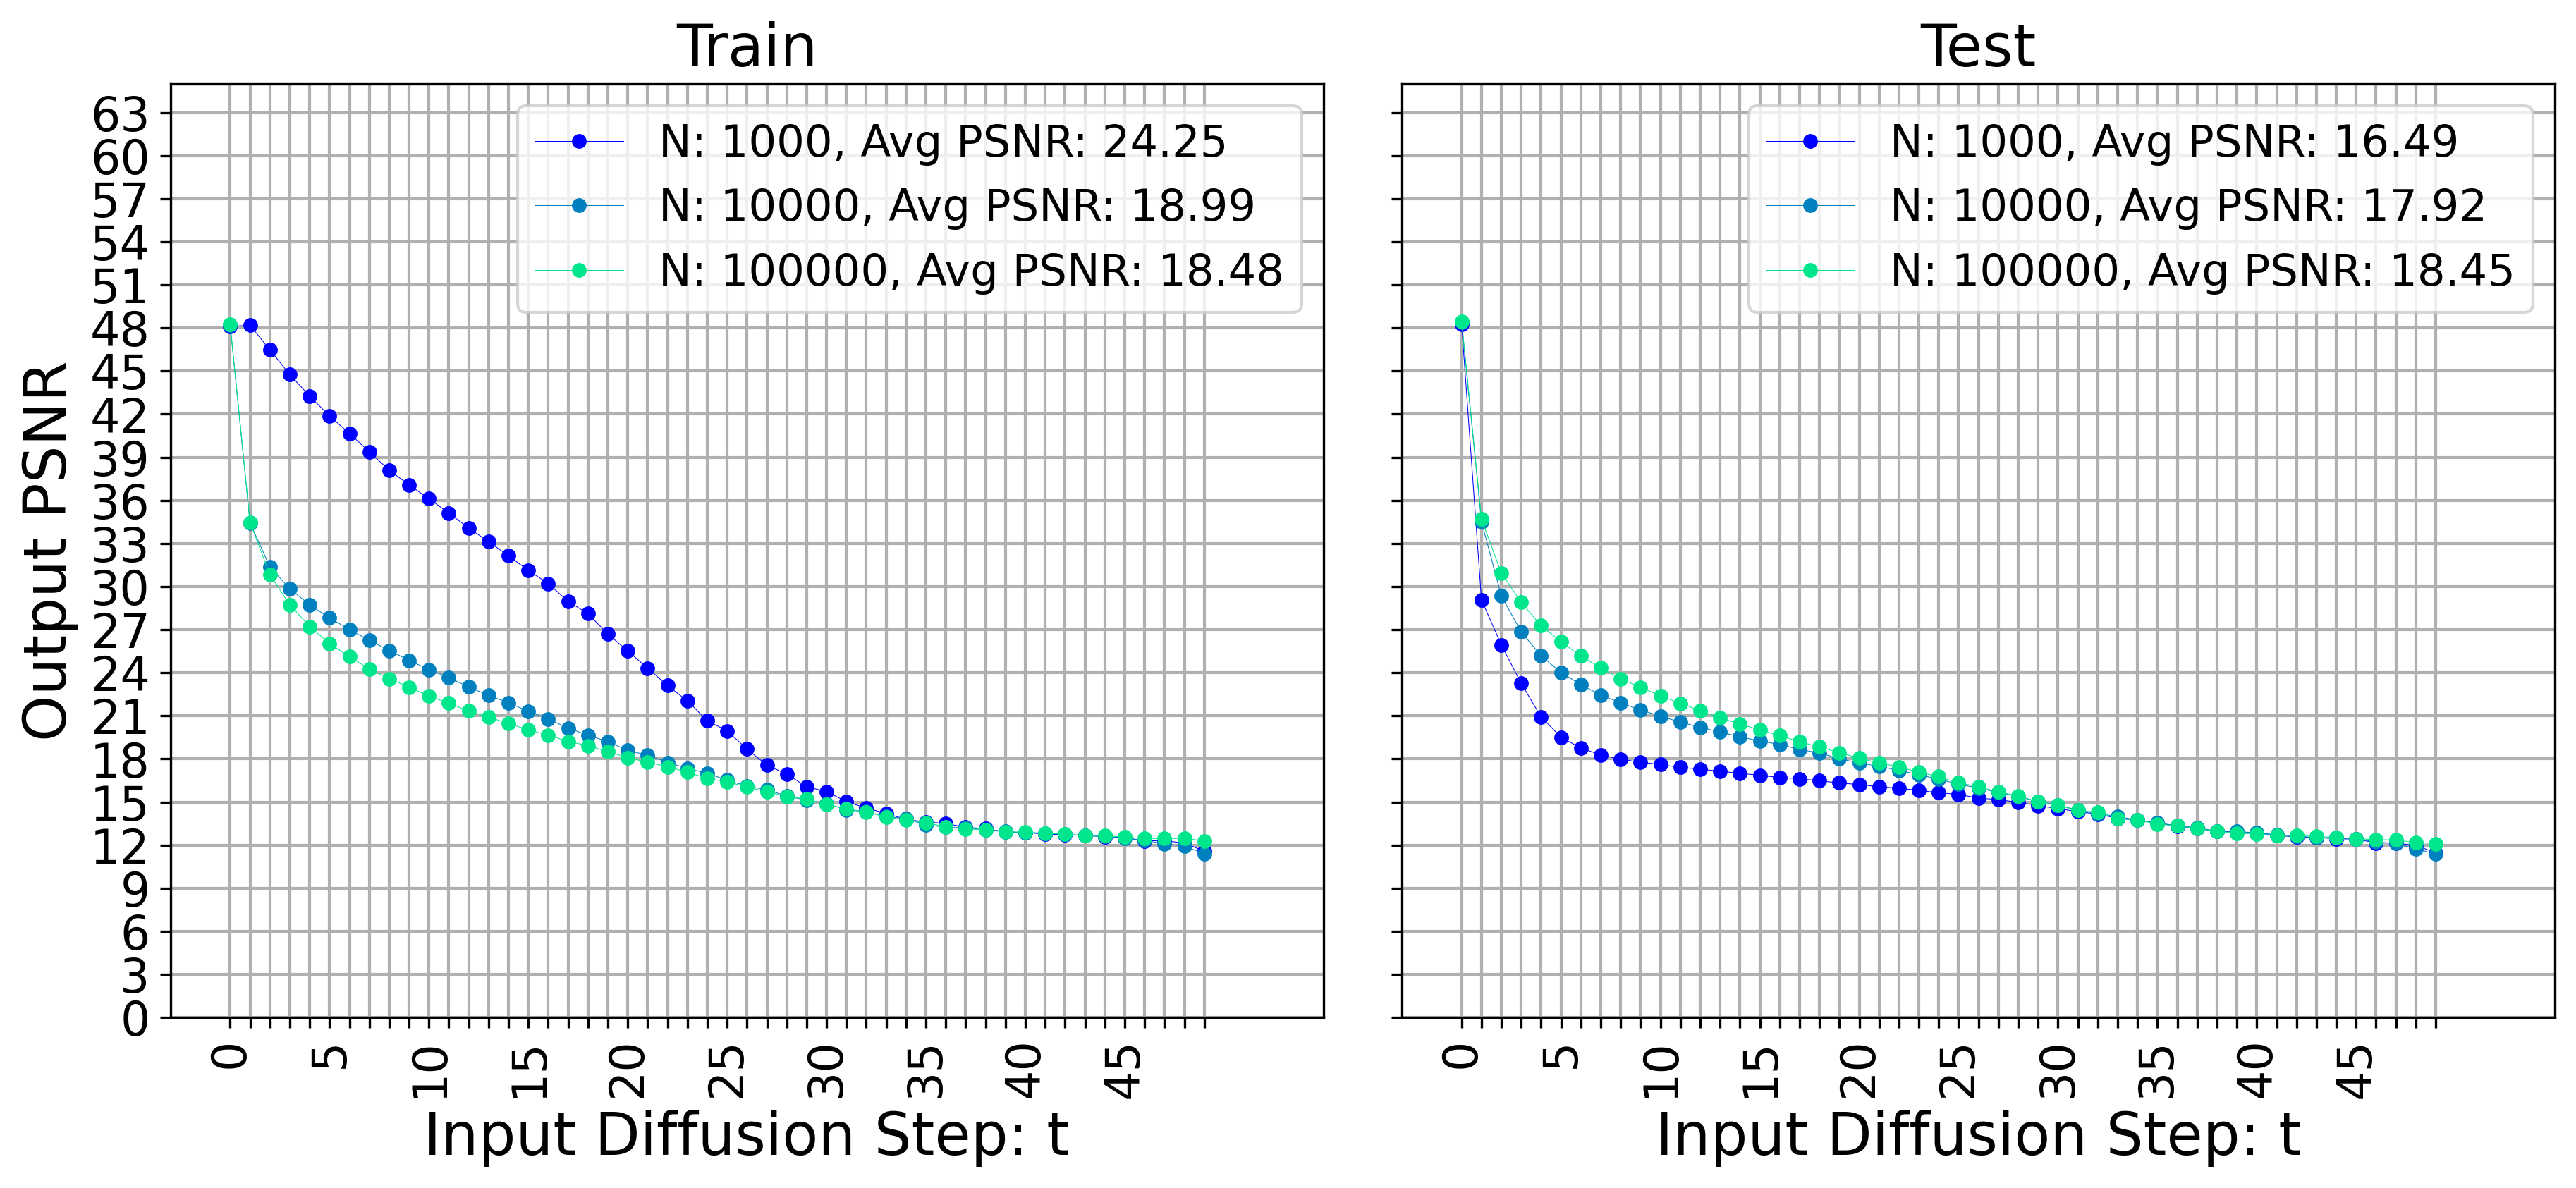}}
&
\raisebox{-0.5\height}{\includegraphics[width=.41\textwidth]{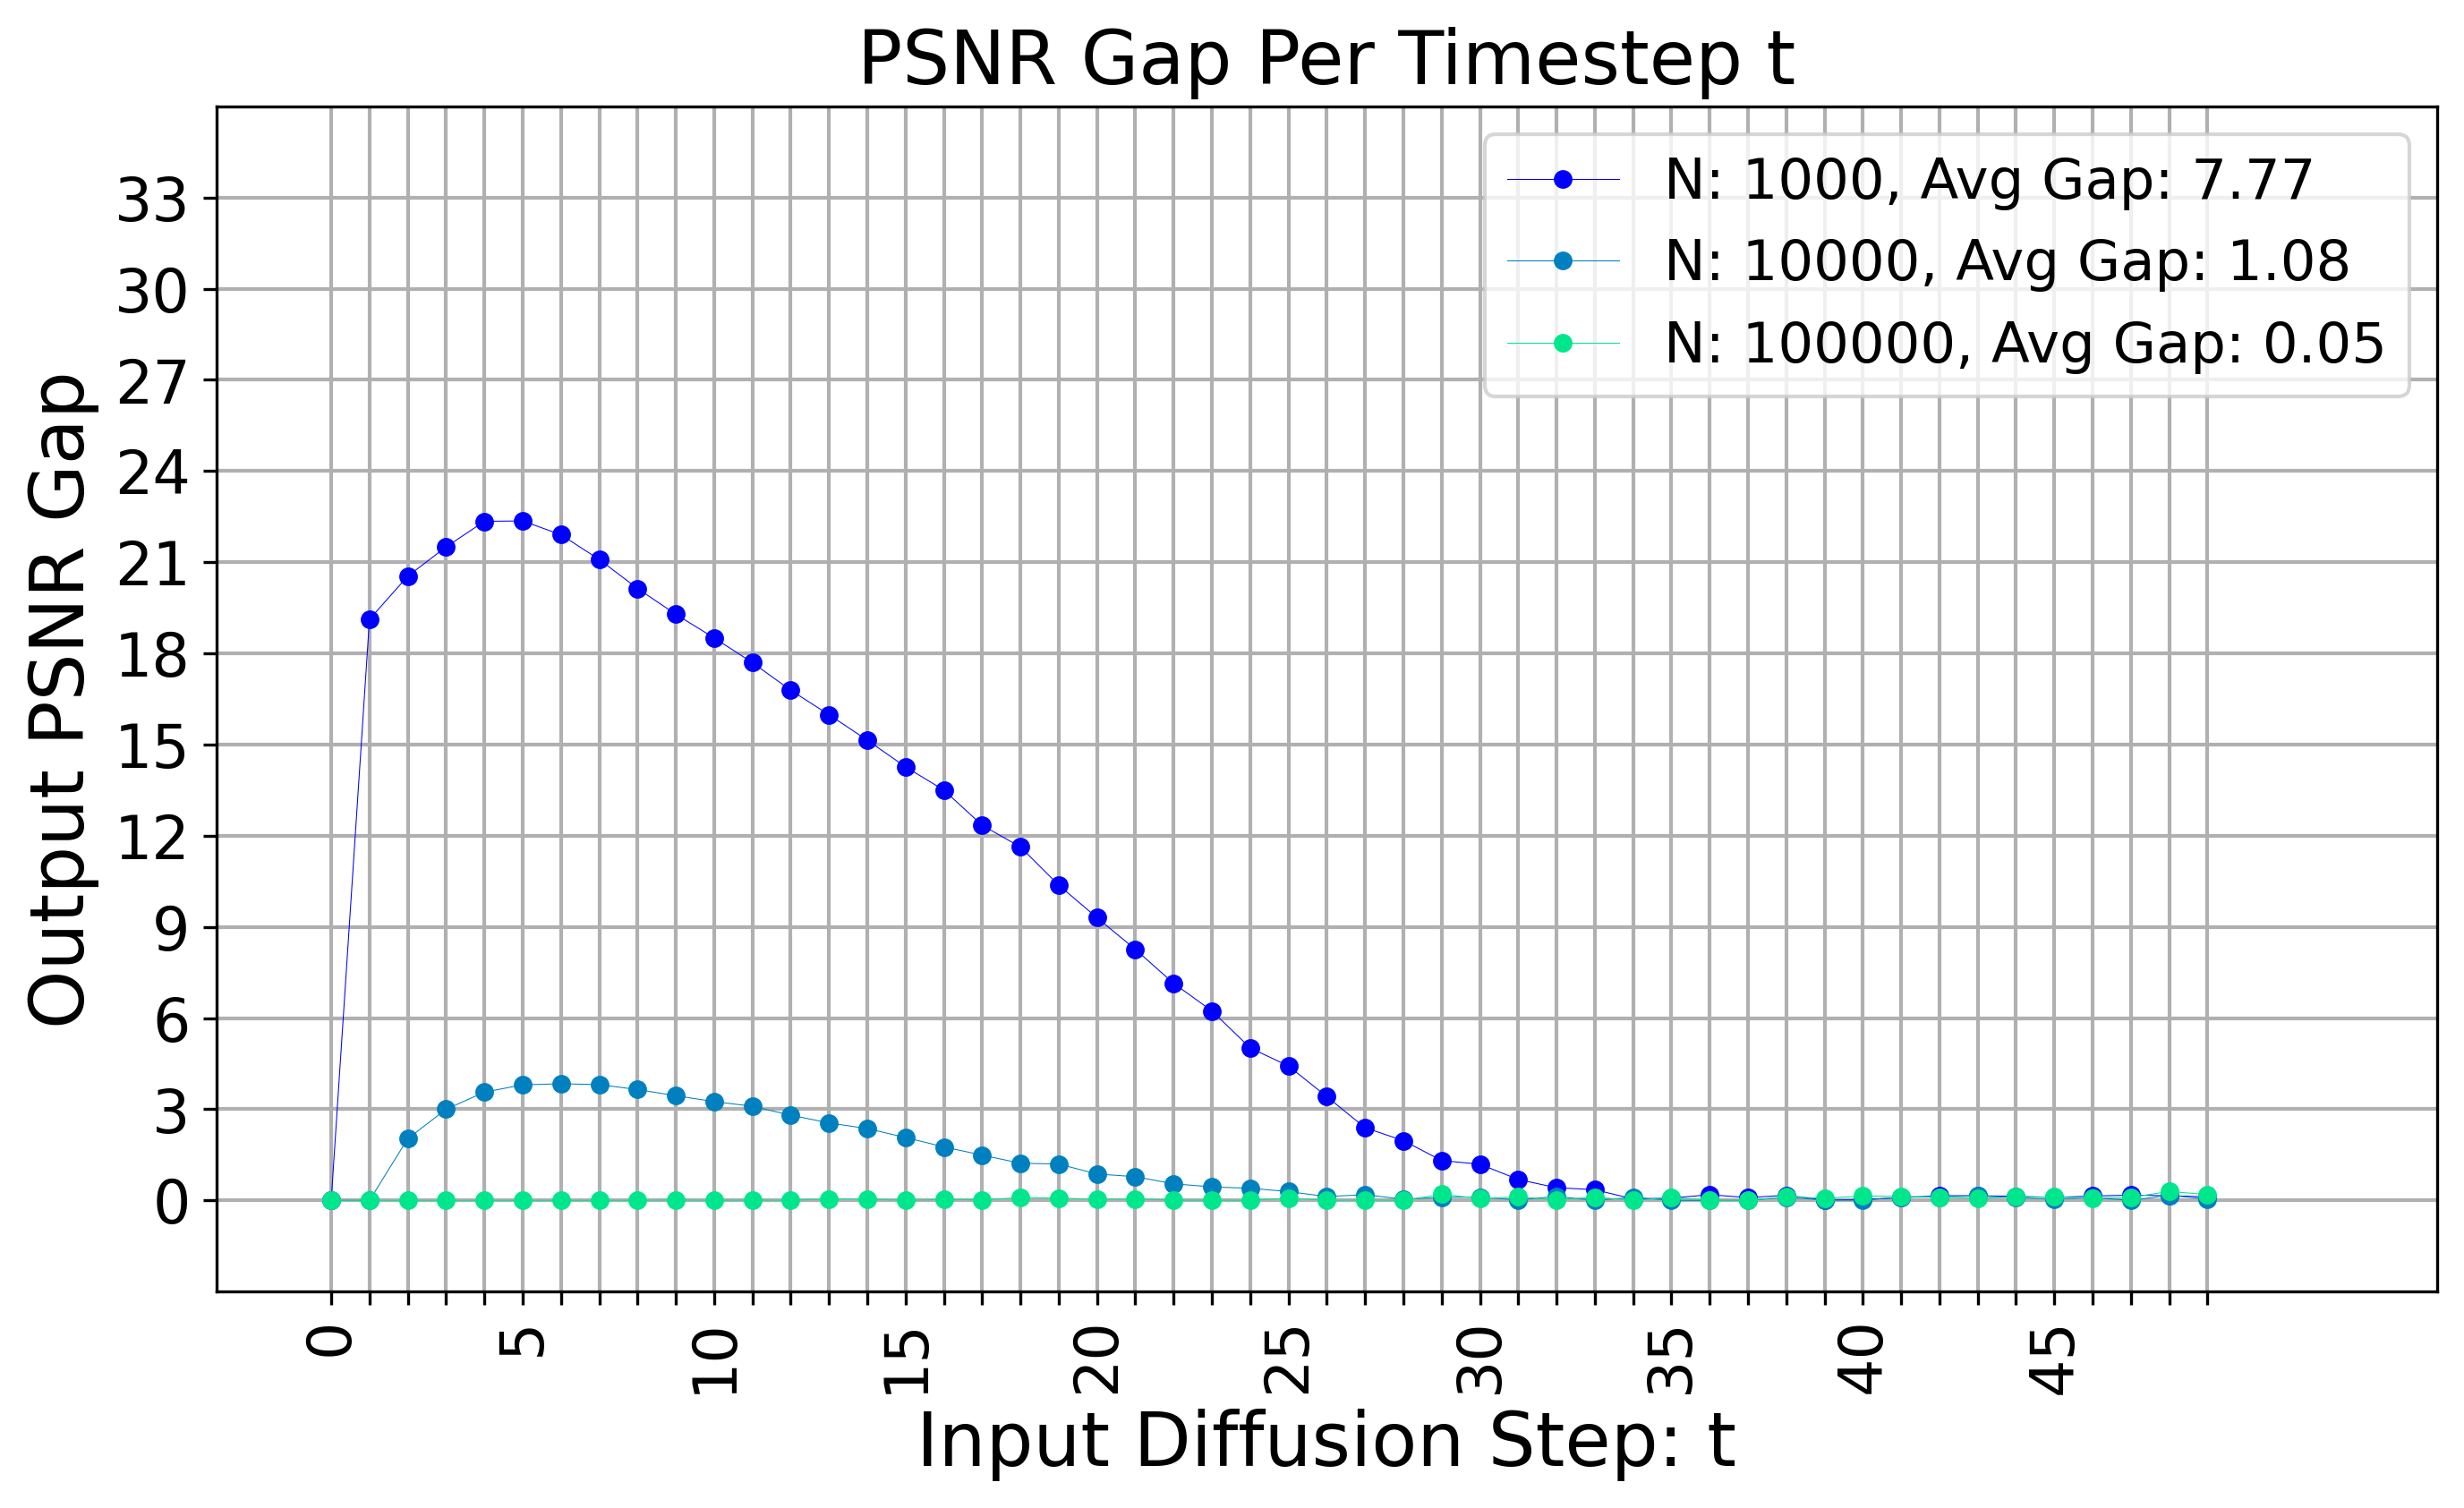}}
\\
\hline
\cellcolor{diff}{\STAB{\rotatebox[origin=c]{90}{DiT-XS/1 w/ Local}}}
&
\raisebox{-0.5\height}{\includegraphics[width=.54\textwidth]{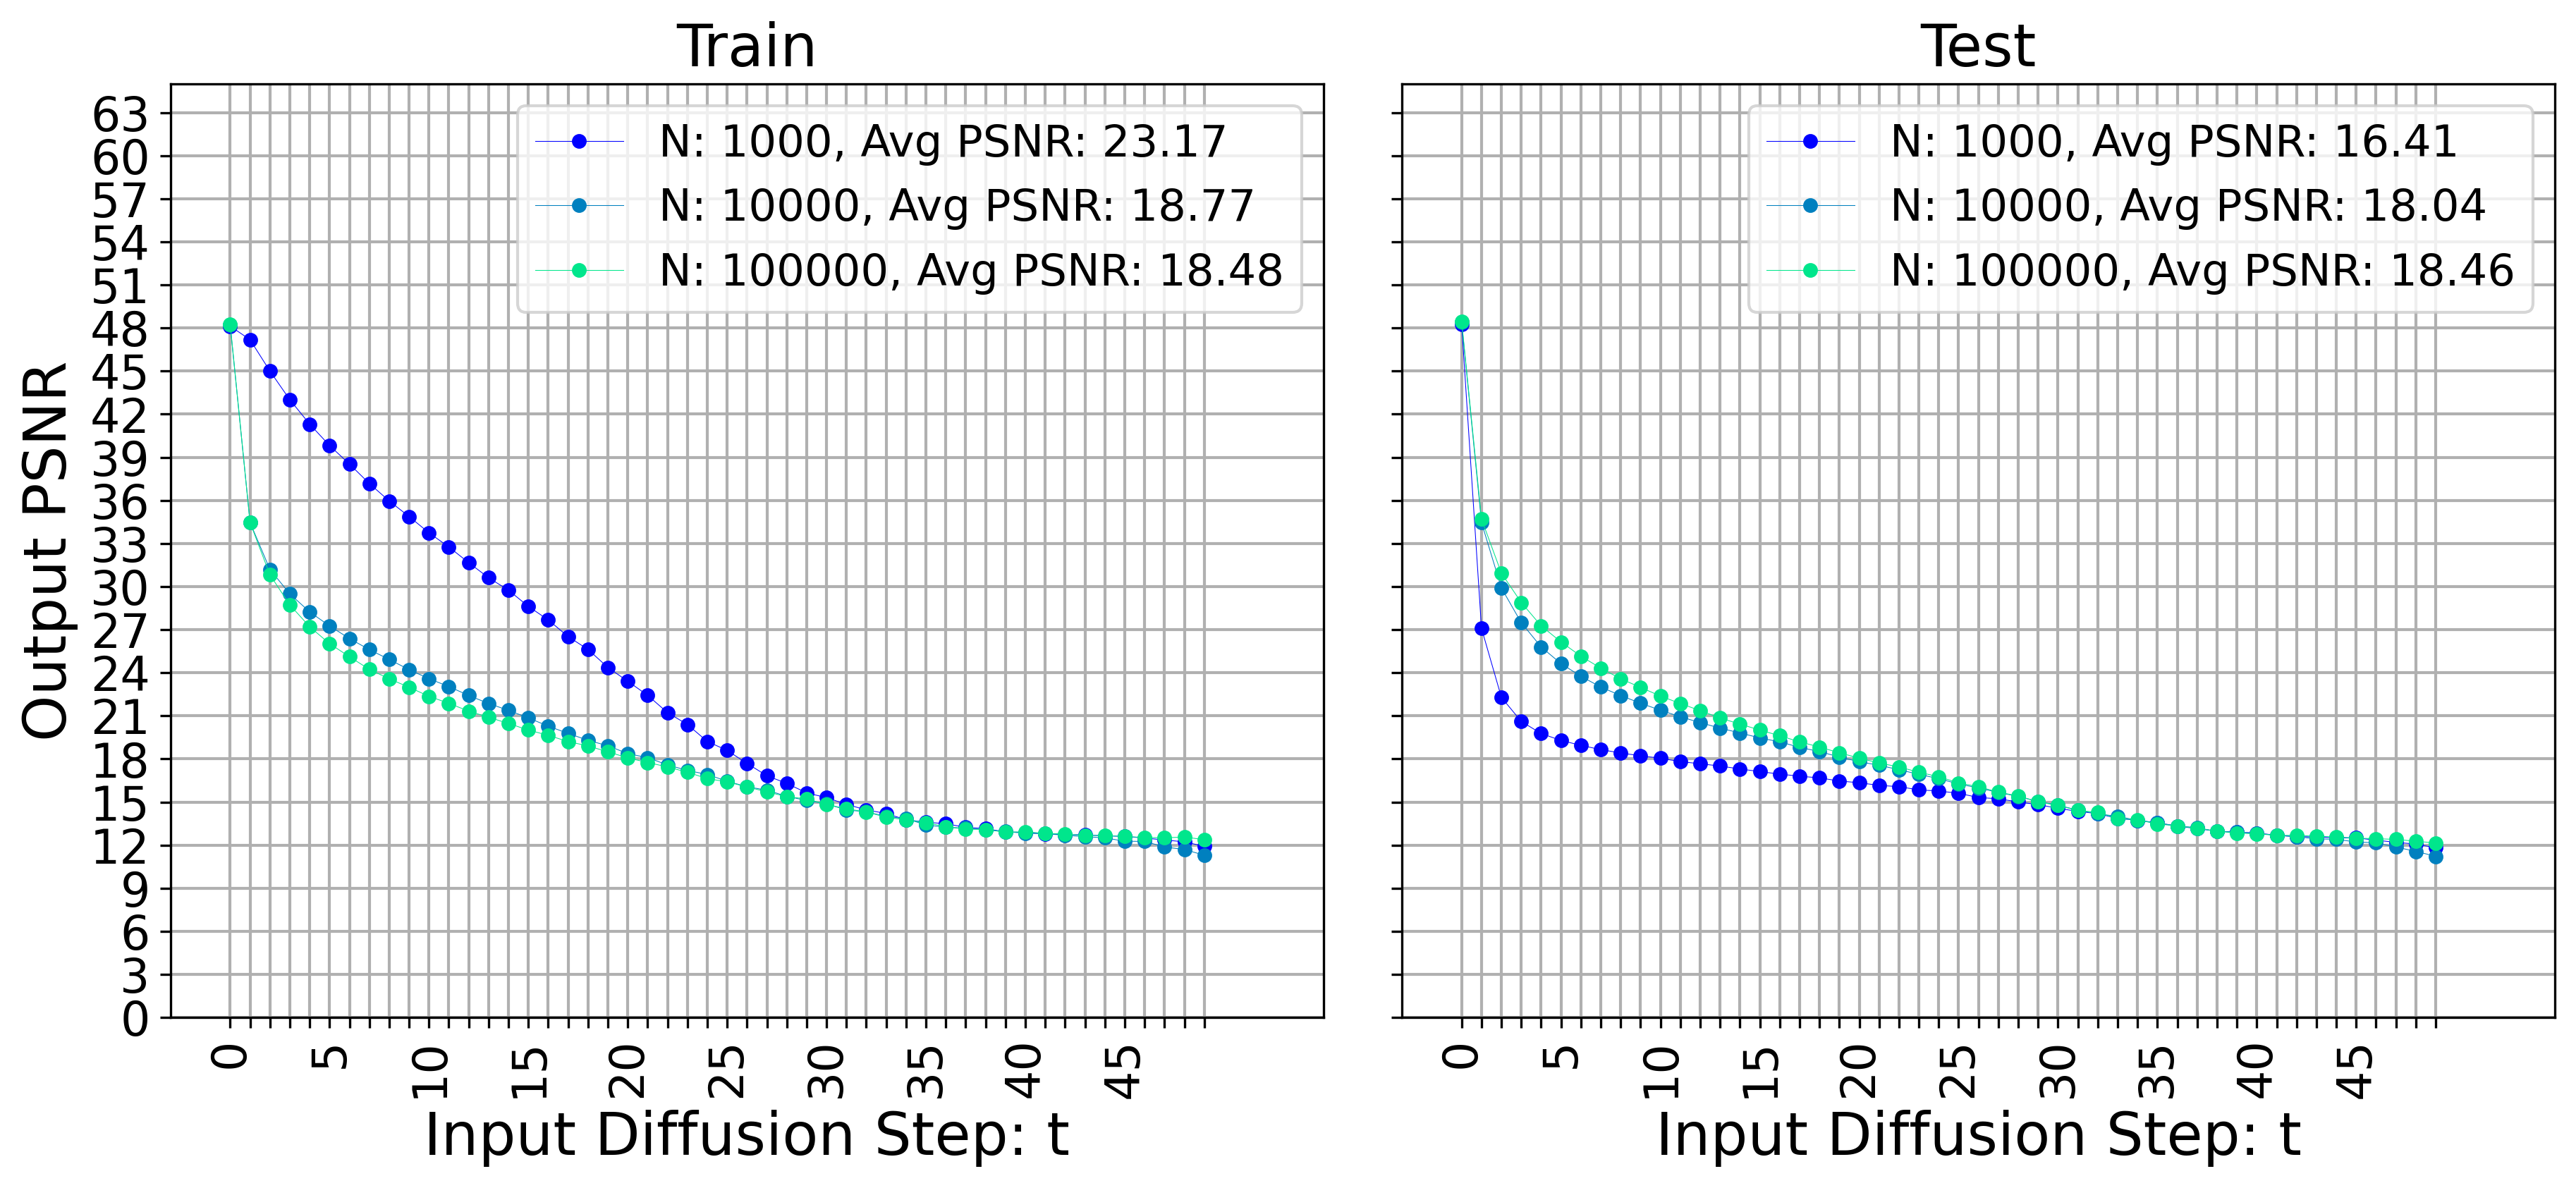}}
&
\raisebox{-0.5\height}{\includegraphics[width=.41\textwidth]{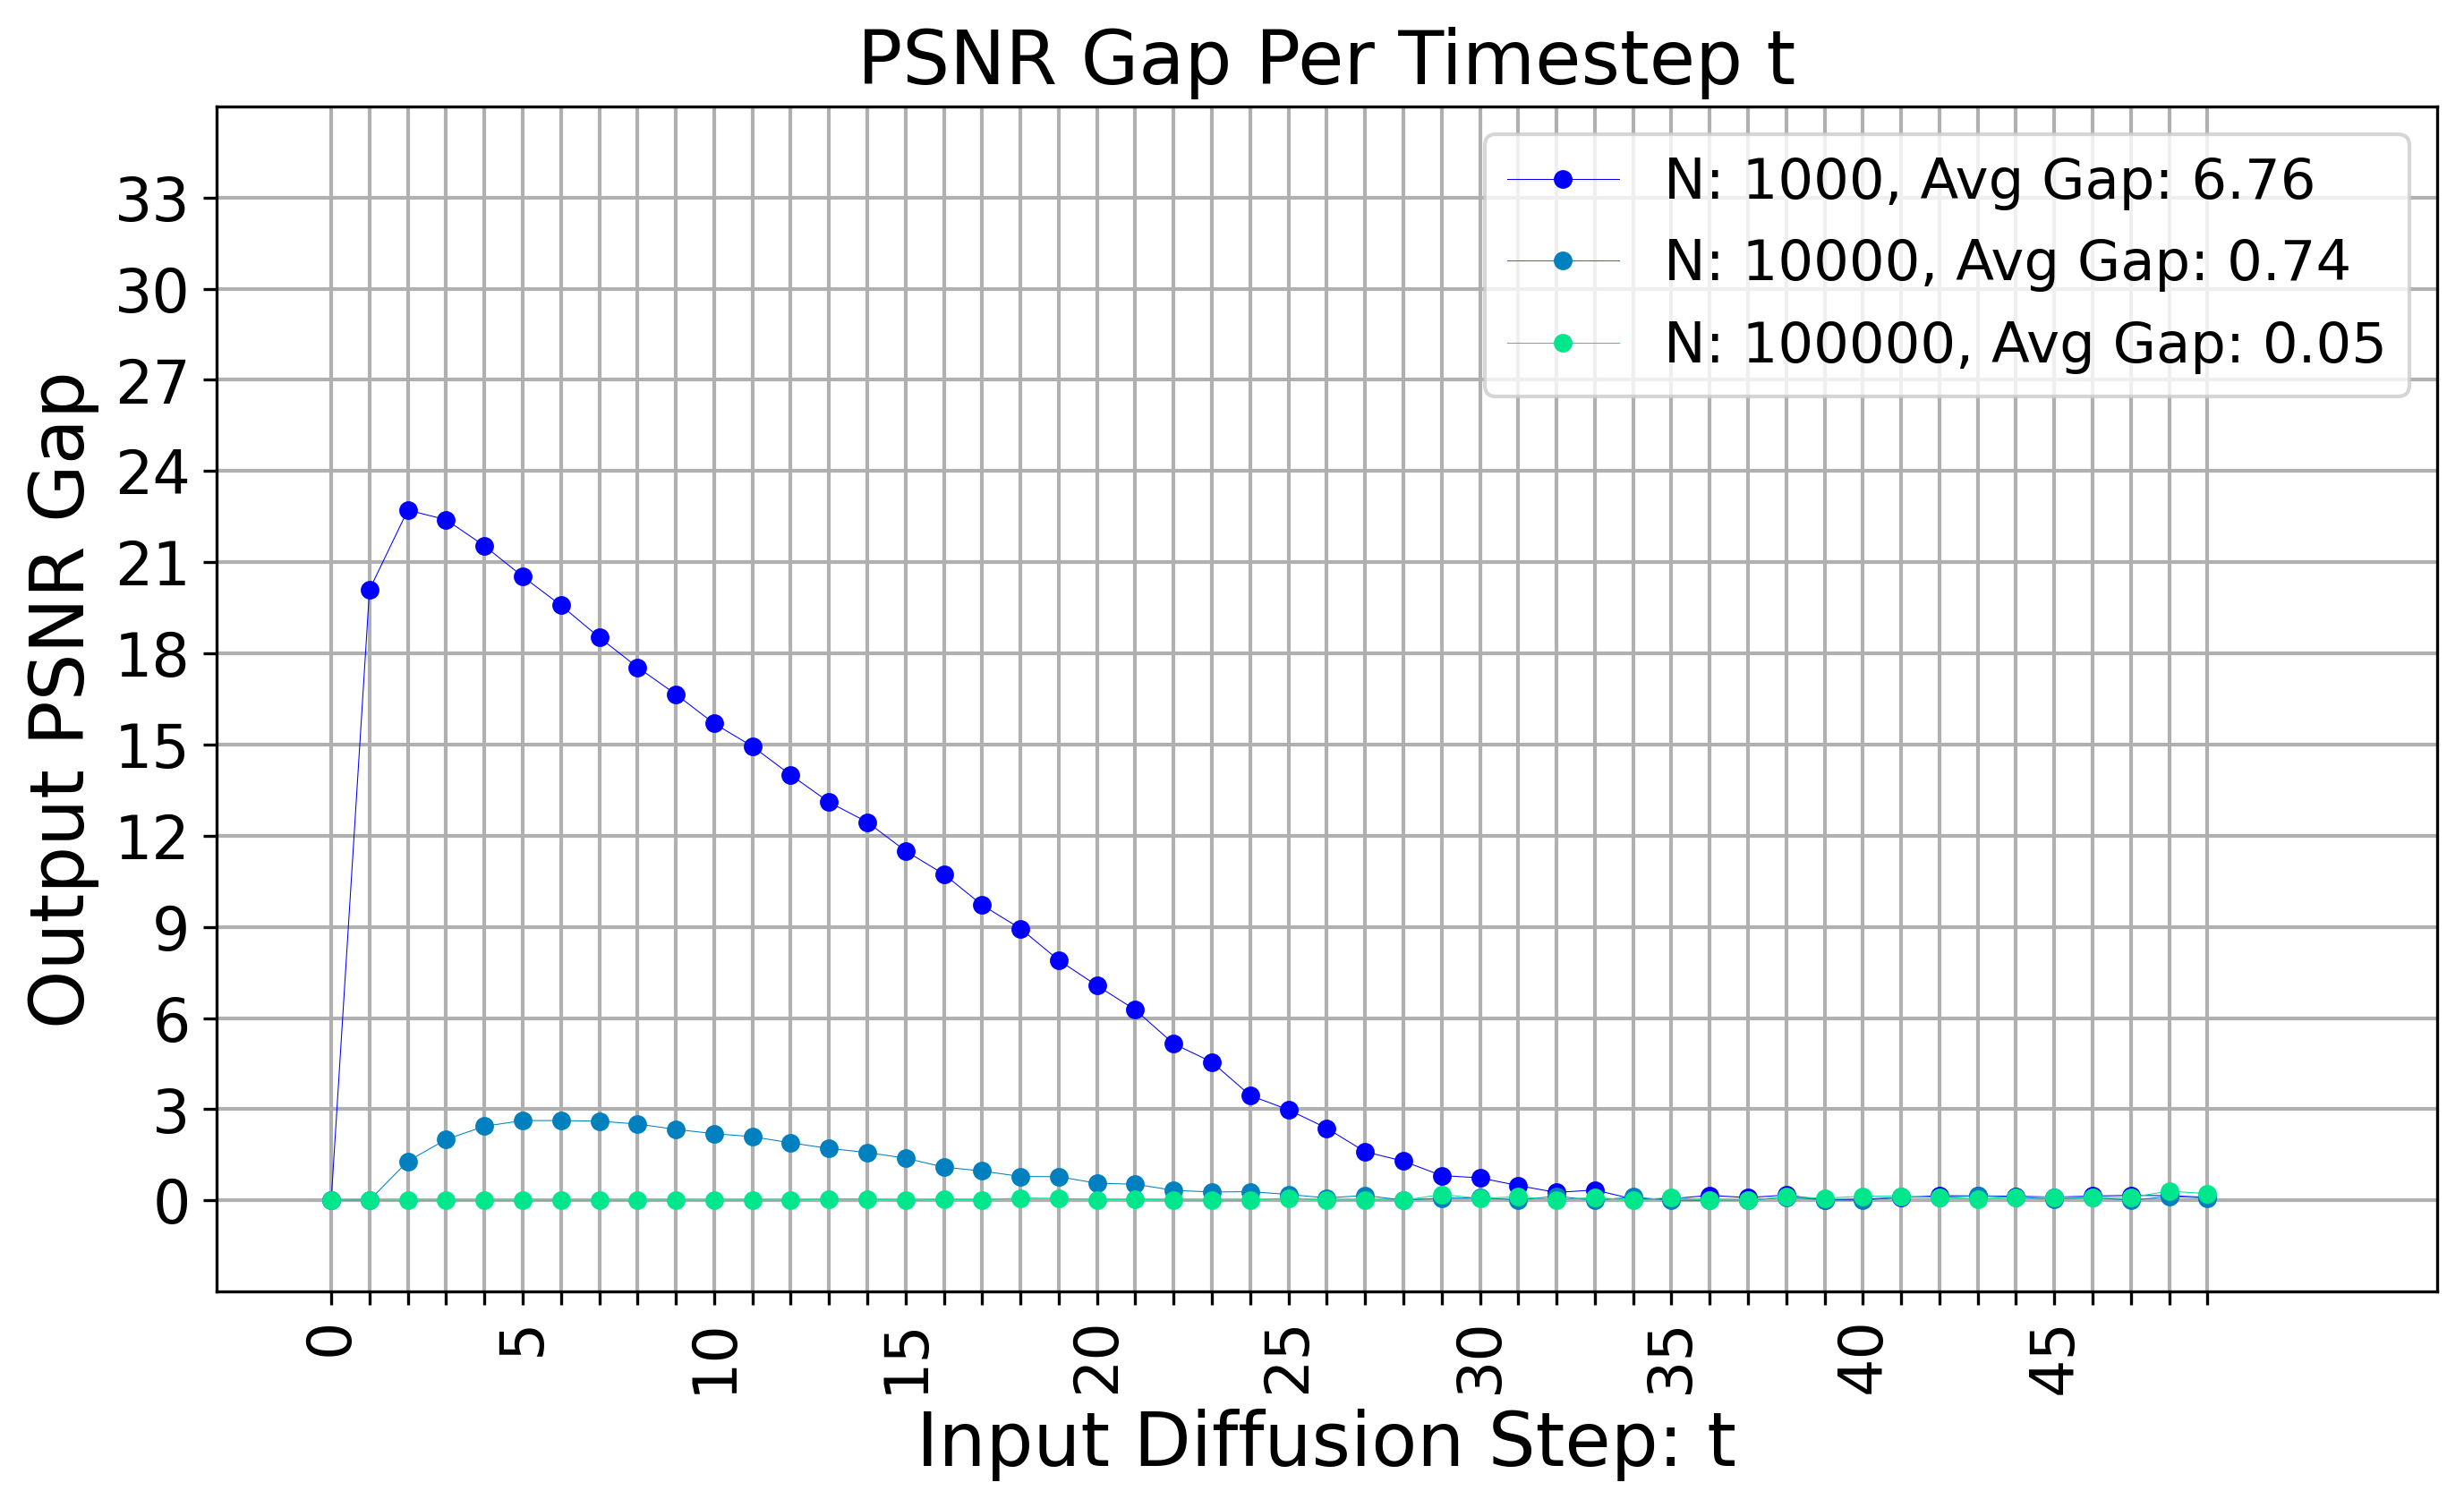}}
\\
\hline
\cellcolor{dit}{\STAB{\rotatebox[origin=c]{90}{DiT-S/1}}}
&
\raisebox{-0.5\height}{\includegraphics[width=.54\textwidth]{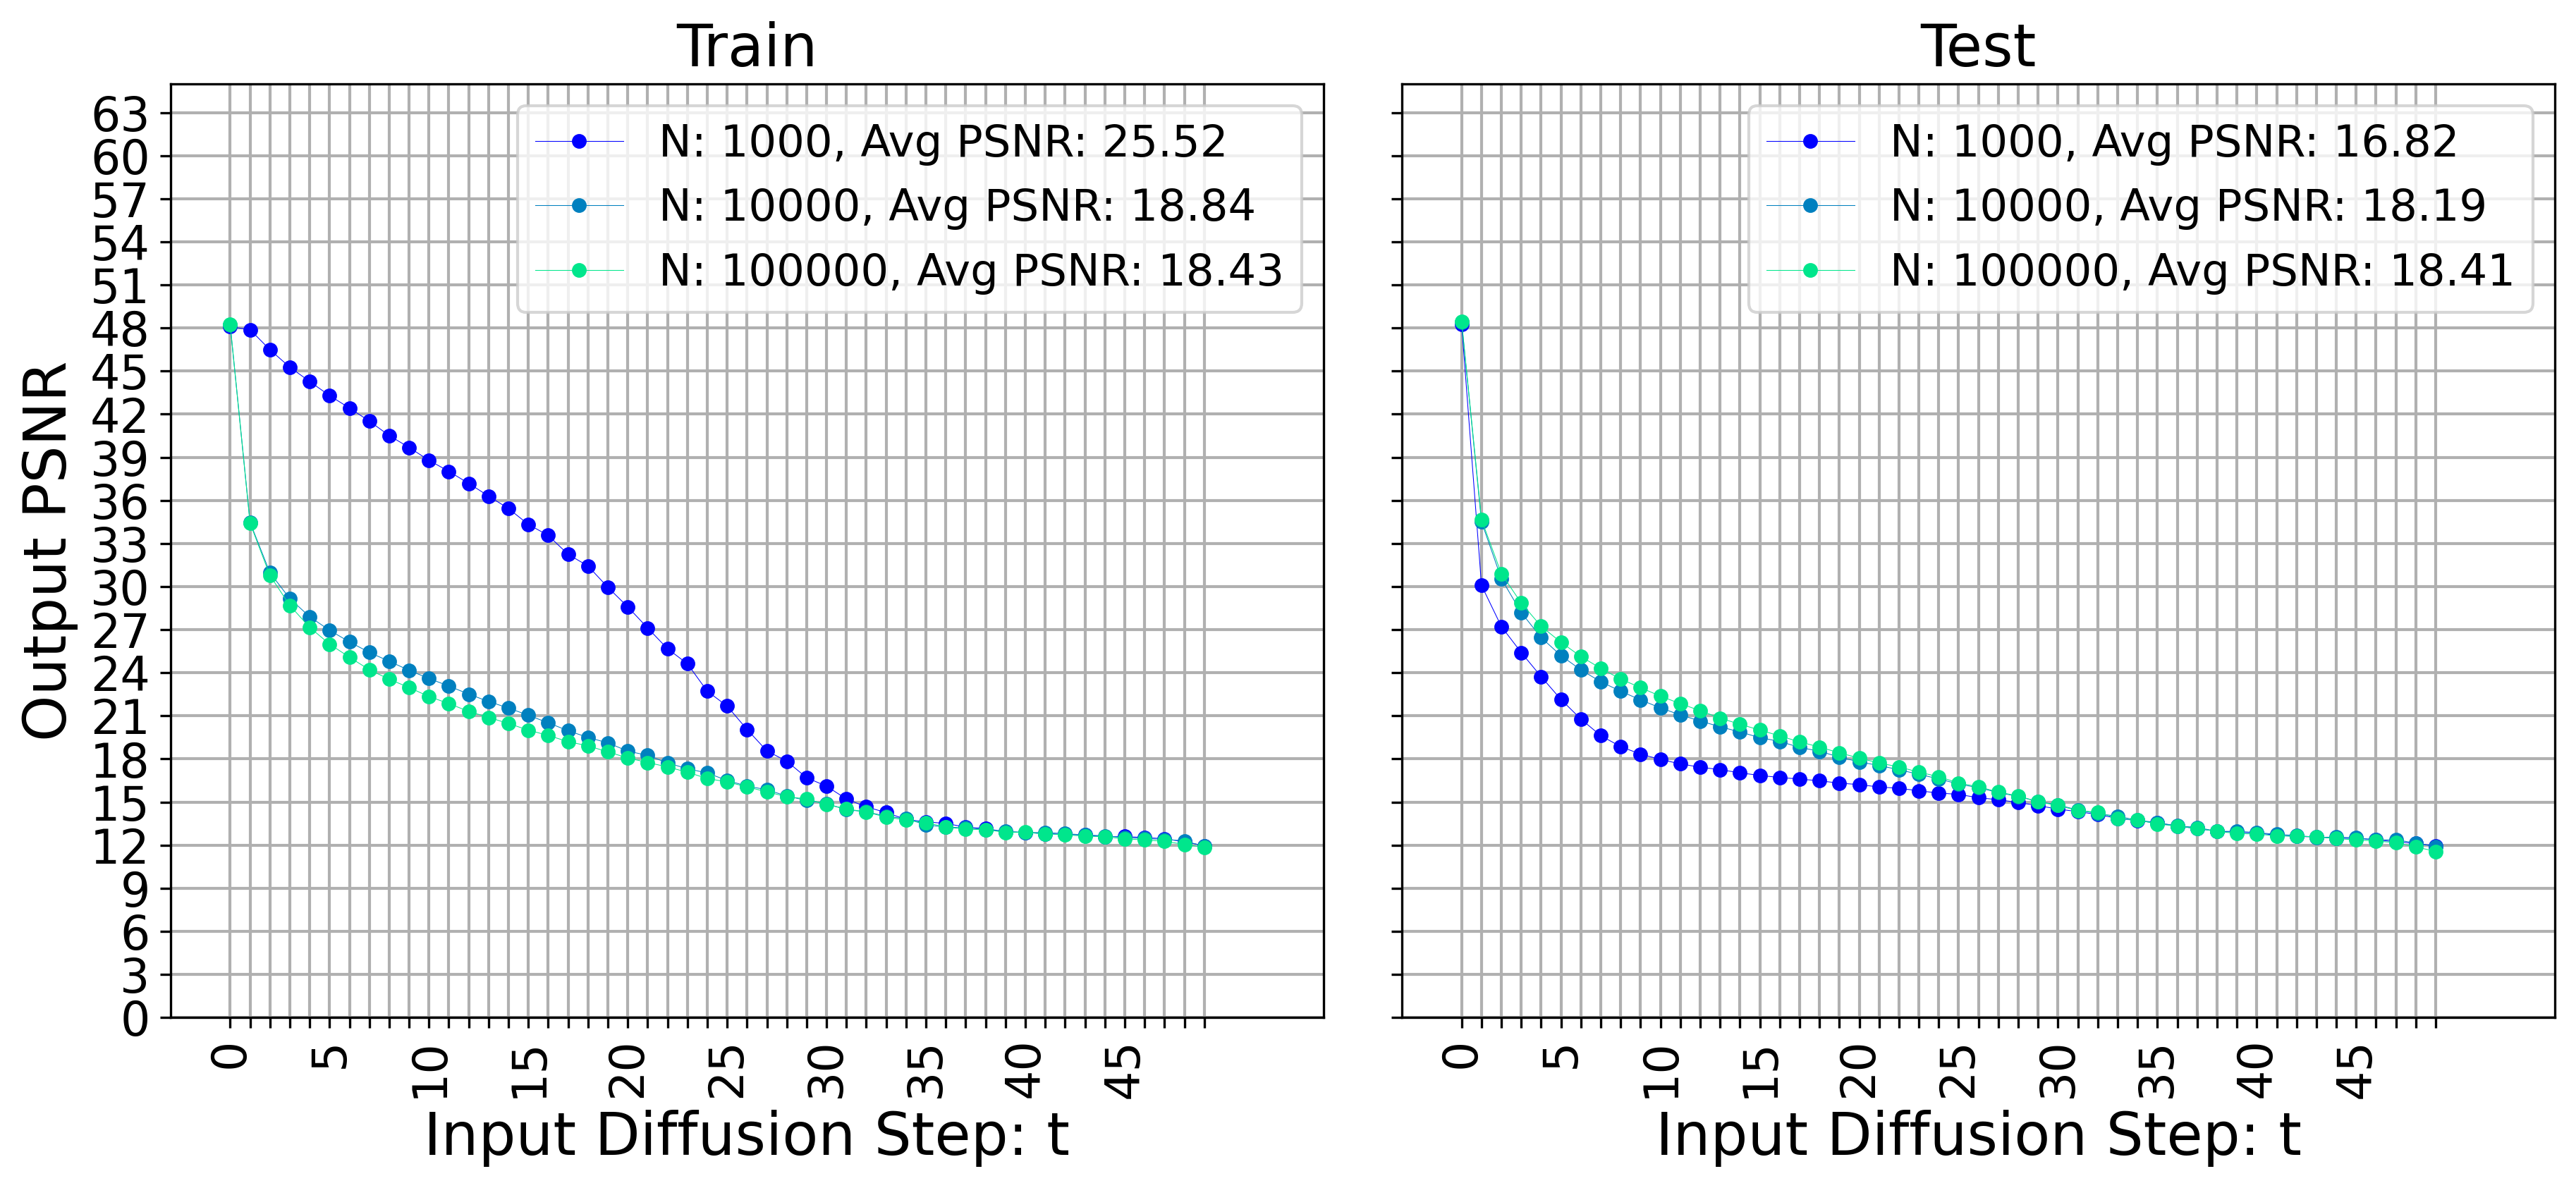}}
&
\raisebox{-0.5\height}{\includegraphics[width=.41\textwidth]{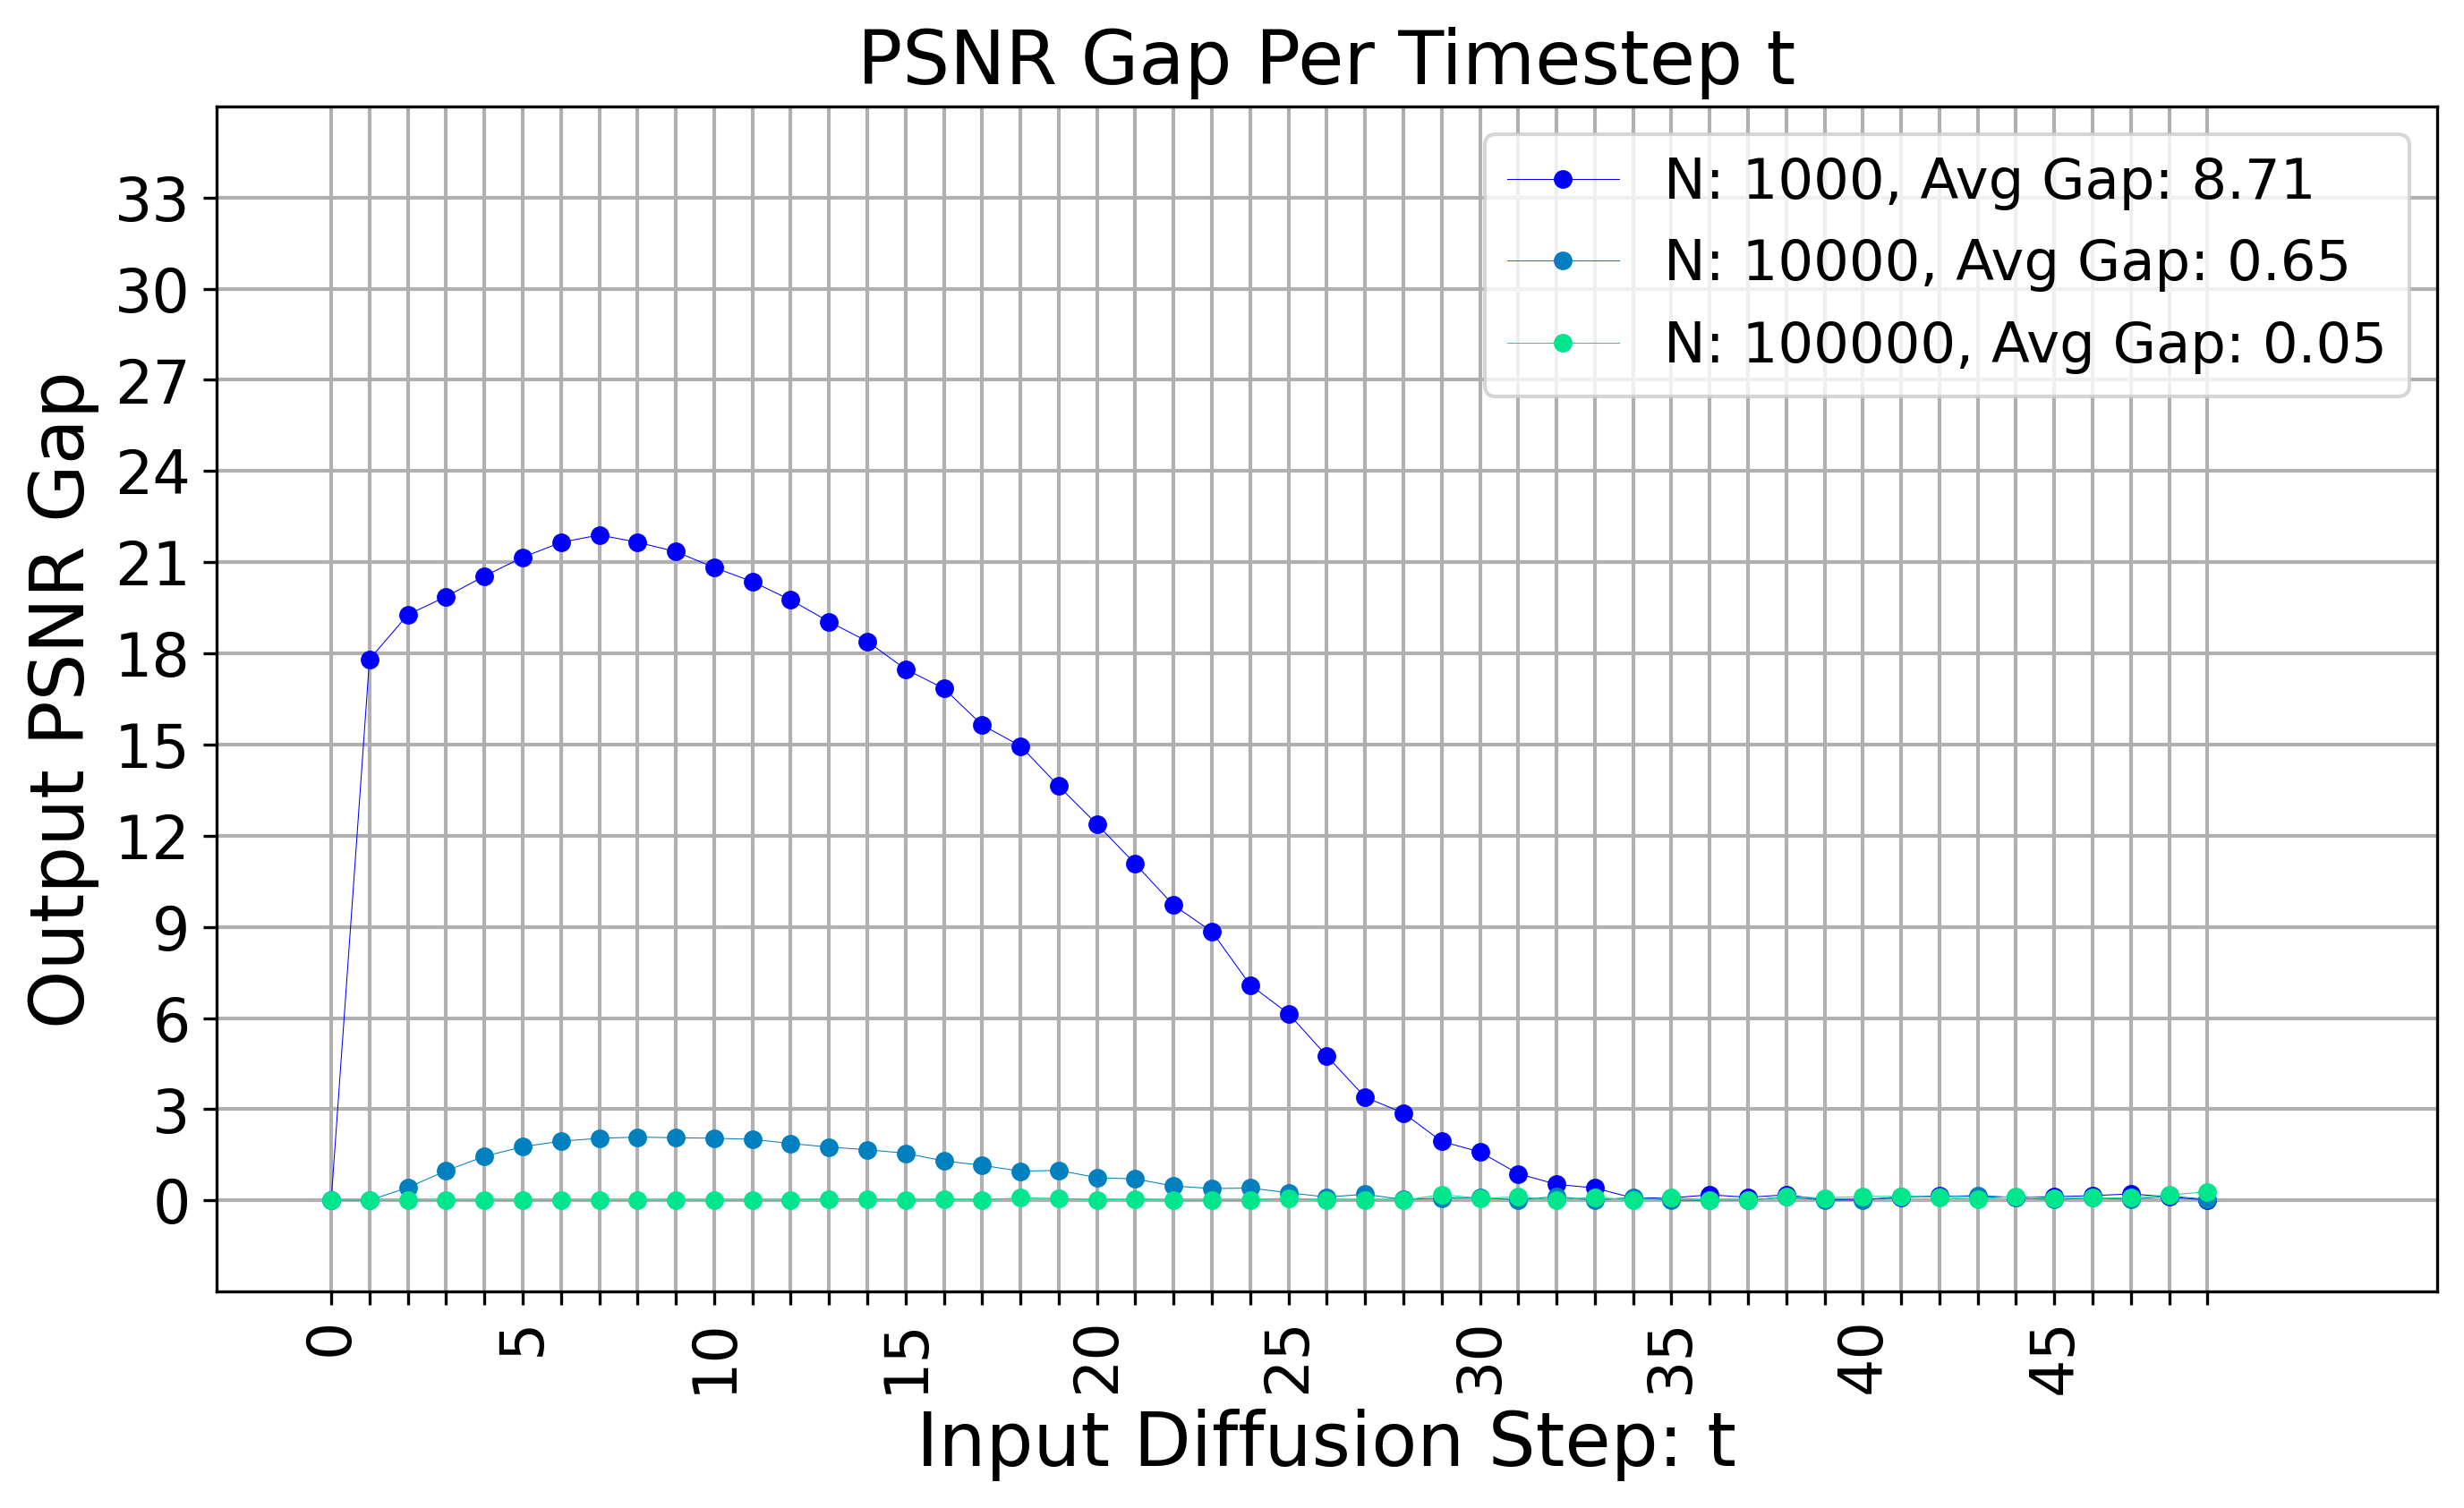}}
\\
\hline
\cellcolor{diff}{\STAB{\rotatebox[origin=c]{90}{DiT-S/1 w/ Local}}}
&
\raisebox{-0.5\height}{\includegraphics[width=.54\textwidth]{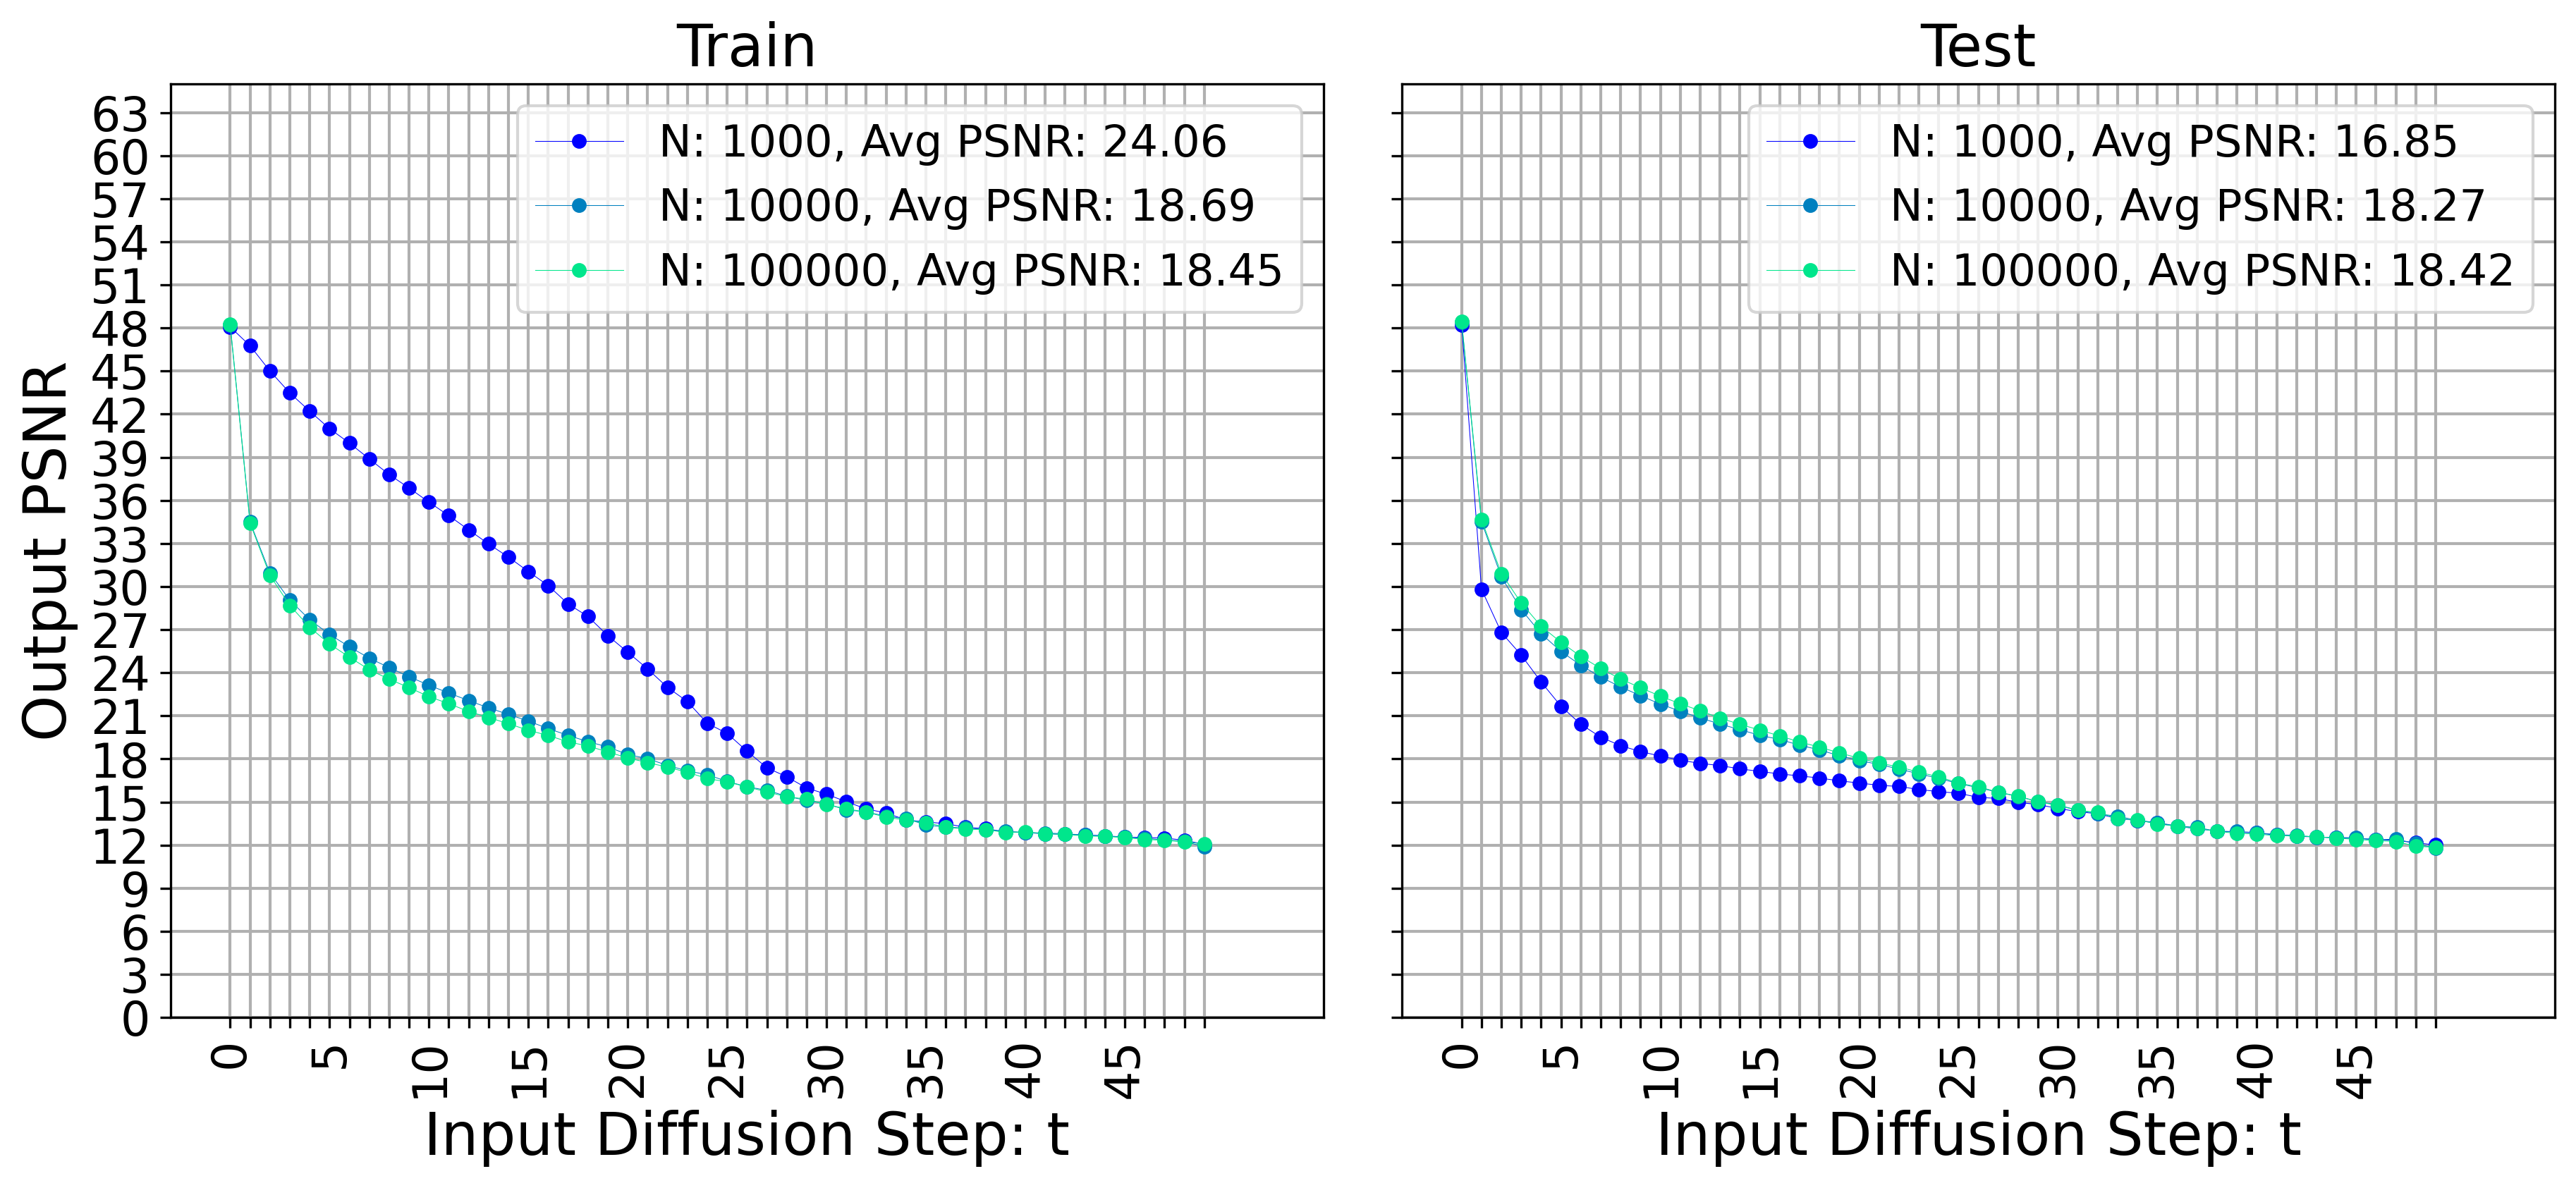}}
&
\raisebox{-0.5\height}{\includegraphics[width=.41\textwidth]{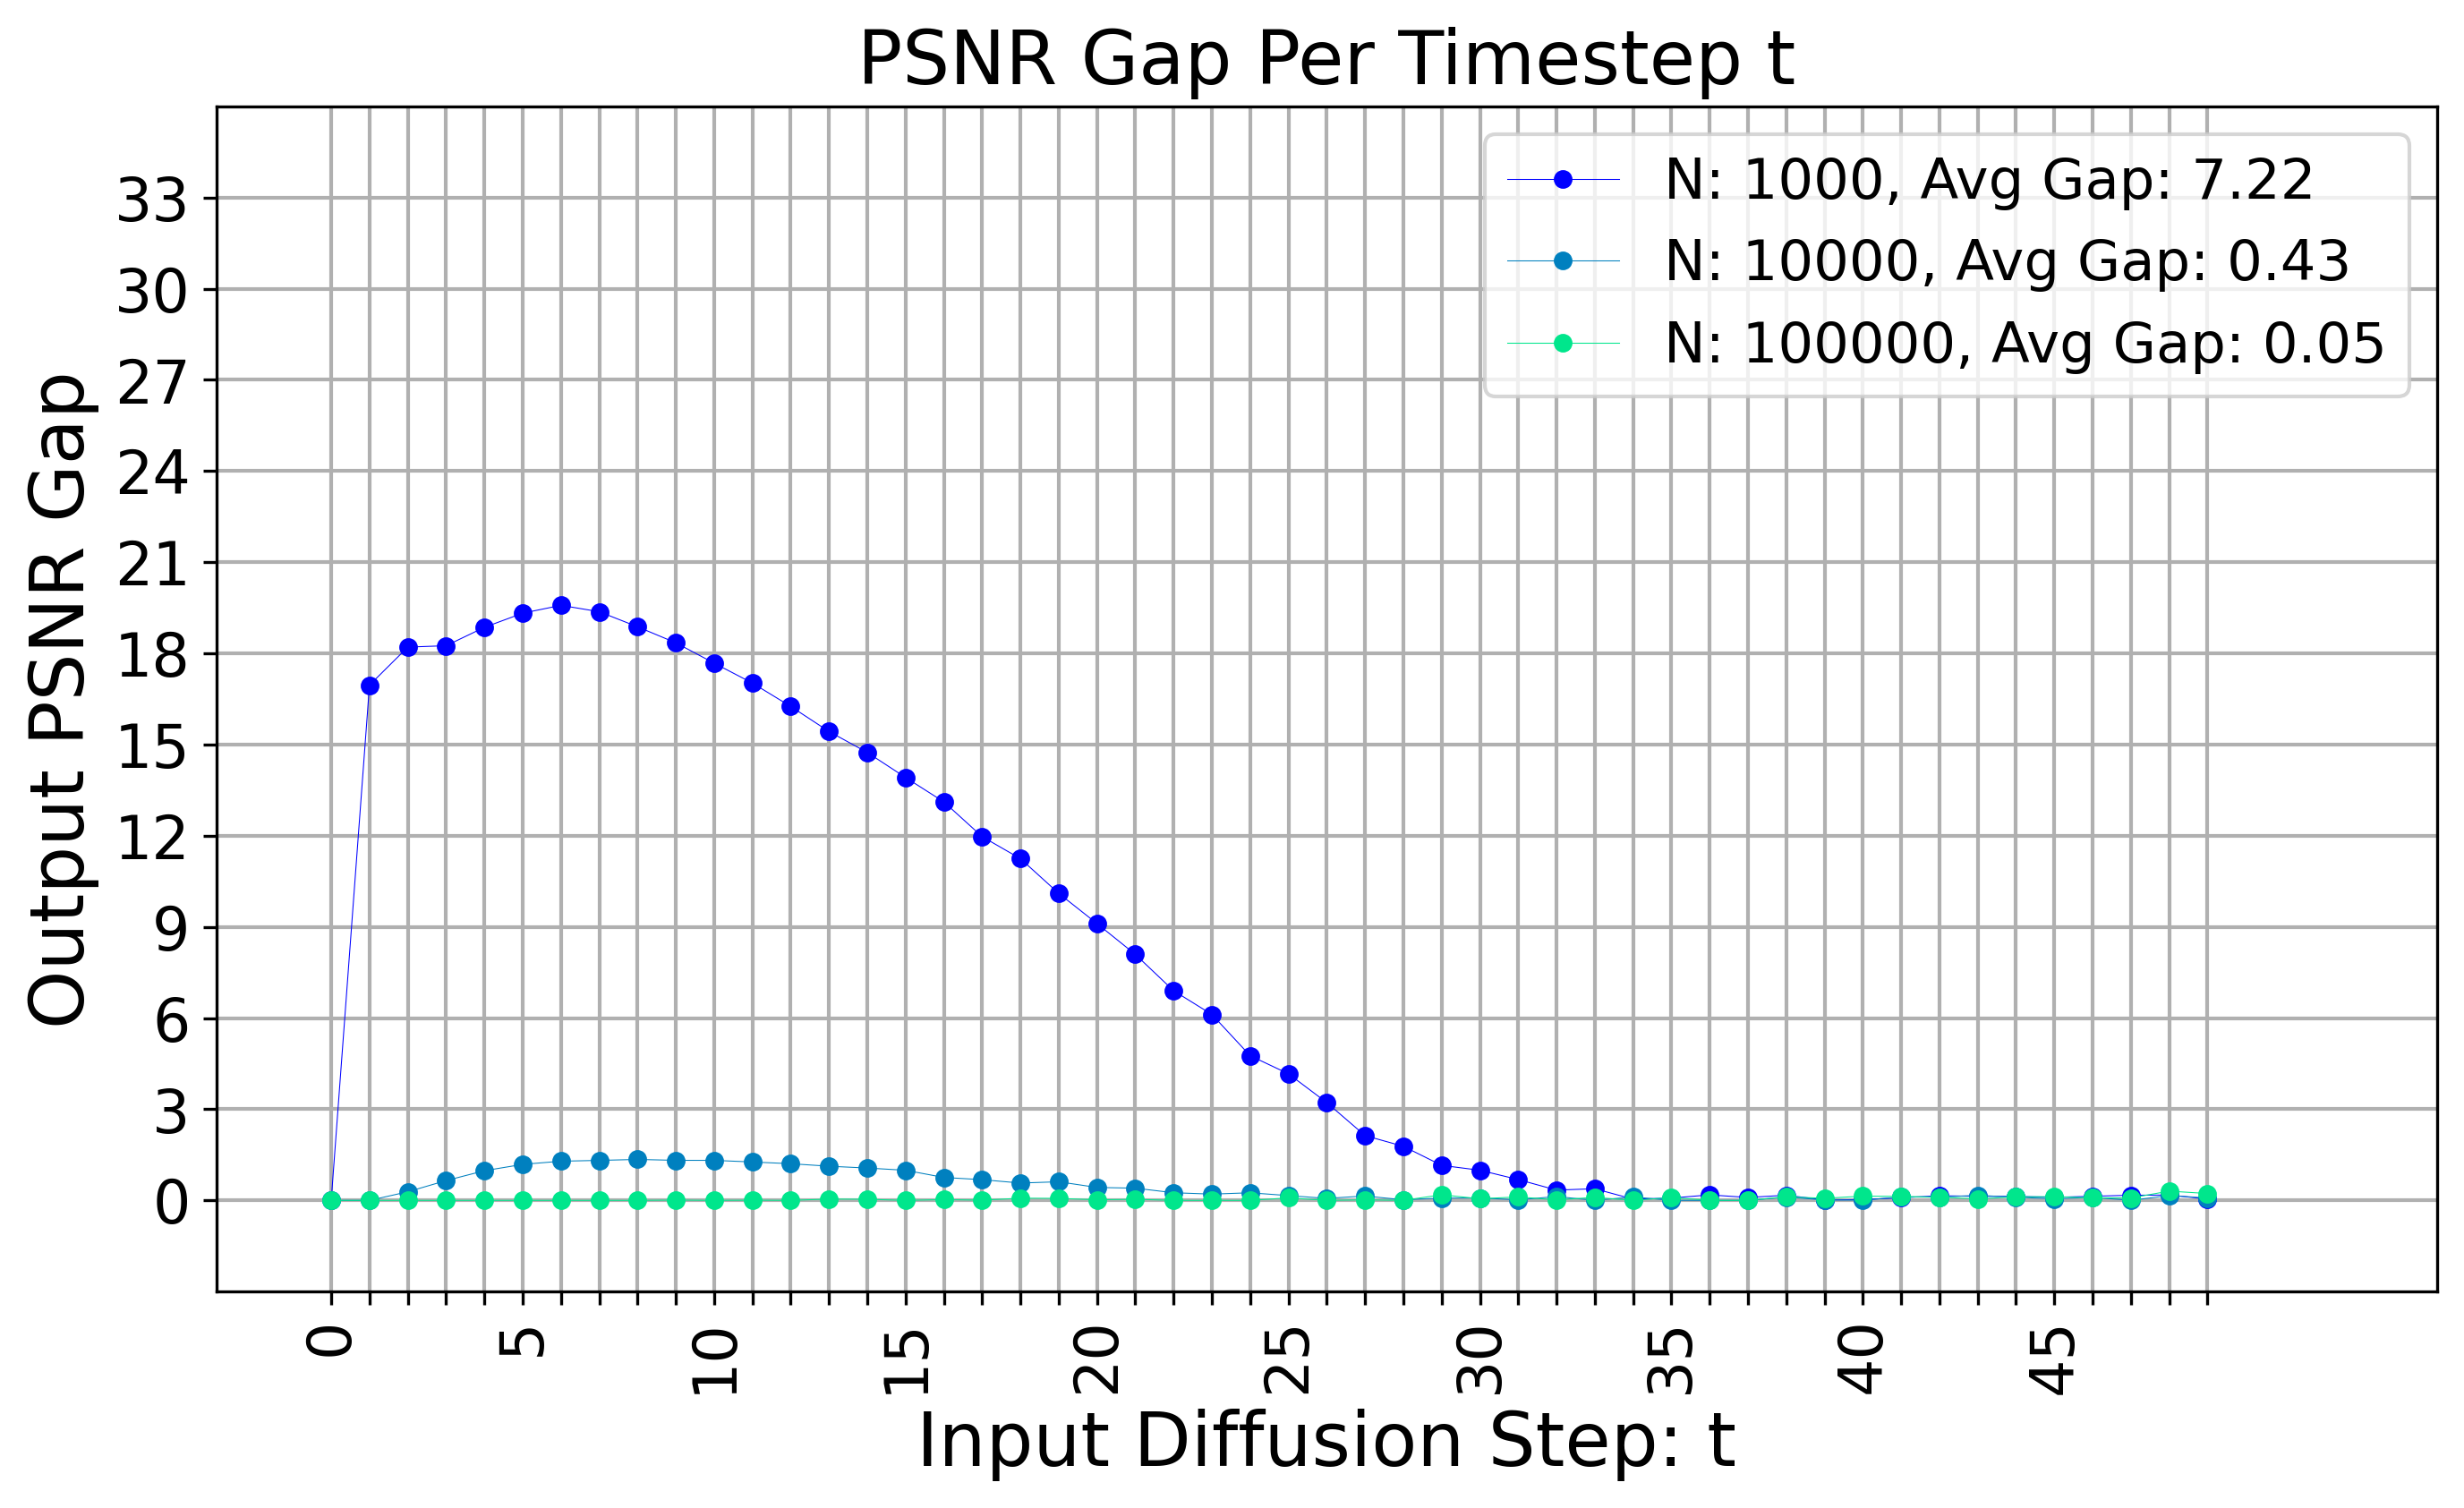}}
\\
&
\multicolumn{1}{c}{(a) PSNR Curves of Training and Testing Sets}
&
\multicolumn{1}{c}{(b) PSNR Gap}
\\
\end{tabular}

\captionof{figure}{The PSNR (a) and PSNR gap (b) comparison on the ImageNet~\citep{deng2009imagenet} dataset.}
\label{fig:row_psnr_imagenet}
\end{table}

\begin{table}[ht]
\centering
\small
\setlength\tabcolsep{1pt}
\setlength{\extrarowheight}{4pt}
\begin{tabular}{lc|c}
\cellcolor{dit}{\STAB{\rotatebox[origin=c]{90}{DiT-XS/1}}}
&
\raisebox{-0.5\height}{\includegraphics[width=.54\textwidth]{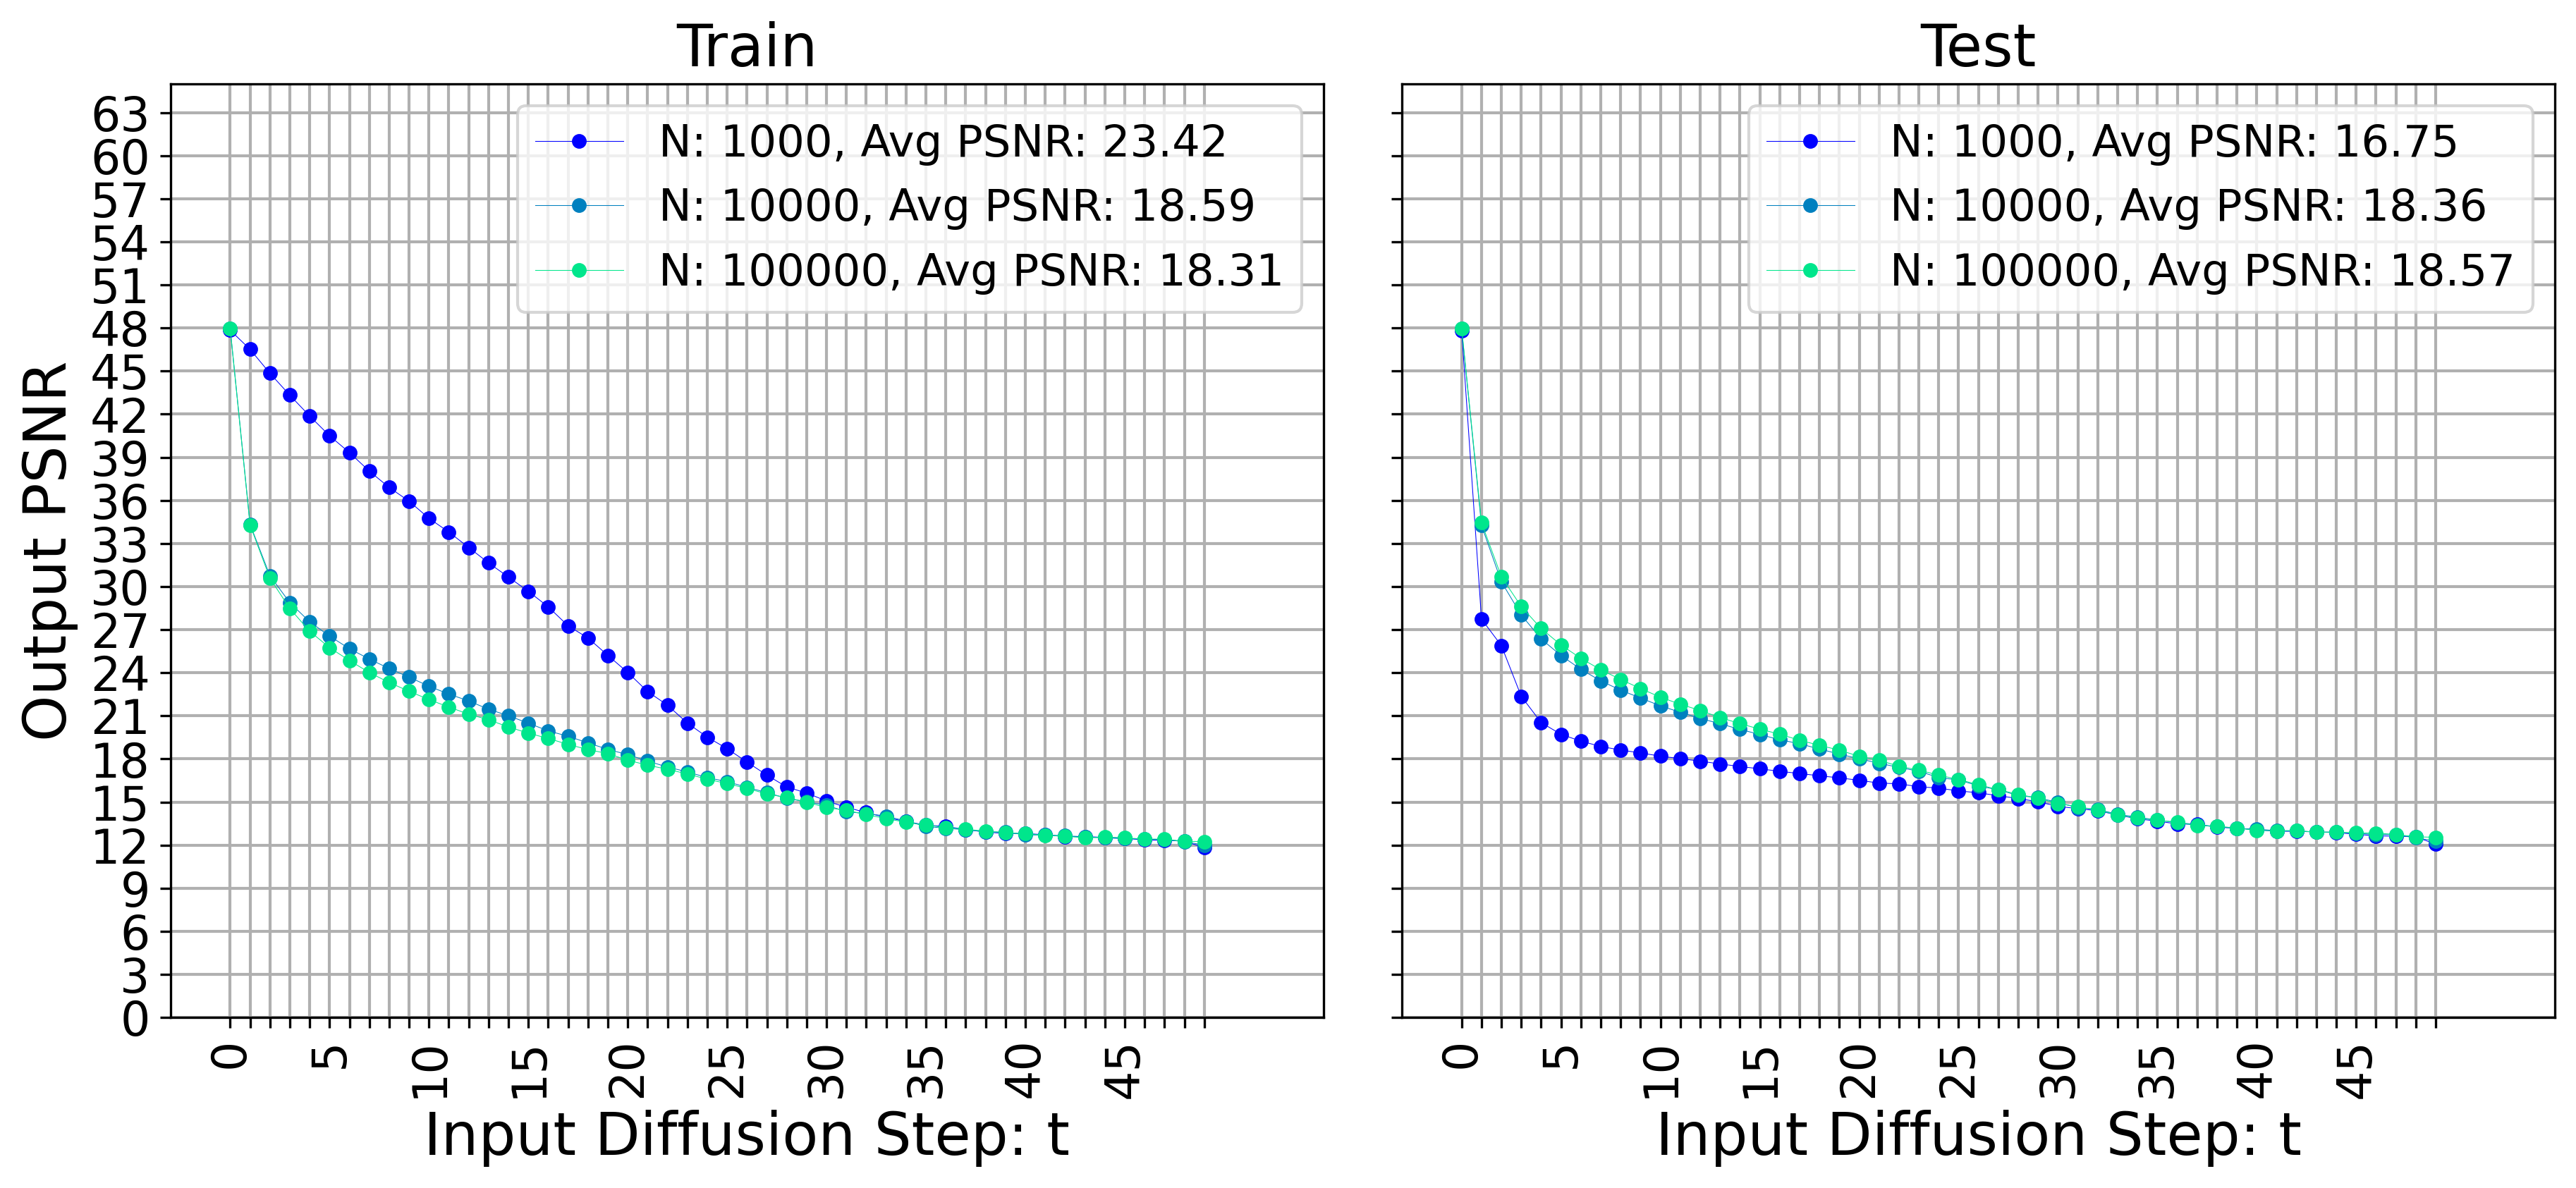}}
&
\raisebox{-0.5\height}{\includegraphics[width=.41\textwidth]{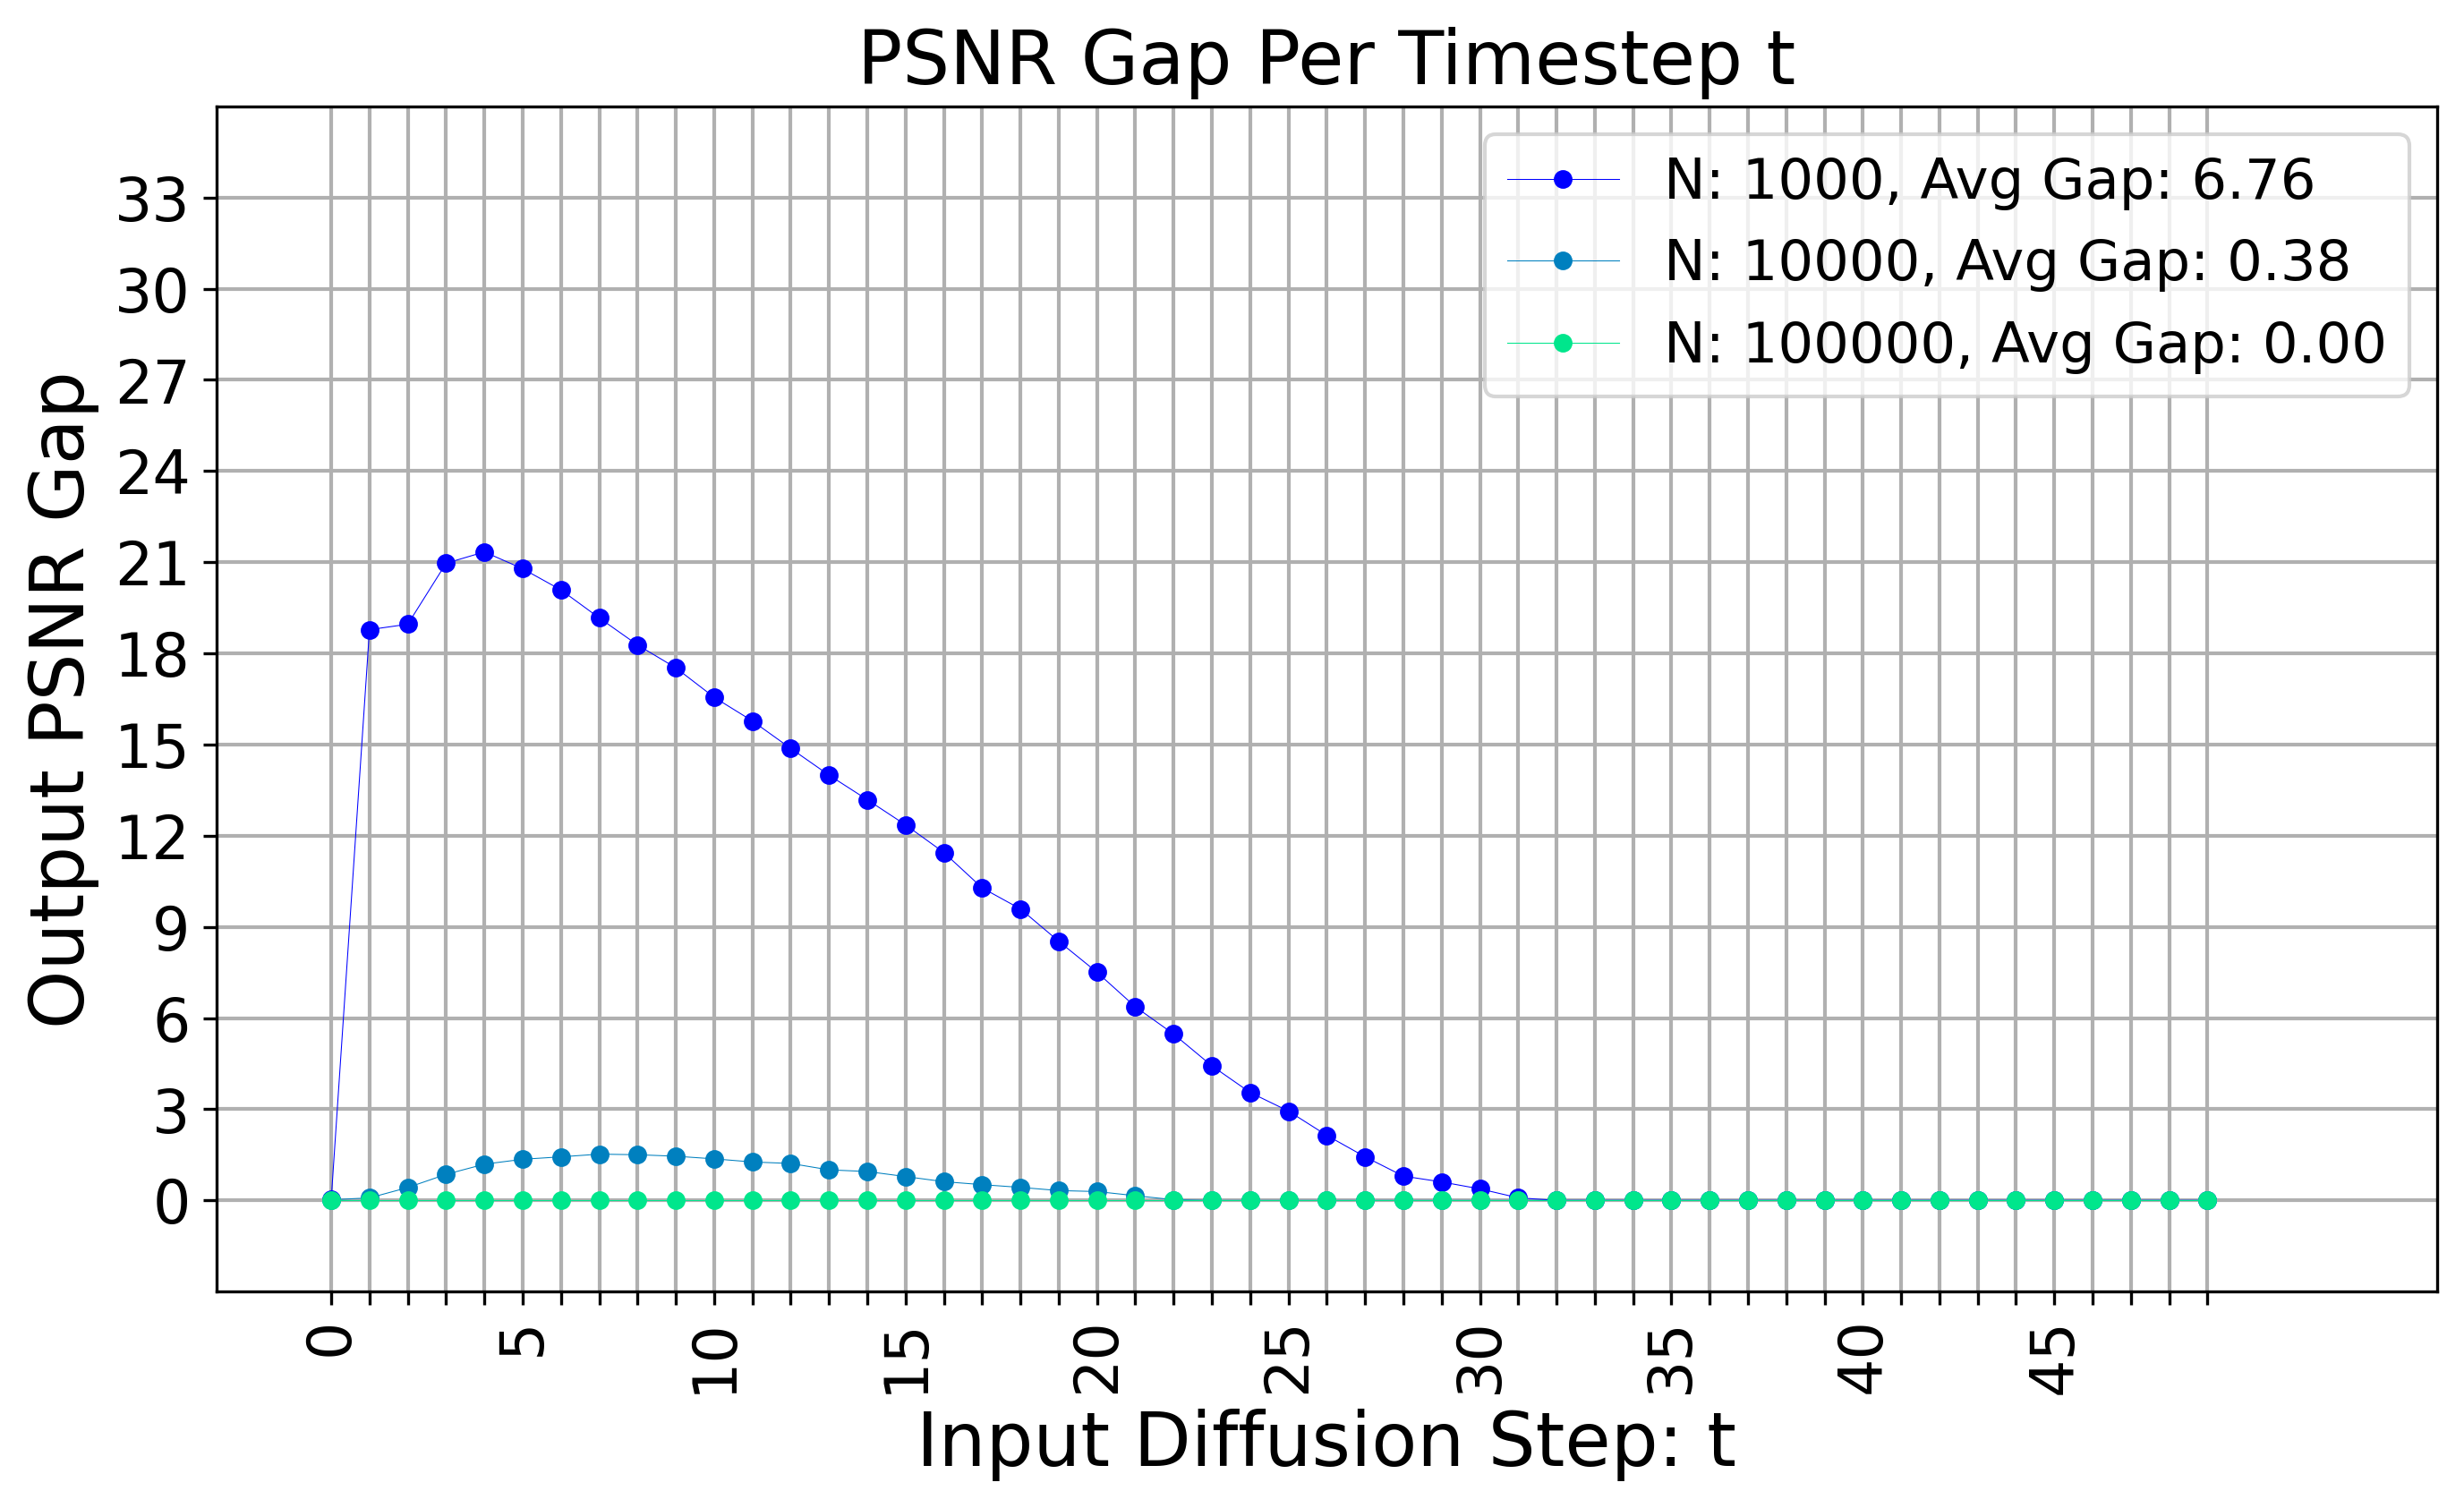}}
\\
\hline
\cellcolor{diff}{\STAB{\rotatebox[origin=c]{90}{DiT-XS/1 w/ Local}}}
&
\raisebox{-0.5\height}{\includegraphics[width=.54\textwidth]{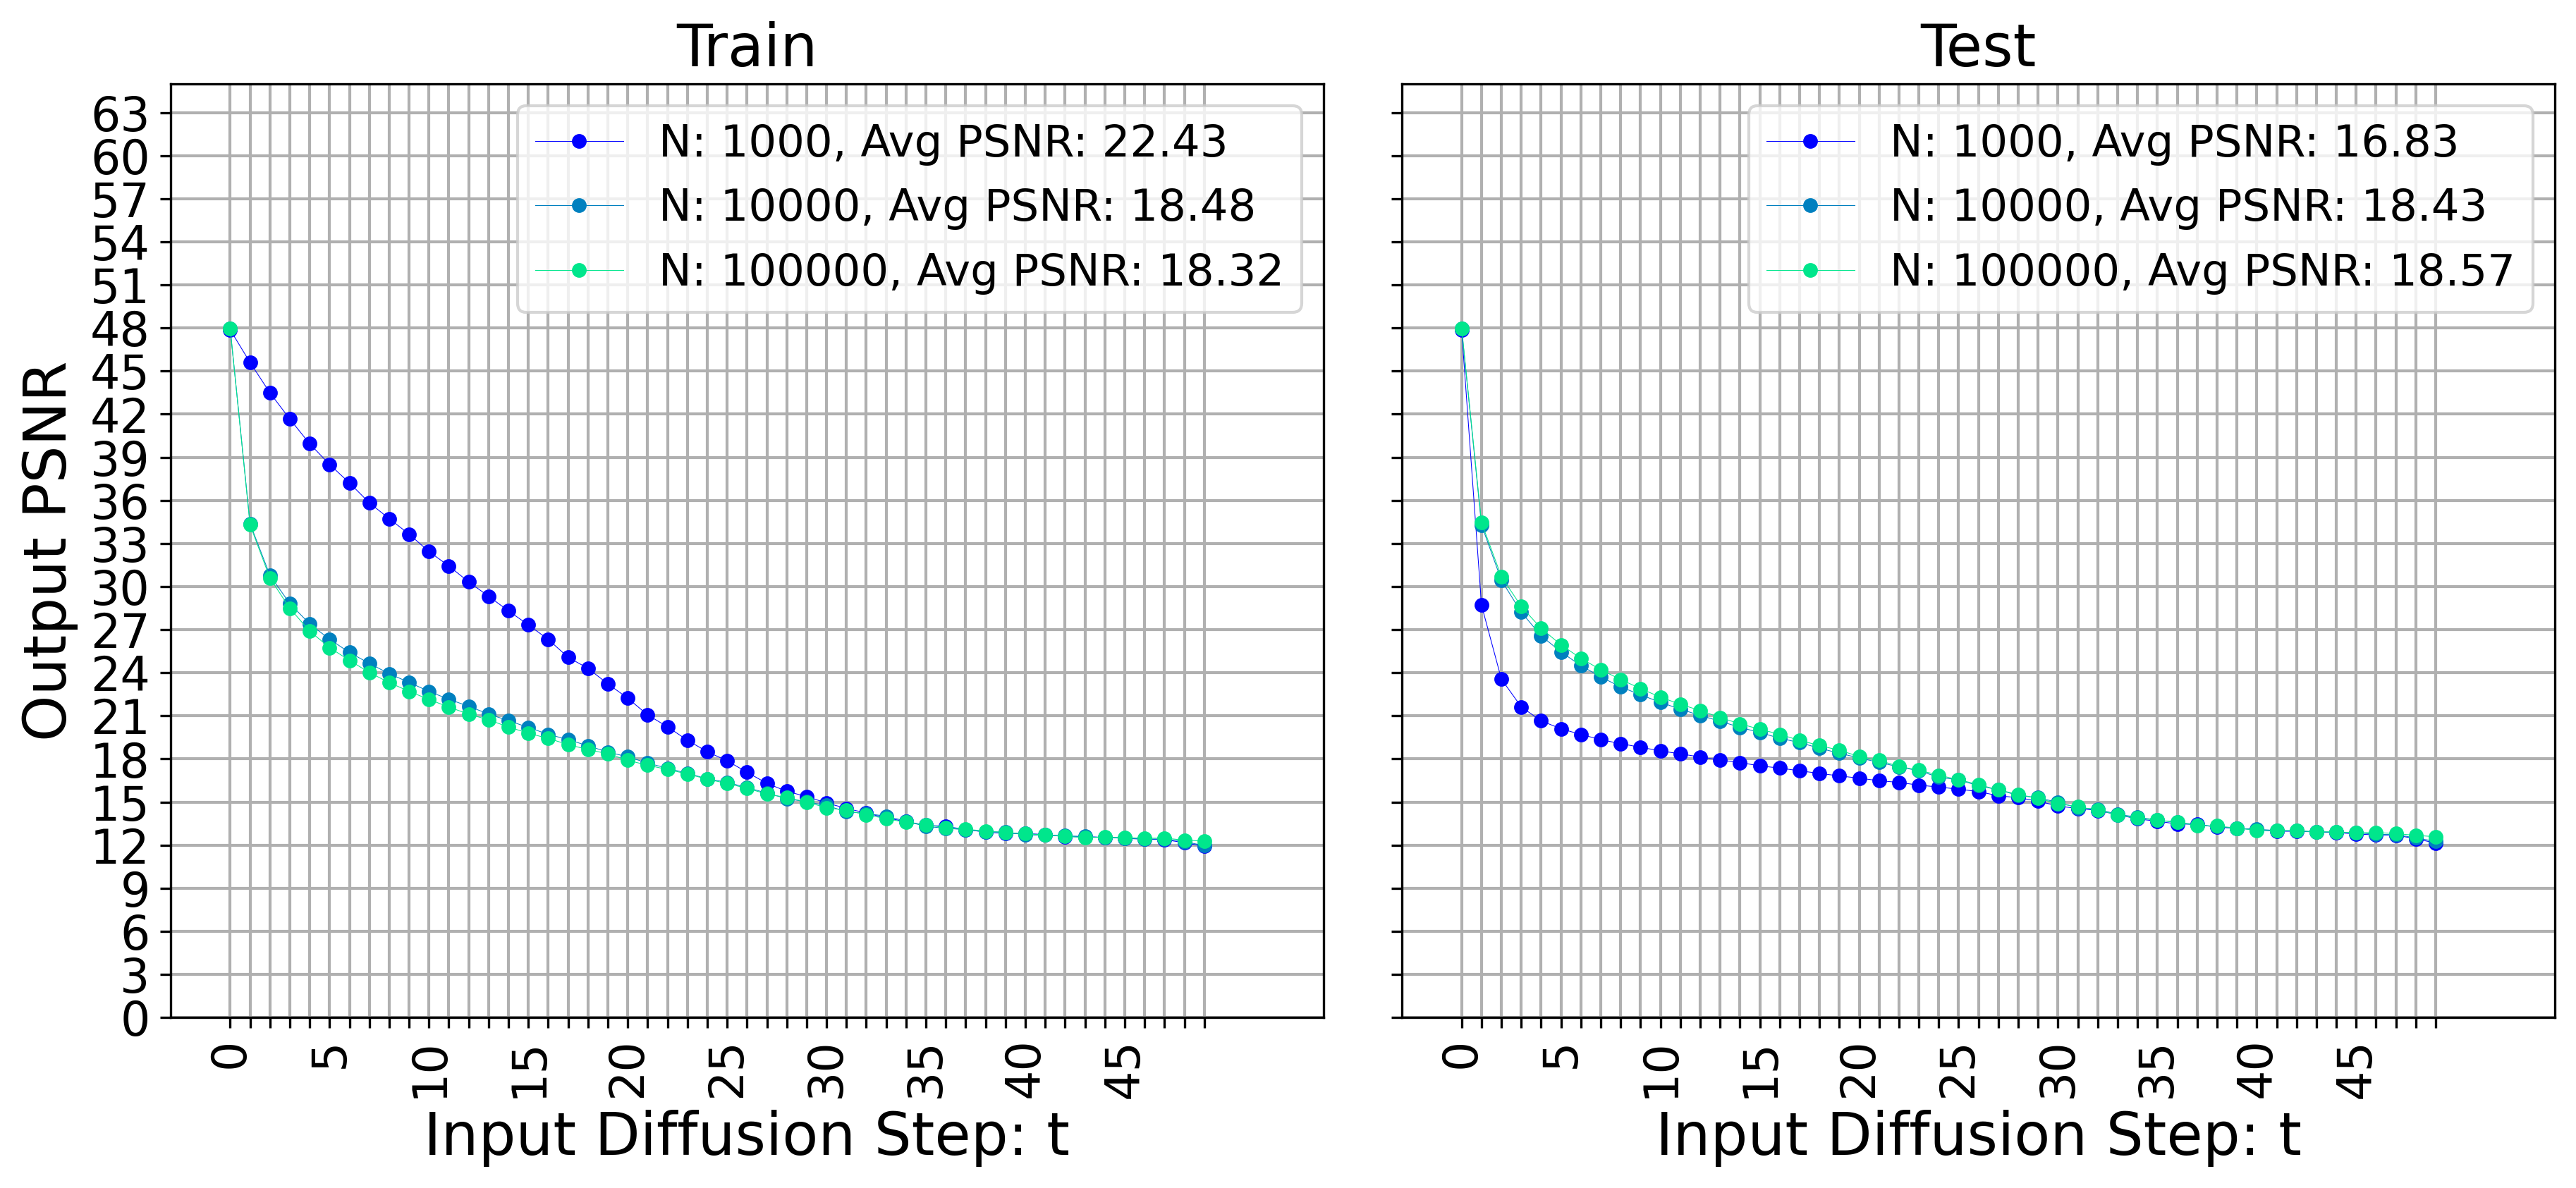}}
&
\raisebox{-0.5\height}{\includegraphics[width=.41\textwidth]{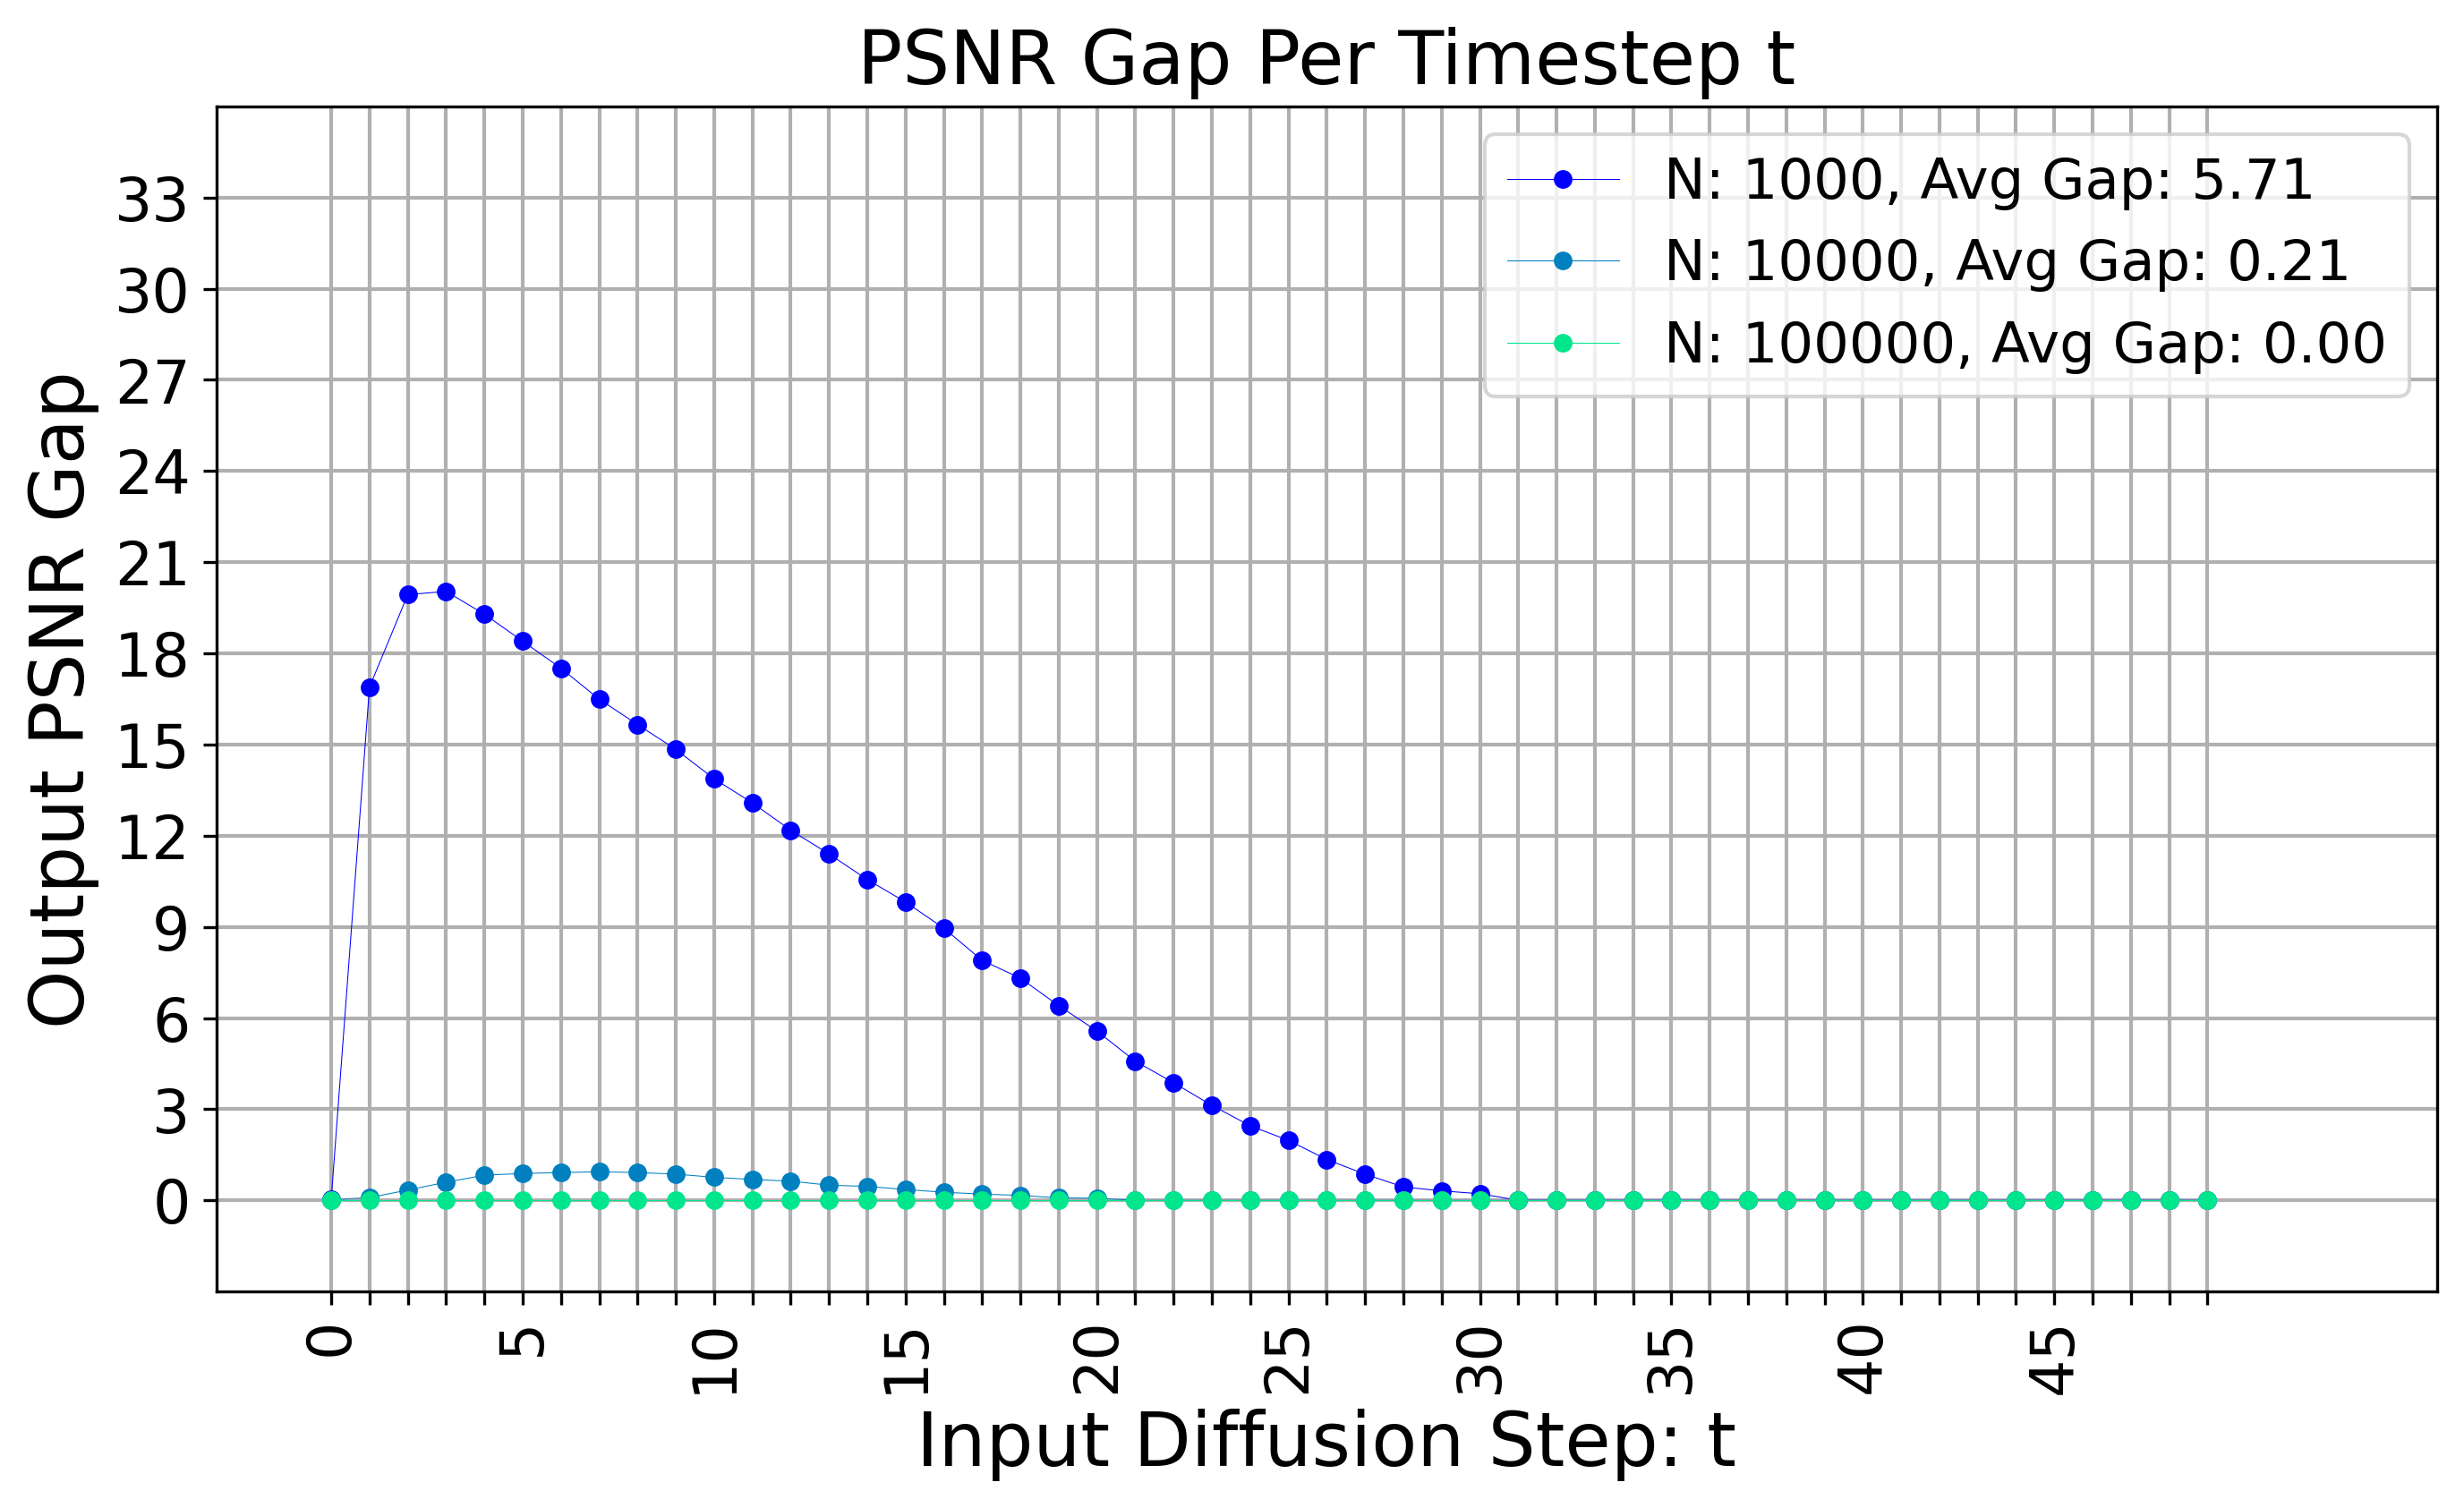}}
\\
\hline
\cellcolor{dit}{\STAB{\rotatebox[origin=c]{90}{DiT-S/1}}}
&
\raisebox{-0.5\height}{\includegraphics[width=.54\textwidth]{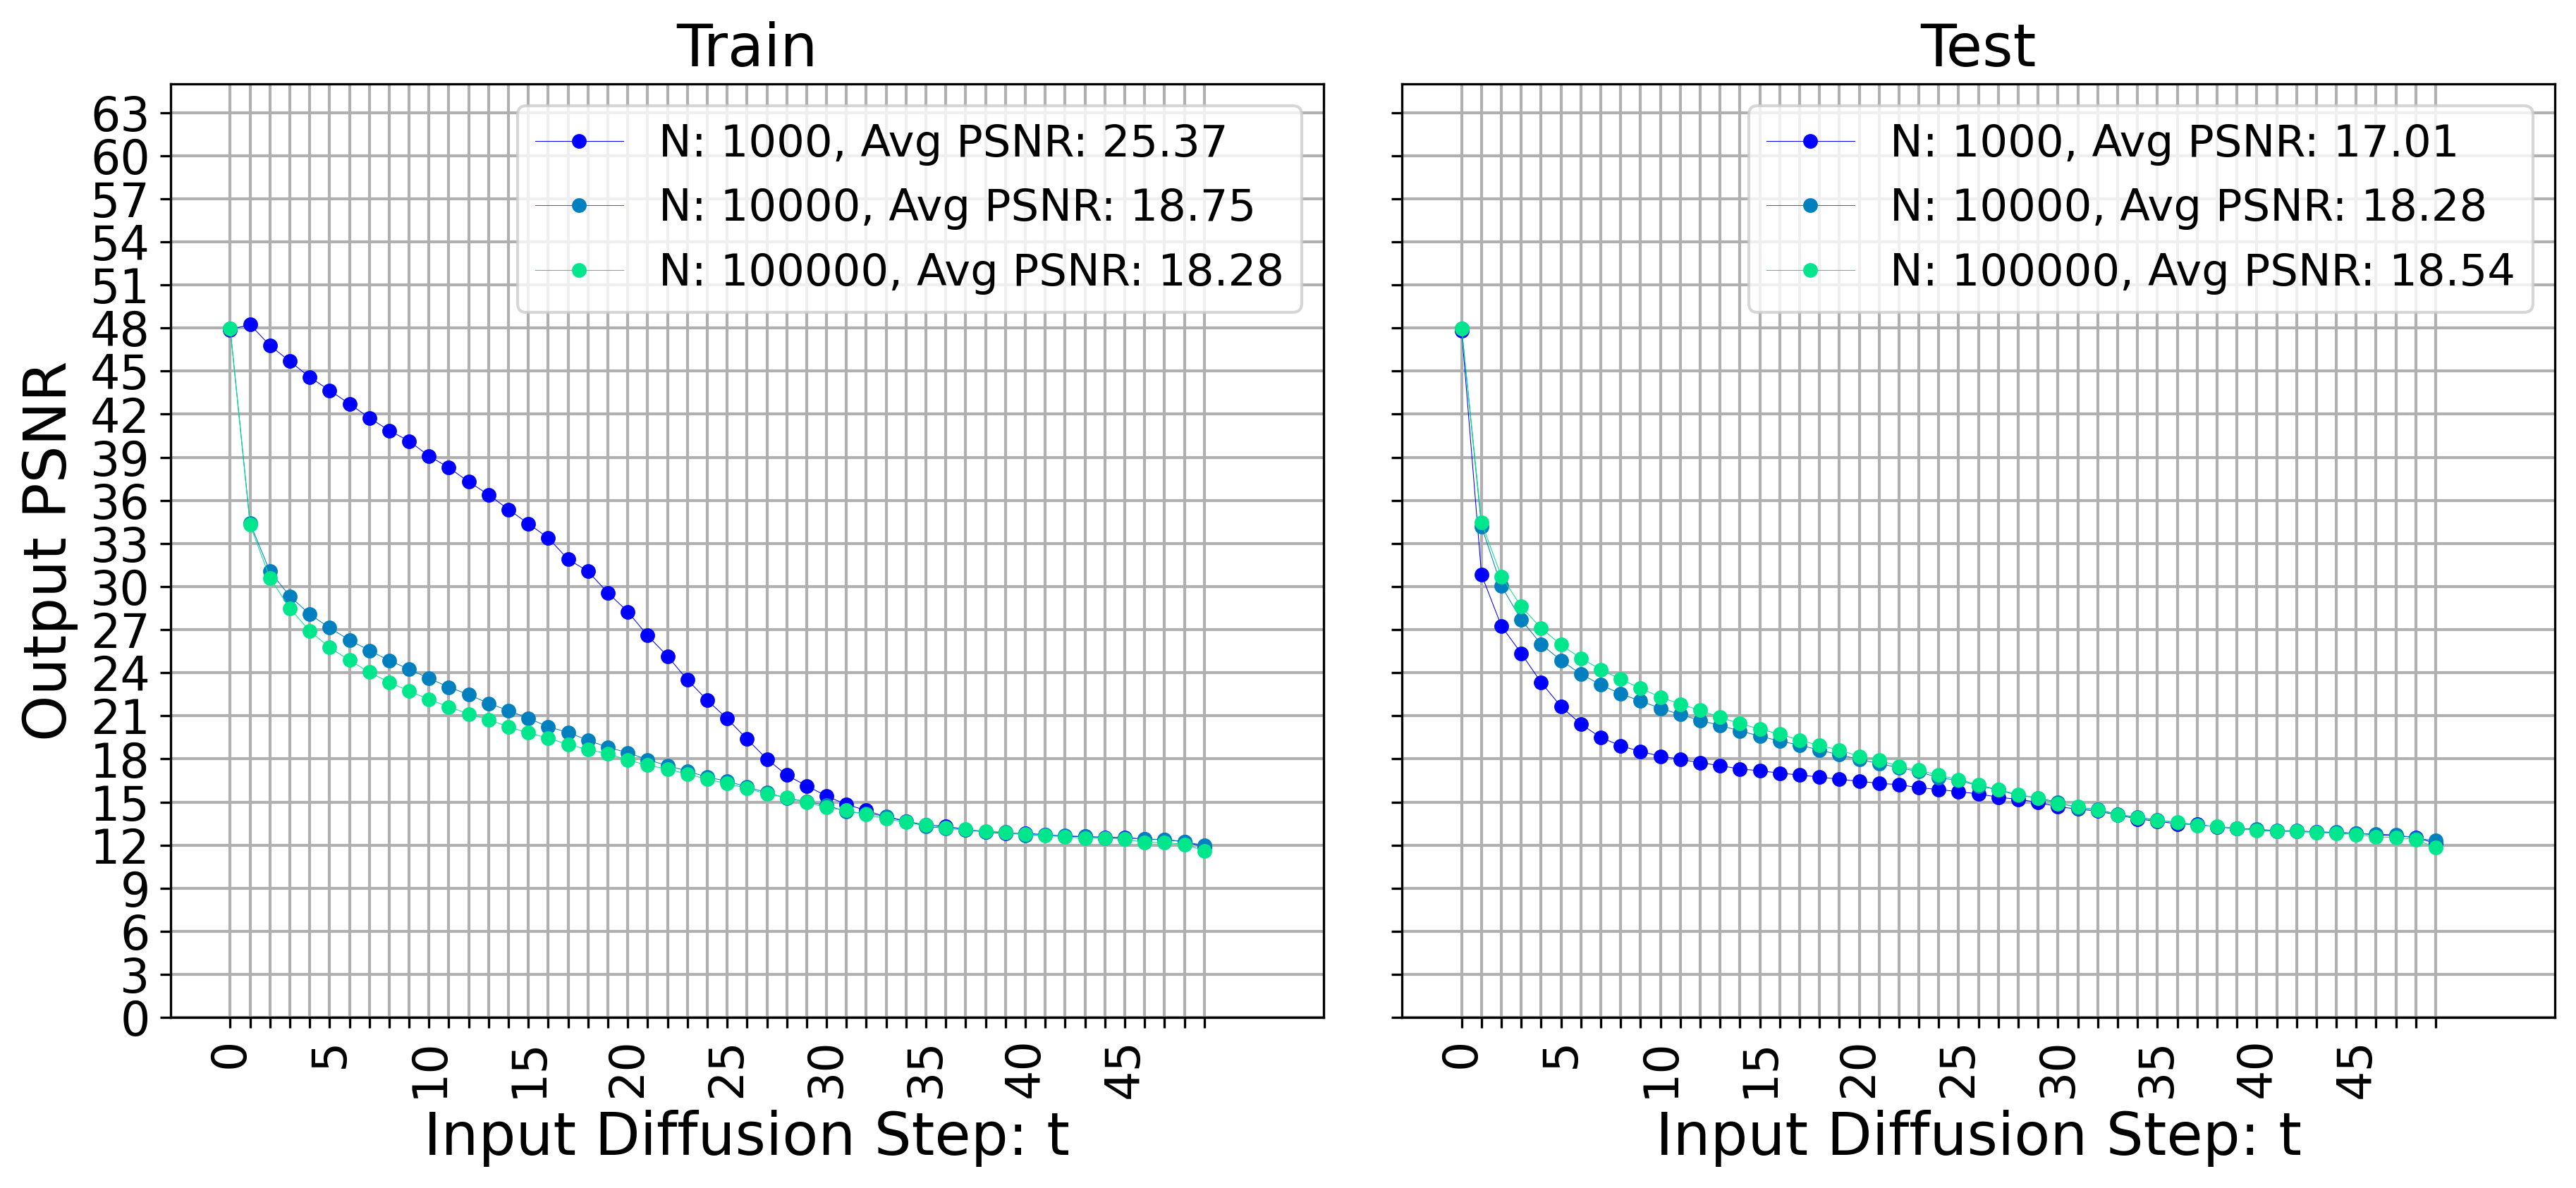}}
&
\raisebox{-0.5\height}{\includegraphics[width=.41\textwidth]{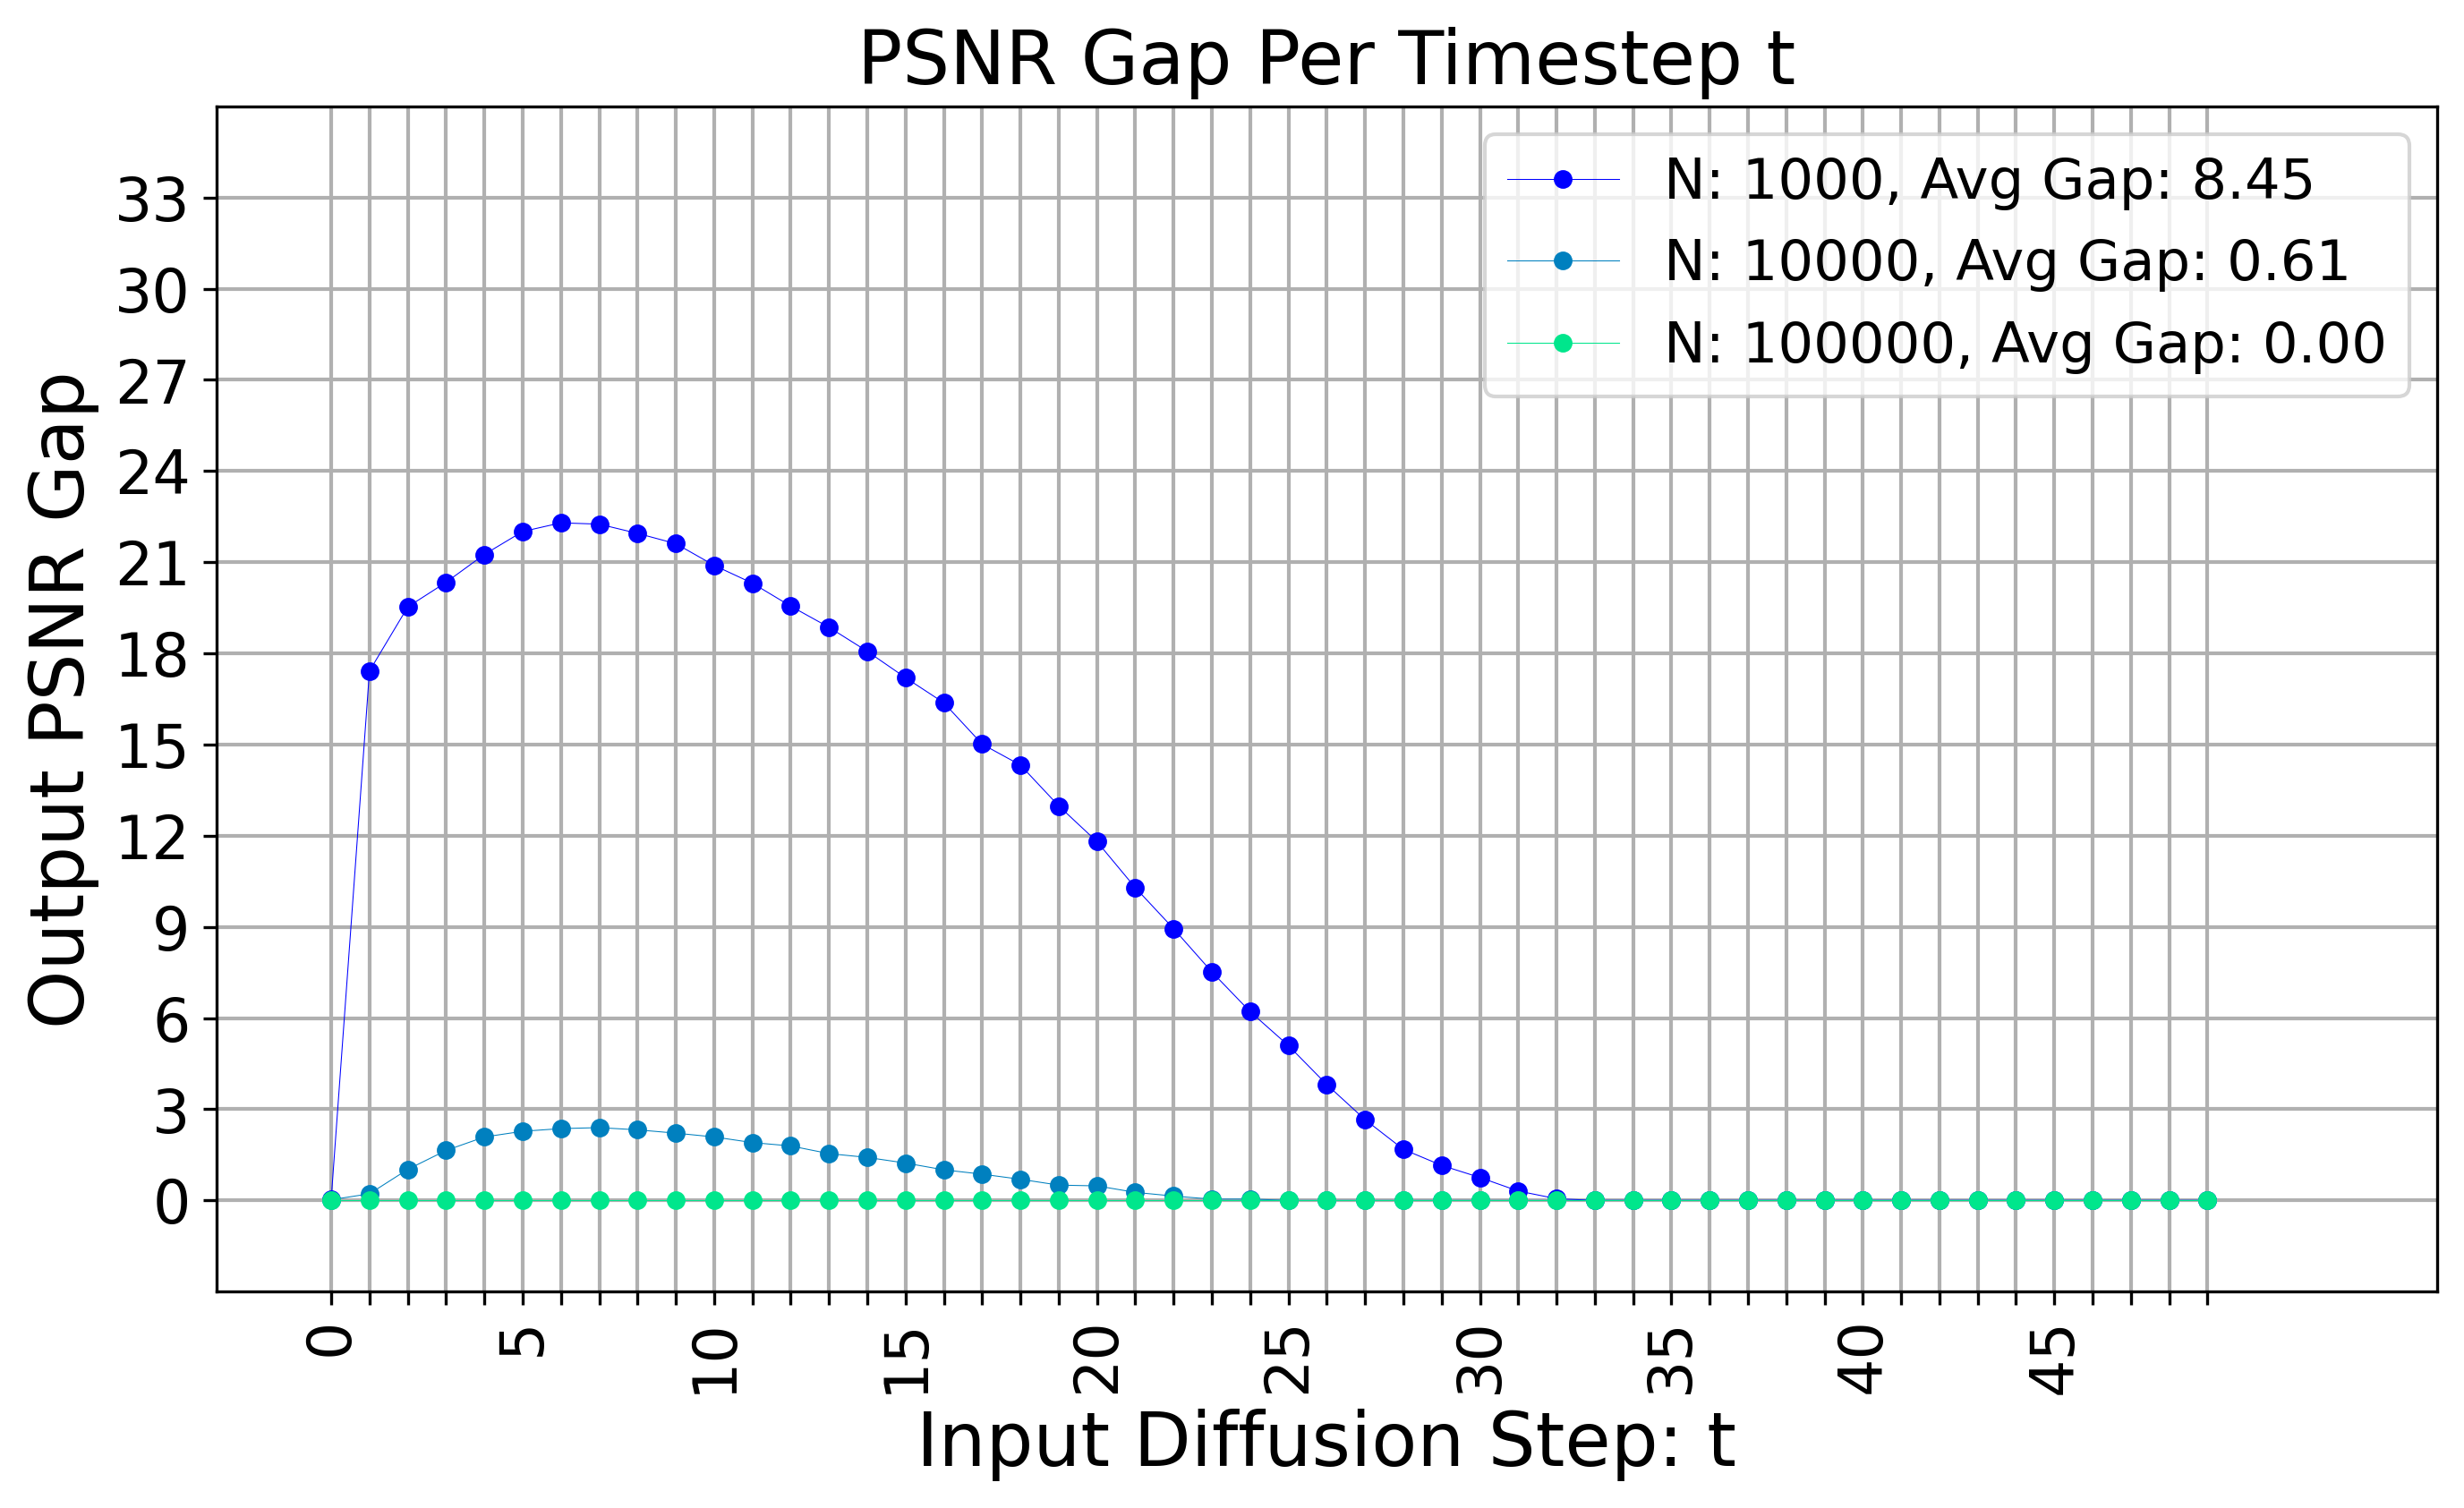}}
\\
\hline
\cellcolor{diff}{\STAB{\rotatebox[origin=c]{90}{DiT-S/1 w/ Local}}}
&
\raisebox{-0.5\height}{\includegraphics[width=.54\textwidth]{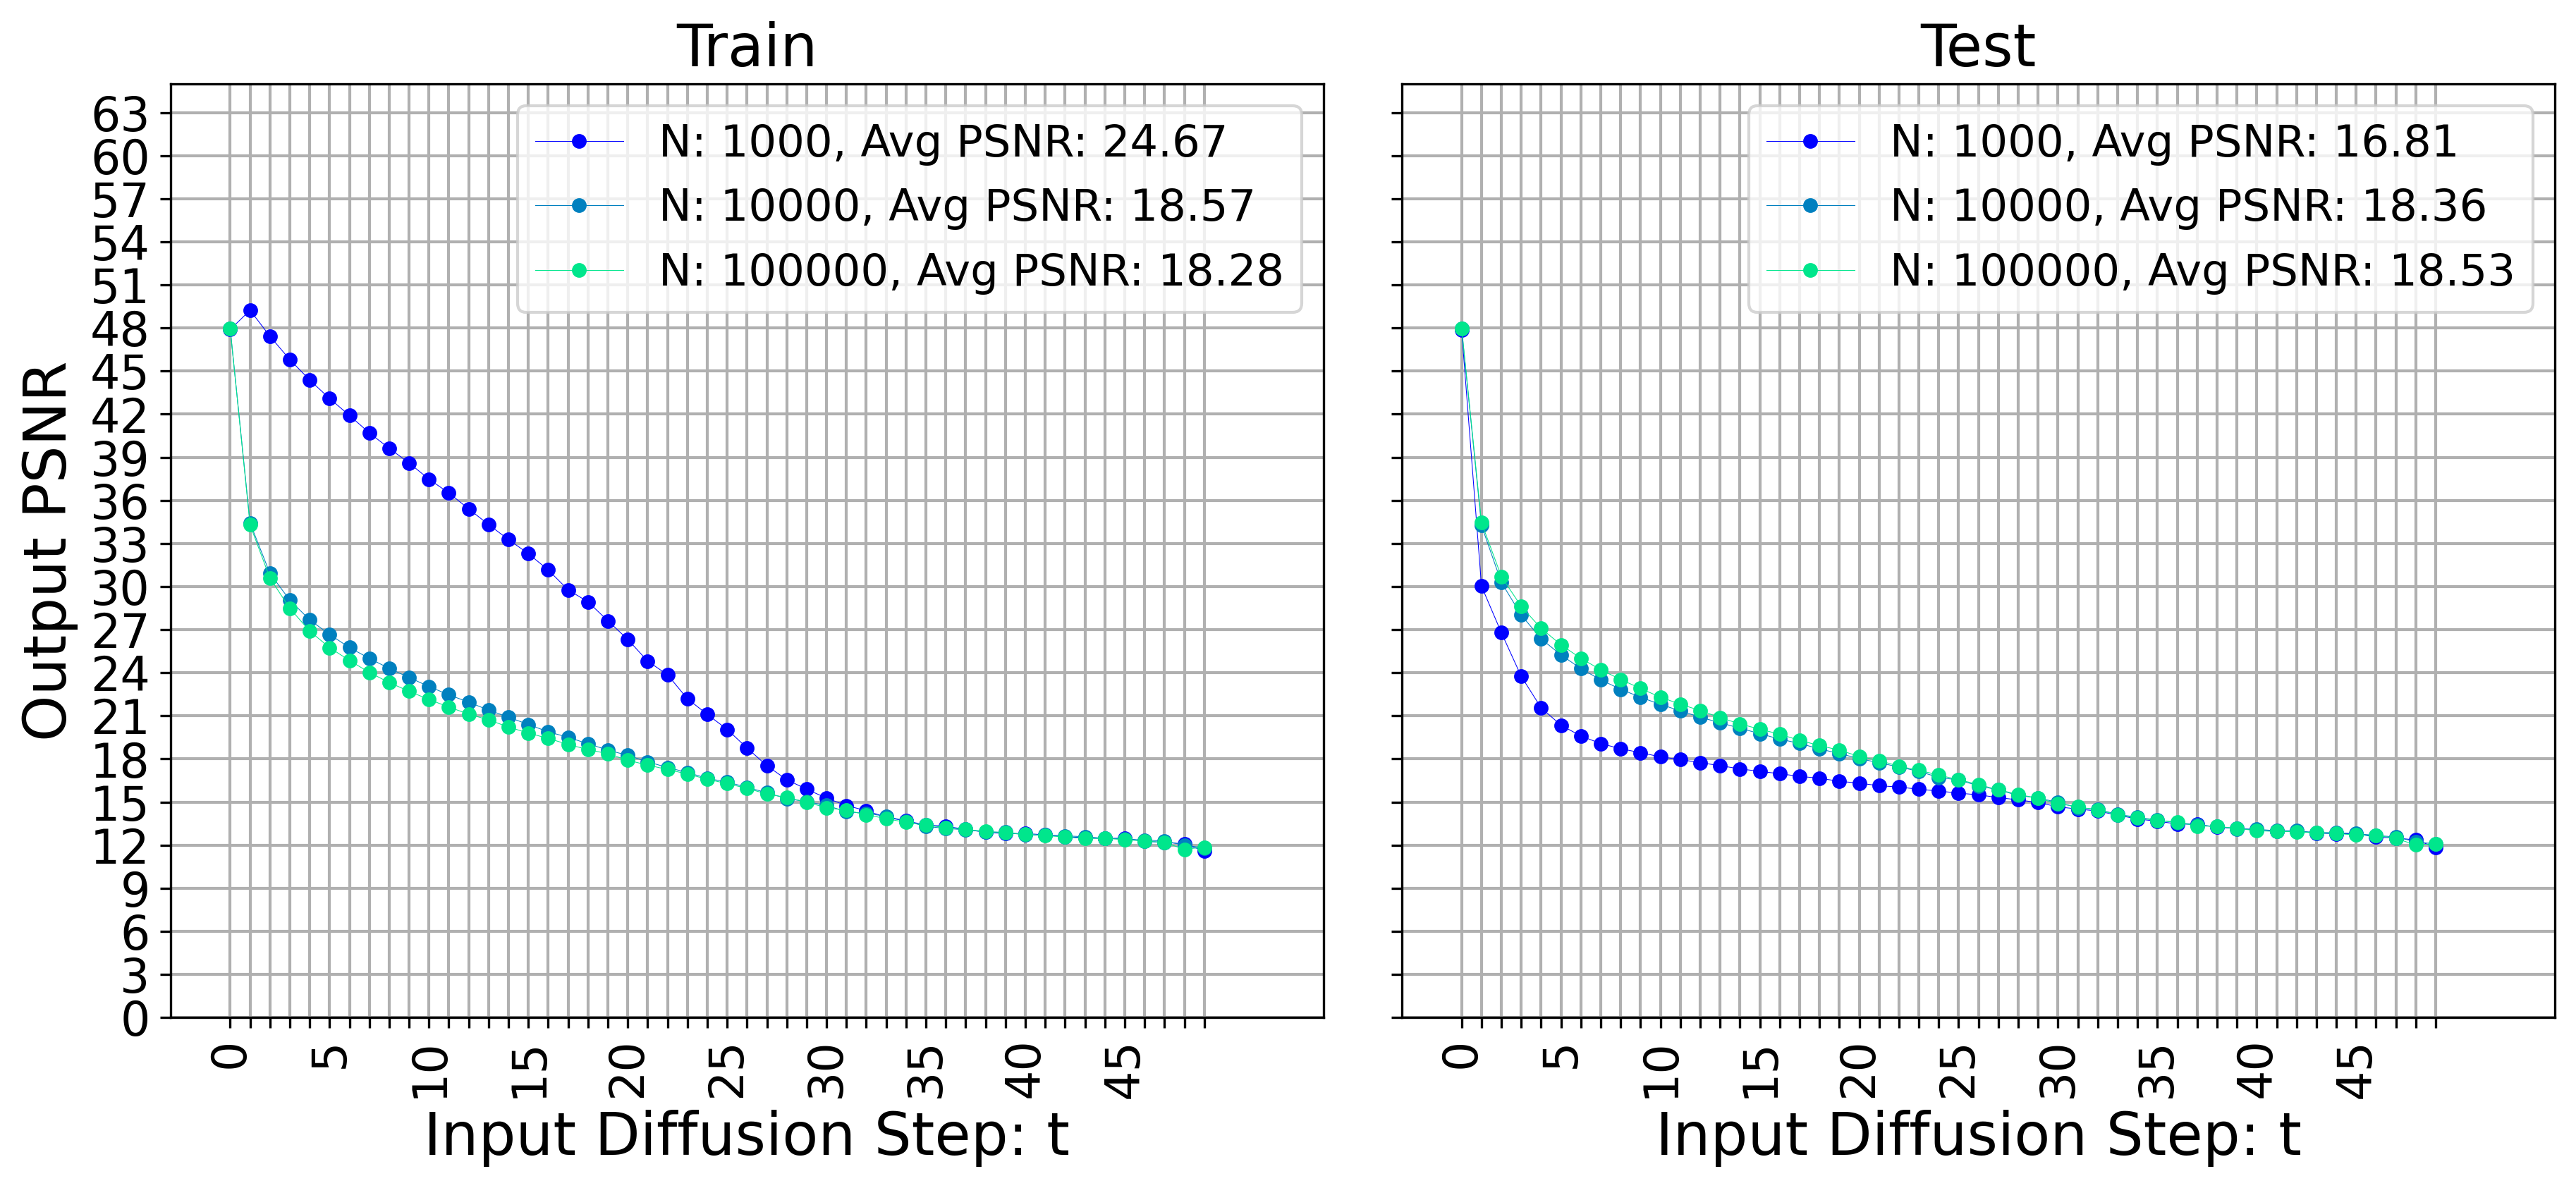}}
&
\raisebox{-0.5\height}{\includegraphics[width=.41\textwidth]{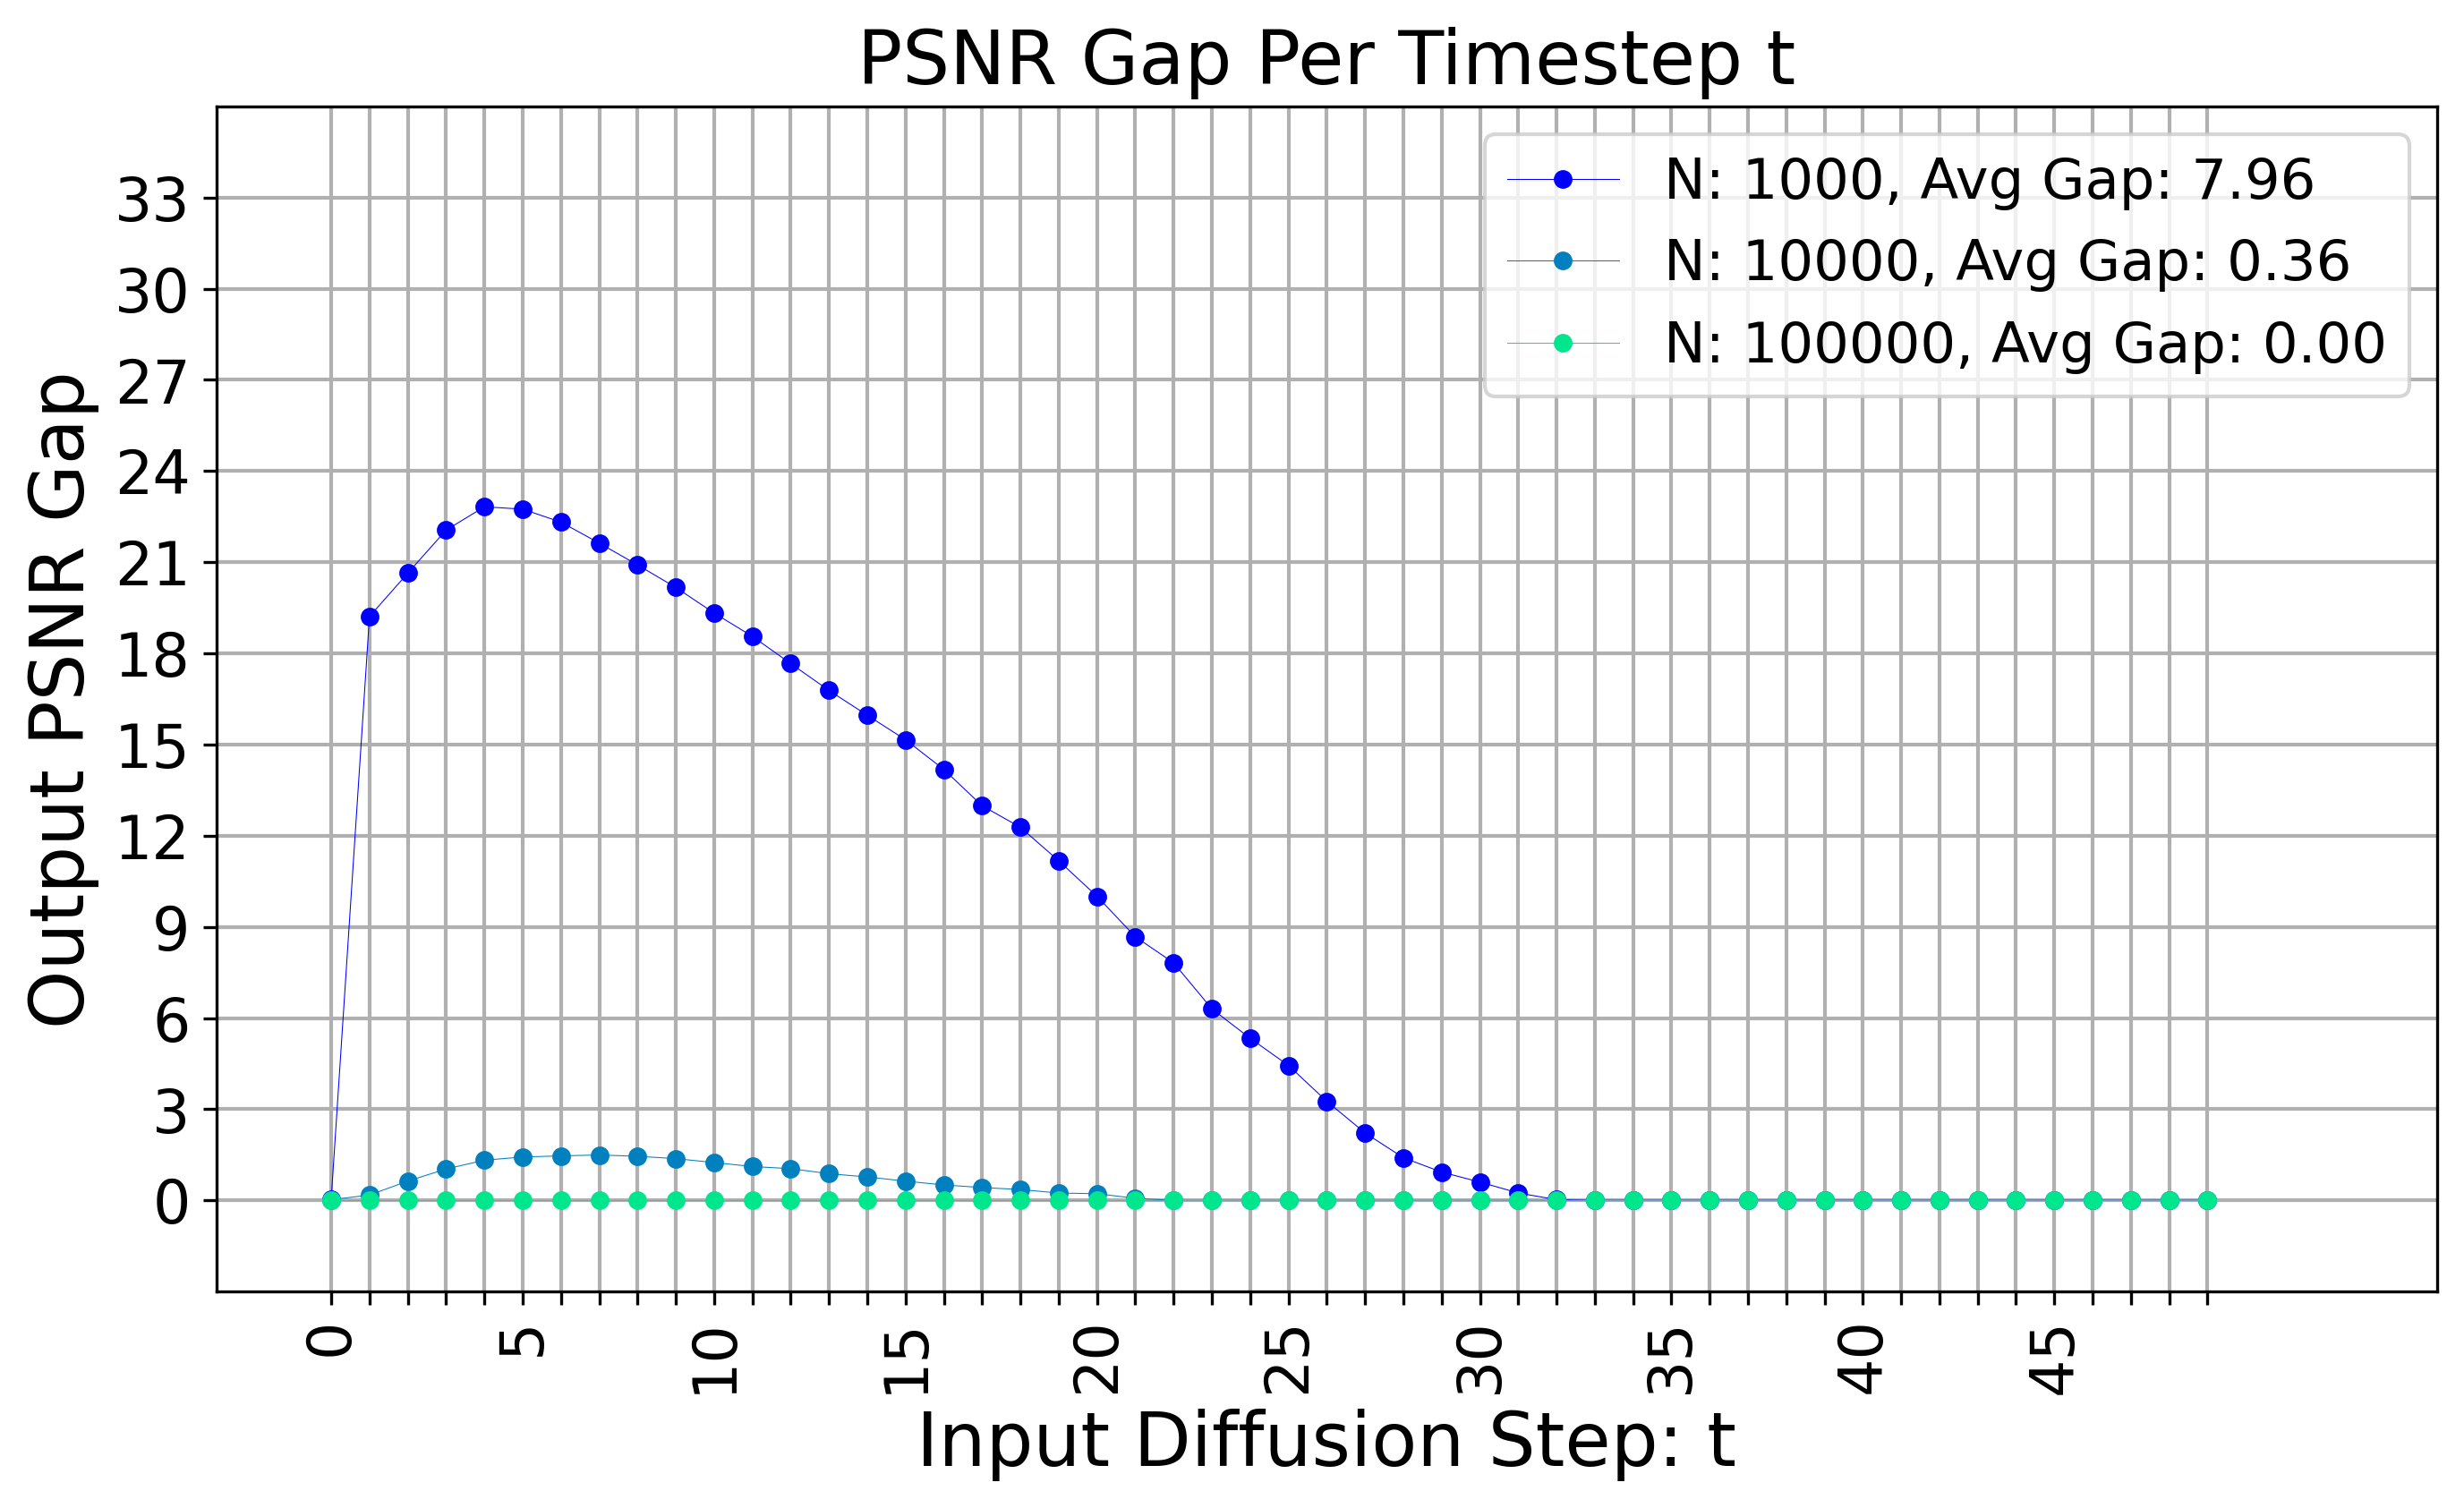}}
\\
&
\multicolumn{1}{c}{(a) PSNR Curves of Training and Testing Sets}
&
\multicolumn{1}{c}{(b) PSNR Gap}
\\
\end{tabular}

\captionof{figure}{The PSNR (a) and PSNR gap (b) comparison on the LSUN (Church)~\citep{yu15lsun} dataset.}
\label{fig:row_psnr_church}
\end{table}

\begin{table}[ht]
\centering
\small
\setlength\tabcolsep{1pt}
\setlength{\extrarowheight}{4pt}
\begin{tabular}{lc|c}
\cellcolor{dit}{\STAB{\rotatebox[origin=c]{90}{DiT-XS/1}}}
&
\raisebox{-0.5\height}{\includegraphics[width=.54\textwidth]{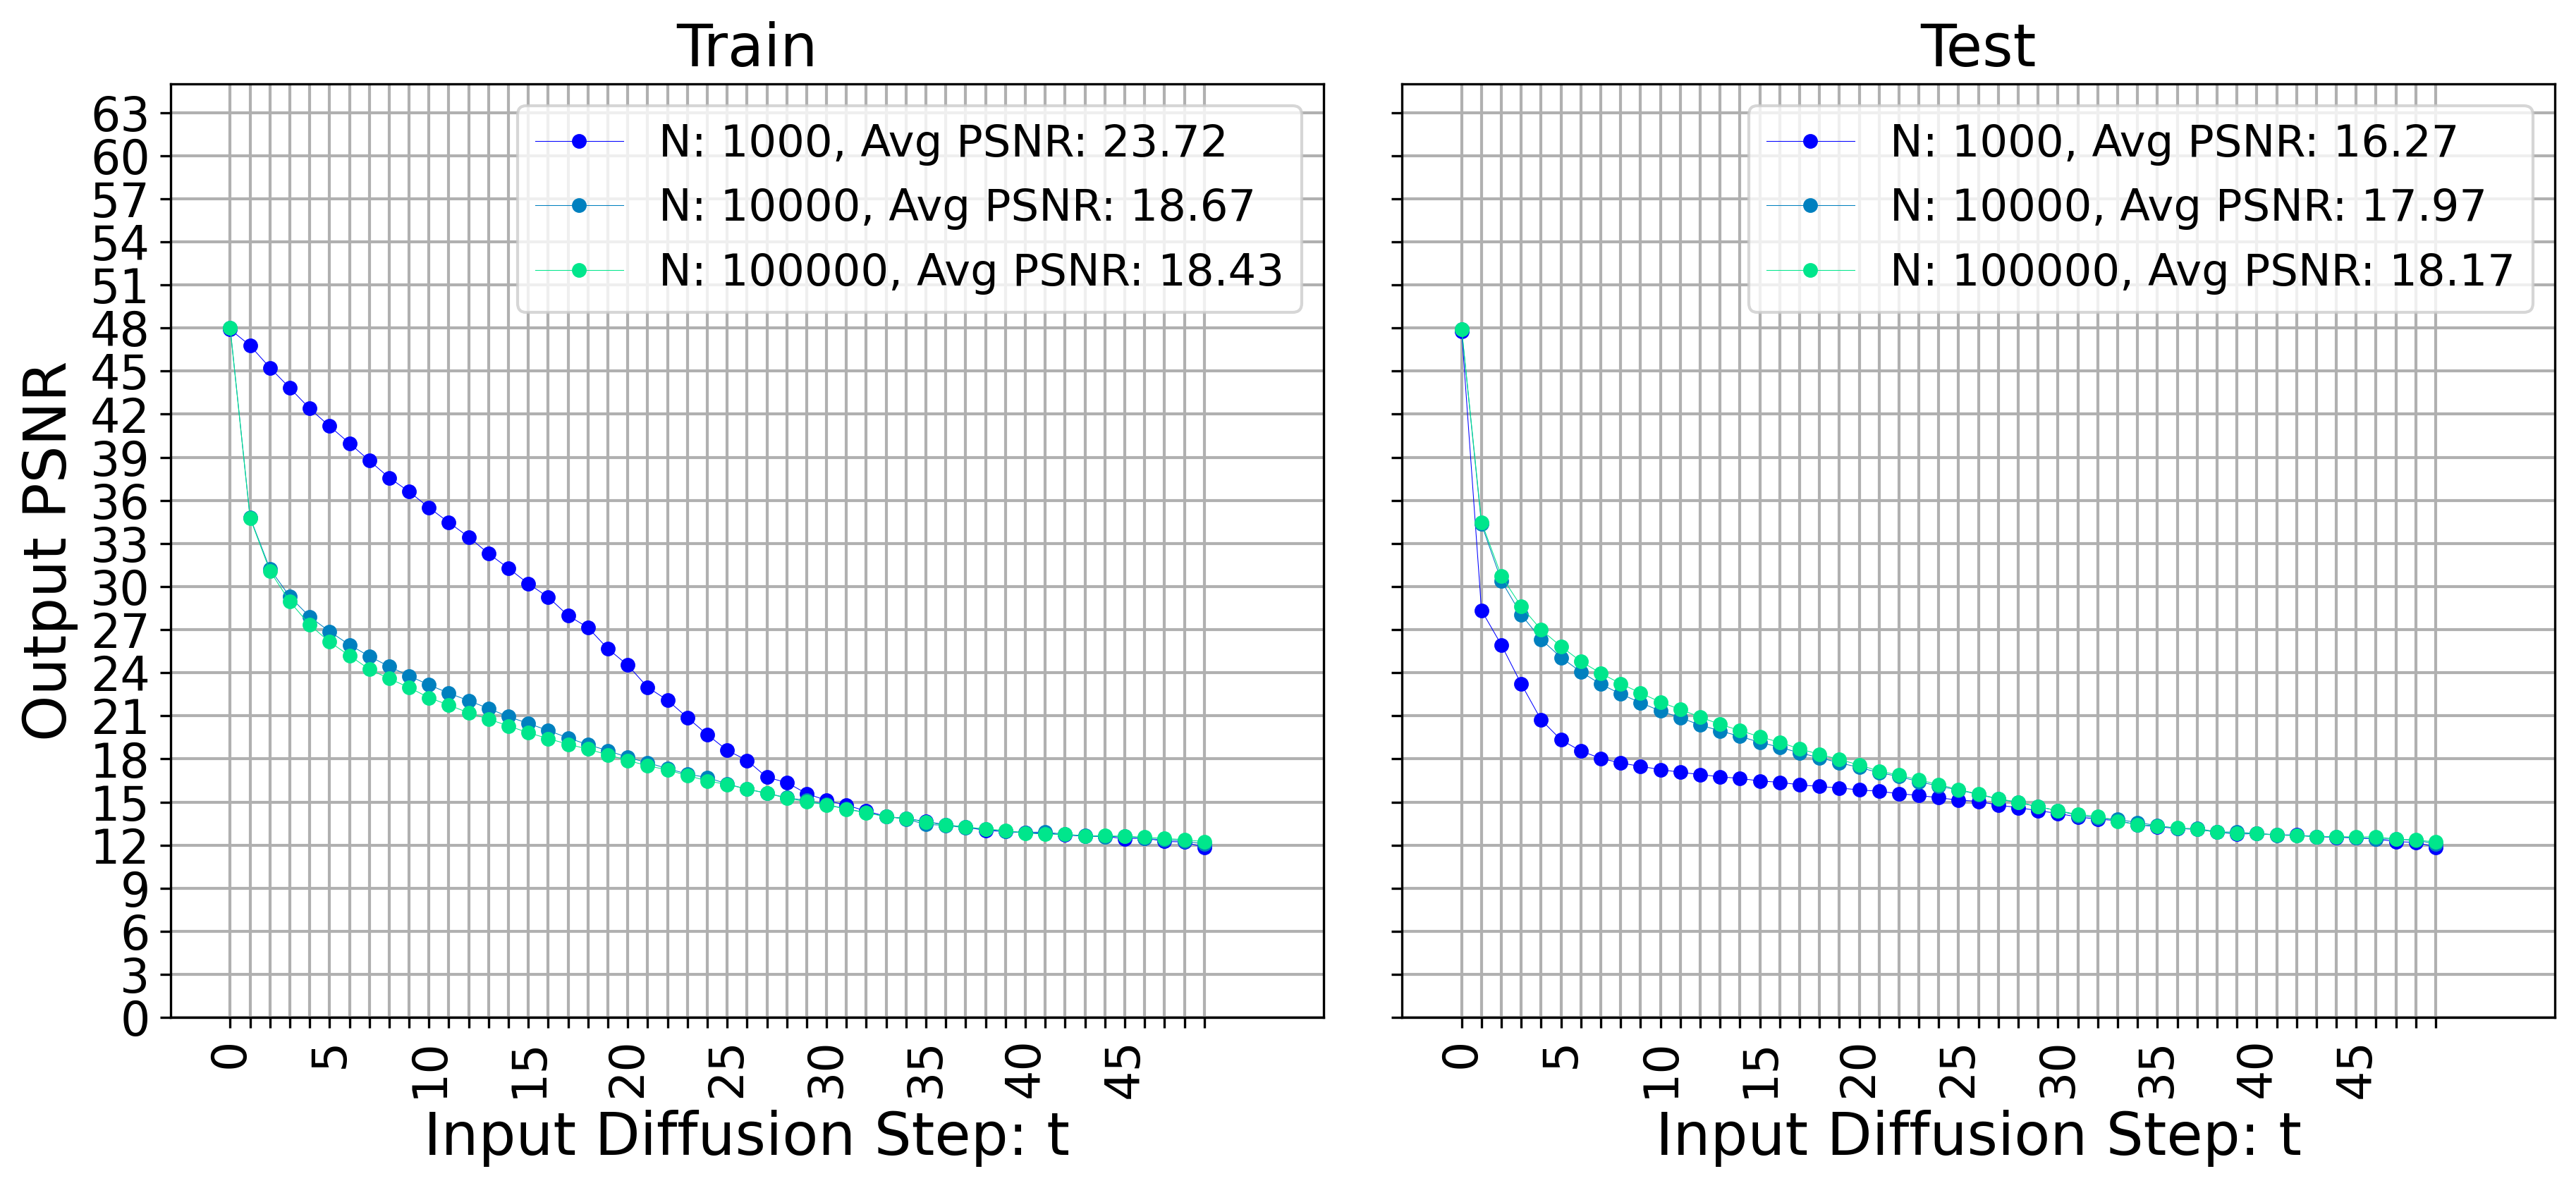}}
&
\raisebox{-0.5\height}{\includegraphics[width=.41\textwidth]{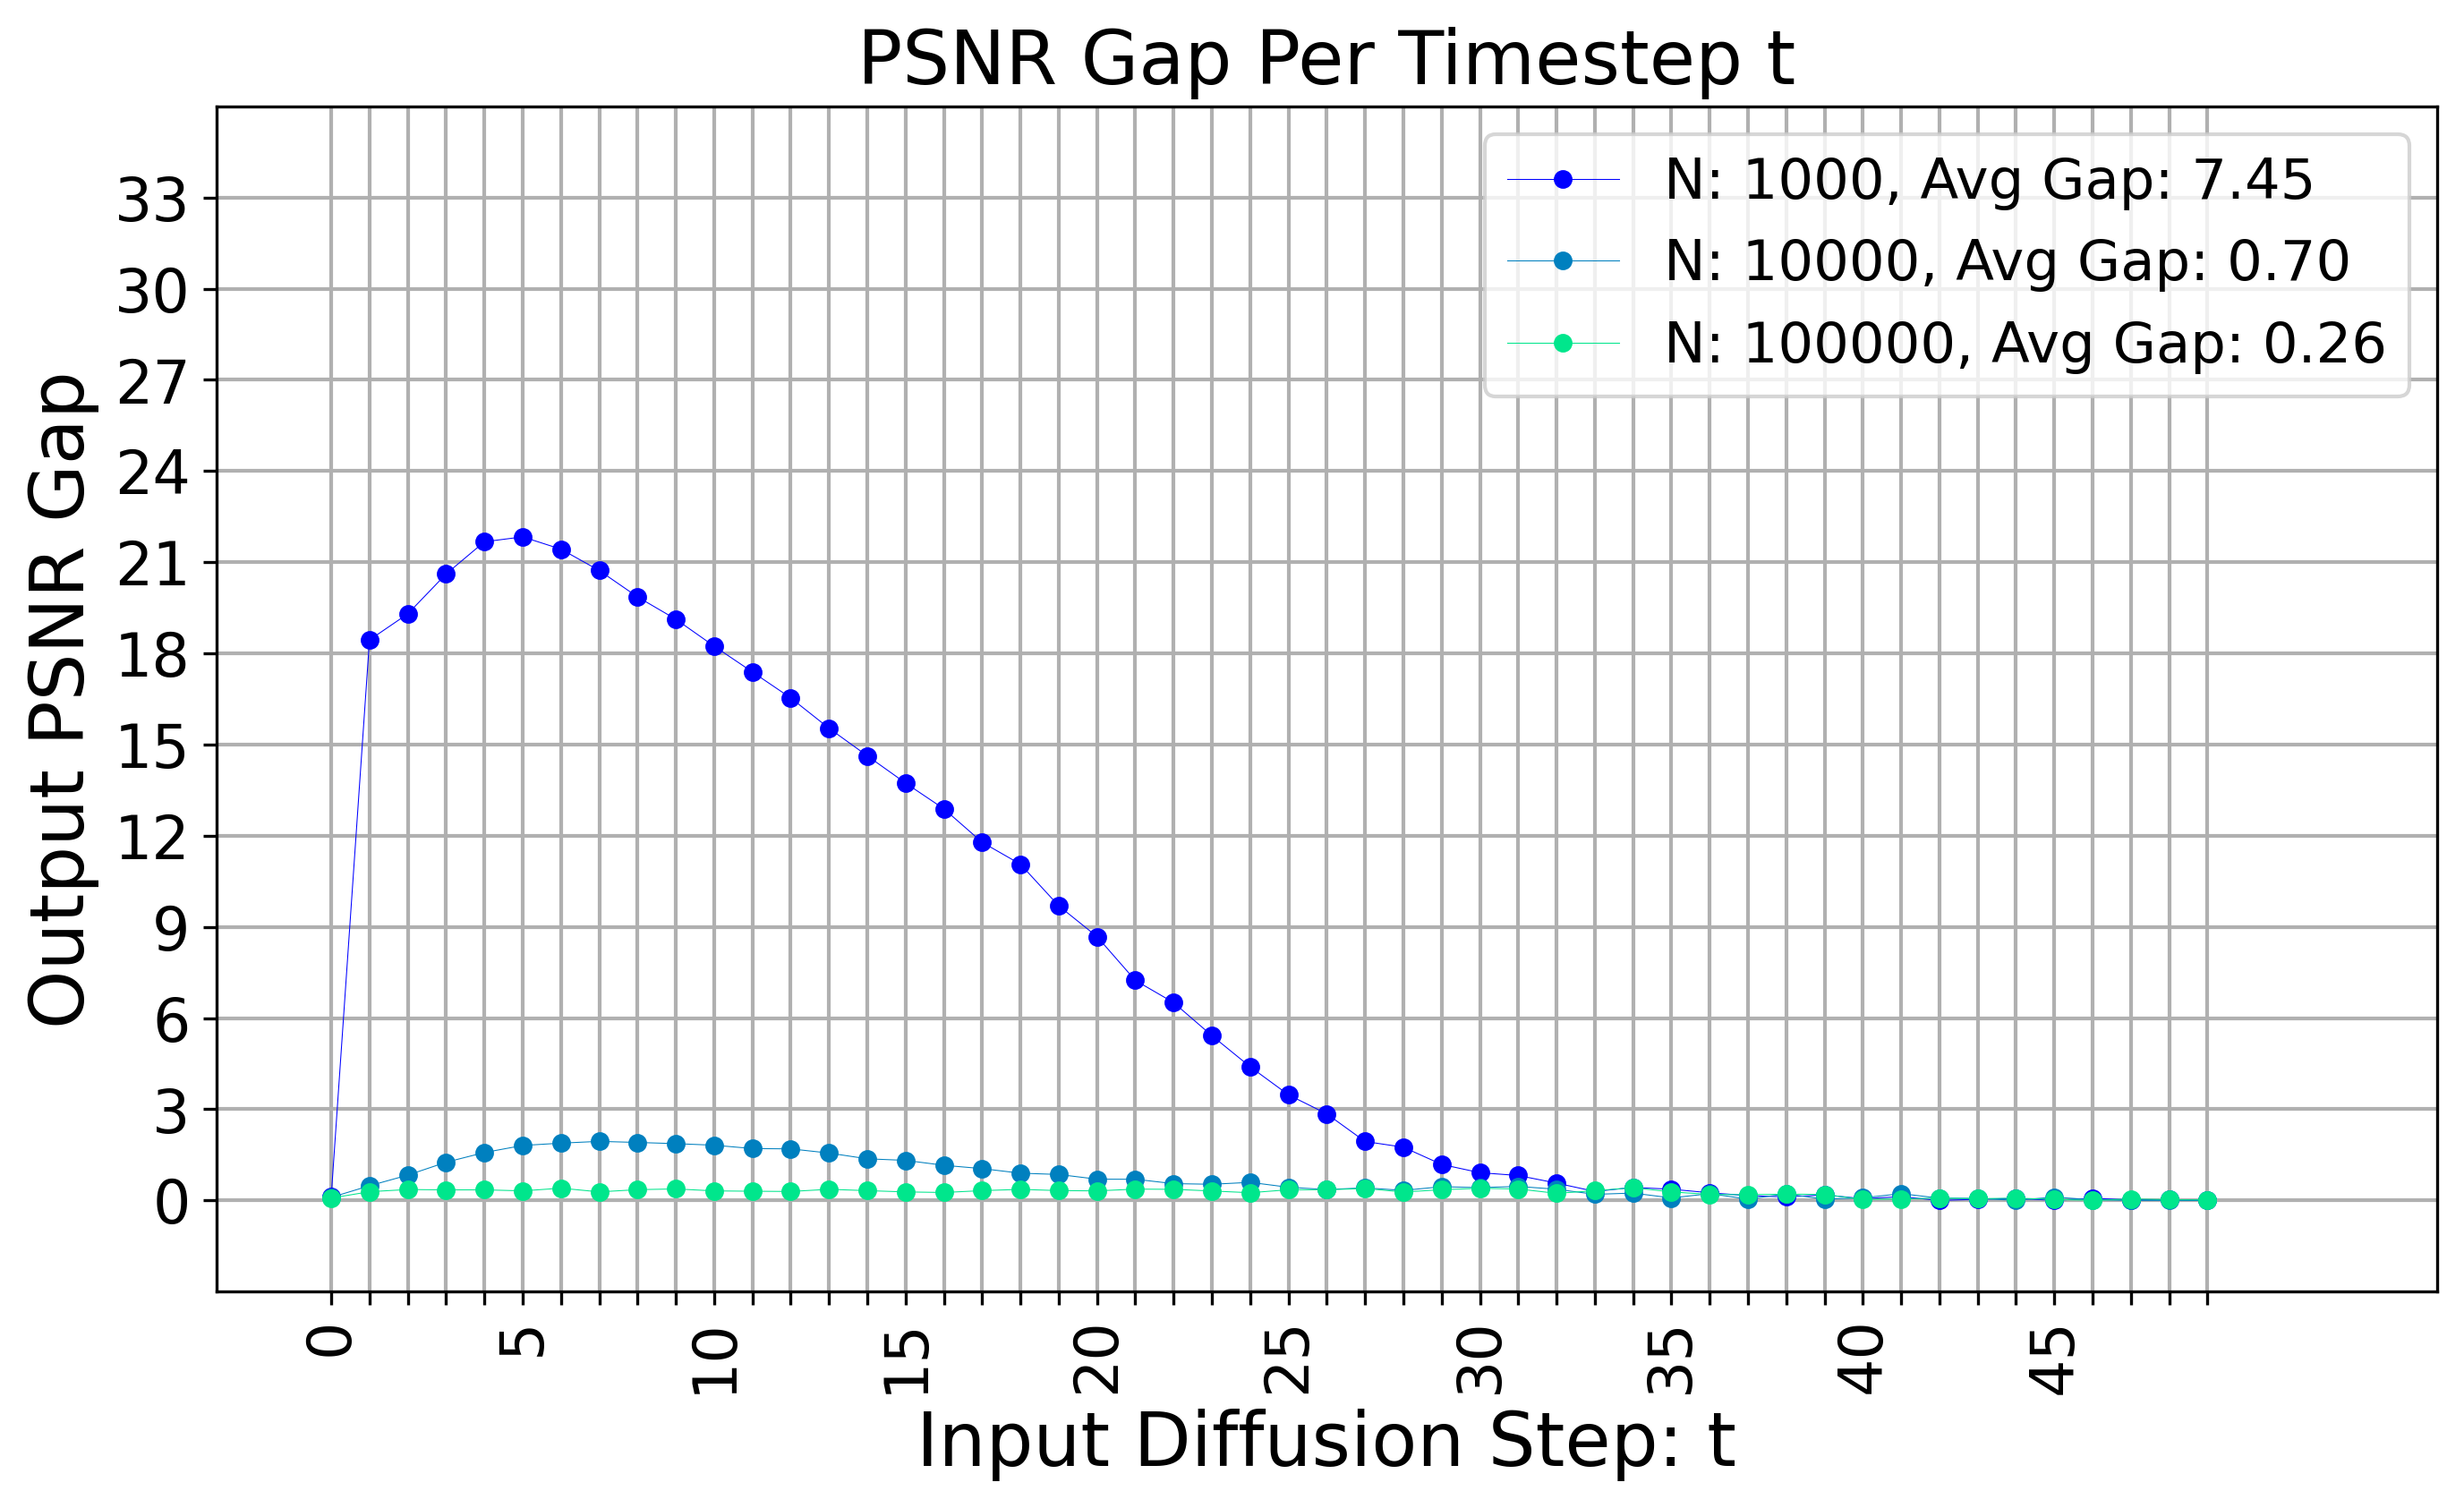}}
\\
\hline
\cellcolor{diff}{\STAB{\rotatebox[origin=c]{90}{DiT-XS/1 w/ Local}}}
&
\raisebox{-0.5\height}{\includegraphics[width=.54\textwidth]{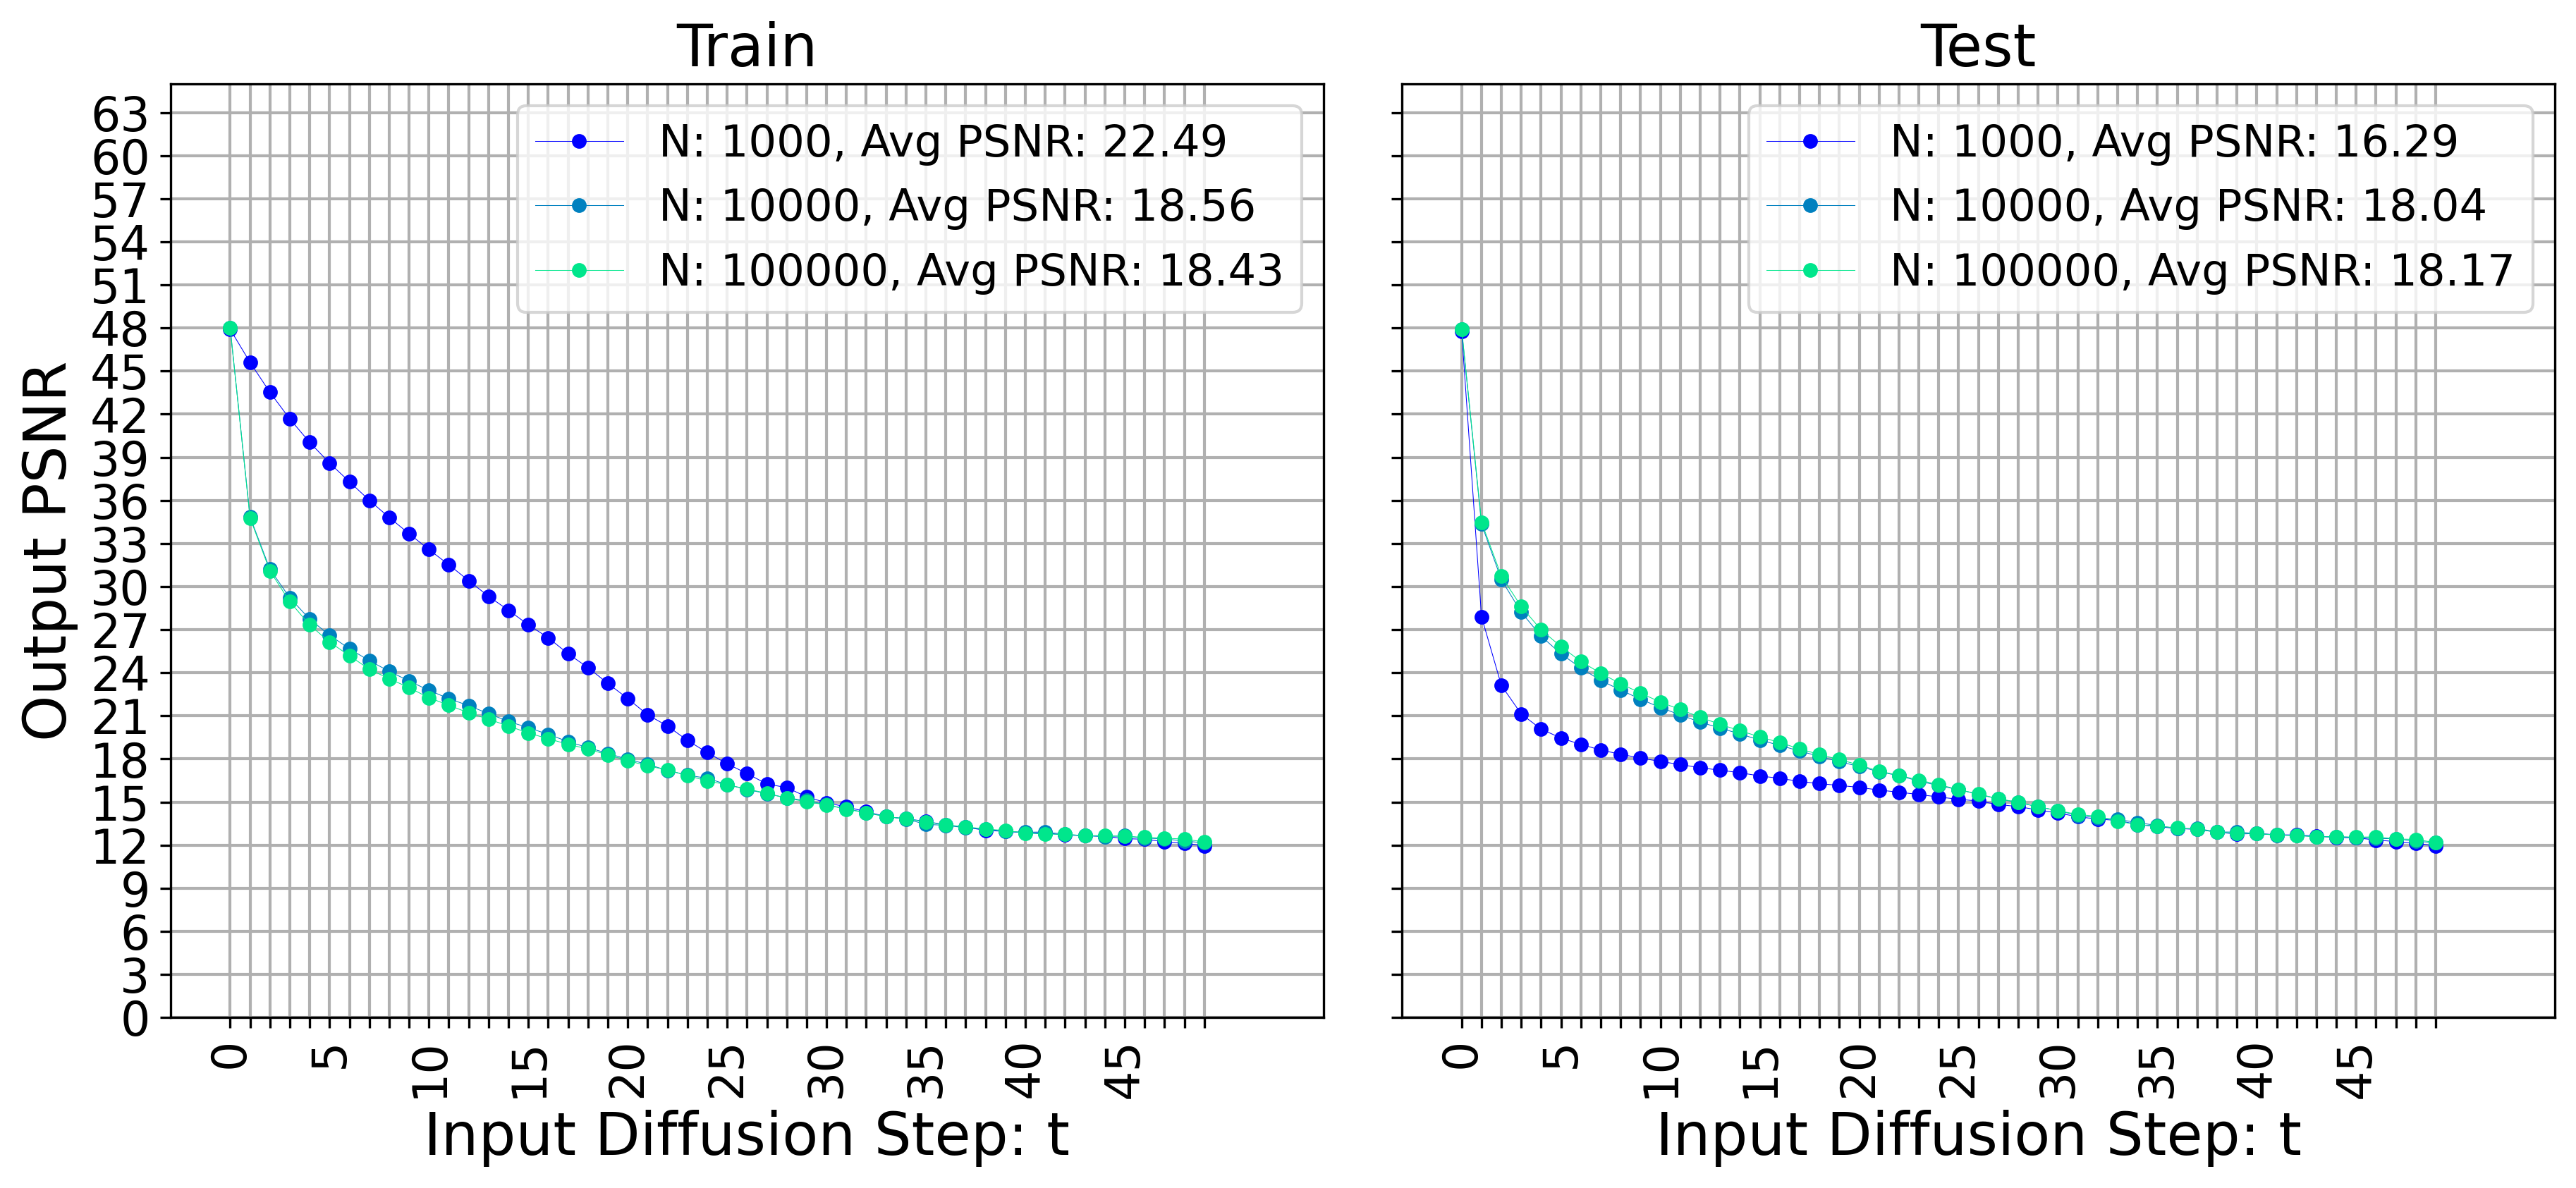}}
&
\raisebox{-0.5\height}{\includegraphics[width=.41\textwidth]{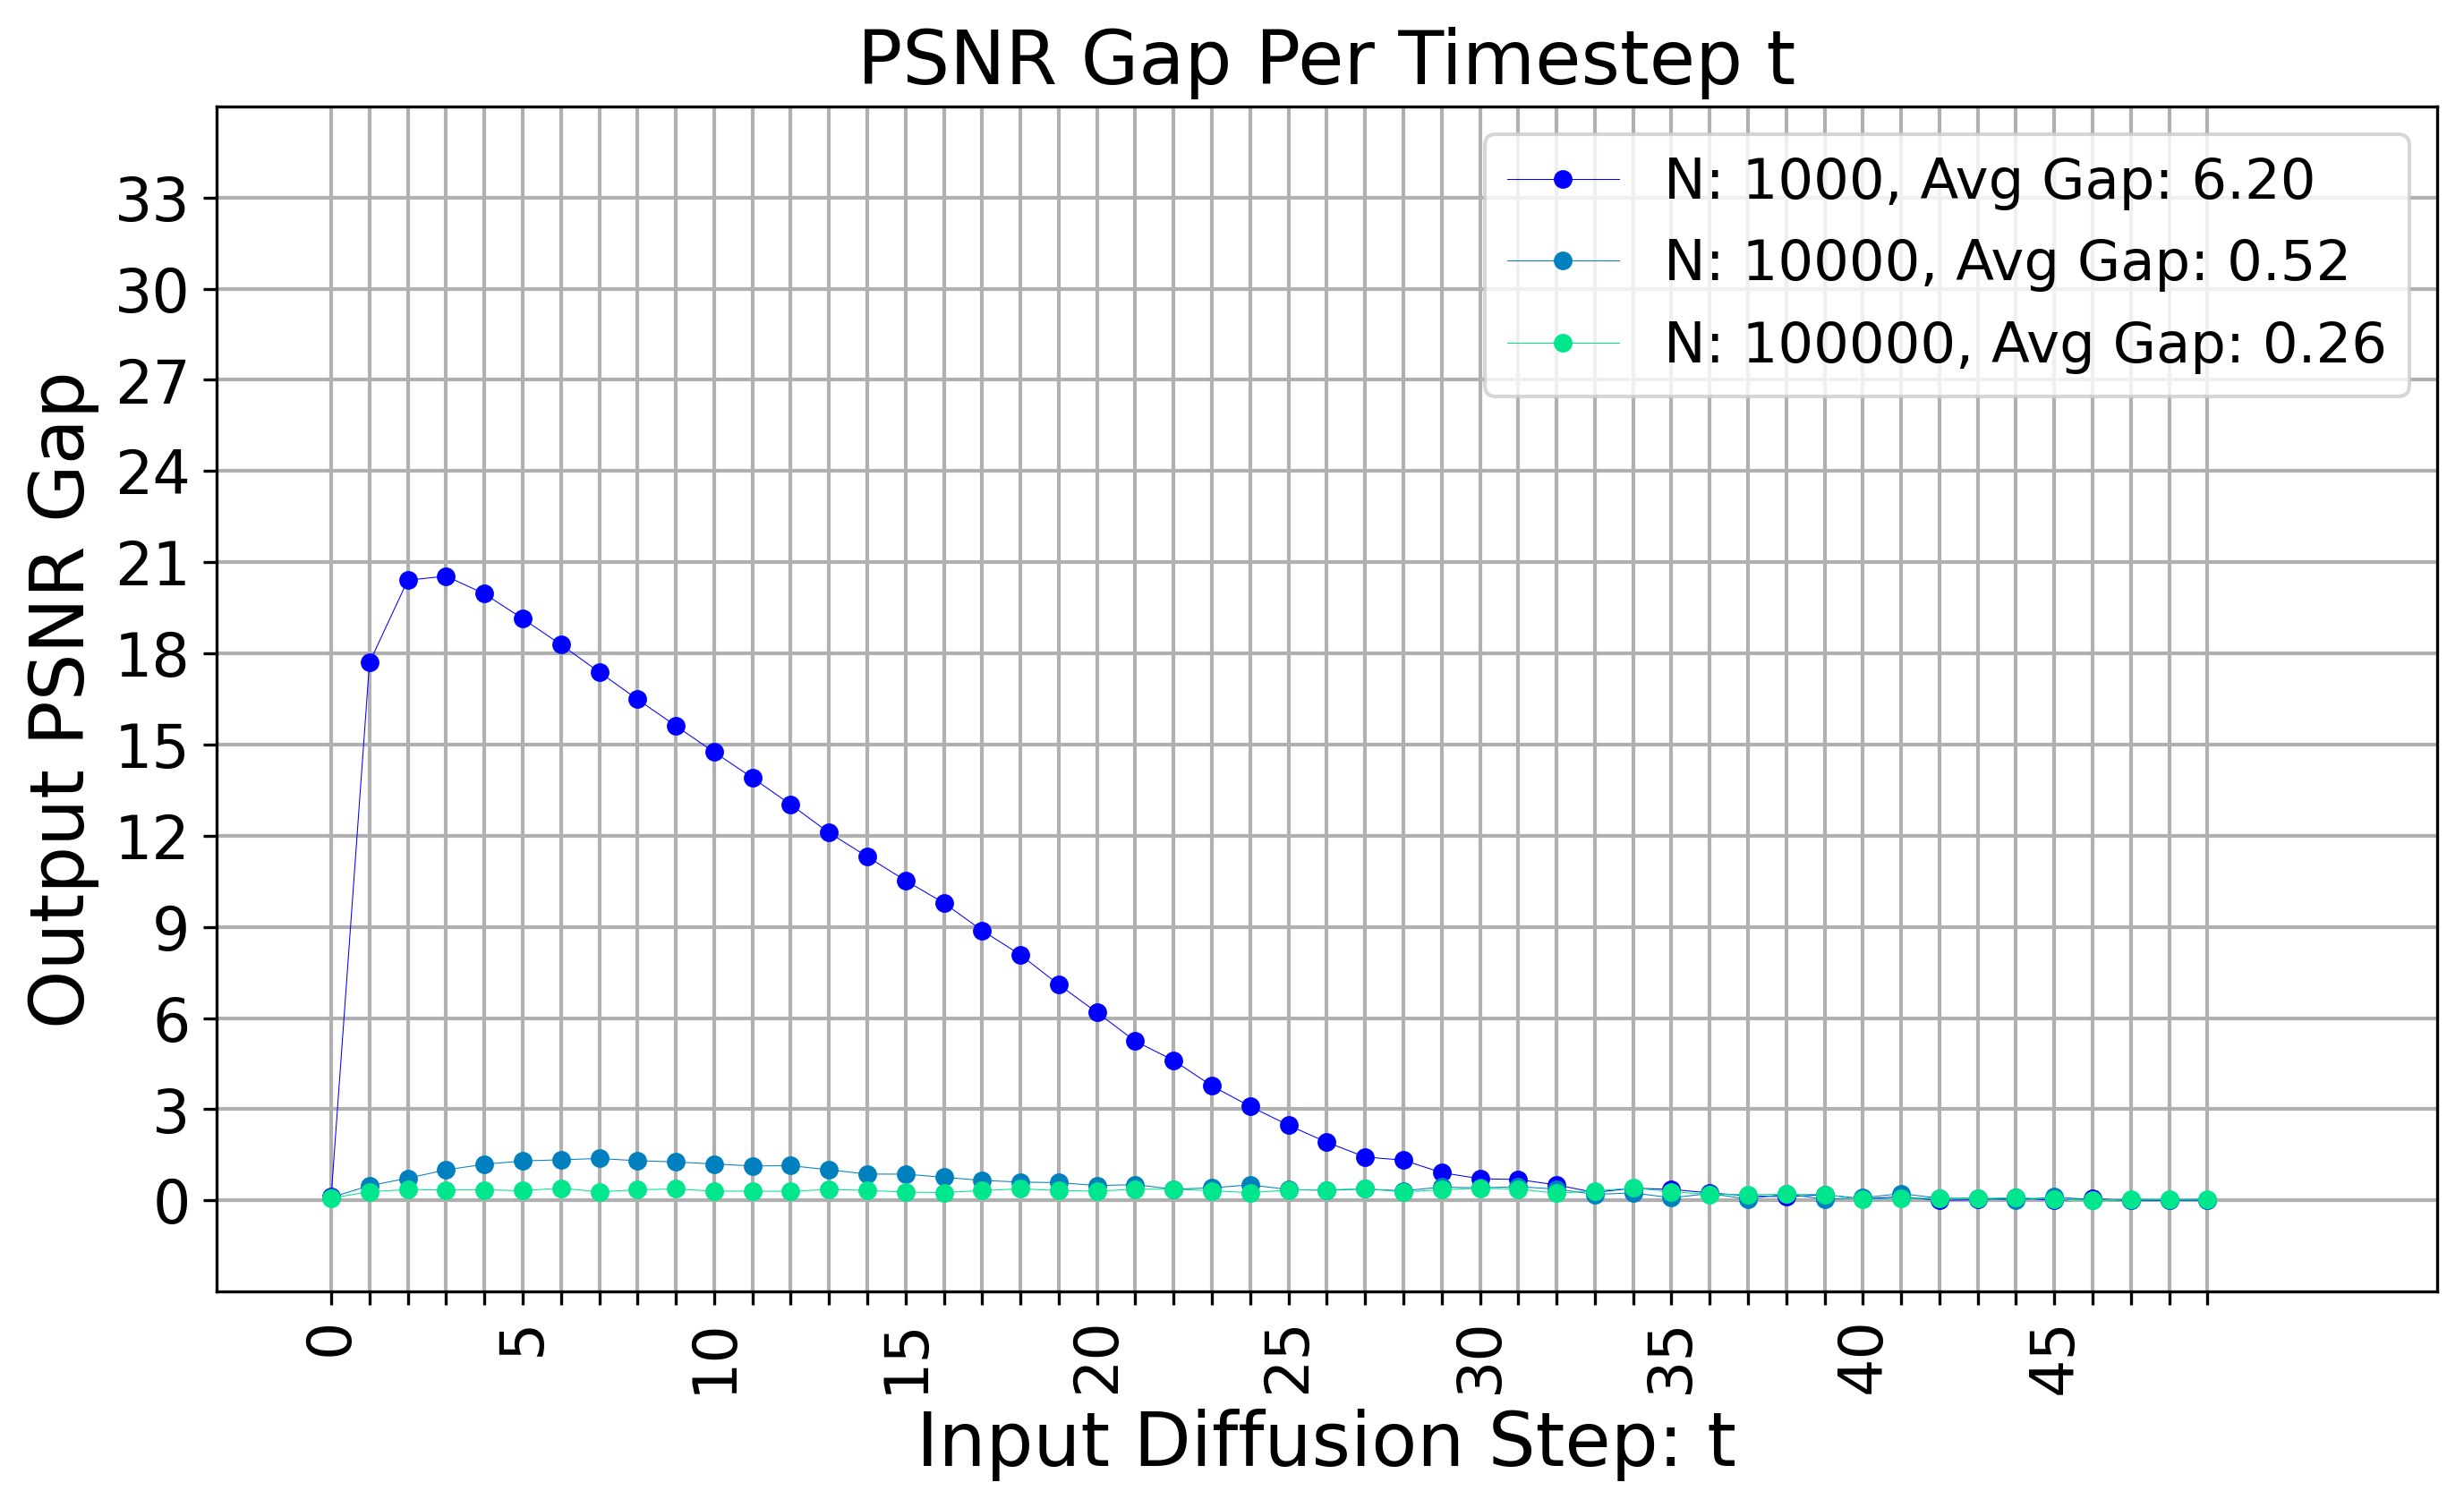}}
\\
\hline
\cellcolor{dit}{\STAB{\rotatebox[origin=c]{90}{DiT-S/1}}}
&
\raisebox{-0.5\height}{\includegraphics[width=.54\textwidth]{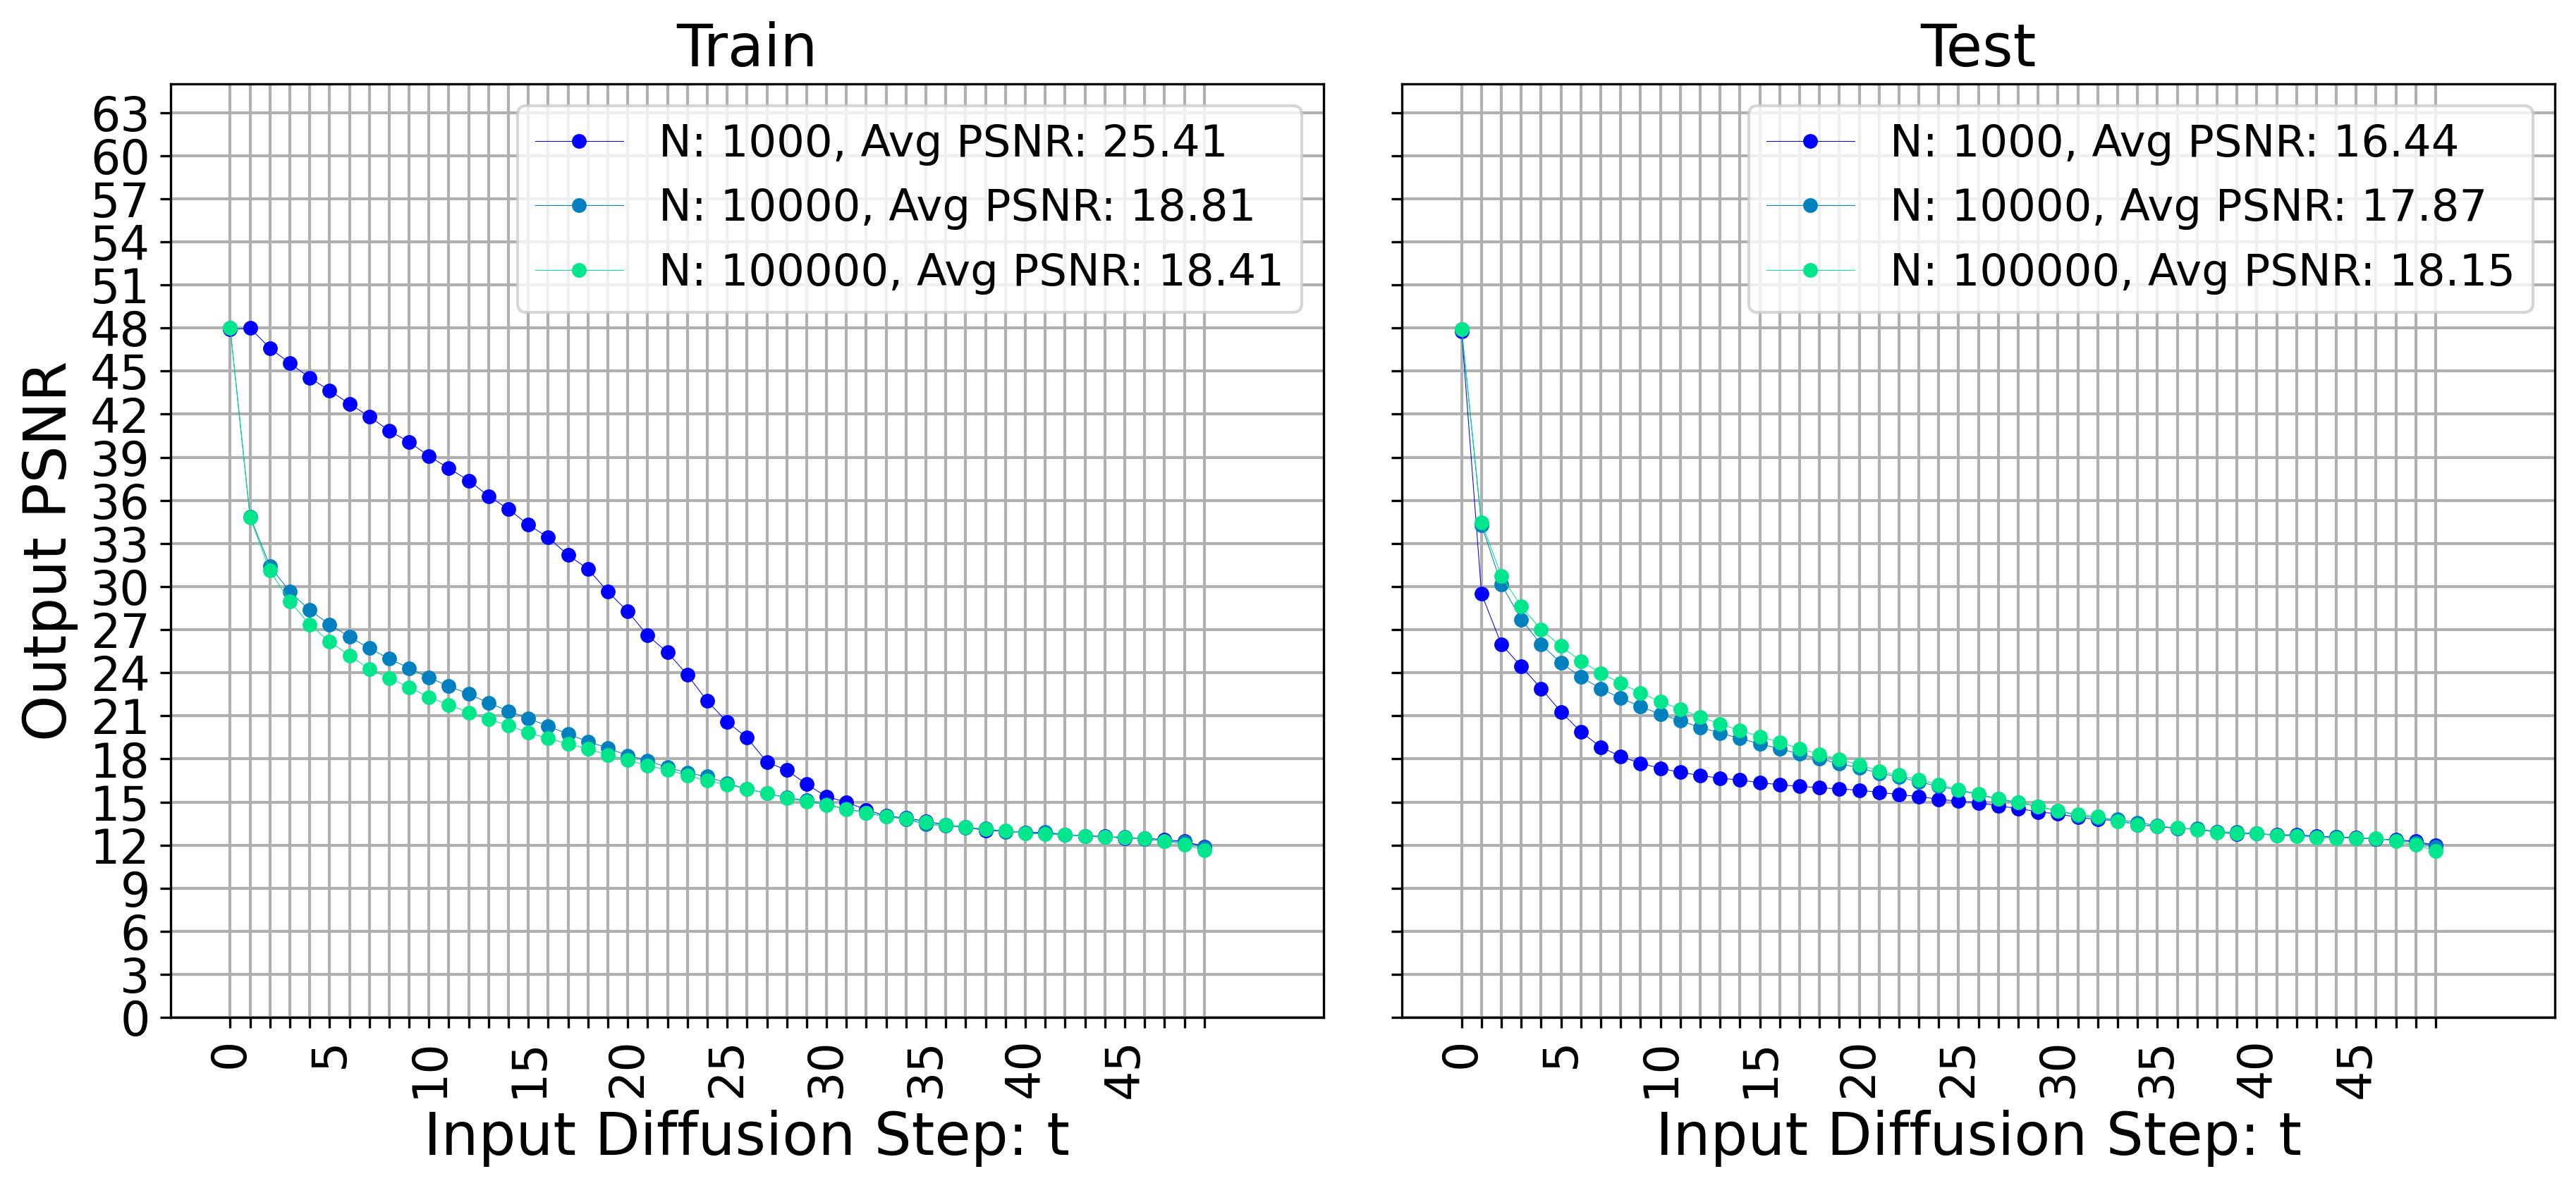}}
&
\raisebox{-0.5\height}{\includegraphics[width=.41\textwidth]{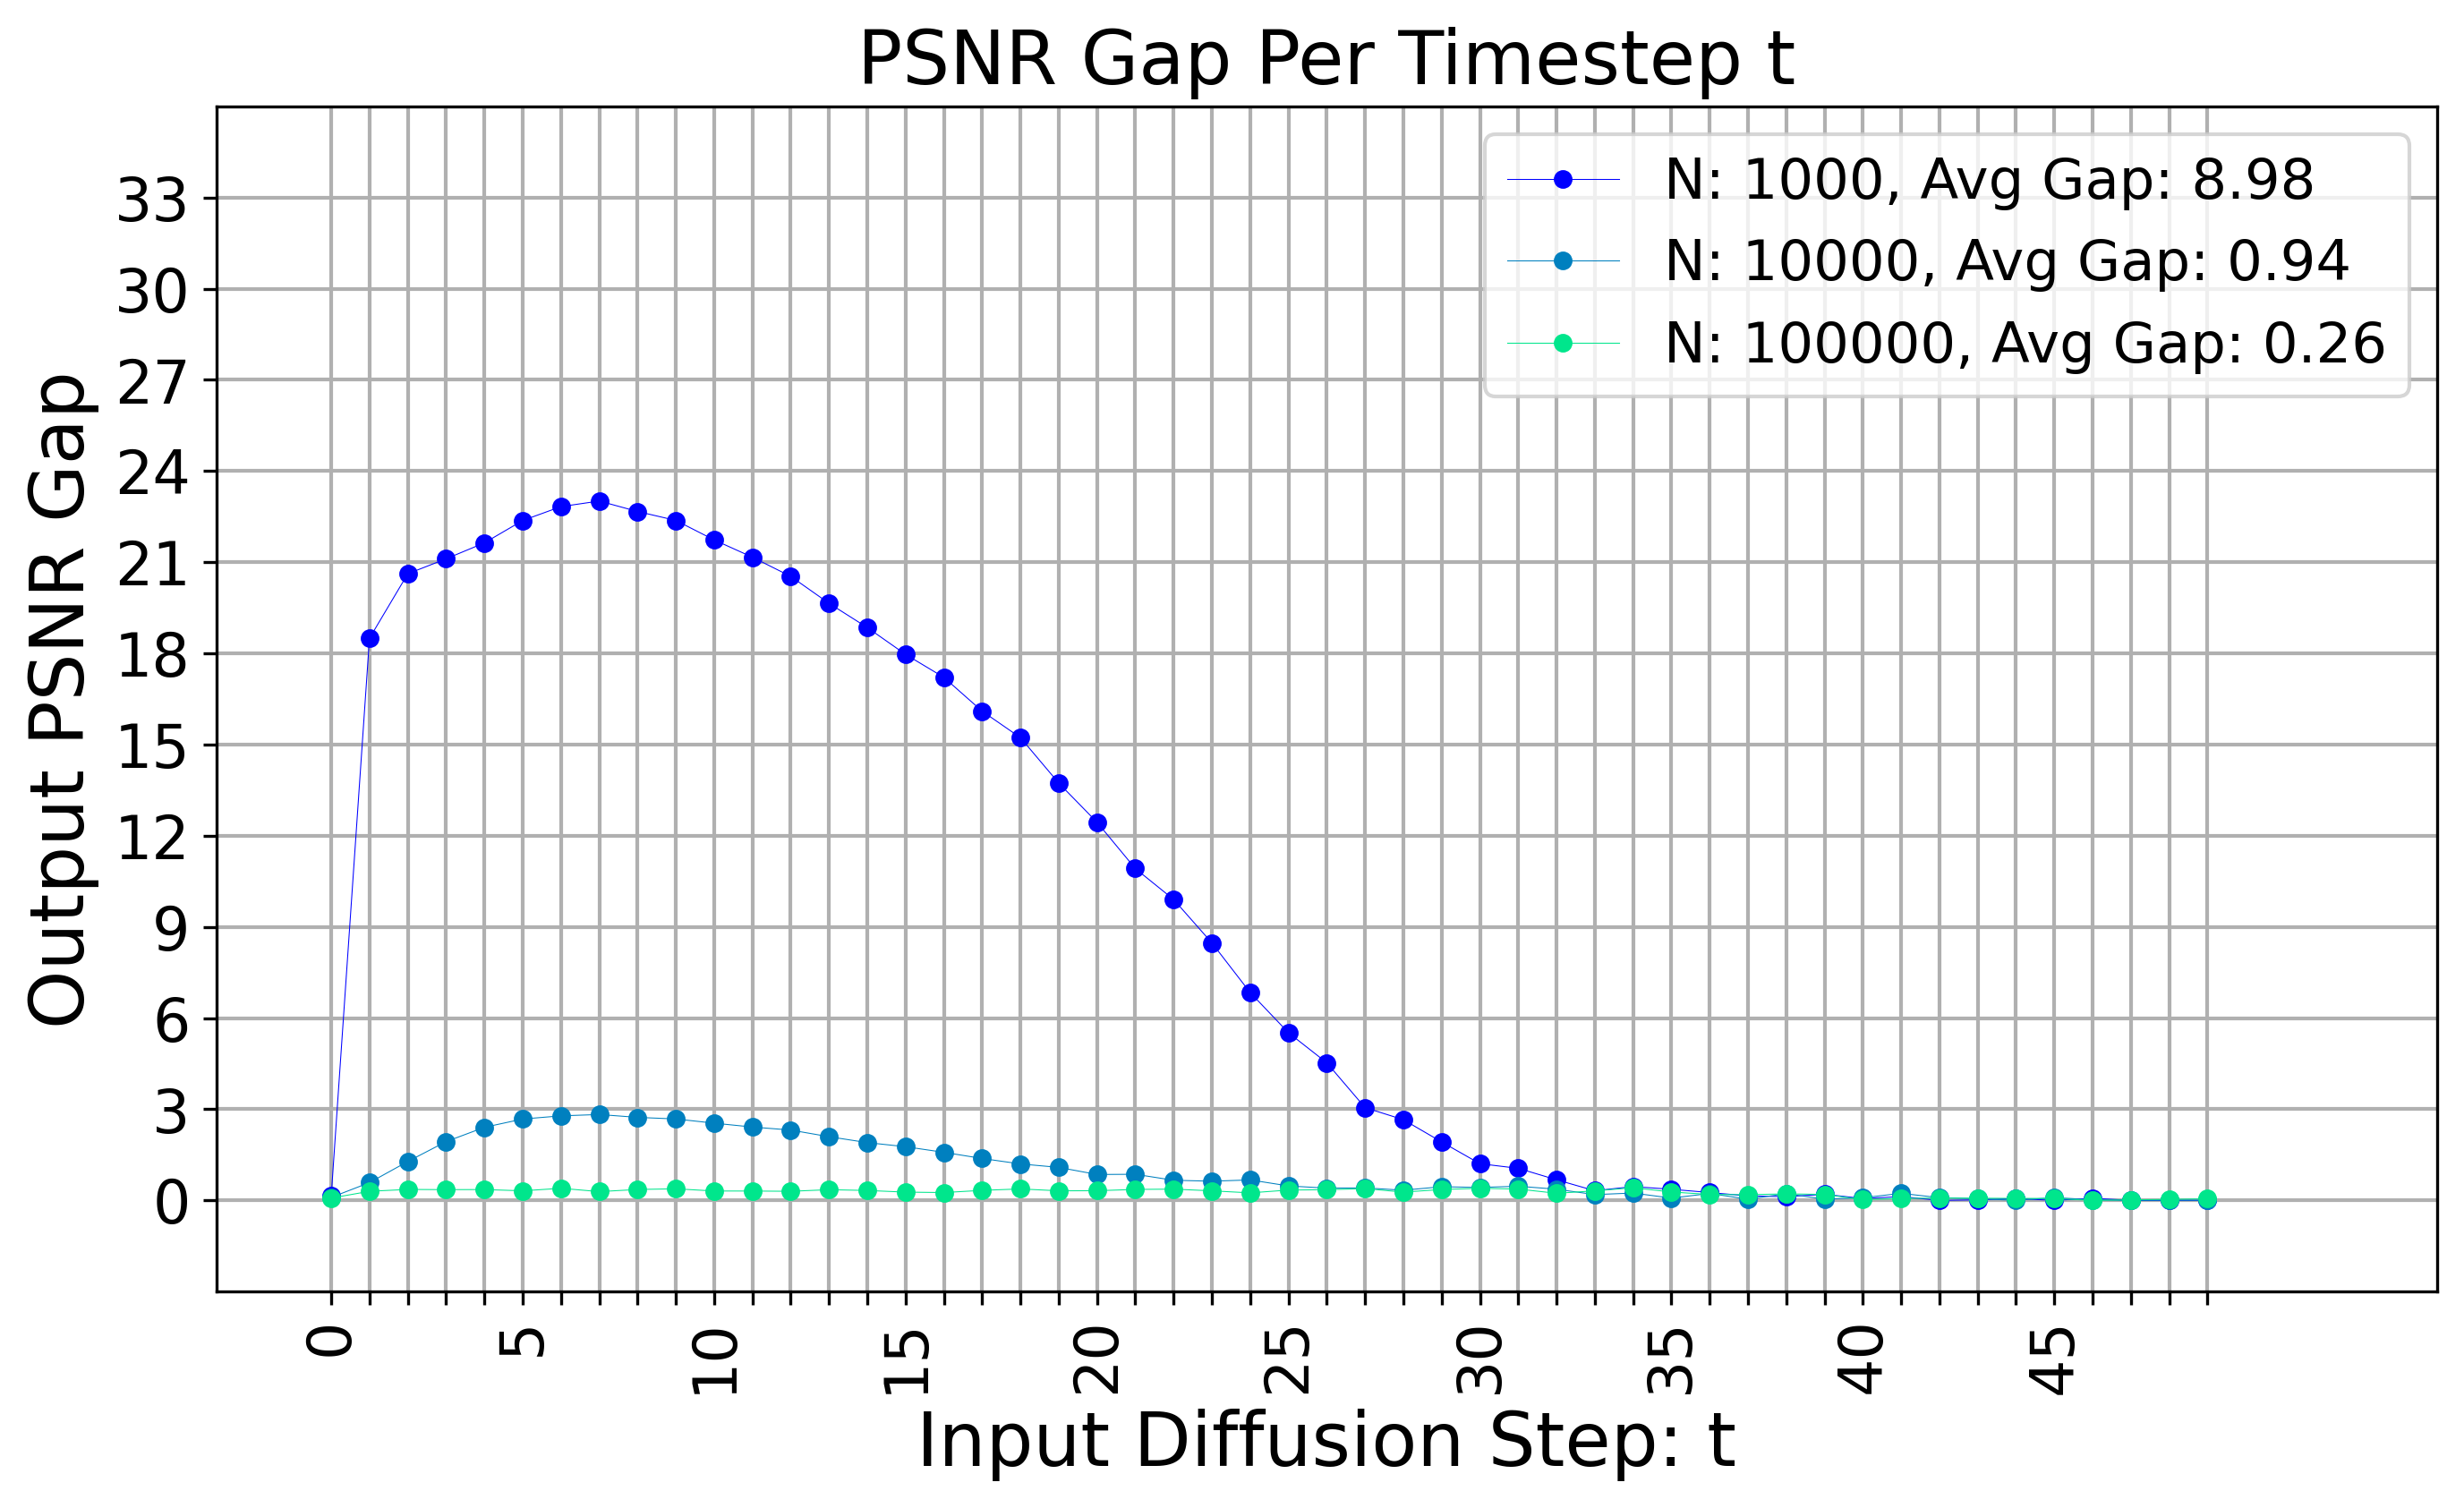}}
\\
\hline
\cellcolor{diff}{\STAB{\rotatebox[origin=c]{90}{DiT-S/1 w/ Local}}}
&
\raisebox{-0.5\height}{\includegraphics[width=.54\textwidth]{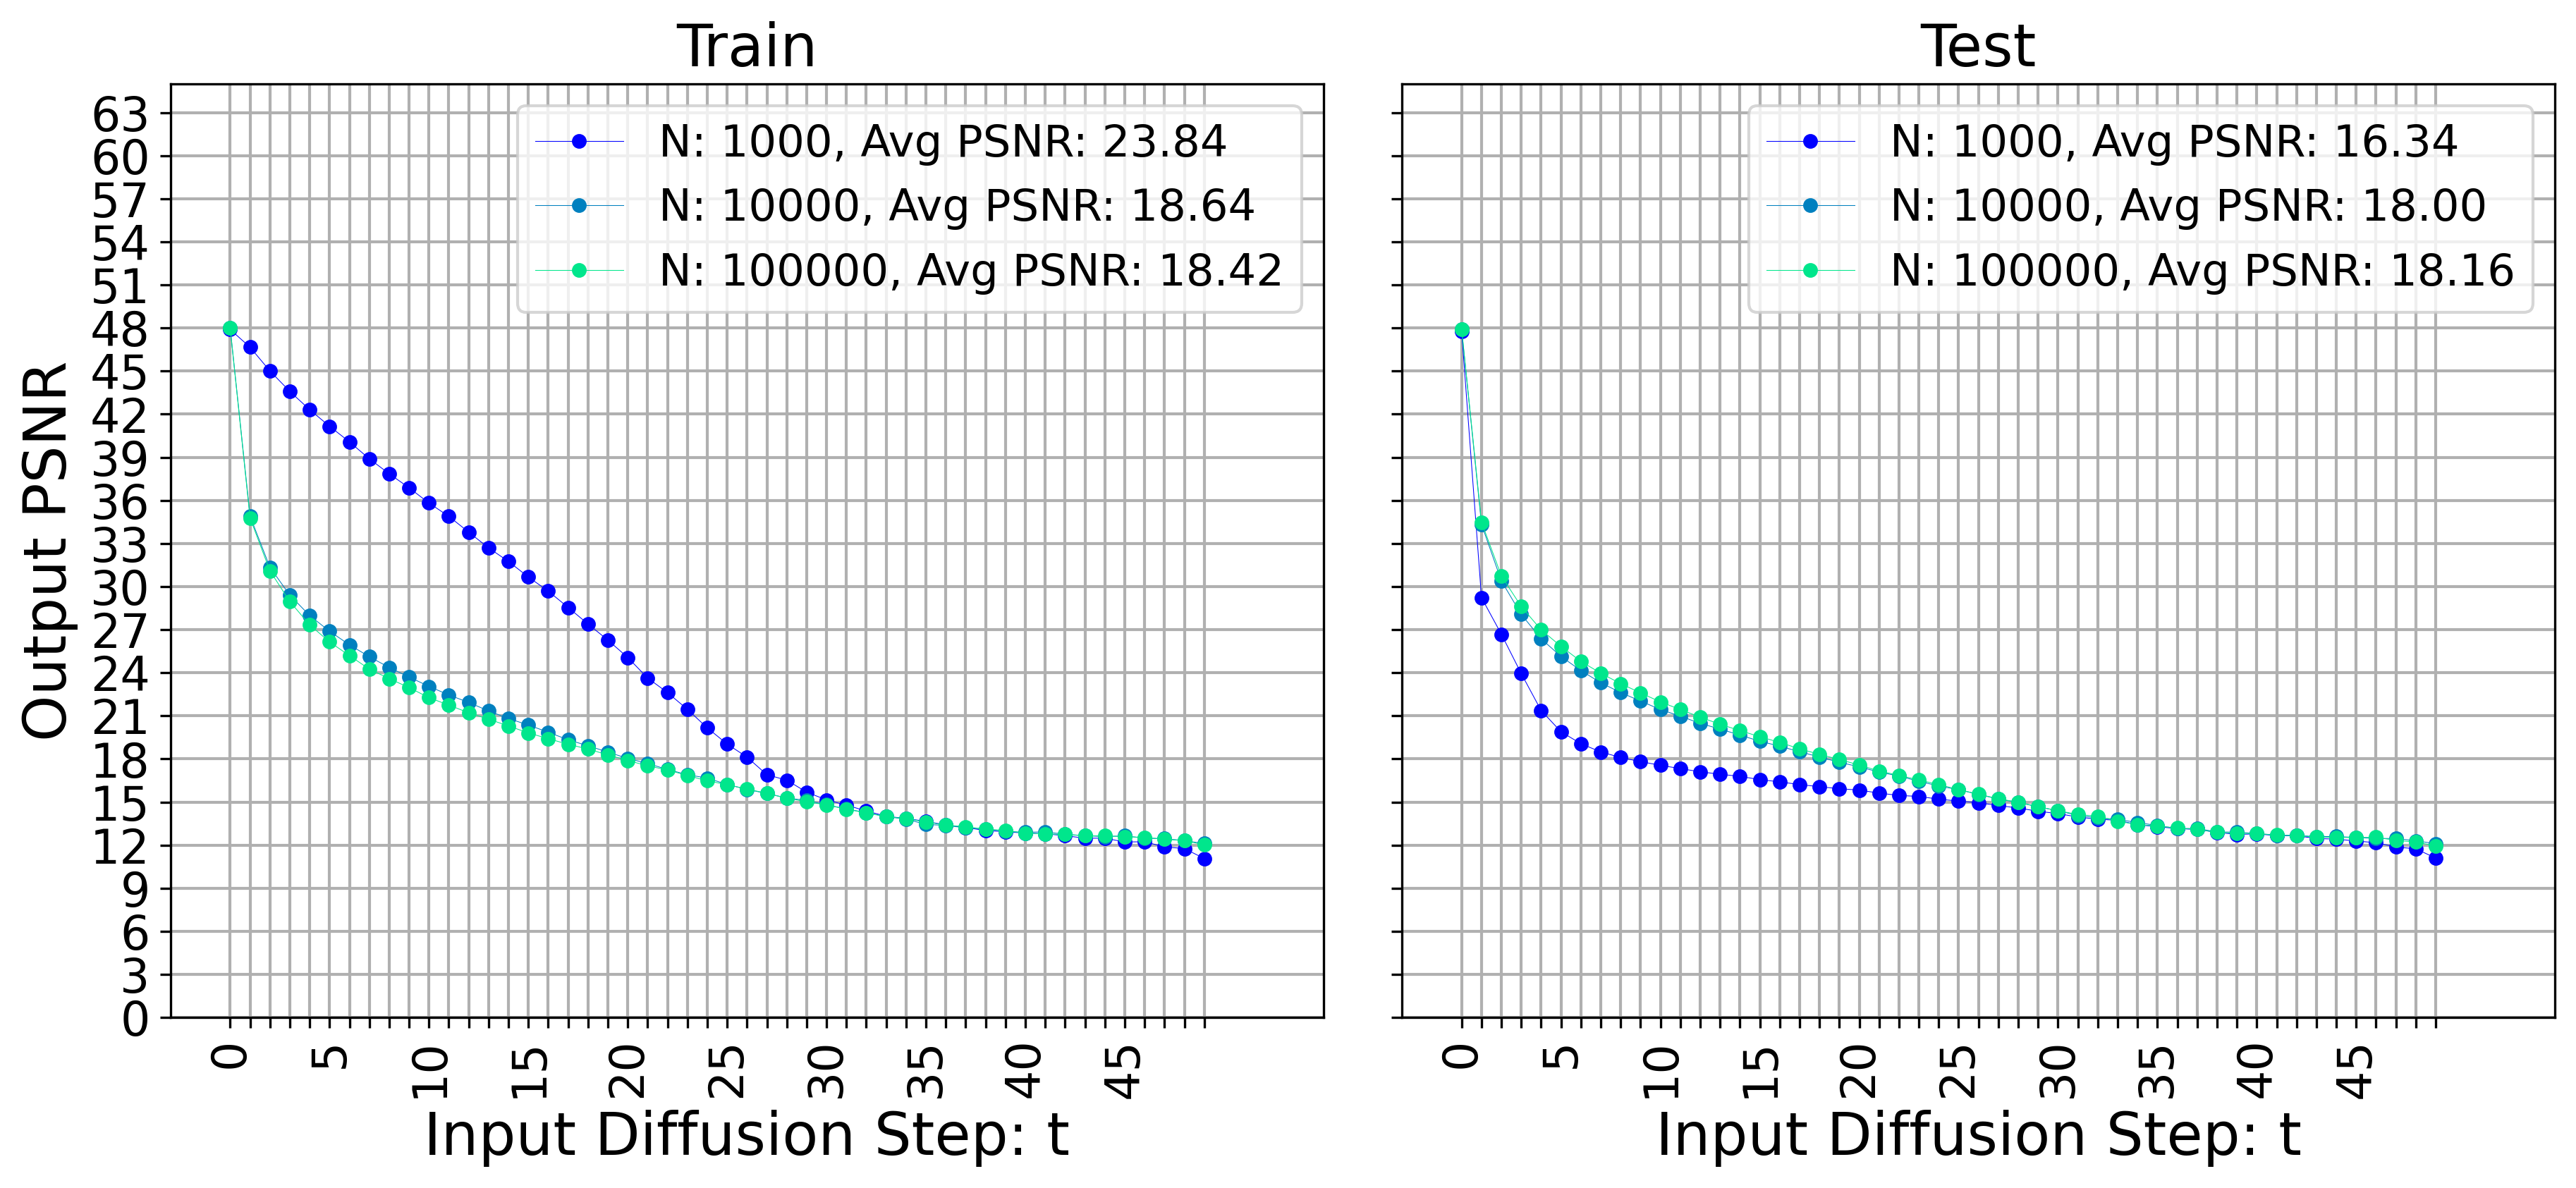}}
&
\raisebox{-0.5\height}{\includegraphics[width=.41\textwidth]{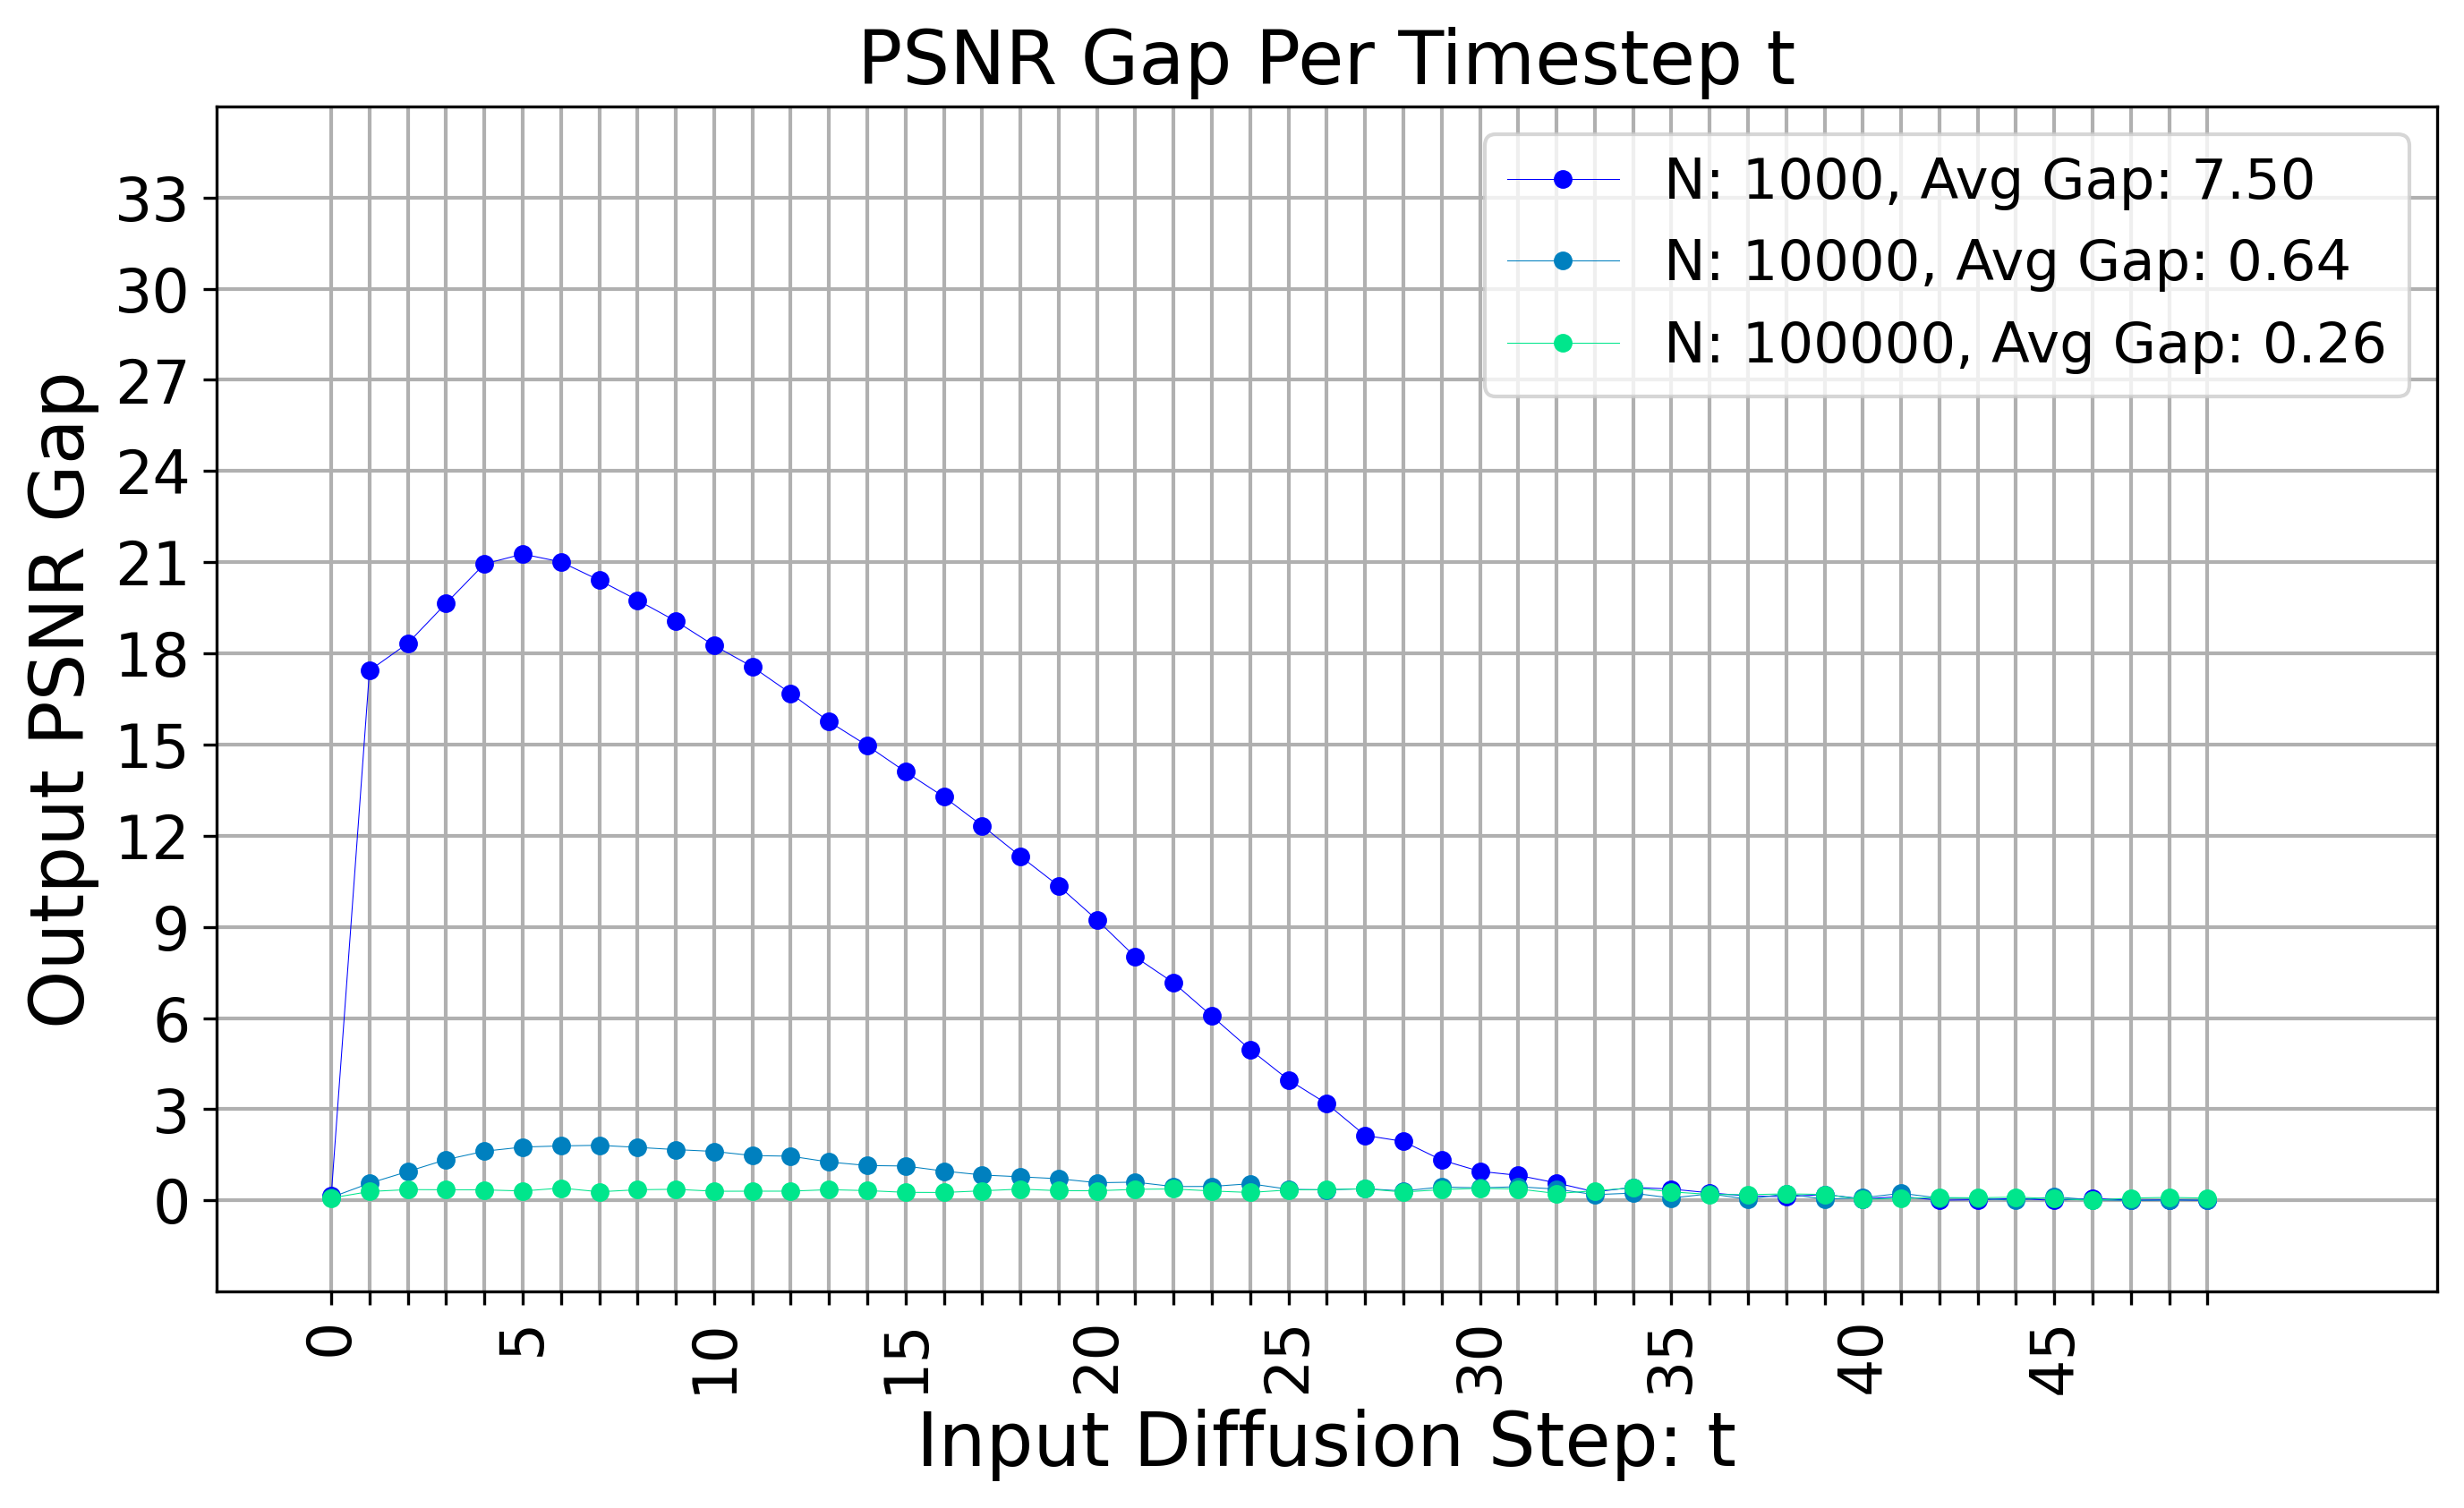}}
\\
&
\multicolumn{1}{c}{(a) PSNR Curves of Training and Testing Sets}
&
\multicolumn{1}{c}{(b) PSNR Gap}
\\
\end{tabular}

\captionof{figure}{The PSNR (a) and PSNR gap (b) comparison on the LSUN (Bedroom)~\citep{yu15lsun} dataset.}
\label{fig:row_psnr_bedroom}
\end{table}

\begin{table}[ht]
\centering
\small
\setlength\tabcolsep{1pt}
\setlength{\extrarowheight}{4pt}
\begin{tabular}{lc|c}
\cellcolor{dit}{\STAB{\rotatebox[origin=c]{90}{DiT-XS/1}}}
&
\raisebox{-0.5\height}{\includegraphics[width=.54\textwidth]{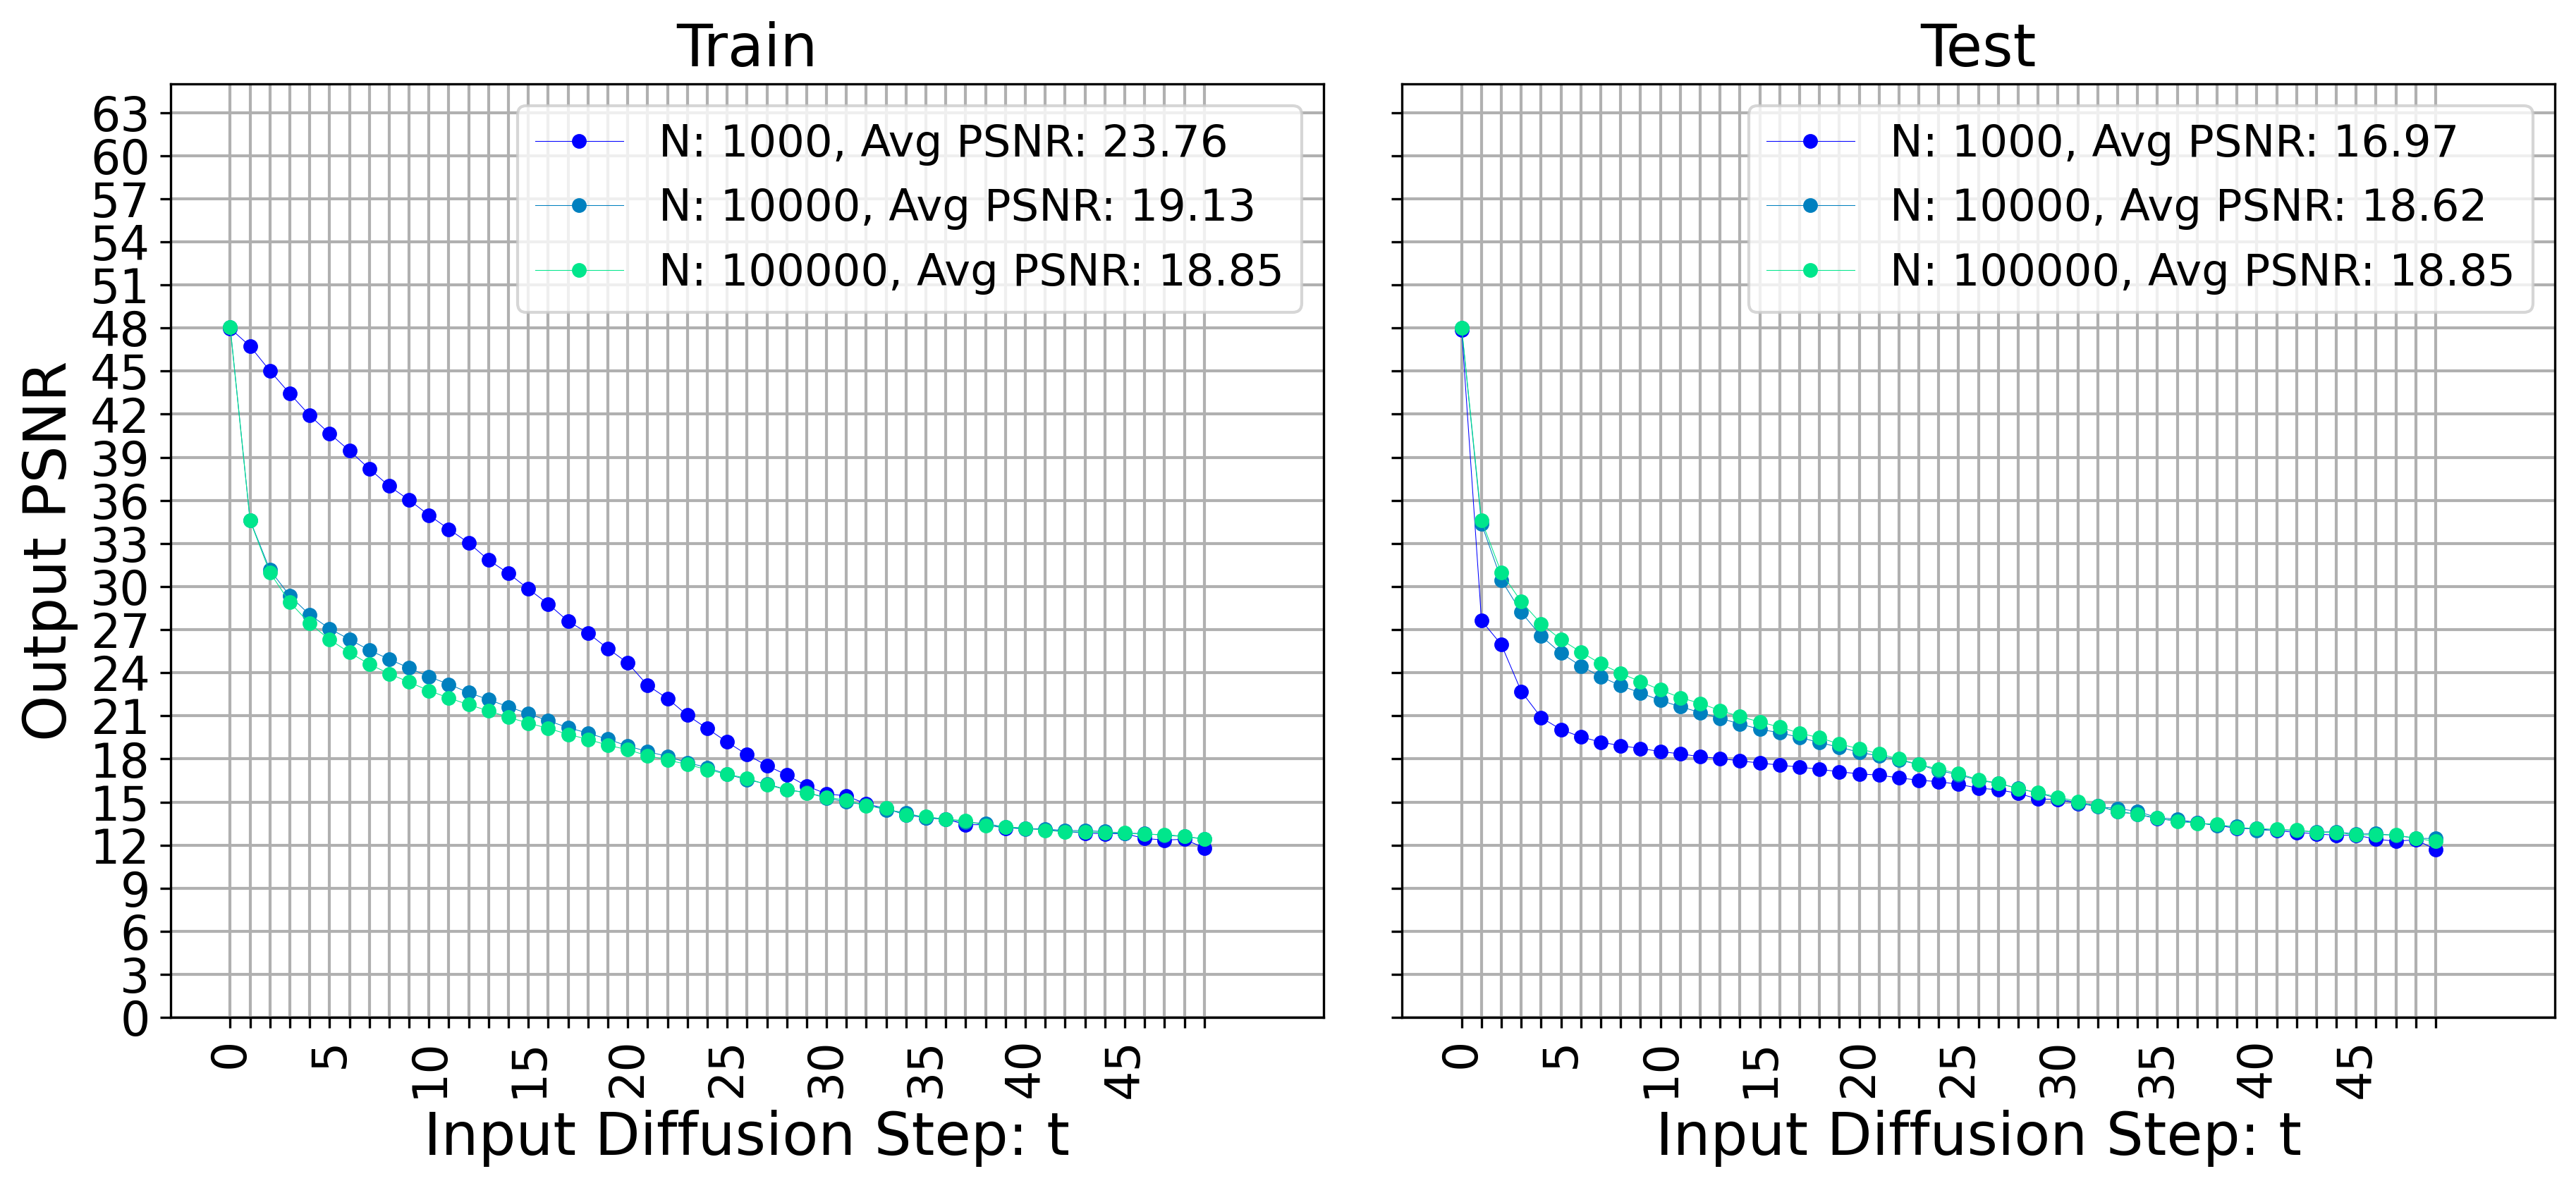}}
&
\raisebox{-0.5\height}{\includegraphics[width=.41\textwidth]{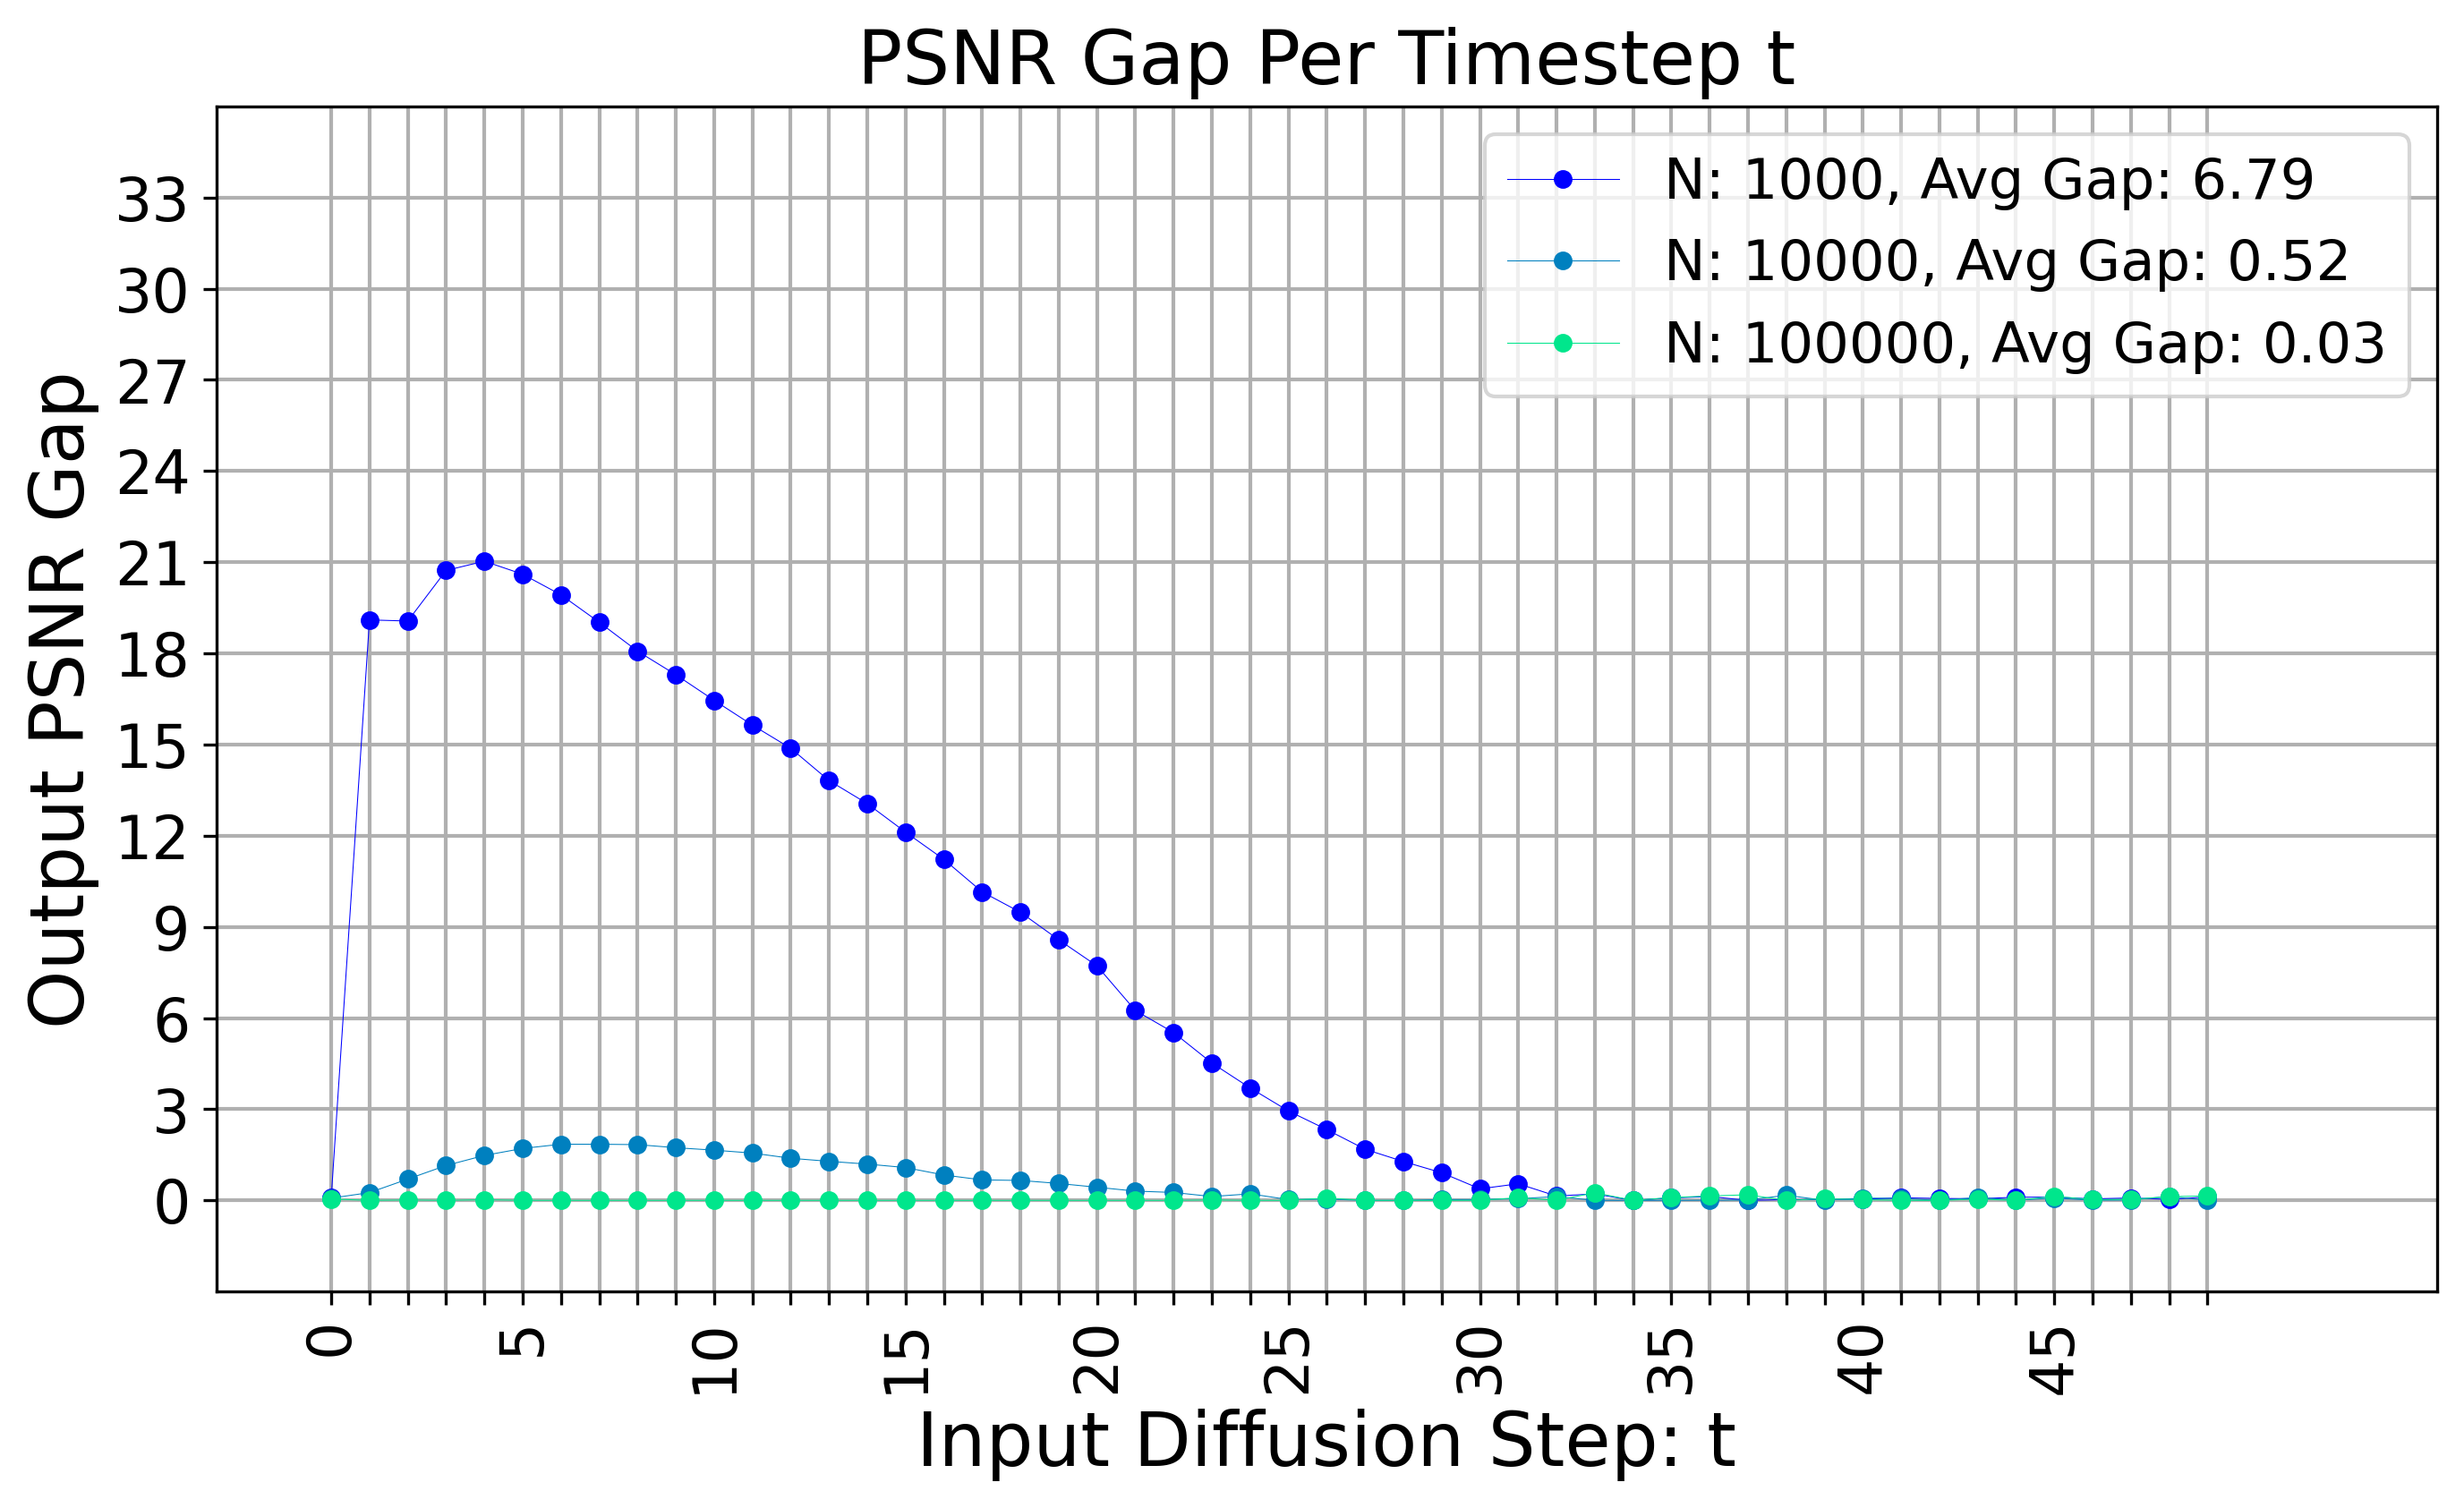}}
\\
\hline
\cellcolor{diff}{\STAB{\rotatebox[origin=c]{90}{DiT-XS/1 w/ Local}}}
&
\raisebox{-0.5\height}{\includegraphics[width=.54\textwidth]{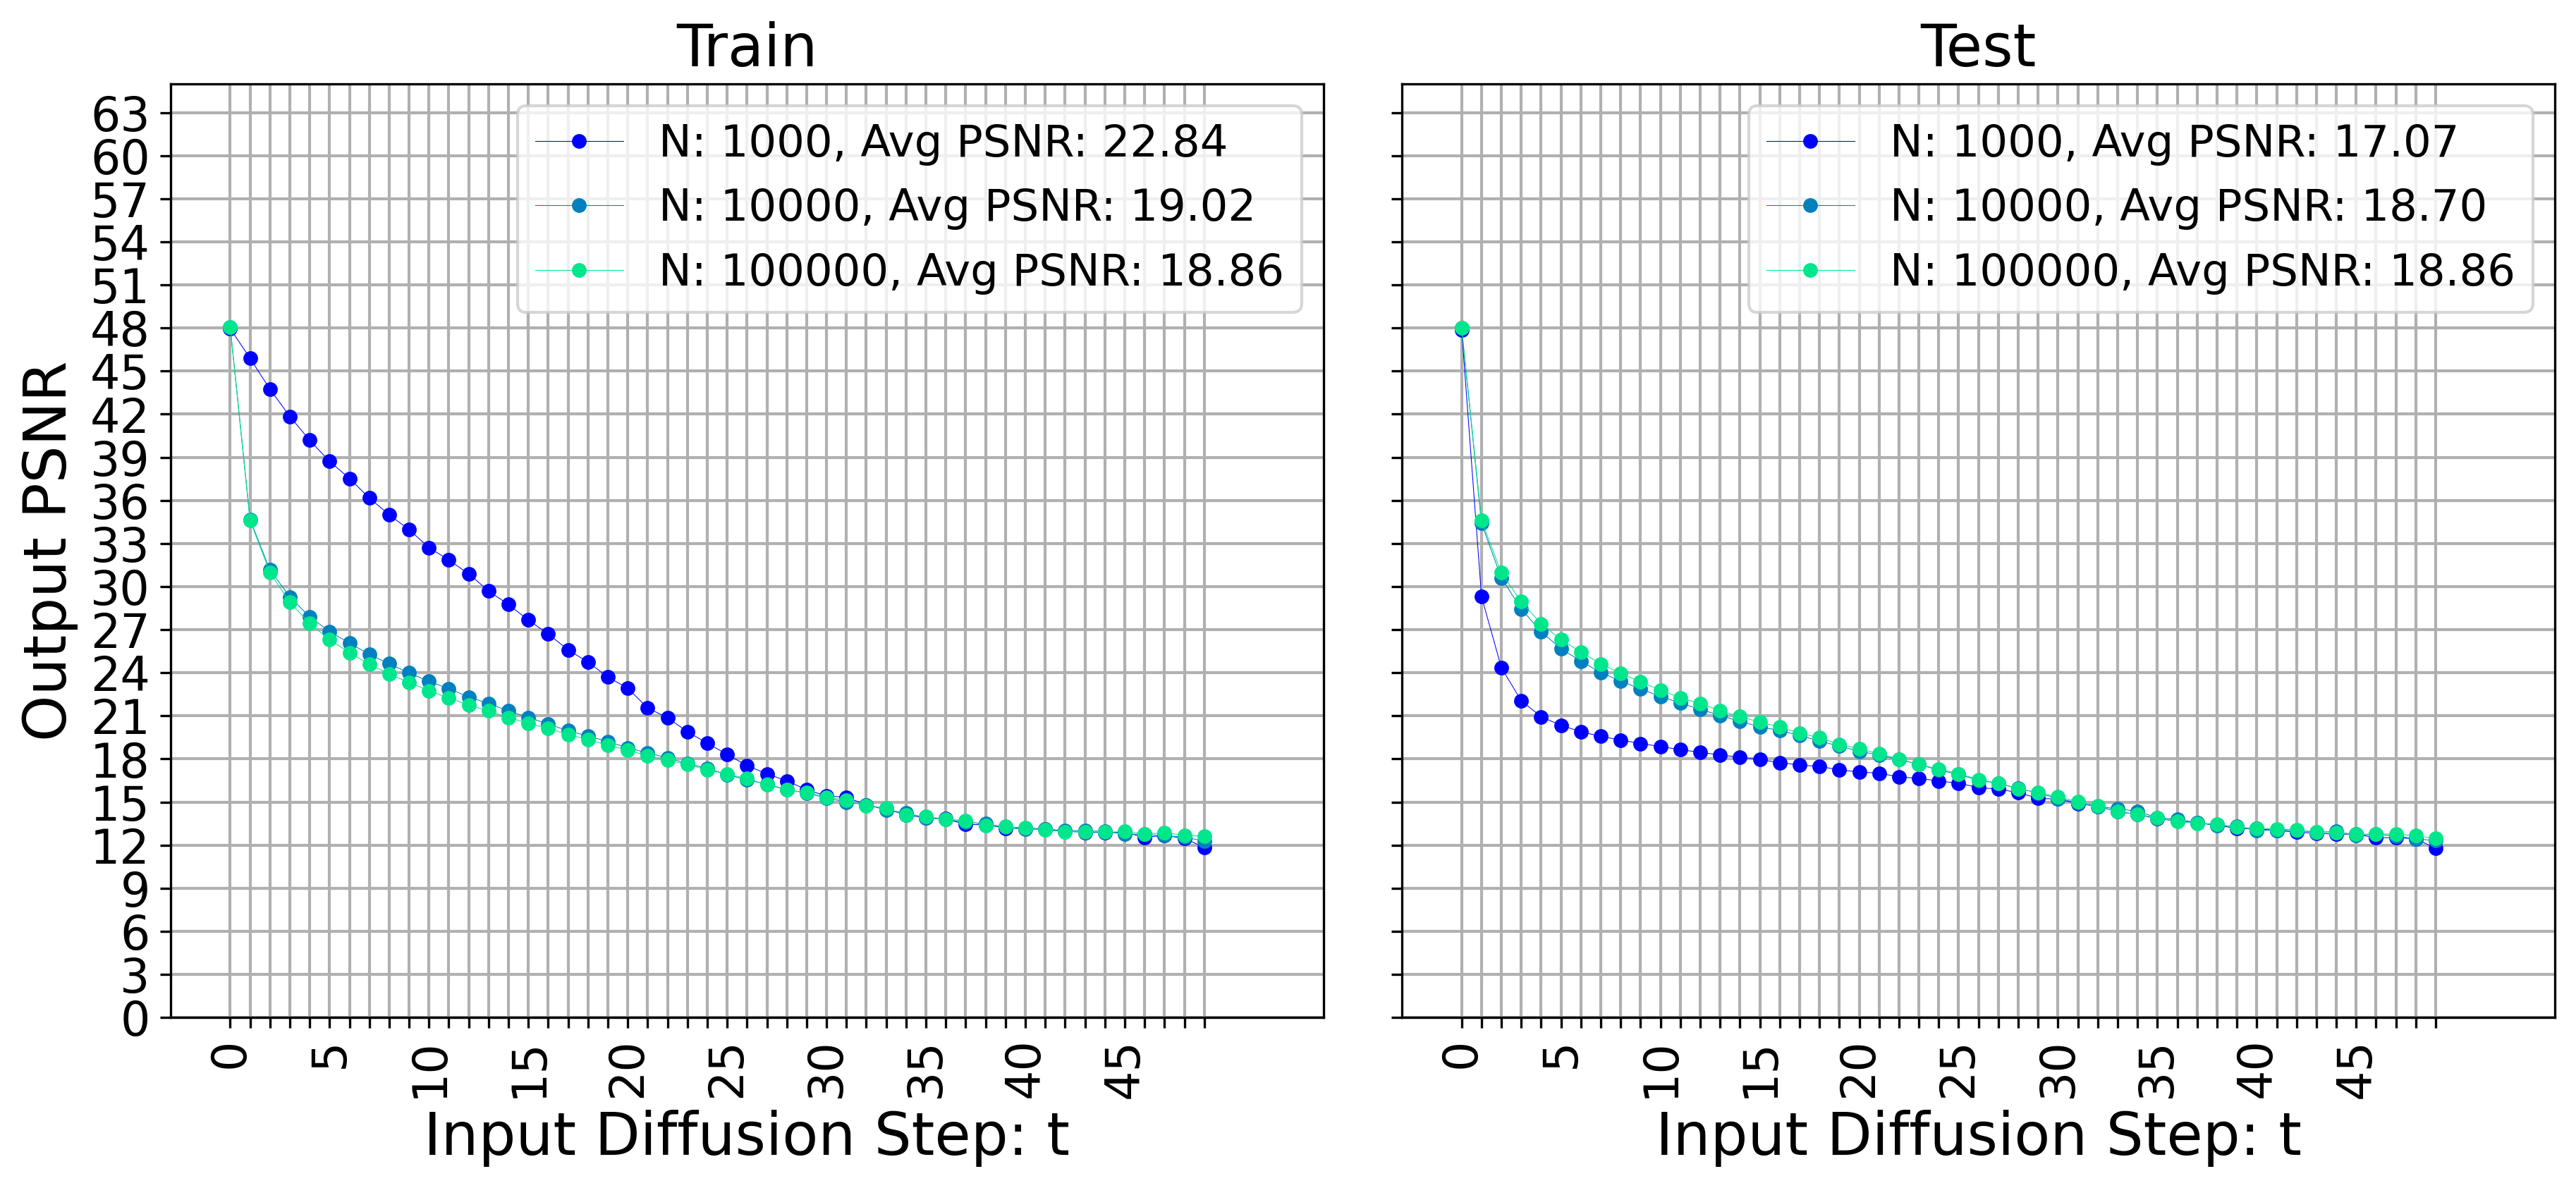}}
&
\raisebox{-0.5\height}{\includegraphics[width=.41\textwidth]{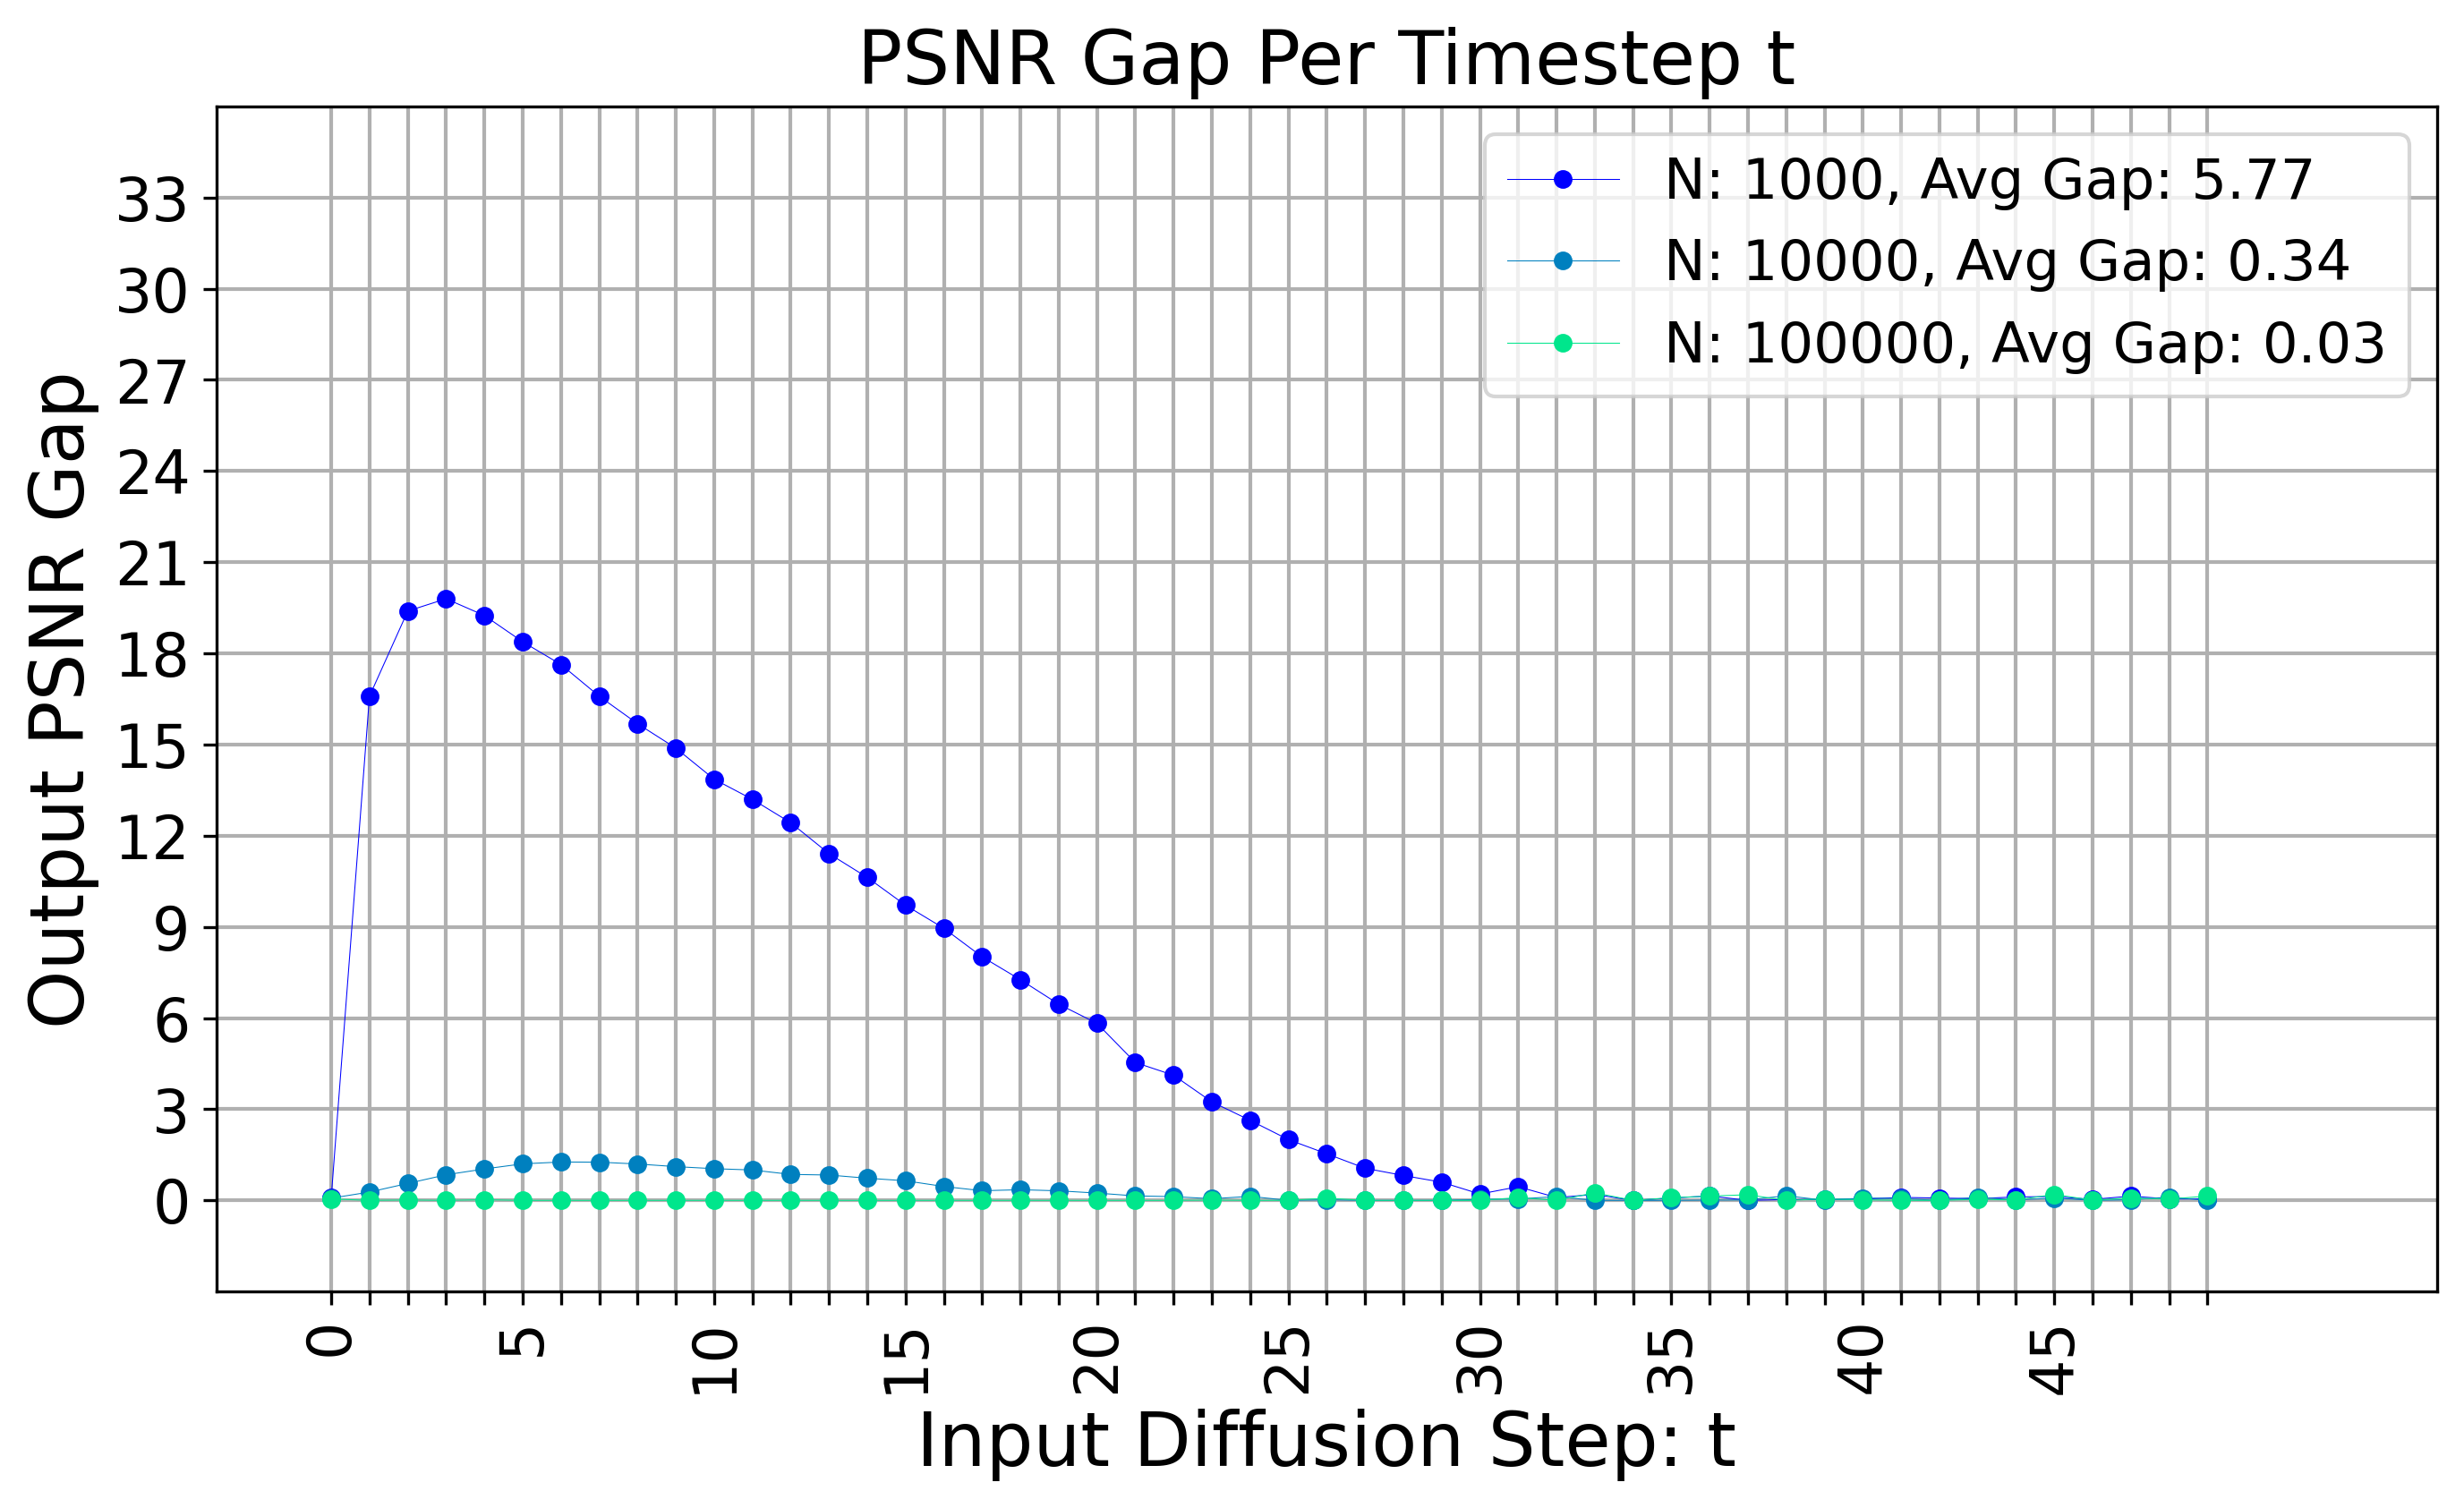}}
\\
\hline
\cellcolor{dit}{\STAB{\rotatebox[origin=c]{90}{DiT-S/1}}}
&
\raisebox{-0.5\height}{\includegraphics[width=.54\textwidth]{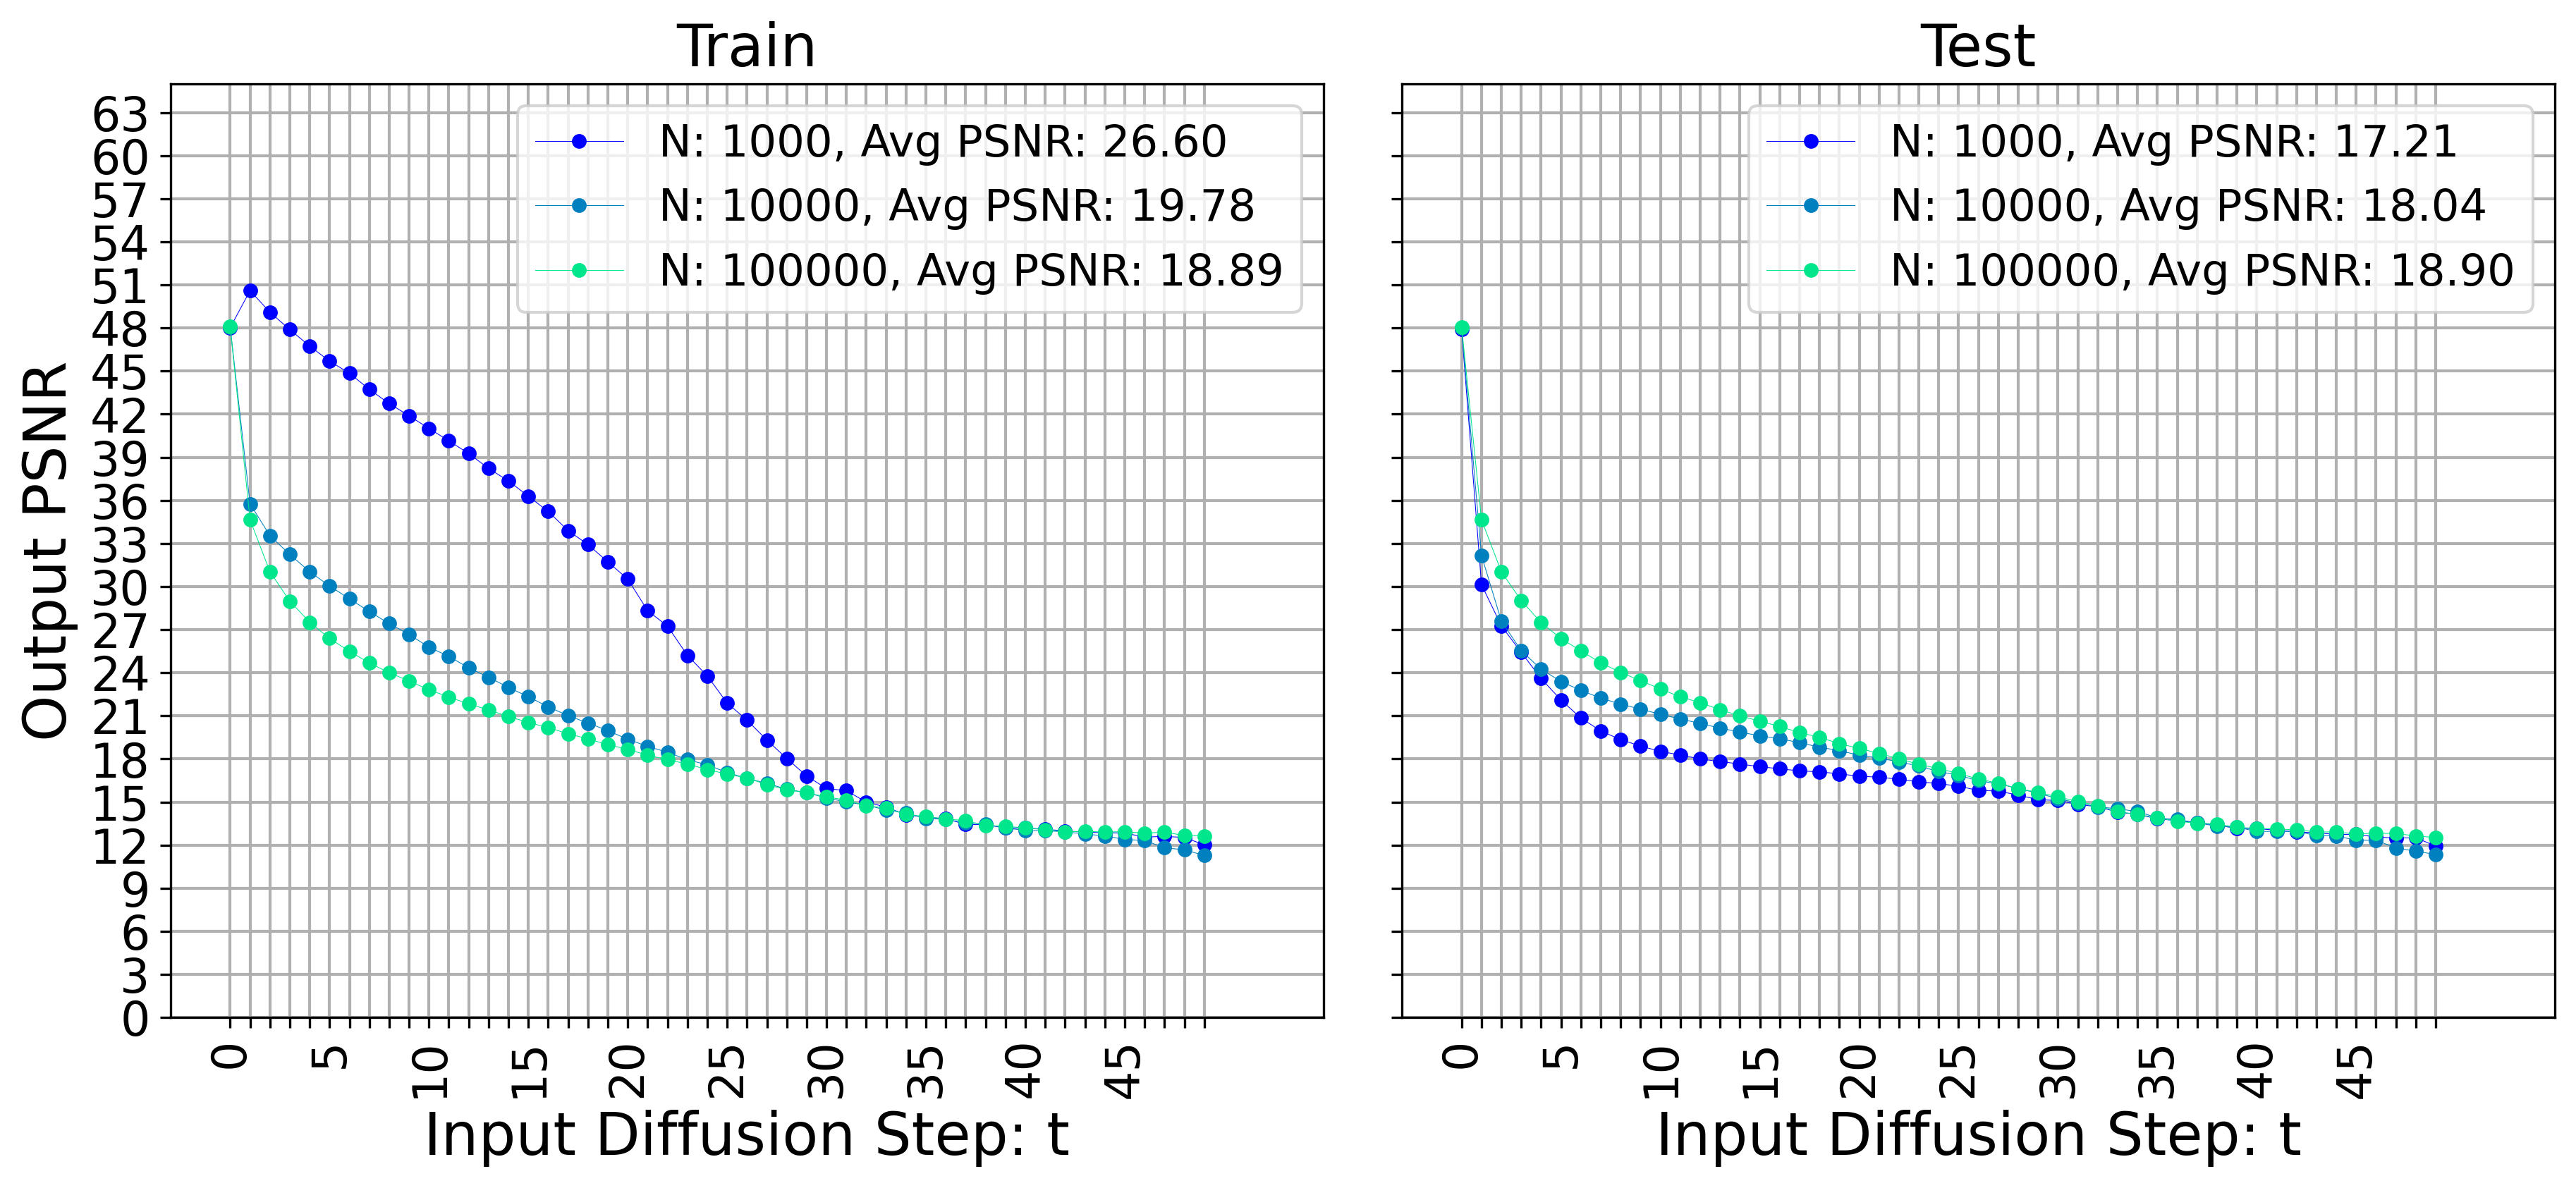}}
&
\raisebox{-0.5\height}{\includegraphics[width=.41\textwidth]{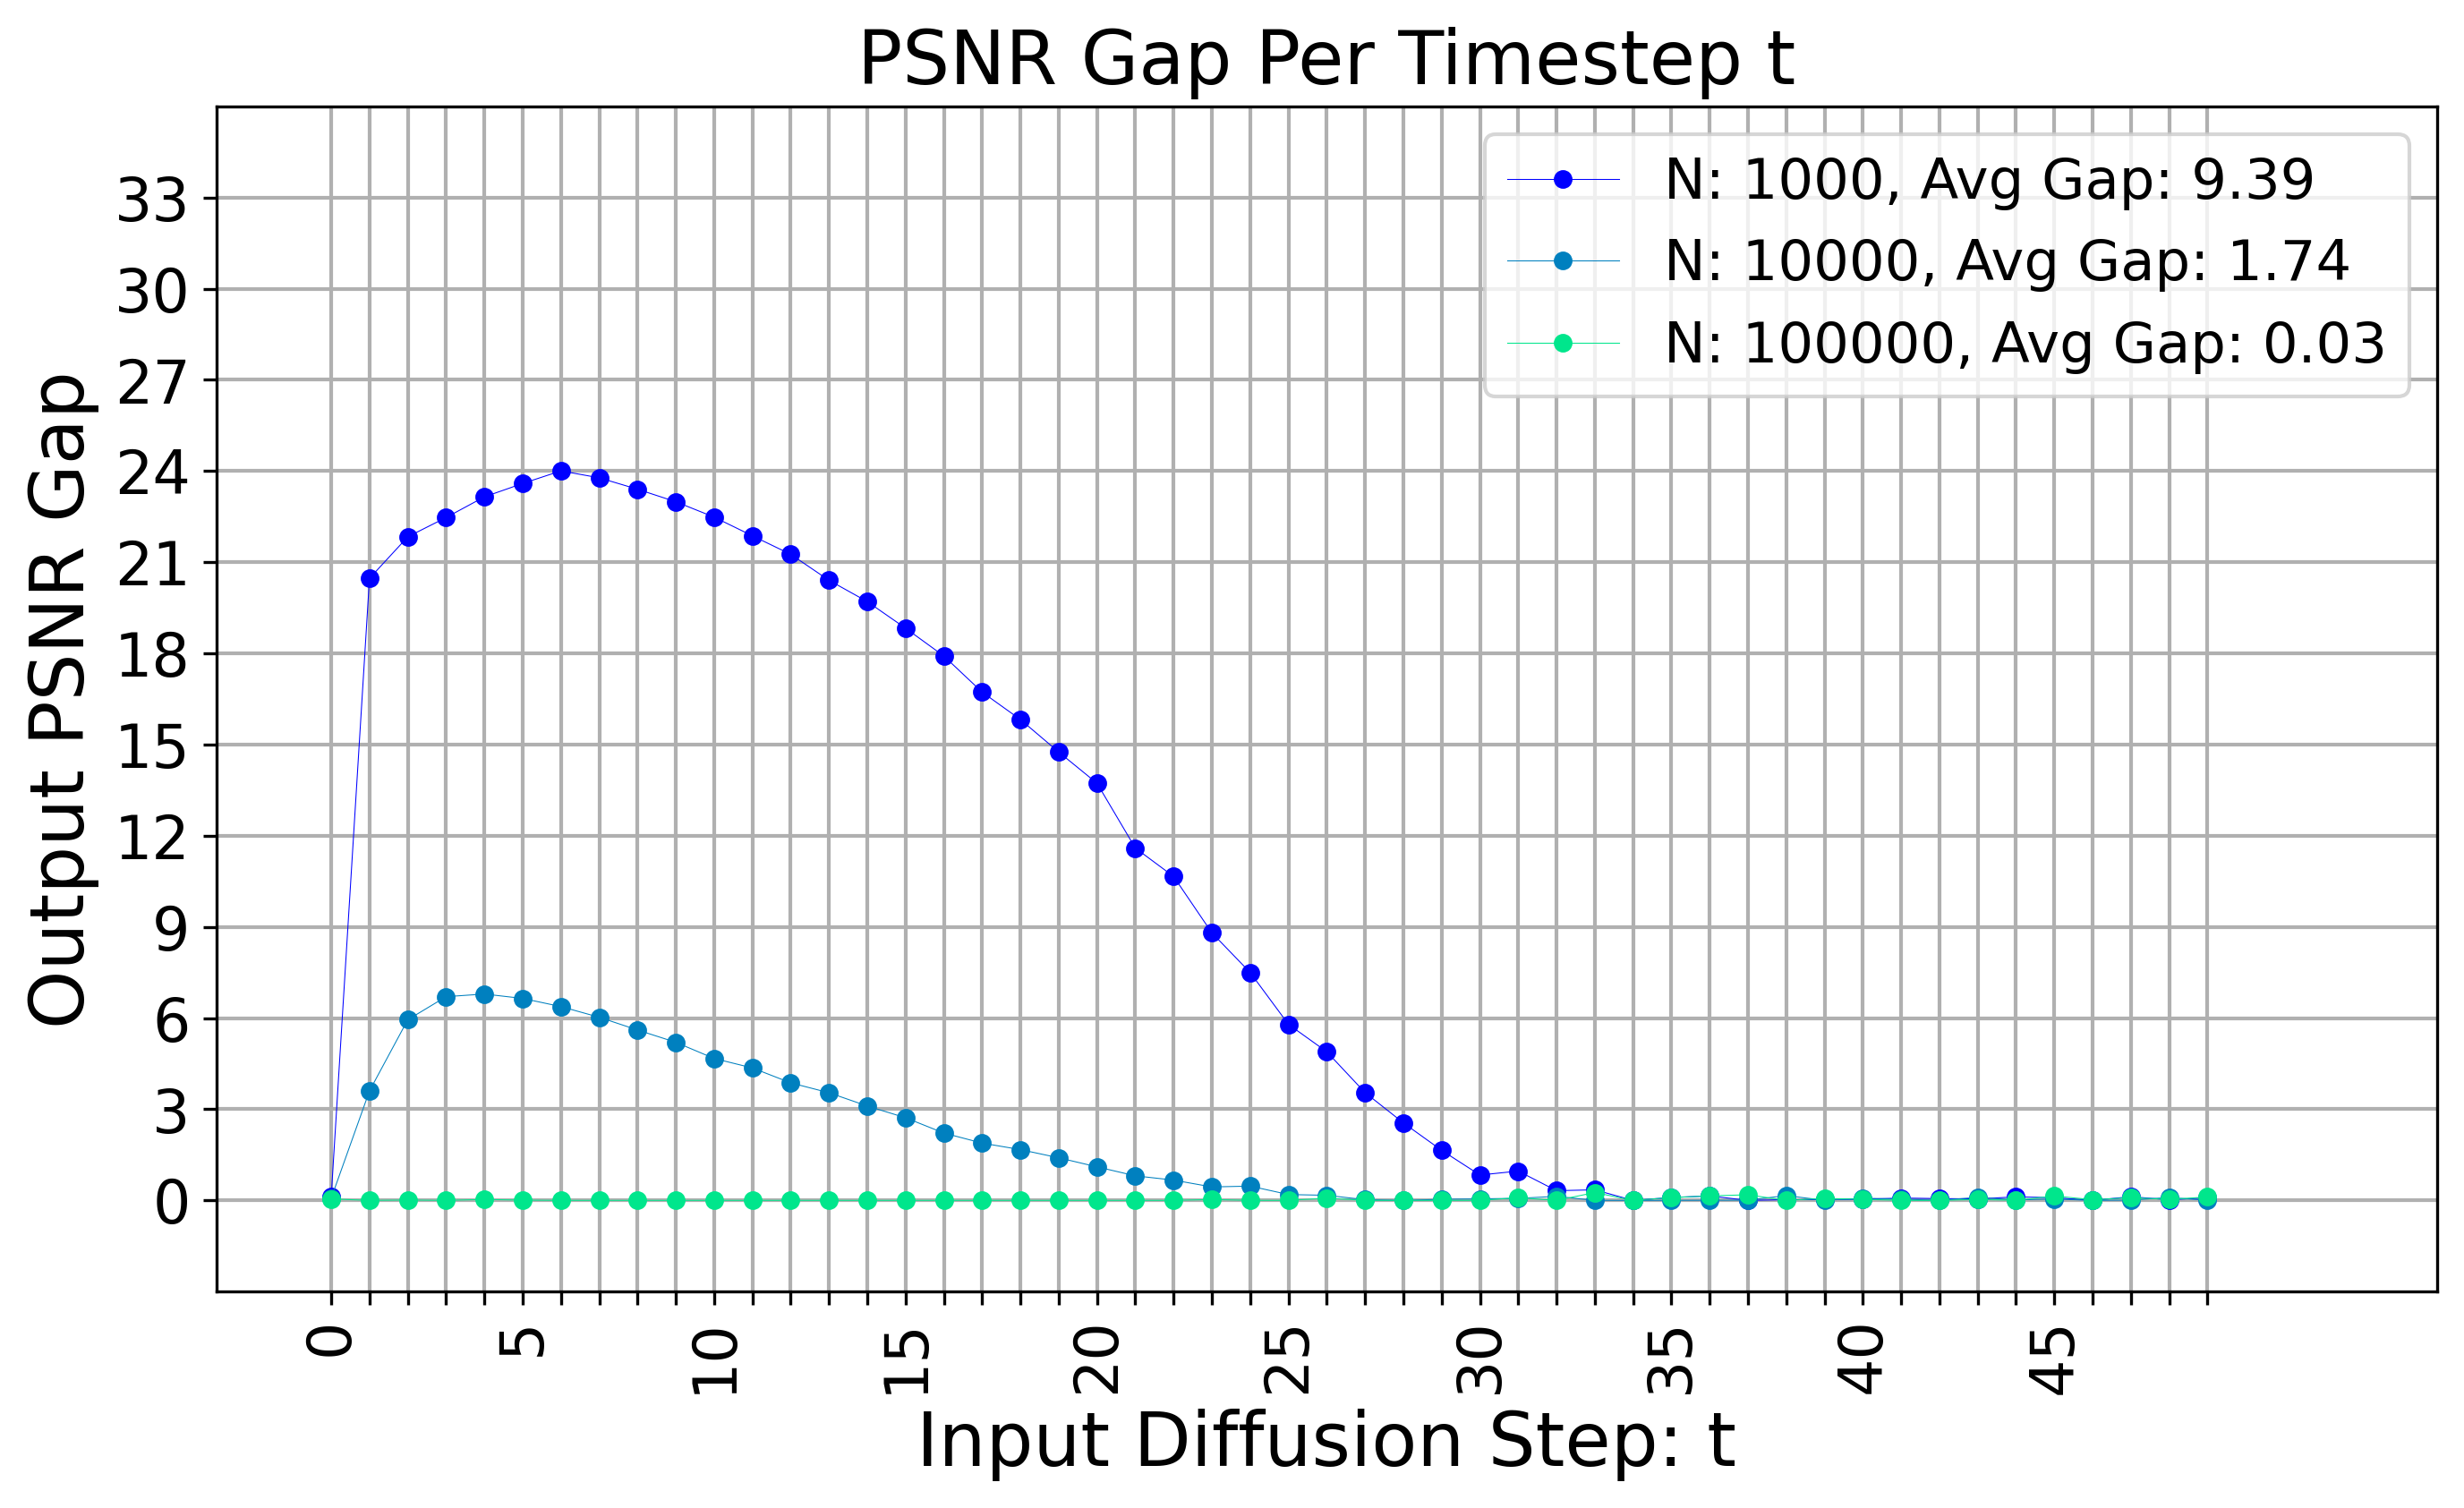}}
\\
\hline
\cellcolor{diff}{\STAB{\rotatebox[origin=c]{90}{DiT-S/1 w/ Local}}}
&
\raisebox{-0.5\height}{\includegraphics[width=.54\textwidth]{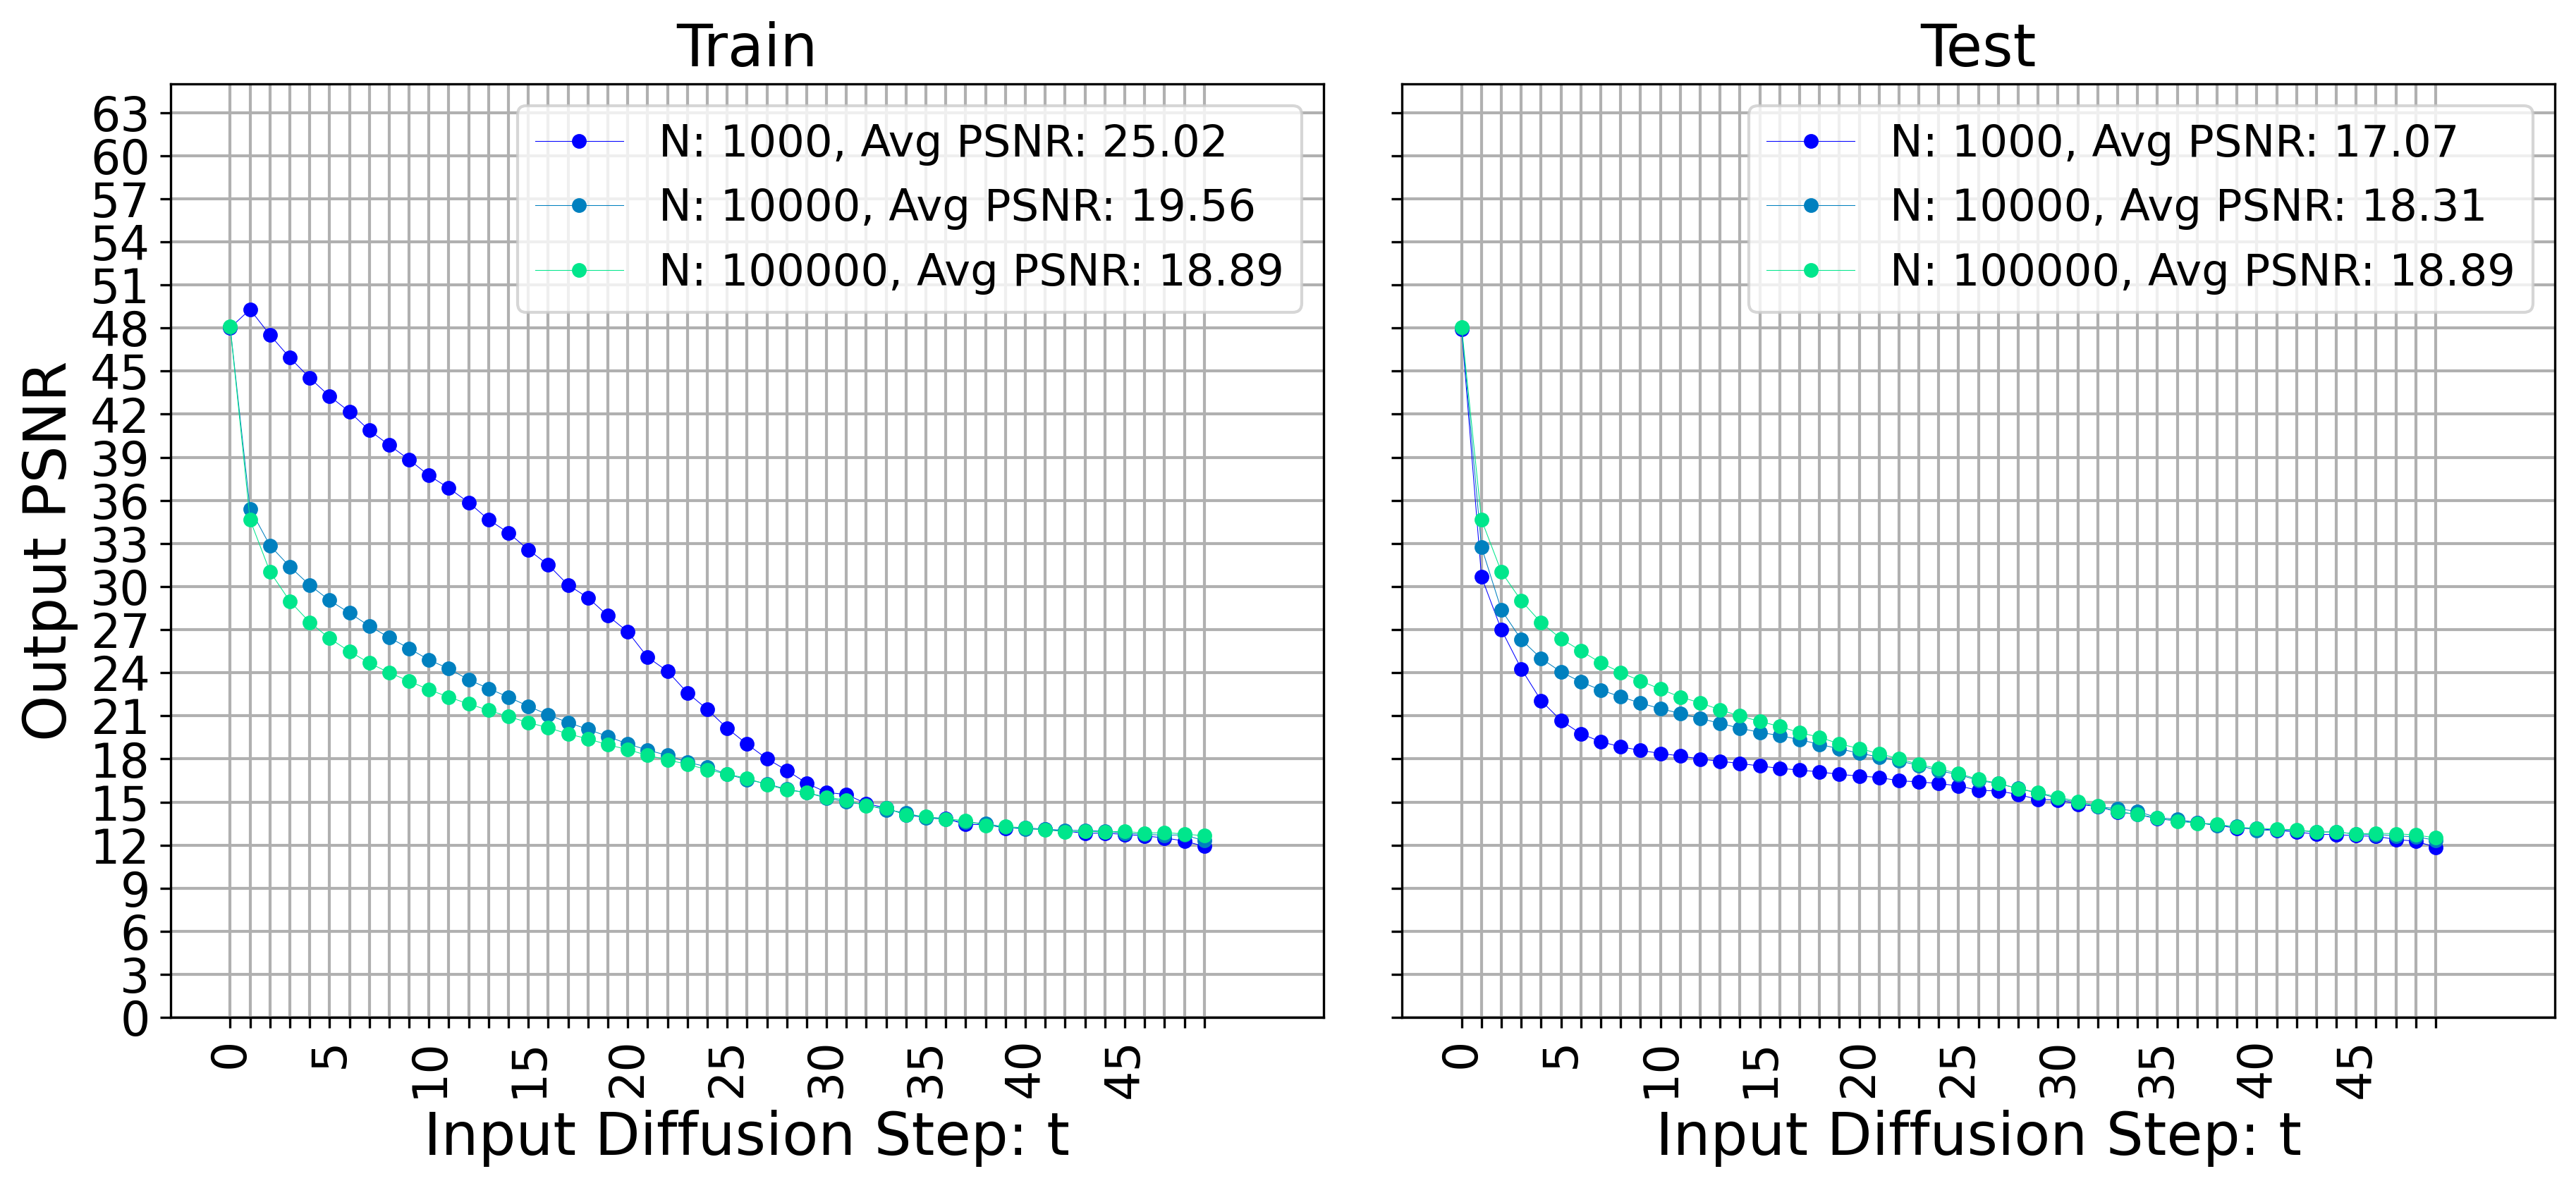}}
&
\raisebox{-0.5\height}{\includegraphics[width=.41\textwidth]{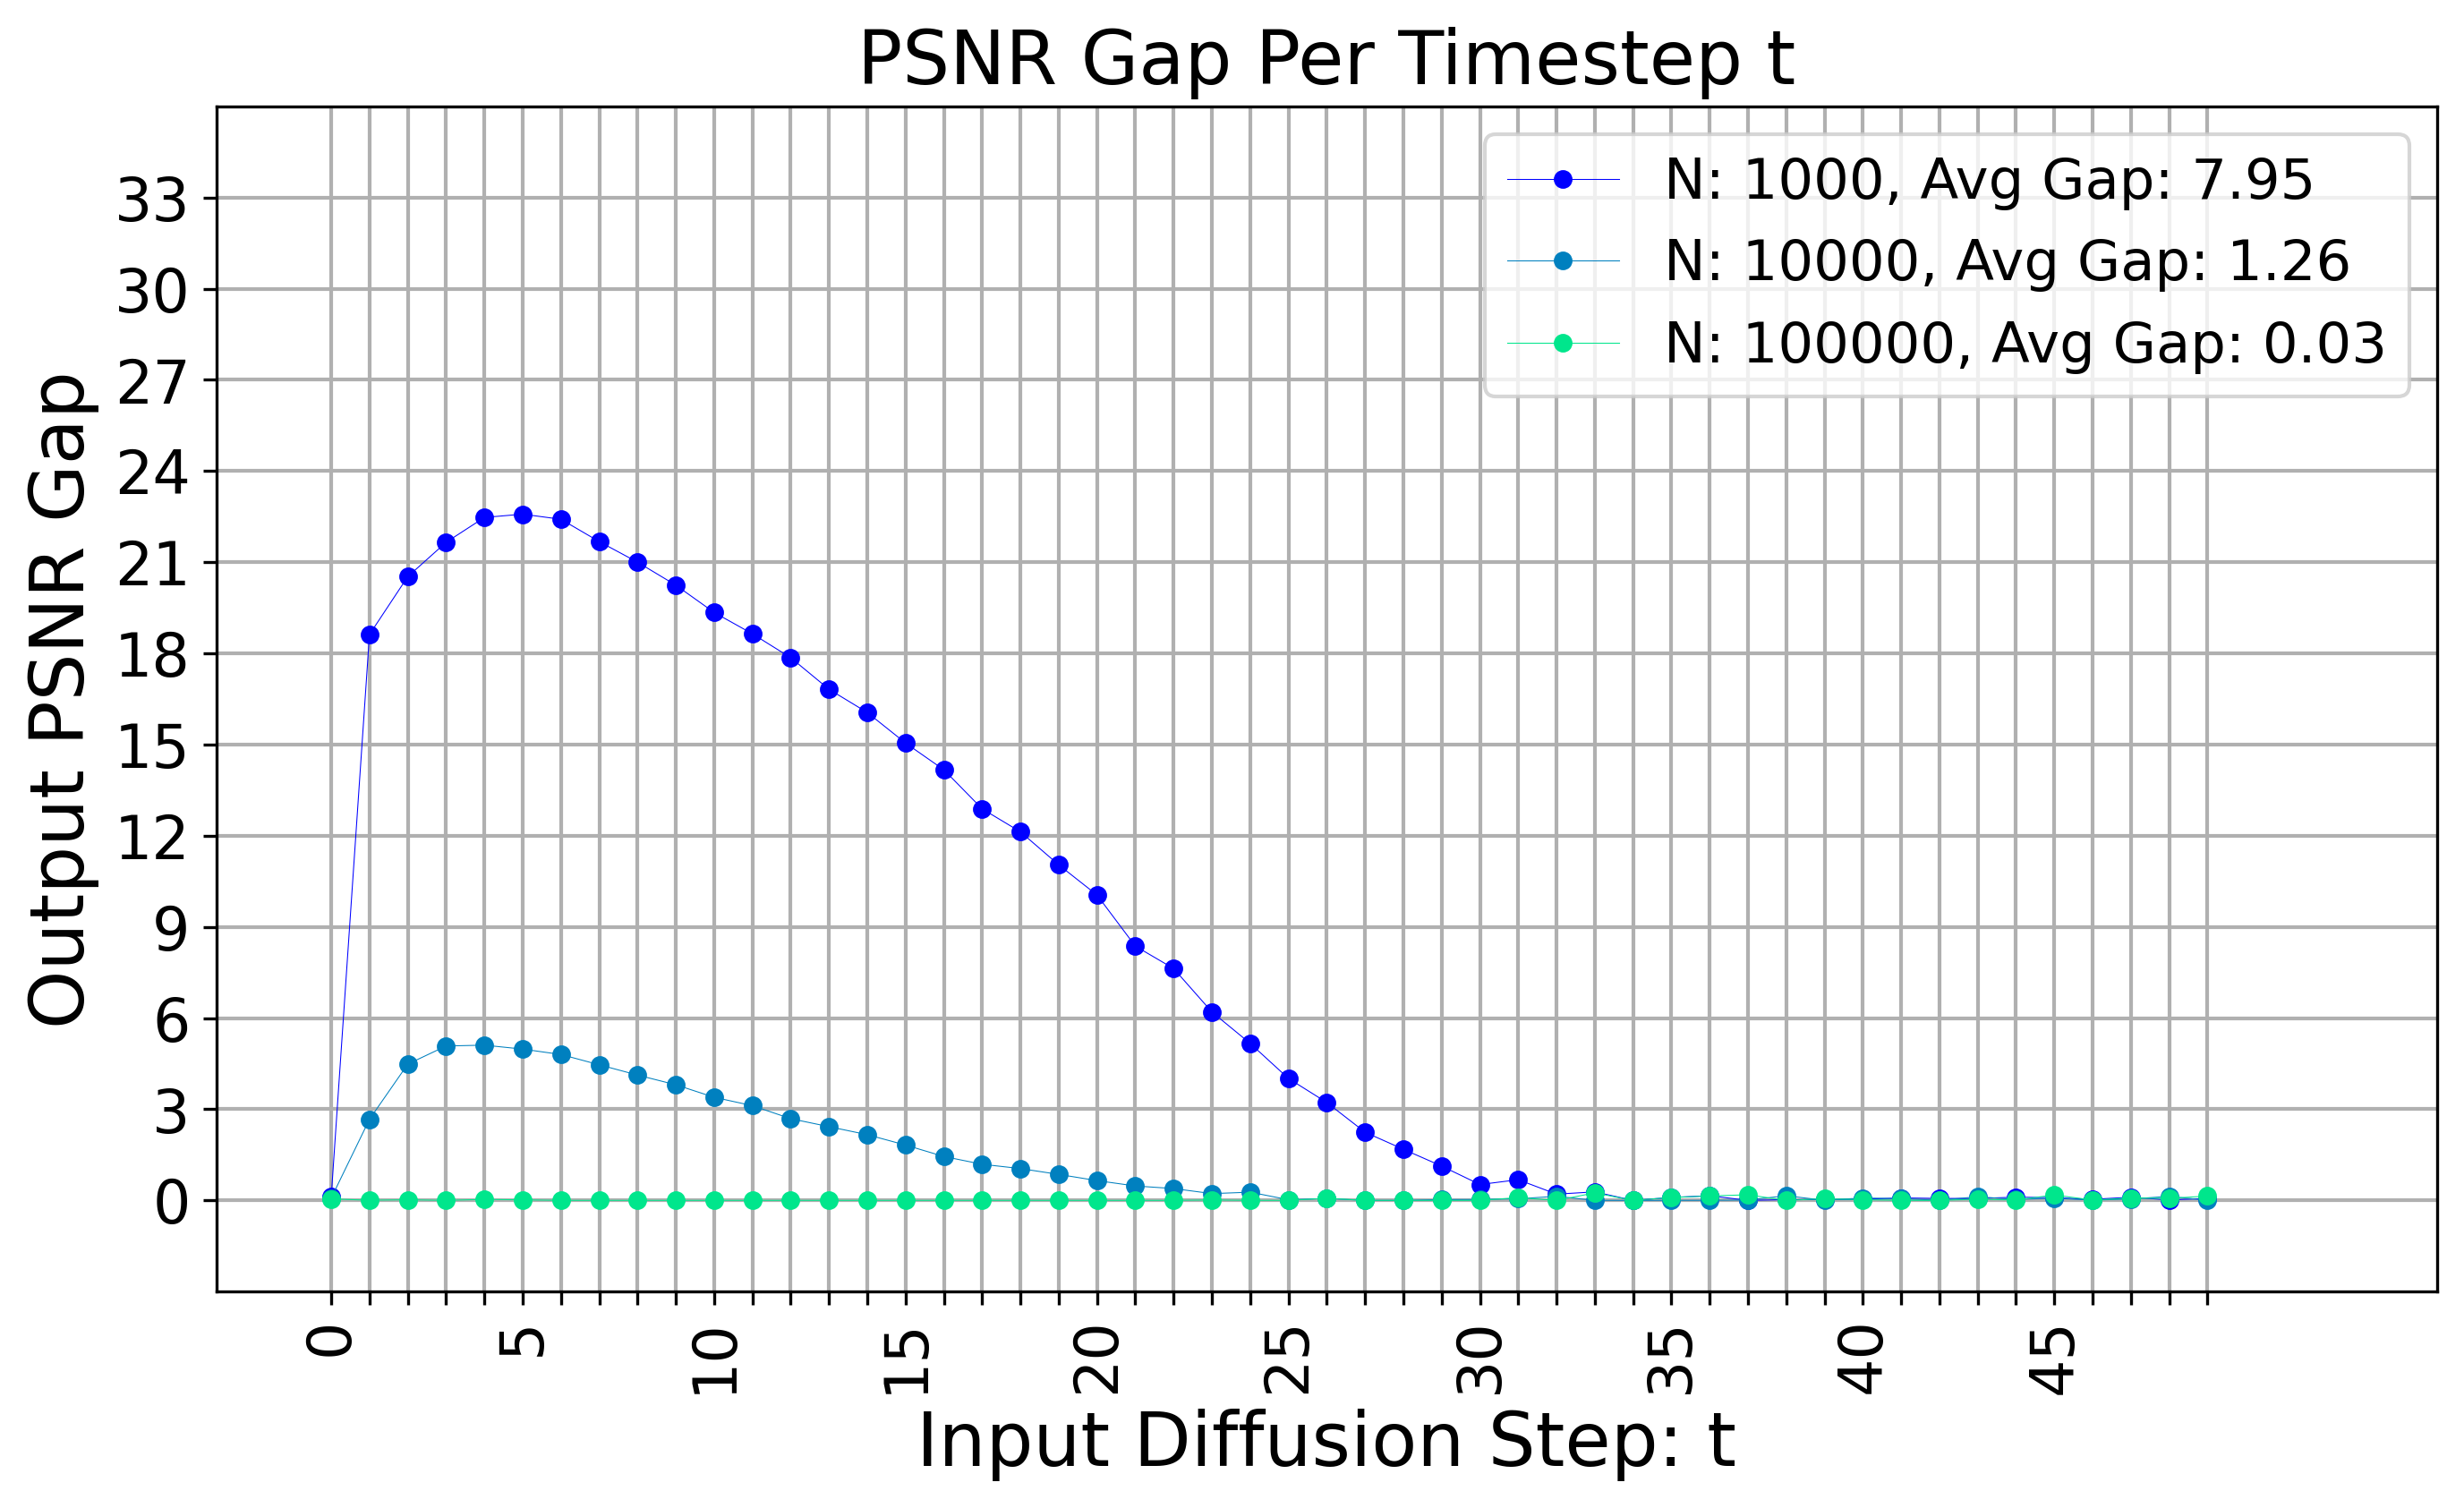}}
\\
&
\multicolumn{1}{c}{(a) PSNR Curves of Training and Testing Sets}
&
\multicolumn{1}{c}{(b) PSNR Gap}
\\
\end{tabular}

\captionof{figure}{The PSNR (a) and PSNR gap (b) comparison on the LSUN (Bridge)~\citep{yu15lsun} dataset.}
\label{fig:row_psnr_bridge}
\end{table}

\begin{table}[ht]
\centering
\small
\setlength\tabcolsep{1pt}
\setlength{\extrarowheight}{4pt}
\begin{tabular}{lc|c}
\cellcolor{dit}{\STAB{\rotatebox[origin=c]{90}{DiT-XS/1}}}
&
\raisebox{-0.5\height}{\includegraphics[width=.54\textwidth]{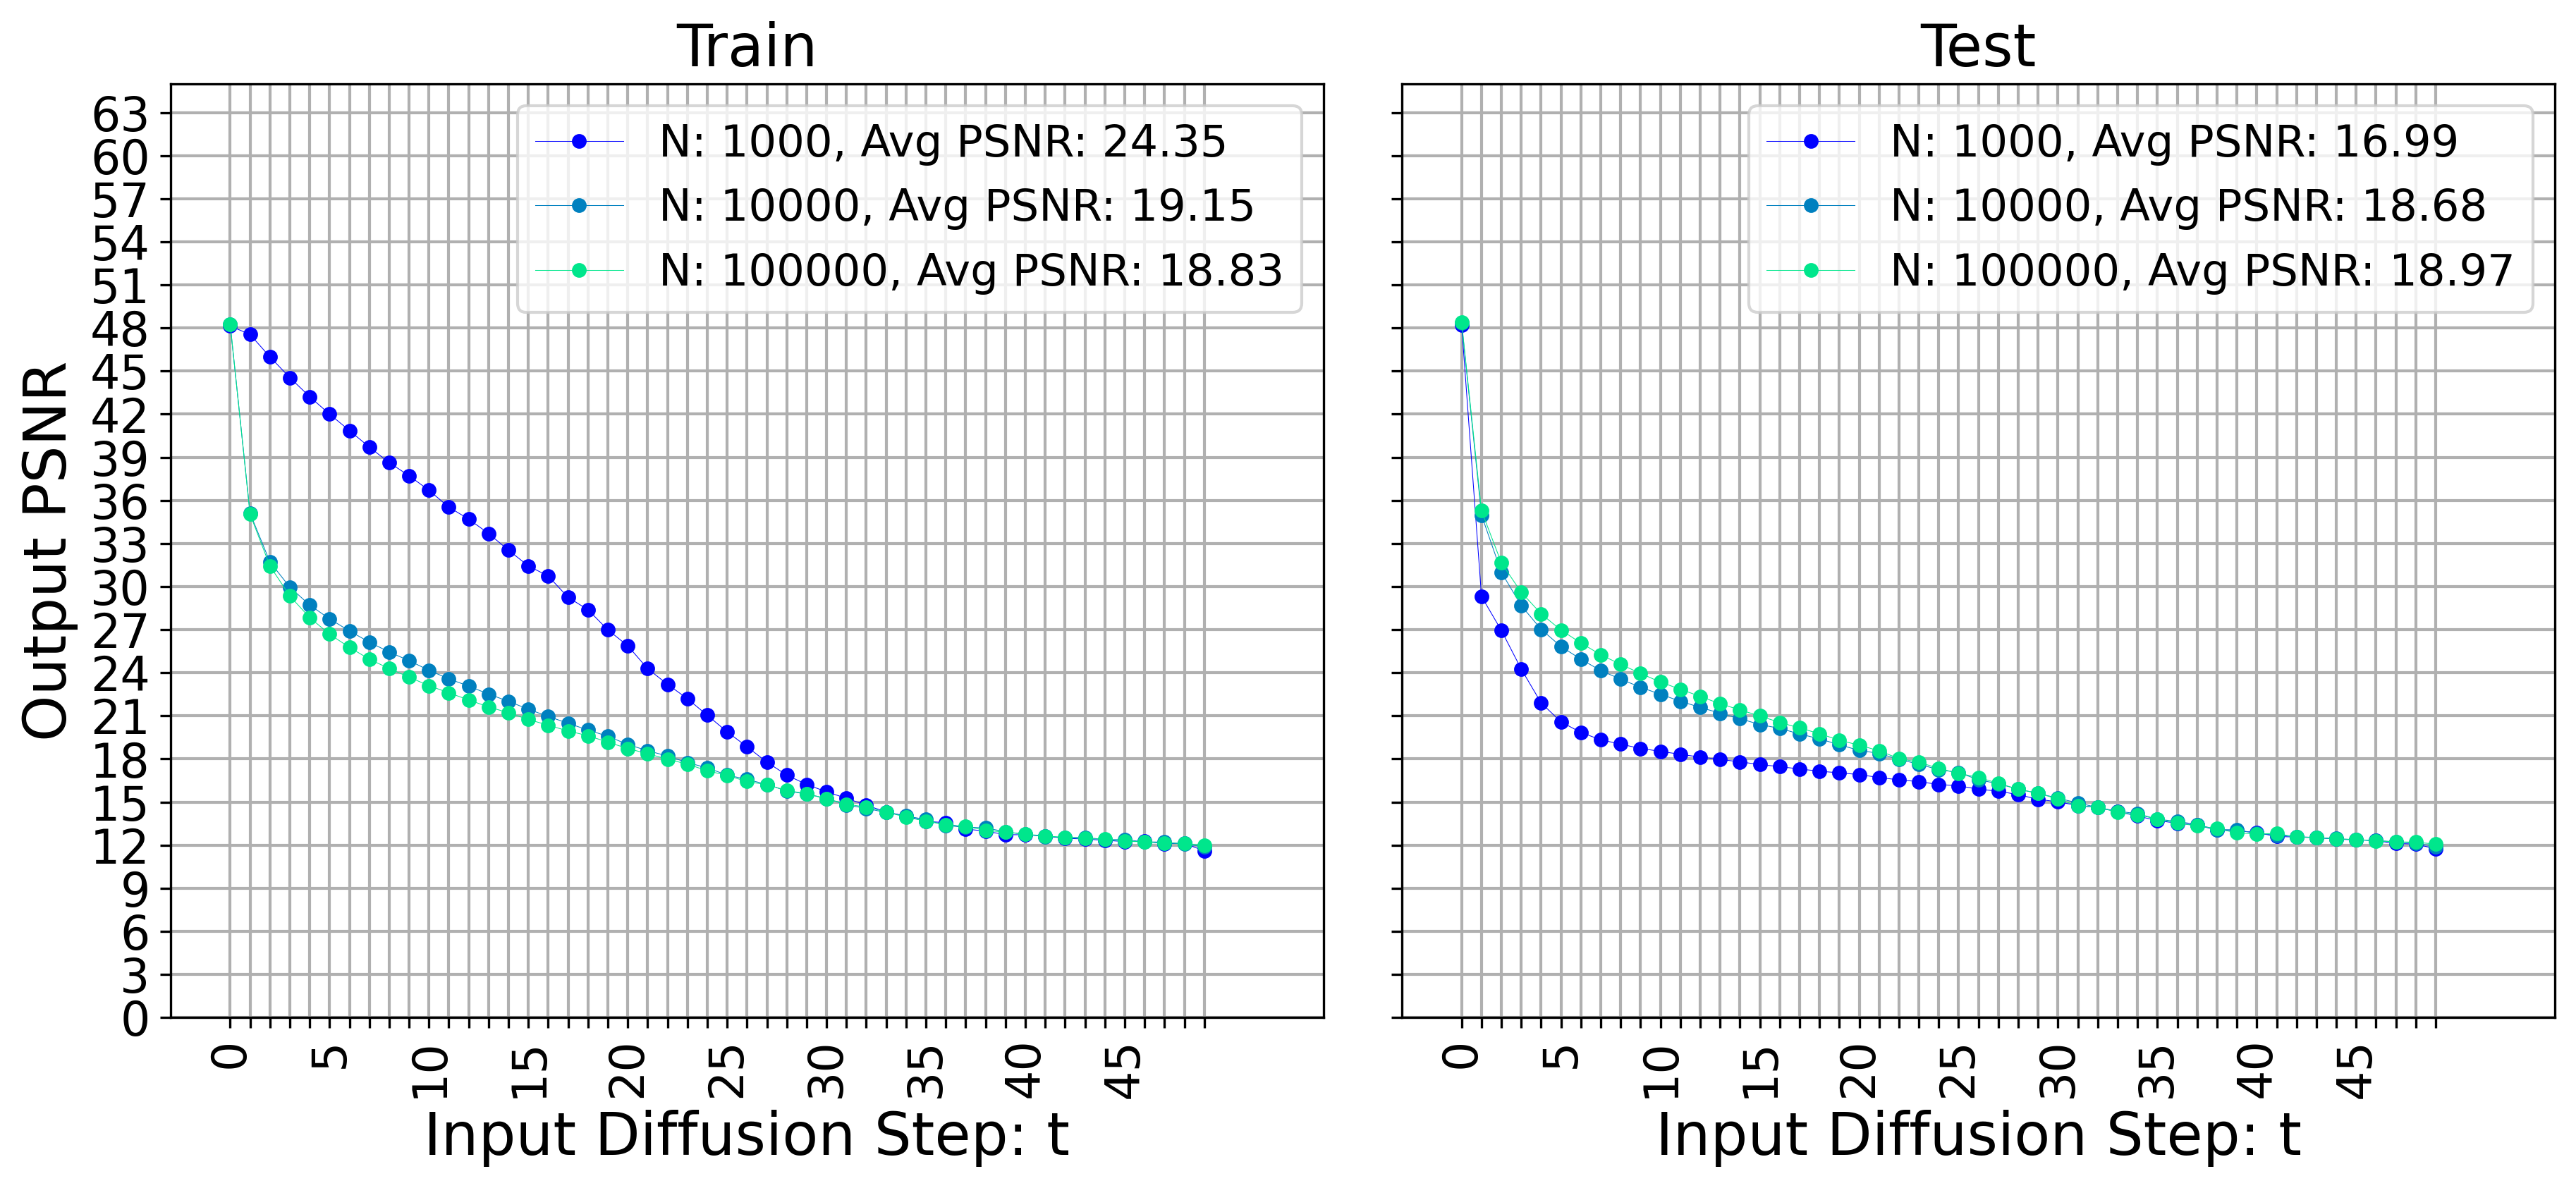}}
&
\raisebox{-0.5\height}{\includegraphics[width=.41\textwidth]{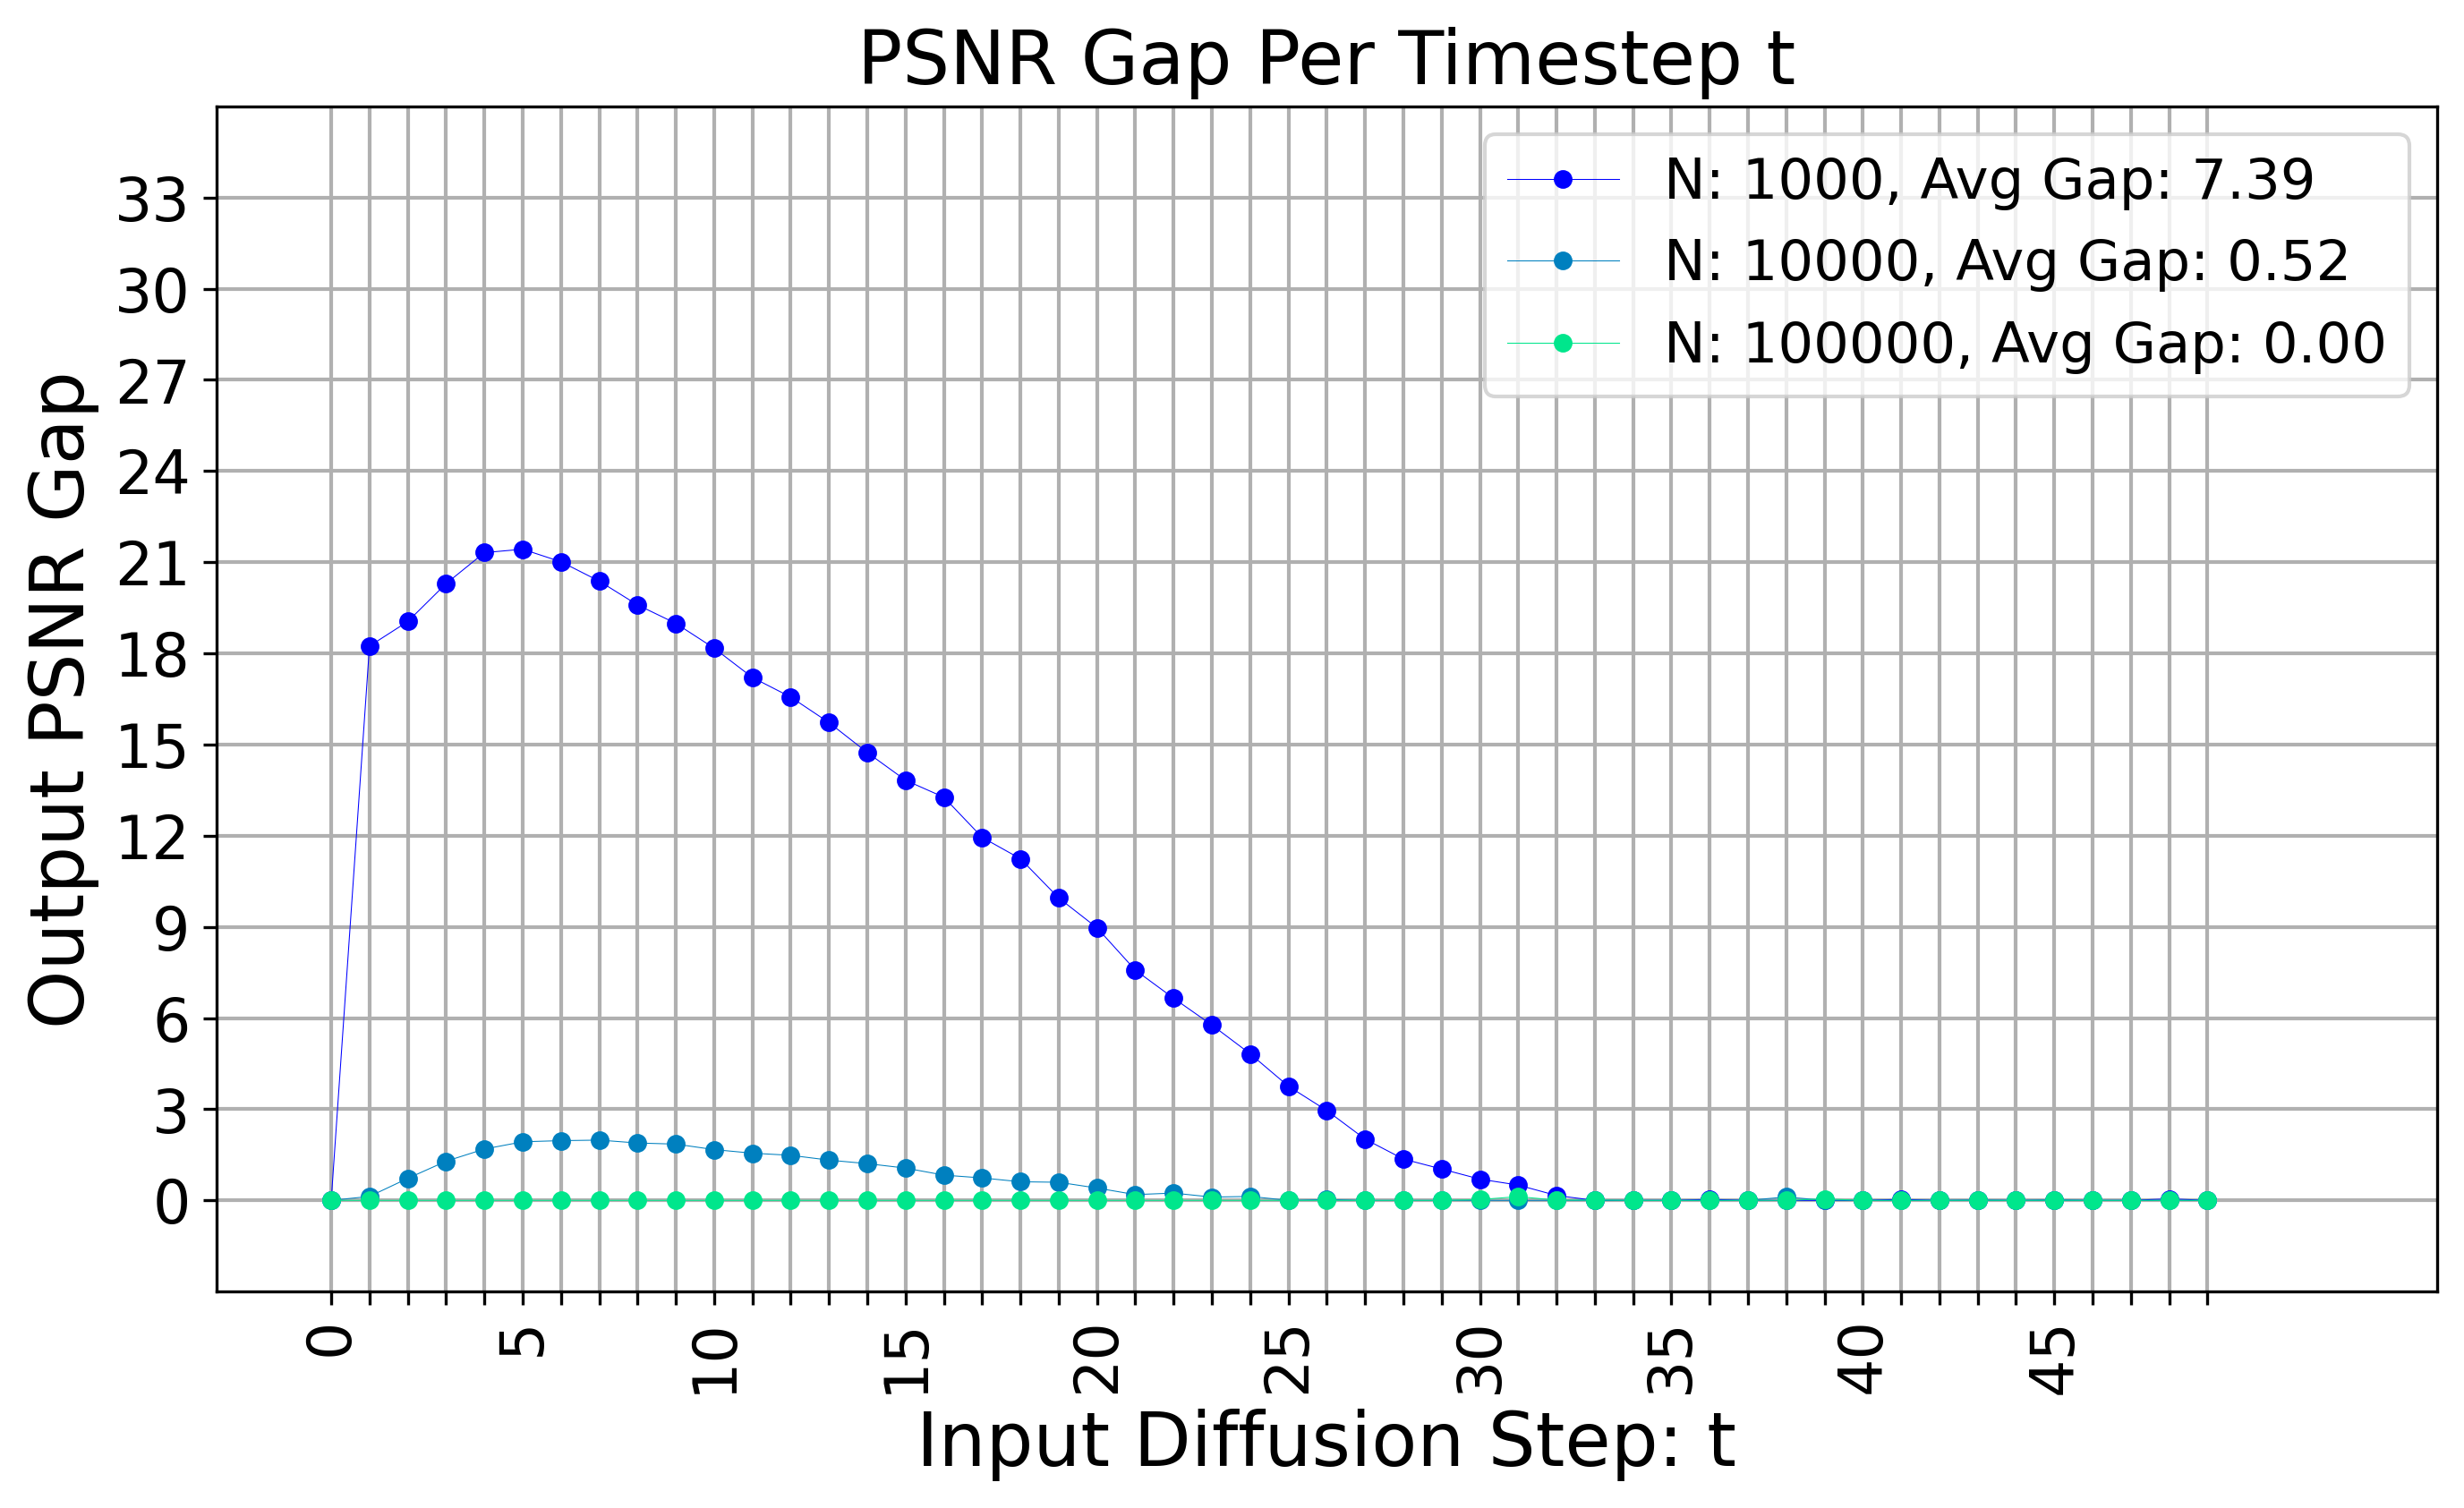}}
\\
\hline
\cellcolor{diff}{\STAB{\rotatebox[origin=c]{90}{DiT-XS/1 w/ Local}}}
&
\raisebox{-0.5\height}{\includegraphics[width=.54\textwidth]{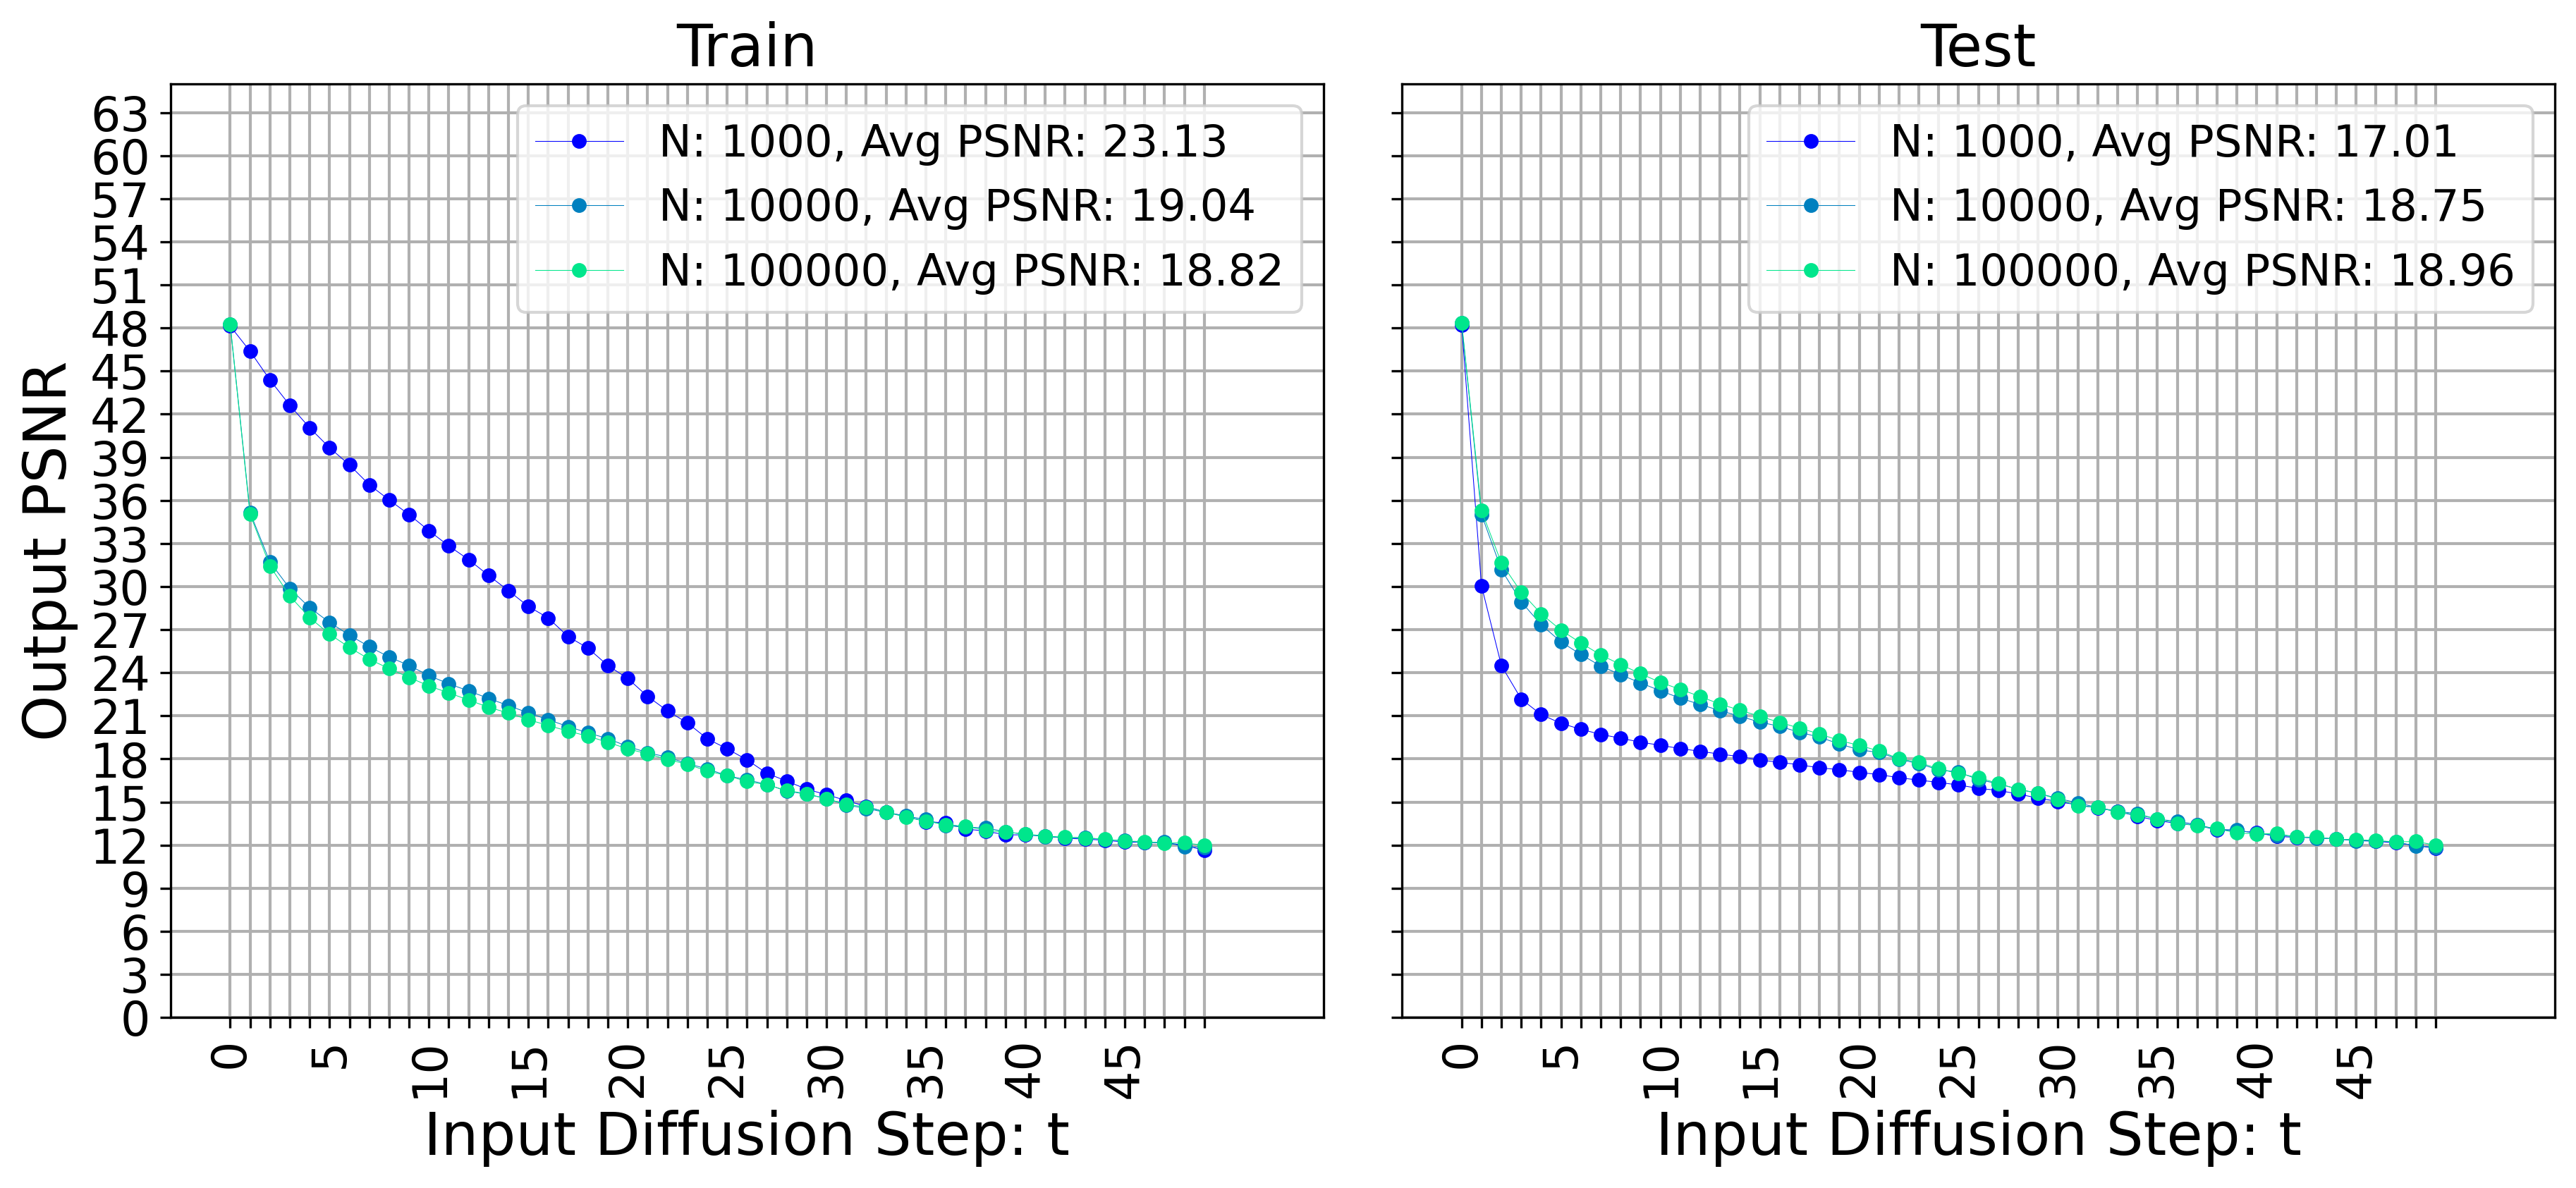}}
&
\raisebox{-0.5\height}{\includegraphics[width=.41\textwidth]{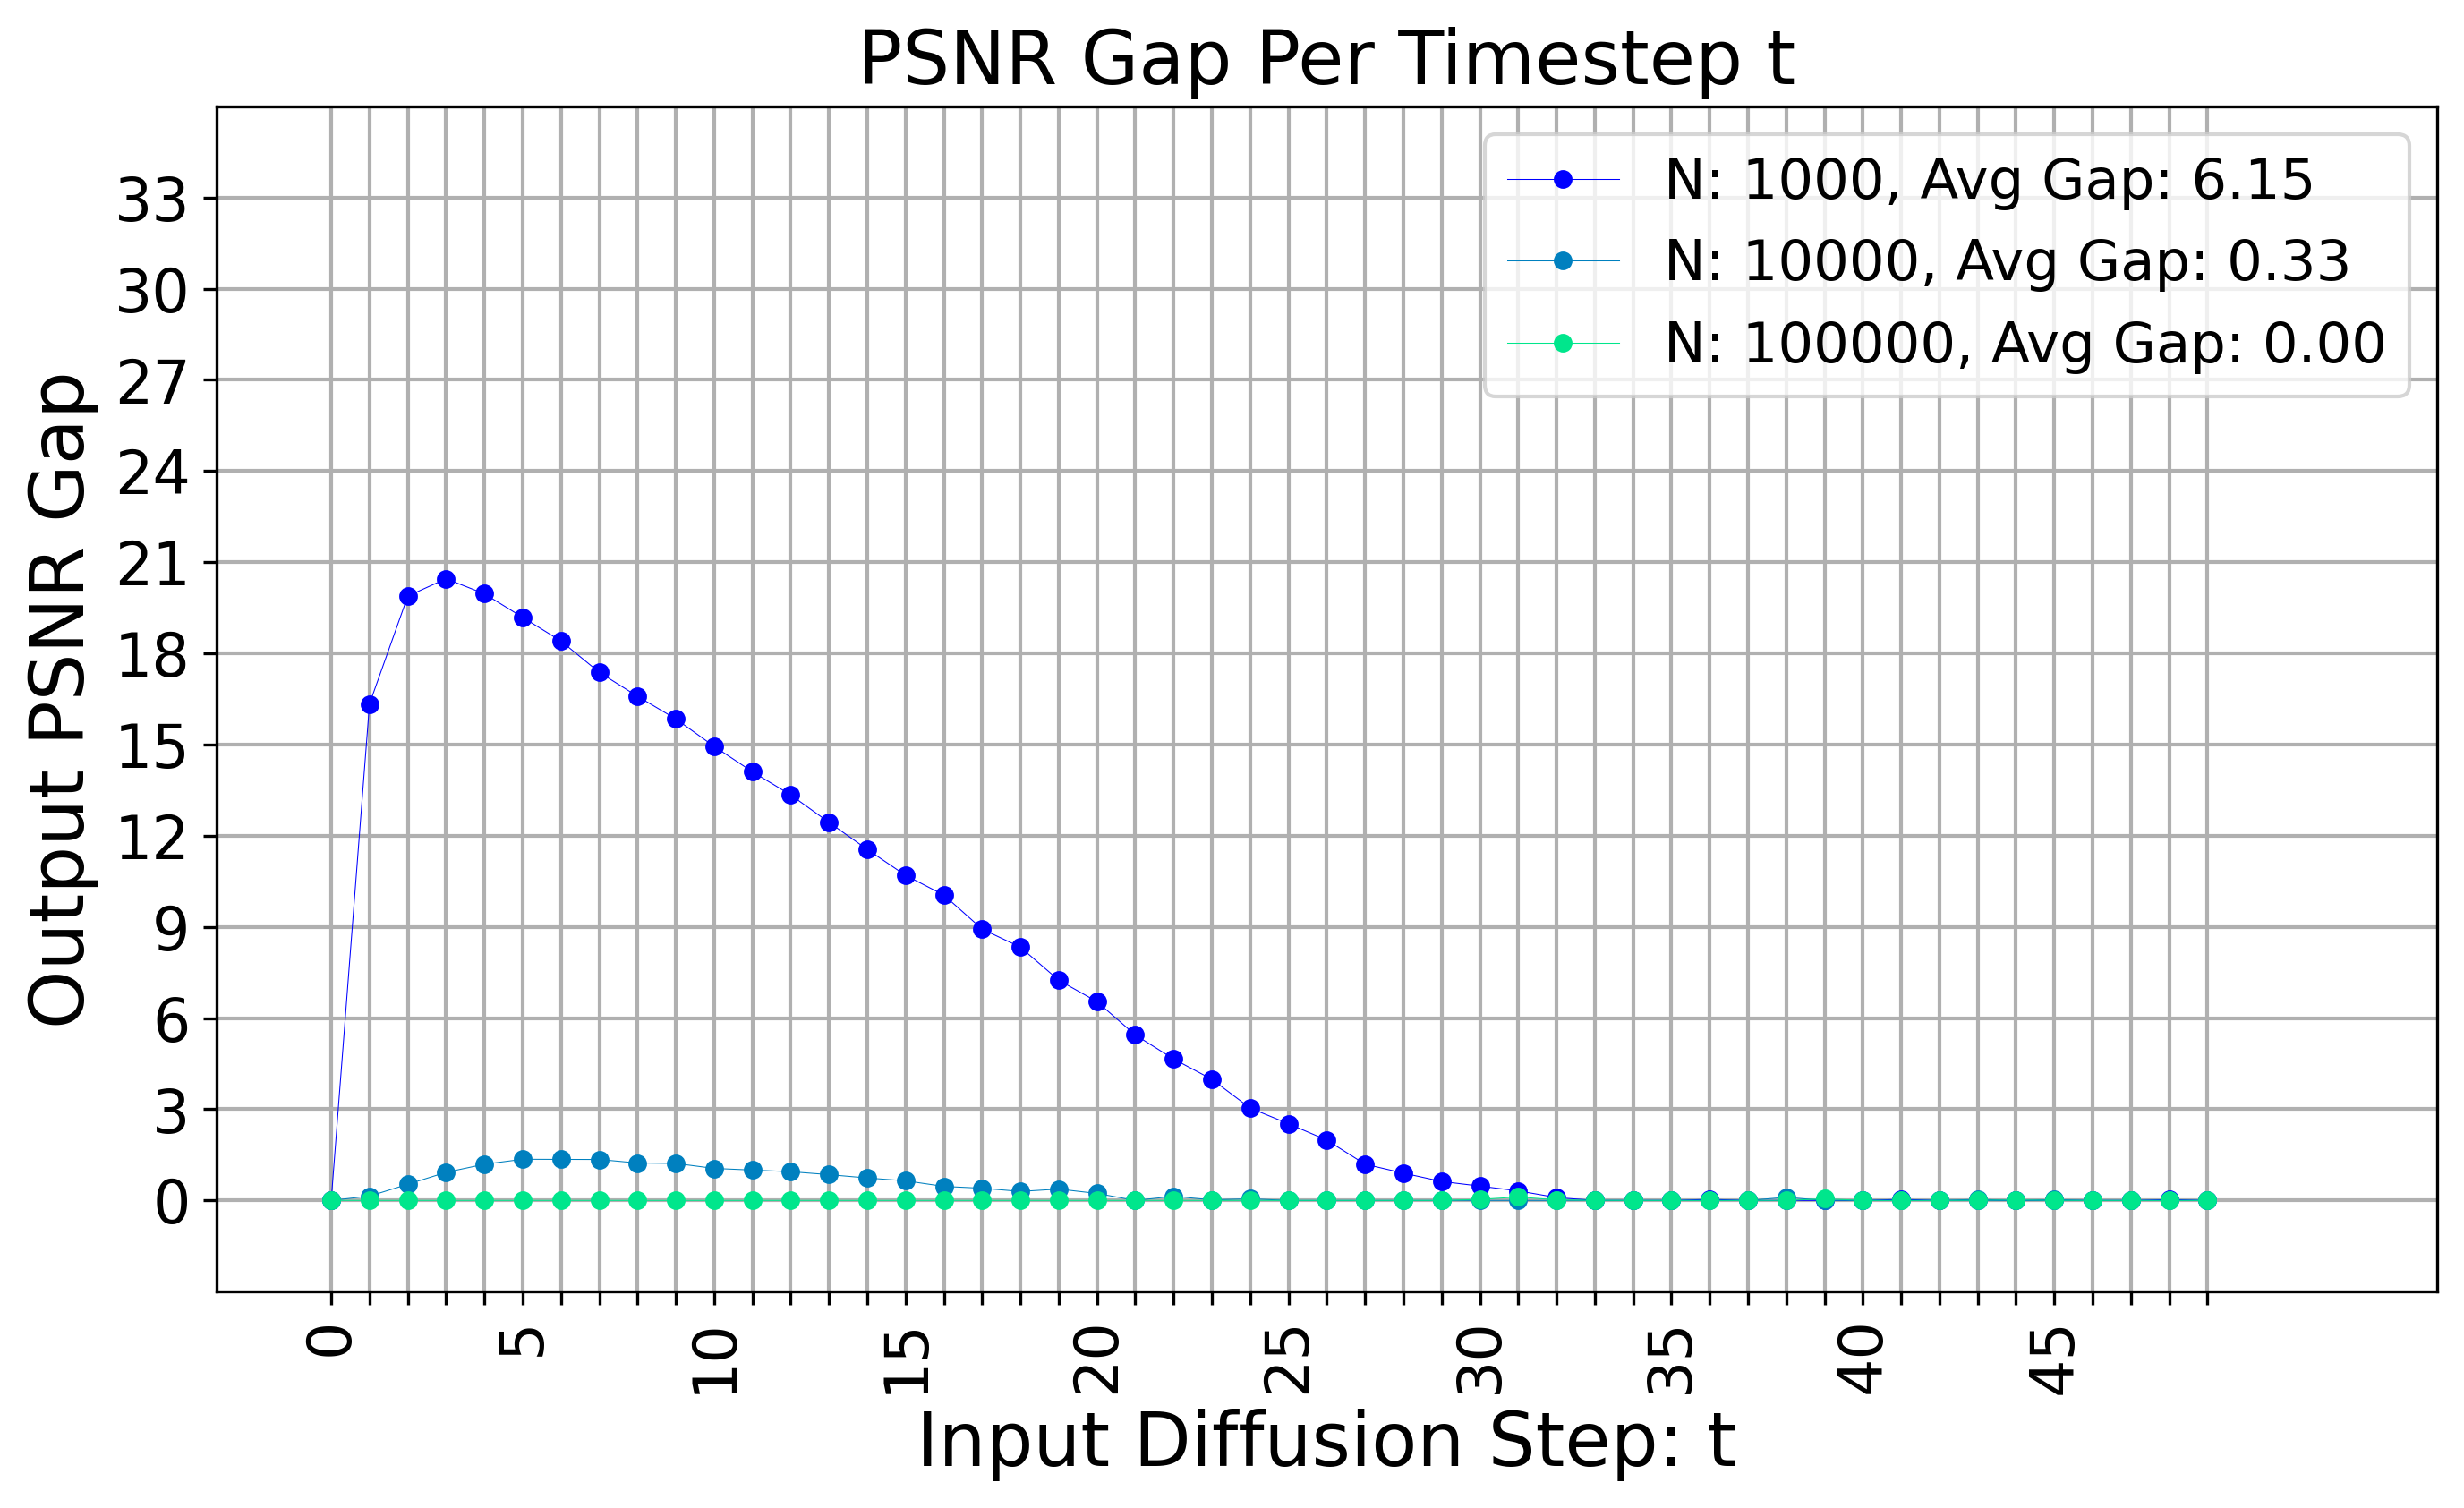}}
\\
\hline
\cellcolor{dit}{\STAB{\rotatebox[origin=c]{90}{DiT-S/1}}}
&
\raisebox{-0.5\height}{\includegraphics[width=.54\textwidth]{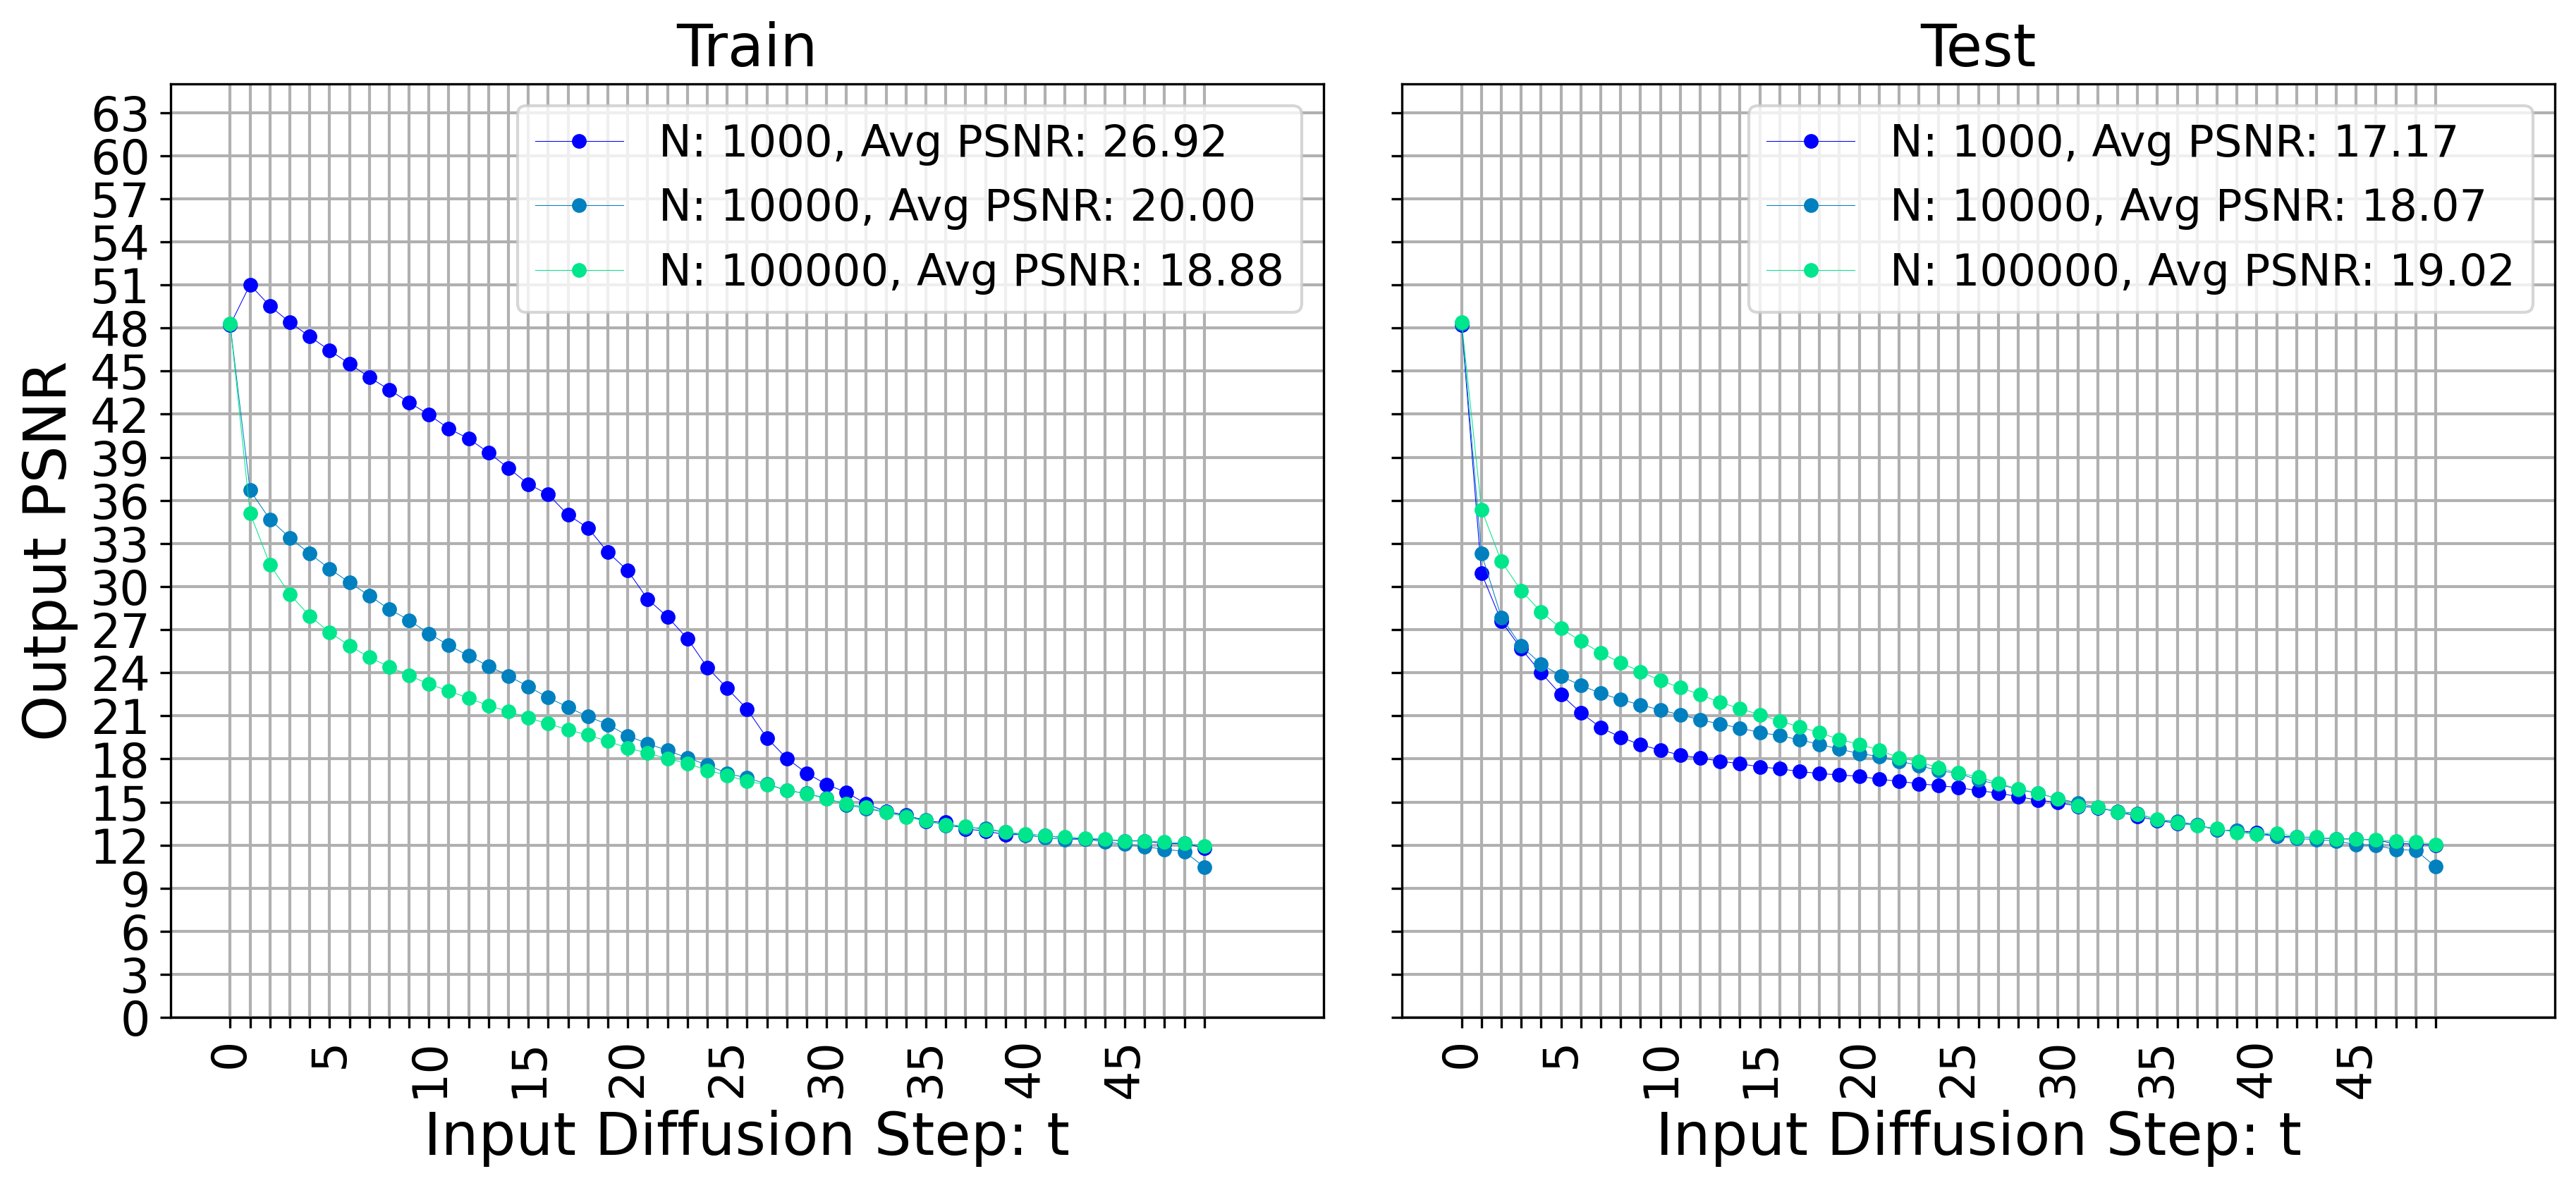}}
&
\raisebox{-0.5\height}{\includegraphics[width=.41\textwidth]{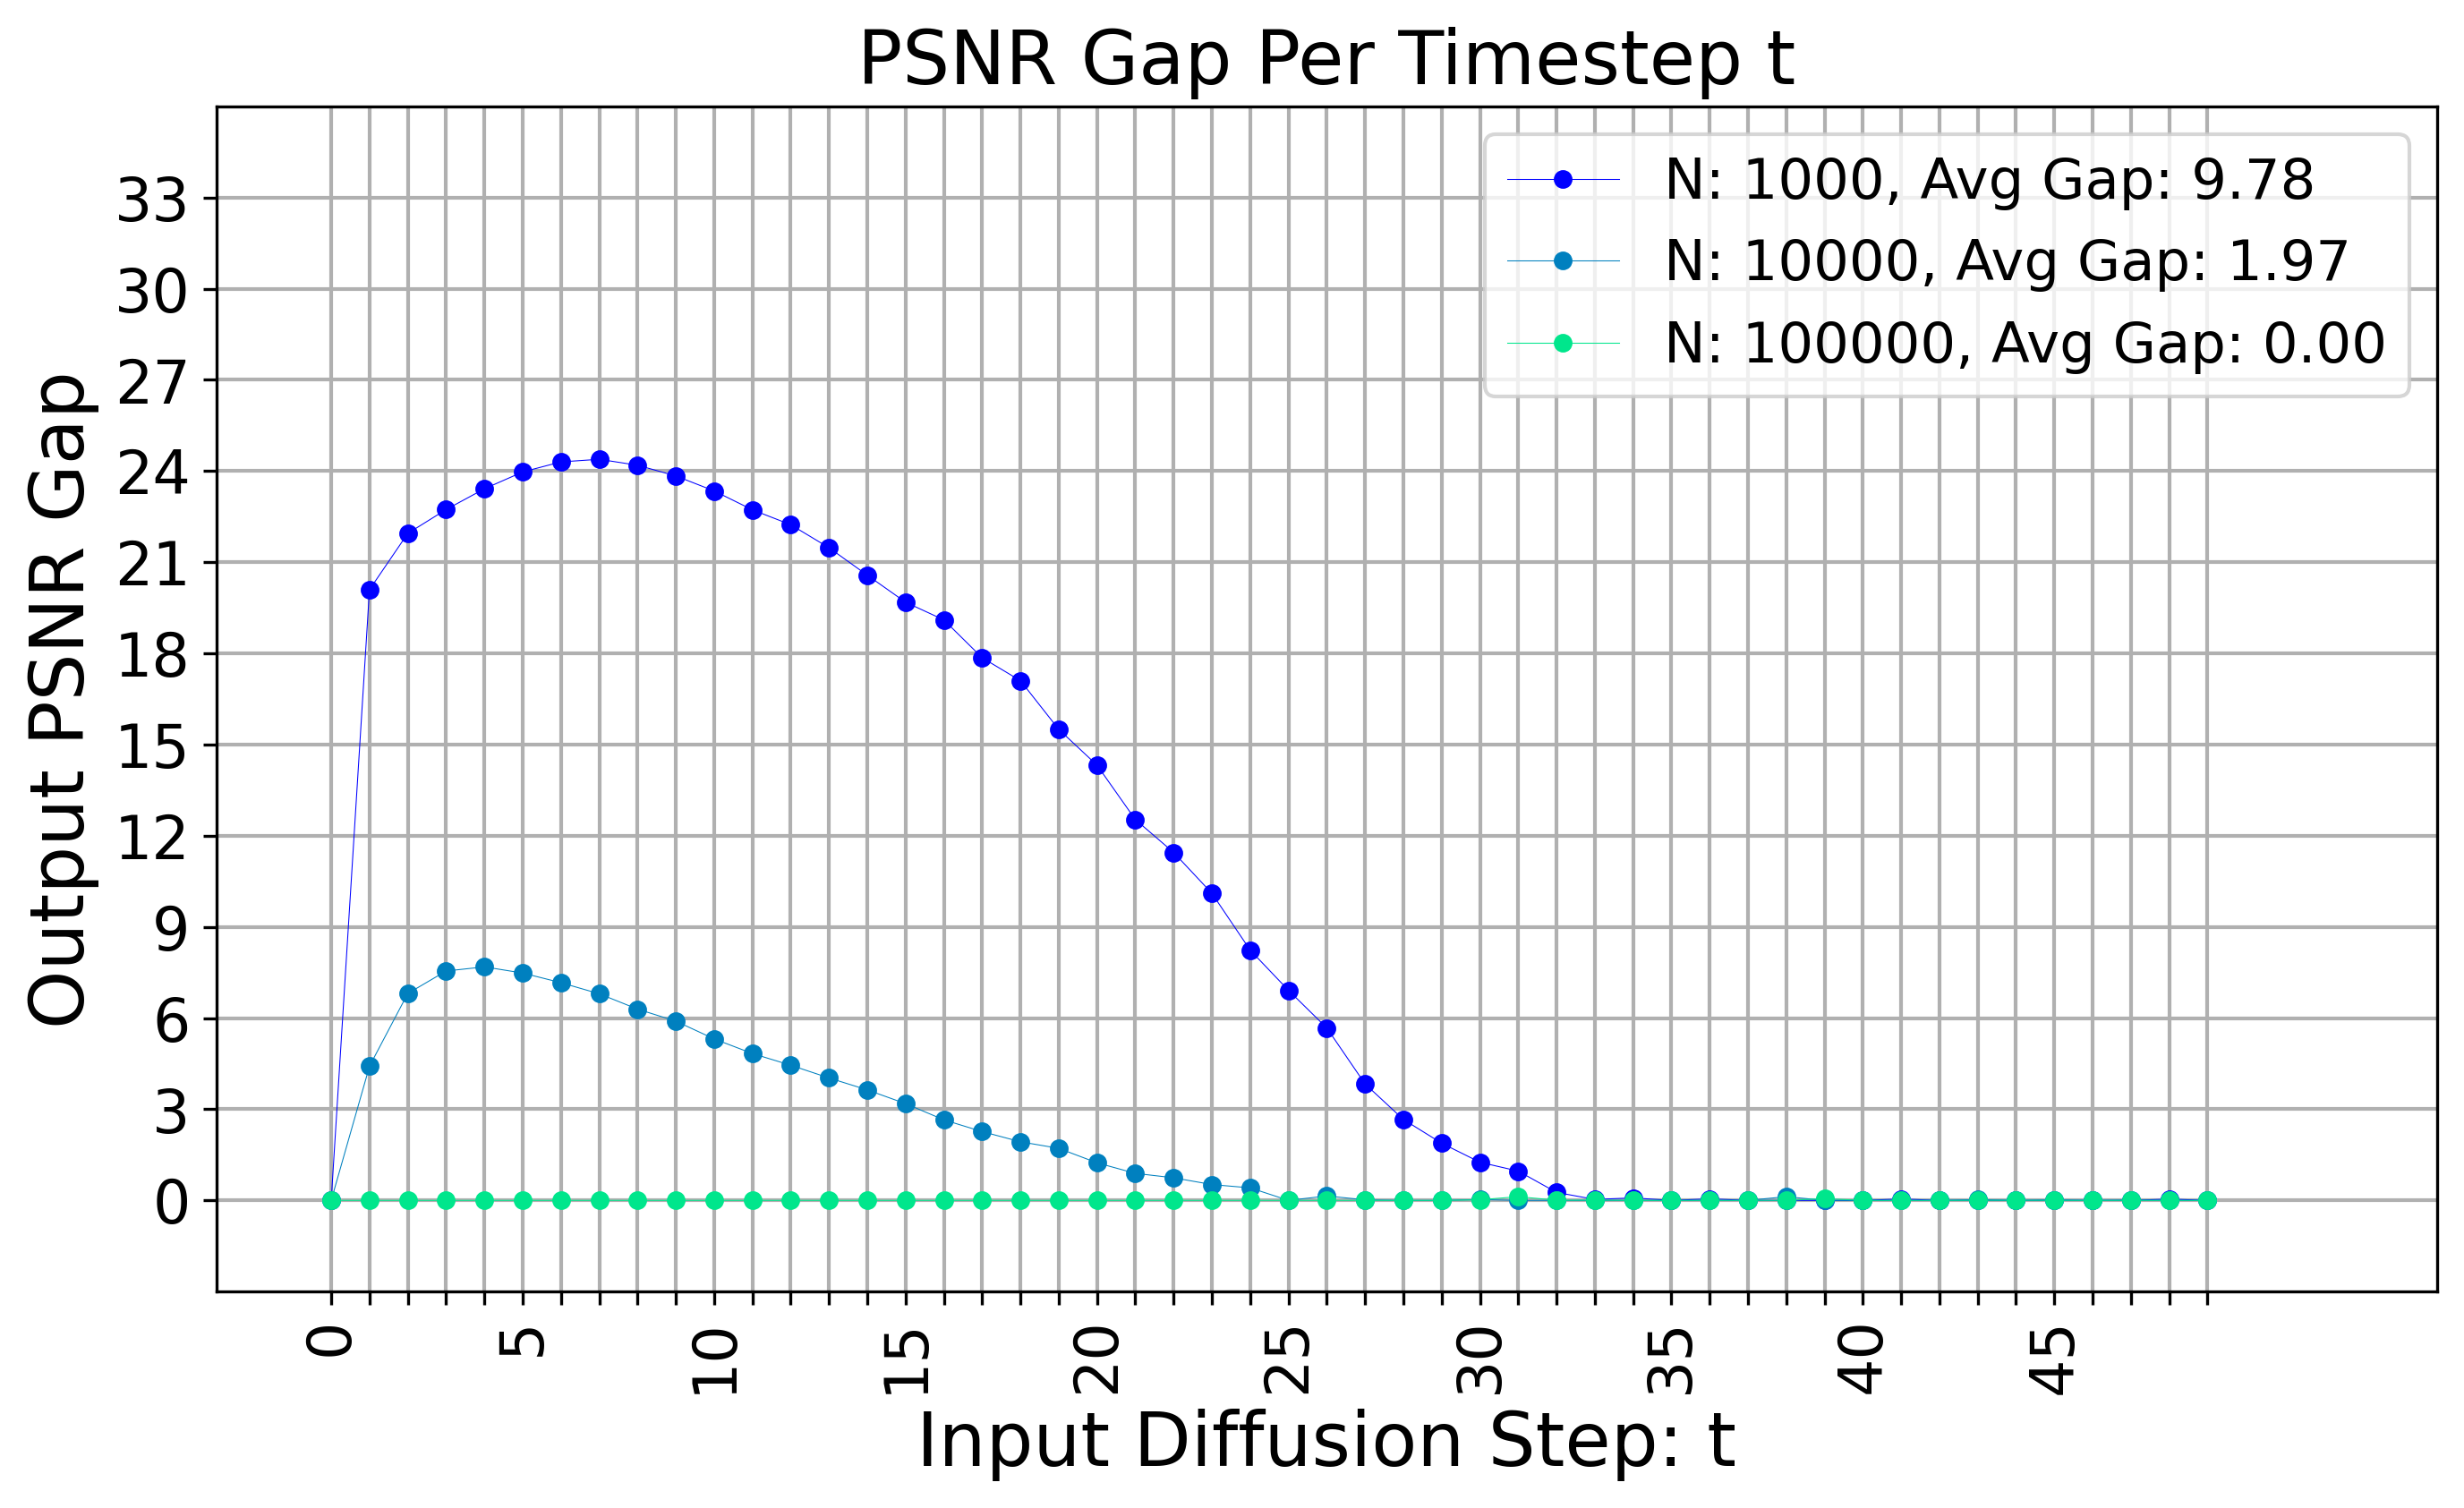}}
\\
\hline
\cellcolor{diff}{\STAB{\rotatebox[origin=c]{90}{DiT-S/1 w/ Local}}}
&
\raisebox{-0.5\height}{\includegraphics[width=.54\textwidth]{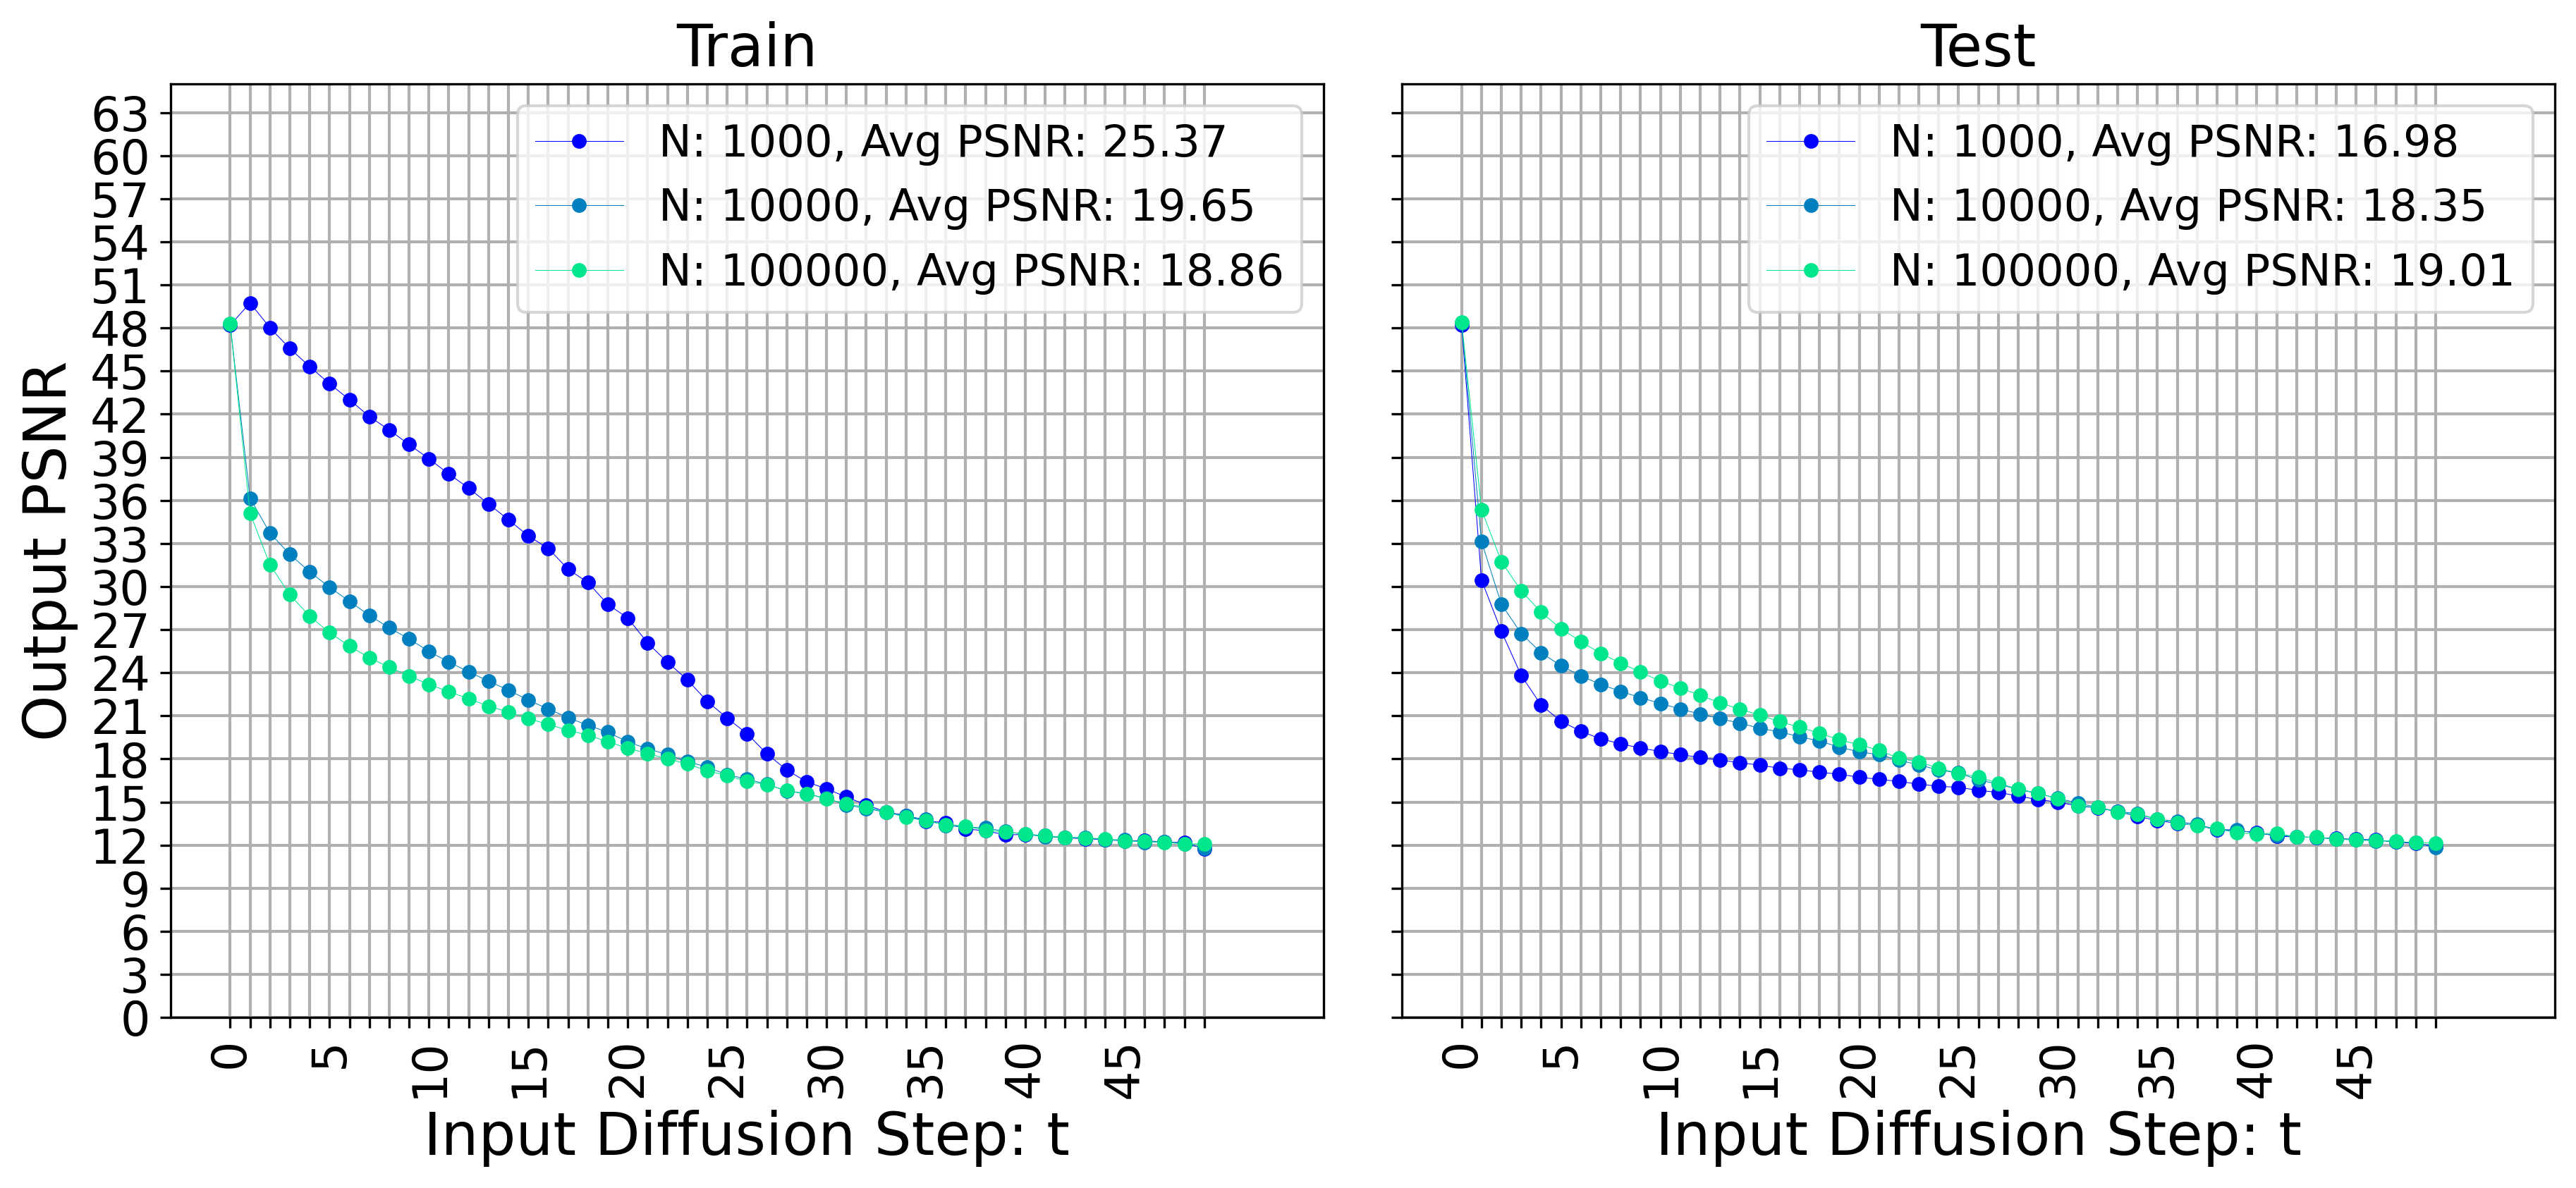}}
&
\raisebox{-0.5\height}{\includegraphics[width=.41\textwidth]{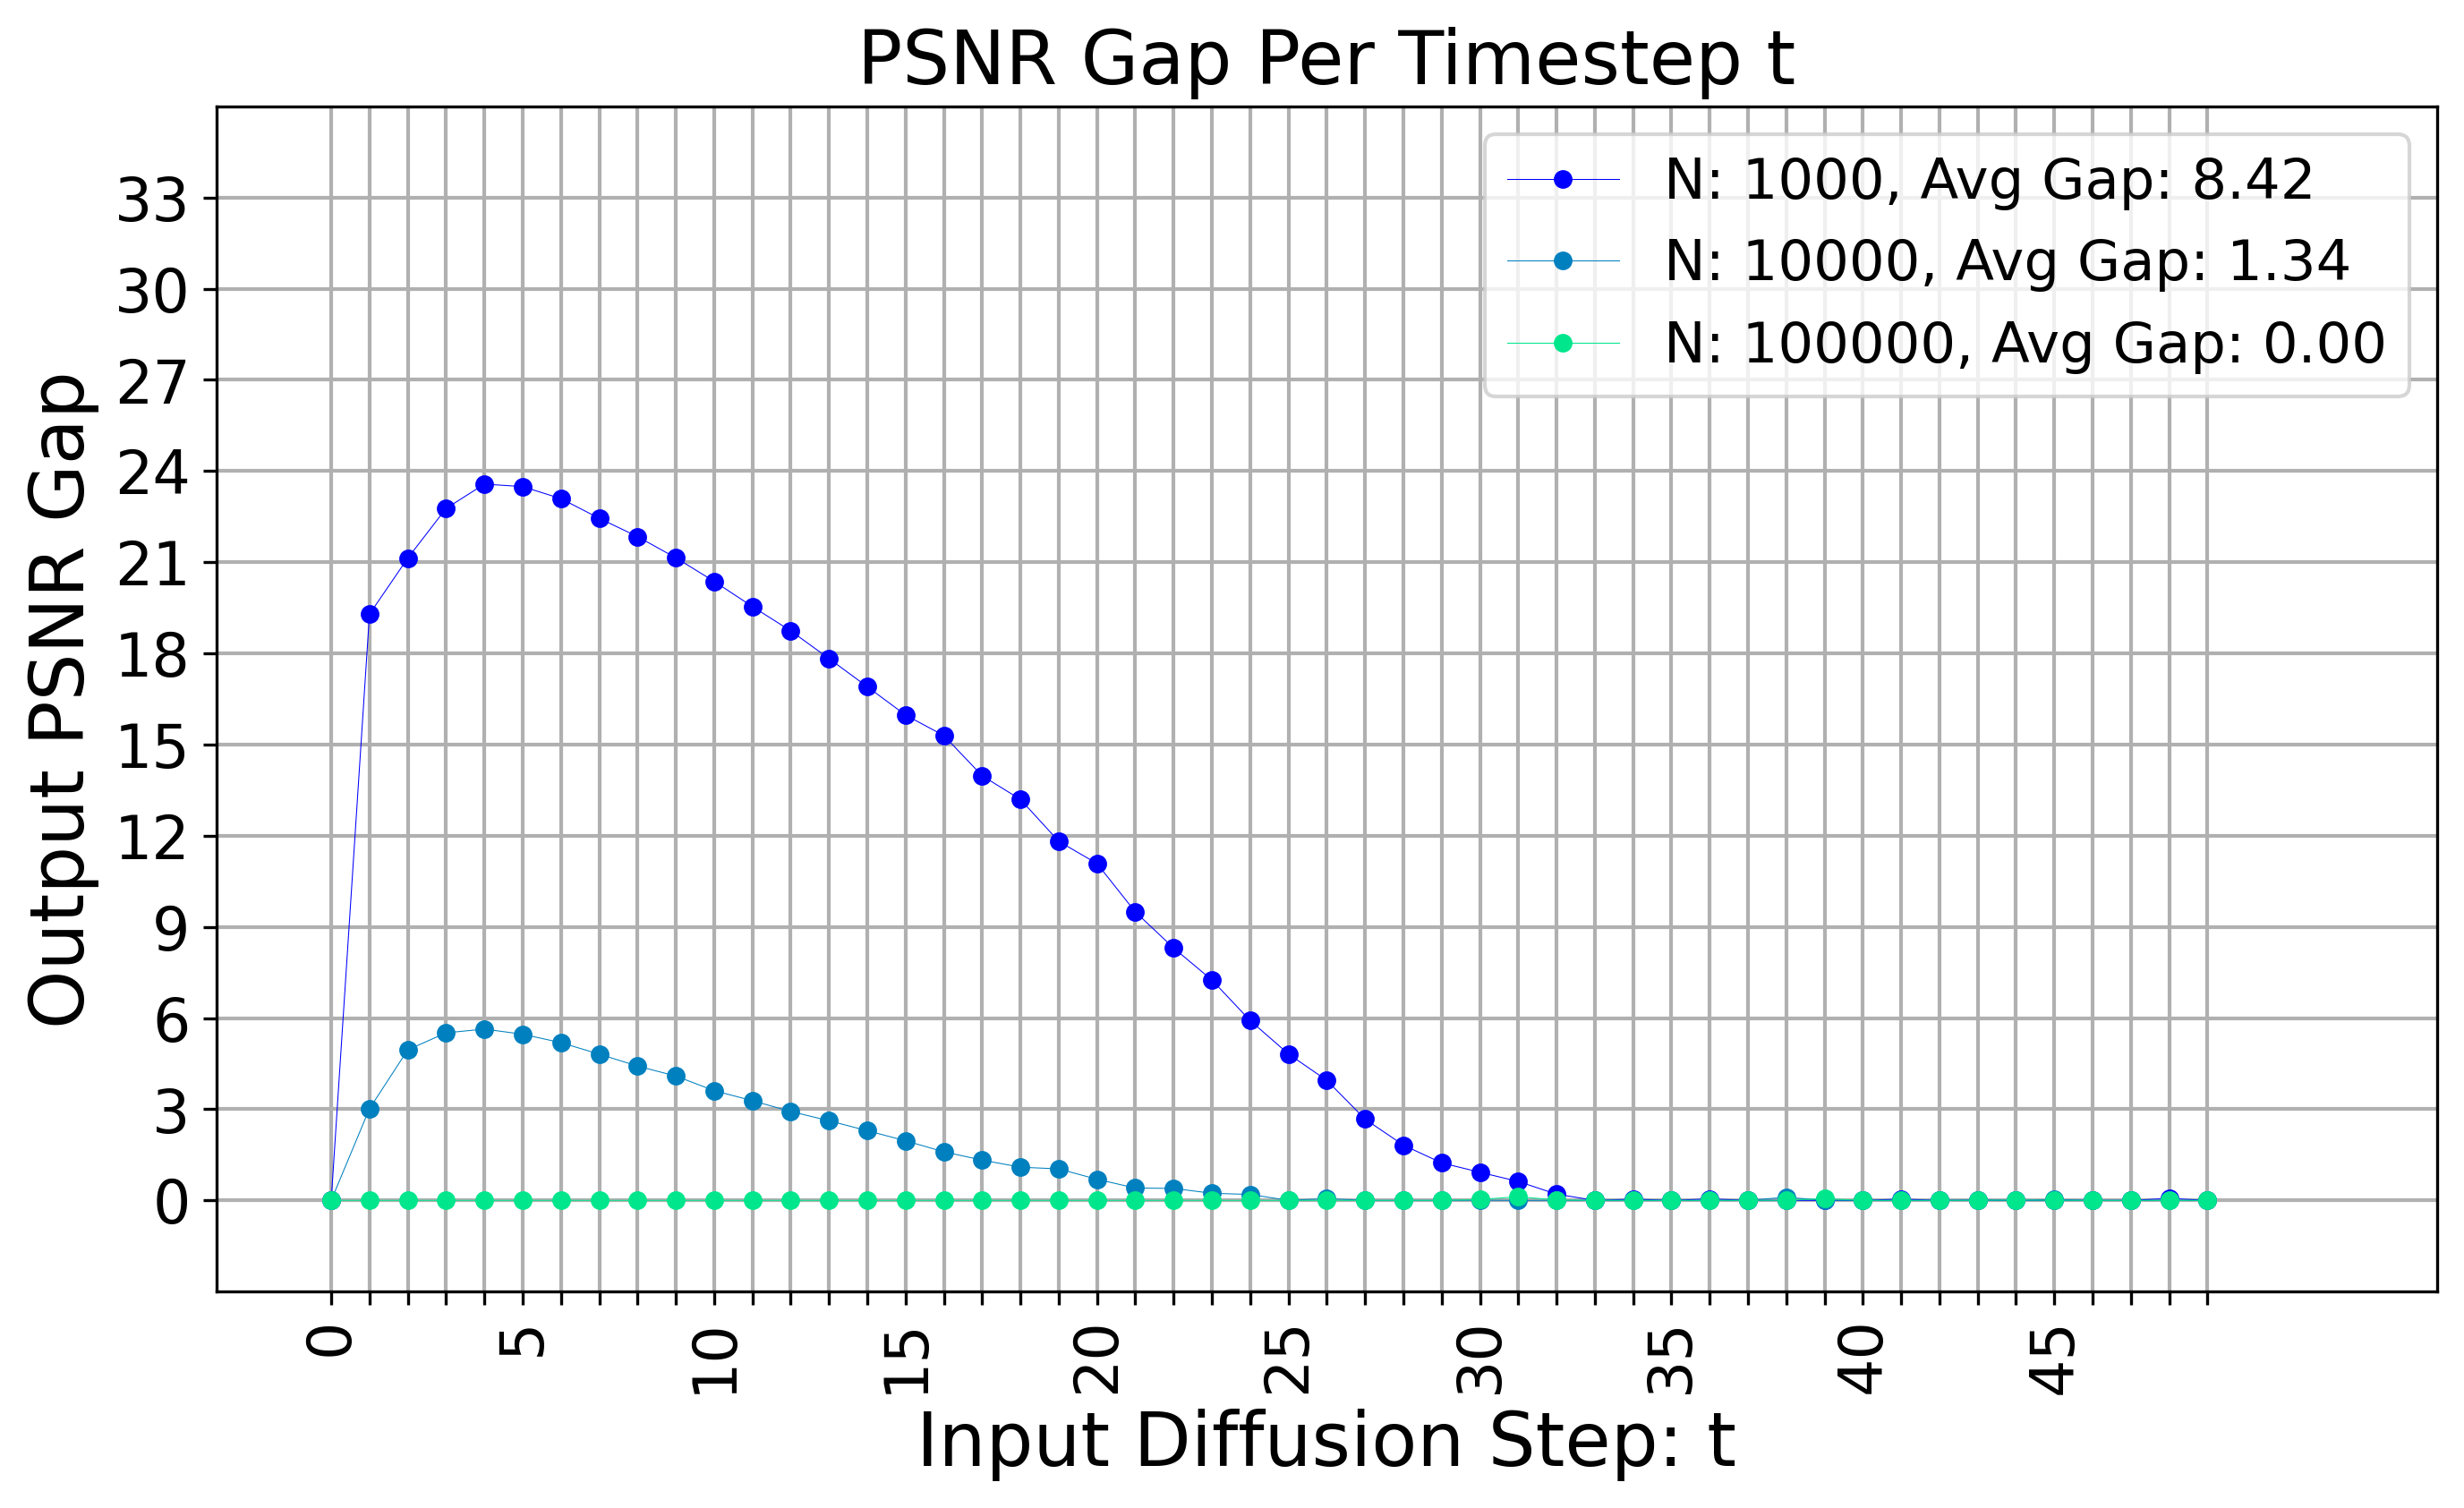}}
\\
&
\multicolumn{1}{c}{(a) PSNR Curves of Training and Testing Sets}
&
\multicolumn{1}{c}{(b) PSNR Gap}
\\
\end{tabular}

\captionof{figure}{The PSNR (a) and PSNR gap (b) comparison on the LSUN (Tower)~\citep{yu15lsun} dataset.}
\label{fig:row_psnr_tower}
\end{table}
